# Supplementary material for: El Agente Estructural: An Artificially Intelligent Molecular Editor
Source: arXiv:2602.04849 source file (2026-11-30)
Supplement: Supplementary file 1 [file MoPNP.tex]

\setlength{\parindent}{5pt} \textbf{\textcolor{blue}{User:}}
\begin{tcolorbox}[
    colback=blue!10,
    colframe=blue,
    width=\textwidth,
    arc=2mm,
    boxrule=0.2mm,
    leftrule=0.2mm, rightrule=0.2mm,
    toprule=0.2mm, bottomrule=0.2mm,
    enhanced,
    breakable
]
\begin{markdown}
Given MoCl3PNP.xyz, the PNP ligand is 2,6-bis(di-tert-butylphosphinomethyl)pyridine.
Find all t-butyl groups attached to the phosphorus atoms. Replace them with hydrogen, methyl, and phenyl, creating separate XYZ files for each replacement.
\end{markdown}
\end{tcolorbox}
\setlength{\parindent}{5pt} \robot \hspace{2pt} \textbf{Estructural}

\begin{tcolorbox}[
    colback=matterbg2,
    colframe=mattergreen1,
    width=\textwidth,
    arc=2mm,
    boxrule=0.2mm,
    leftrule=0.2mm, rightrule=0.2mm,
    toprule=0.2mm, bottomrule=0.2mm,
    enhanced,
    breakable
]
\textbf{Tool used:}

\setlength{\parindent}{5pt}\underline{\texttt{Tool Name:}} \texttt{repl\_tool}\par
\setlength{\parindent}{5pt}\underline{\texttt{Arguments:}}\par
\setlength{\parindent}{10pt}\texttt{code =}\par
\begin{verbatim}
import os
import shutil

project_dir = 'MoCl3PNP_derivatives_project'
if not os.path.exists(project_dir):
    os.makedirs(project_dir)

src = 'MoCl3PNP.xyz'
dst = os.path.join(project_dir, 'MoCl3PNP.xyz')
if os.path.exists(src):
    shutil.copy(src, dst)
    print(f"Copied {src} to {dst}")
else:
    print(f"{src} not found")
\end{verbatim}\par
\smallskip
\setlength{\parindent}{5pt}\underline{\texttt{Tool Name:}} \texttt{get\_atomic\_neighbors}\par
\setlength{\parindent}{5pt}\underline{\texttt{Arguments:}}\par
\setlength{\parindent}{10pt}\texttt{target = P}\par
\setlength{\parindent}{10pt}\texttt{file\_path = MoCl3PNP\_derivatives\_project/MoCl3PNP.xyz}\par
\smallskip
\end{tcolorbox}

\setlength{\parindent}{5pt} \robot \hspace{2pt} \textbf{Estructural}

\begin{tcolorbox}[
    colback=matterbg2,
    colframe=mattergreen1,
    width=\textwidth,
    arc=2mm,
    boxrule=0.2mm,
    leftrule=0.2mm, rightrule=0.2mm,
    toprule=0.2mm, bottomrule=0.2mm,
    enhanced,
    breakable
]
\textbf{Tool used:}

\setlength{\parindent}{5pt}\underline{\texttt{Tool Name:}} \texttt{get\_atomic\_neighbors}\par
\setlength{\parindent}{5pt}\underline{\texttt{Arguments:}}\par
\setlength{\parindent}{10pt}\texttt{target = P}\par
\setlength{\parindent}{10pt}\texttt{file\_path = MoCl3PNP.xyz}\par
\smallskip
\setlength{\parindent}{5pt}\underline{\texttt{Tool Name:}} \texttt{repl\_tool}\par
\setlength{\parindent}{5pt}\underline{\texttt{Arguments:}}\par
\setlength{\parindent}{10pt}\texttt{code =}\par
\begin{verbatim}
import os
print(os.listdir('MoCl3PNP_derivatives_project'))
\end{verbatim}\par
\smallskip
\end{tcolorbox}

\setlength{\parindent}{5pt} \robot \hspace{2pt} \textbf{Estructural}

\begin{tcolorbox}[
    colback=matterbg2,
    colframe=mattergreen1,
    width=\textwidth,
    arc=2mm,
    boxrule=0.2mm,
    leftrule=0.2mm, rightrule=0.2mm,
    toprule=0.2mm, bottomrule=0.2mm,
    enhanced,
    breakable
]
\textbf{Tool used:}

\setlength{\parindent}{5pt}\underline{\texttt{Tool Name:}} \texttt{repl\_tool}\par
\setlength{\parindent}{5pt}\underline{\texttt{Arguments:}}\par
\setlength{\parindent}{10pt}\texttt{code =}\par
\begin{verbatim}
import numpy as np

def read_xyz(path):
    with open(path, 'r') as f:
        lines = f.readlines()
    num_atoms = int(lines[0])
    atoms = []
    coords = []
    for line in lines[2:2+num_atoms]:
        parts = line.split()
        atoms.append(parts[0])
        coords.append([float(x) for x in parts[1:4]])
    return atoms, np.array(coords)

atoms, coords = read_xyz('MoCl3PNP.xyz')
targets = [7, 11, 15, 21, 22, 26]

for i in targets:
    c_neighbors = 0
    neighbor_indices = []
    for j, (atom, coord) in enumerate(zip(atoms, coords)):
        if i == j: continue
        dist = np.linalg.norm(coords[i] - coords[j])
        if dist < 1.7: # C-C is ~1.5, P-C is ~1.85. 1.7 should catch C-C but maybe exclude P-C? 
                       # Actually P-C is around 1.8. Let's strictly look for C neighbors.
            if atom == 'C':
                c_neighbors += 1
                neighbor_indices.append(j)
    
    print(f"Atom {i} ({atoms[i]}) has {c_neighbors} Carbon neighbors: {neighbor_indices}")

\end{verbatim}\par
\smallskip
\end{tcolorbox}

\setlength{\parindent}{5pt} \robot \hspace{2pt} \textbf{Estructural}

\begin{tcolorbox}[
    colback=matterbg2,
    colframe=mattergreen1,
    width=\textwidth,
    arc=2mm,
    boxrule=0.2mm,
    leftrule=0.2mm, rightrule=0.2mm,
    toprule=0.2mm, bottomrule=0.2mm,
    enhanced,
    breakable
]
\textbf{Tool used:}

\setlength{\parindent}{5pt}\underline{\texttt{Tool Name:}} \texttt{replace\_branch\_with\_predefined\_FG}\par
\setlength{\parindent}{5pt}\underline{\texttt{Arguments:}}\par
\setlength{\parindent}{10pt}\texttt{output\_path = MoCl3PNP\_derivatives\_project/MoCl3PNP\_H.xyz}\par
\setlength{\parindent}{10pt}\texttt{FG\_name = H}\par
\setlength{\parindent}{10pt}\texttt{bond\_pair = [[4, 7], [4, 11], [5, 22], [5, 26]]}\par
\setlength{\parindent}{10pt}\texttt{core\_file\_path = MoCl3PNP\_derivatives\_project/MoCl3PNP.xyz}\par
\smallskip
\setlength{\parindent}{5pt}\underline{\texttt{Tool Name:}} \texttt{replace\_branch\_with\_predefined\_FG}\par
\setlength{\parindent}{5pt}\underline{\texttt{Arguments:}}\par
\setlength{\parindent}{10pt}\texttt{output\_path = MoCl3PNP\_derivatives\_project/MoCl3PNP\_Me.xyz}\par
\setlength{\parindent}{10pt}\texttt{FG\_name = Me}\par
\setlength{\parindent}{10pt}\texttt{bond\_pair = [[4, 7], [4, 11], [5, 22], [5, 26]]}\par
\setlength{\parindent}{10pt}\texttt{core\_file\_path = MoCl3PNP\_derivatives\_project/MoCl3PNP.xyz}\par
\smallskip
\setlength{\parindent}{5pt}\underline{\texttt{Tool Name:}} \texttt{replace\_branch\_with\_predefined\_FG}\par
\setlength{\parindent}{5pt}\underline{\texttt{Arguments:}}\par
\setlength{\parindent}{10pt}\texttt{output\_path = MoCl3PNP\_derivatives\_project/MoCl3PNP\_Ph.xyz}\par
\setlength{\parindent}{10pt}\texttt{FG\_name = Ph}\par
\setlength{\parindent}{10pt}\texttt{bond\_pair = [[4, 7], [4, 11], [5, 22], [5, 26]]}\par
\setlength{\parindent}{10pt}\texttt{core\_file\_path = MoCl3PNP\_derivatives\_project/MoCl3PNP.xyz}\par
\smallskip
\end{tcolorbox}

\setlength{\parindent}{5pt} \robot \hspace{2pt} \textbf{Estructural}

\begin{tcolorbox}[
    colback=matterbg2,
    colframe=mattergreen1,
    width=\textwidth,
    arc=2mm,
    boxrule=0.2mm,
    leftrule=0.2mm, rightrule=0.2mm,
    toprule=0.2mm, bottomrule=0.2mm,
    enhanced,
    breakable
]
\textbf{Action:}

\begin{markdown}
Based on the analysis of the `MoCl3PNP.xyz` structure, I have successfully identified the *tert*-butyl groups attached to the Phosphorus atoms and generated the three requested derivative structures.

**Execution Details:**

1.  **Structure Analysis:**
    *   **Phosphorus Atoms:** Identified at indices **4** and **5**.
    *   **Ligand Topology:** By analyzing the coordination environment, I distinguished the *tert*-butyl groups from the pyridine-linker backbone:
        *   **Linker Carbons:** Atoms **15** (connected to P4) and **21** (connected to P5) were identified as methylene bridges (-CH2-) connecting to the pyridine ring.
        *   **t-Butyl Quaternary Carbons:** Atoms **7, 11** (connected to P4) and **22, 26** (connected to P5) were identified as the anchor points for the *tert*-butyl groups.
    *   **Target Bonds:** The bonds selected for replacement were `P(4)-C(7)`, `P(4)-C(11)`, `P(5)-C(22)`, and `P(5)-C(26)`.

2.  **Modifications:**
    *   Replaced the four *tert*-butyl branches with **Hydrogen (H)**.
    *   Replaced the four *tert*-butyl branches with **Methyl (Me)**.
    *   Replaced the four *tert*-butyl branches with **Phenyl (Ph)**.

3.  **File Generation:**
    All files have been organized into the project folder `MoCl3PNP_derivatives_project`.
    *   `MoCl3PNP_derivatives_project/MoCl3PNP_H.xyz`
    *   `MoCl3PNP_derivatives_project/MoCl3PNP_Me.xyz`
    *   `MoCl3PNP_derivatives_project/MoCl3PNP_Ph.xyz`

The requested derivatives are now ready for use.
\end{markdown}

\end{tcolorbox}
