# Supplementary material for: El Agente Estructural: An Artificially Intelligent Molecular Editor
Source: arXiv:2602.04849 source file (2026-11-30)
Supplement: Supplementary file 2 [file TDSO.tex]

\setlength{\parindent}{5pt} \textbf{\textcolor{blue}{User:}}
\begin{tcolorbox}[
    colback=blue!10,
    colframe=blue,
    width=\textwidth,
    arc=2mm,
    boxrule=0.2mm,
    leftrule=0.2mm, rightrule=0.2mm,
    toprule=0.2mm, bottomrule=0.2mm,
    enhanced,
    breakable
]
\begin{markdown}
What do you find in local directory
\end{markdown}
\end{tcolorbox}
\setlength{\parindent}{5pt} \robot \hspace{2pt} \textbf{Estructural}

\begin{tcolorbox}[
    colback=matterbg2,
    colframe=mattergreen1,
    width=\textwidth,
    arc=2mm,
    boxrule=0.2mm,
    leftrule=0.2mm, rightrule=0.2mm,
    toprule=0.2mm, bottomrule=0.2mm,
    enhanced,
    breakable
]
\textbf{Action:}

\begin{markdown}
Based on the current working directory, I can see the following files:

```
+-- Reaction.png
+-- TS.png
```

**Summary of files found:**

| File Name | Description |
|-----------|-------------|
| `Reaction.png` | Likely an image showing a chemical reaction (mechanism diagram, reaction scheme, etc.) |
| `TS.png` | Likely an image showing a Transition State (TS) structure |

Both files are PNG images, which typically contain chemistry-related visualizations such as reaction mechanisms, molecular structures, or transition state geometries.

Would you like me to:
1. **View either of these images** to analyze their content?
2. **Generate molecular structures** based on what's shown in these images?
3. **Perform any specific molecular editing** tasks based on these files?

Just let me know how you'd like to proceed!
\end{markdown}

\end{tcolorbox}

\setlength{\parindent}{5pt} \textbf{\textcolor{blue}{User:}}
\begin{tcolorbox}[
    colback=blue!10,
    colframe=blue,
    width=\textwidth,
    arc=2mm,
    boxrule=0.2mm,
    leftrule=0.2mm, rightrule=0.2mm,
    toprule=0.2mm, bottomrule=0.2mm,
    enhanced,
    breakable
]
\begin{markdown}
OK, what does the Reaction.png tells
\end{markdown}
\end{tcolorbox}
\setlength{\parindent}{5pt} \robot \hspace{2pt} \textbf{Estructural}

\begin{tcolorbox}[
    colback=matterbg2,
    colframe=mattergreen1,
    width=\textwidth,
    arc=2mm,
    boxrule=0.2mm,
    leftrule=0.2mm, rightrule=0.2mm,
    toprule=0.2mm, bottomrule=0.2mm,
    enhanced,
    breakable
]
\textbf{Action:}

\begin{markdown}
I'll view the Reaction.png file to analyze its contents.
\end{markdown}

\textbf{Tool used:}

\setlength{\parindent}{5pt}\underline{\texttt{Tool Name:}} \texttt{view\_png\_file}\par
\setlength{\parindent}{5pt}\underline{\texttt{Arguments:}}\par
\setlength{\parindent}{10pt}\texttt{png\_file\_relative\_path = Reaction.png}\par
\smallskip
\end{tcolorbox}

\setlength{\parindent}{5pt} \robot \hspace{2pt} \textbf{Estructural}

\begin{tcolorbox}[
    colback=matterbg2,
    colframe=mattergreen1,
    width=\textwidth,
    arc=2mm,
    boxrule=0.2mm,
    leftrule=0.2mm, rightrule=0.2mm,
    toprule=0.2mm, bottomrule=0.2mm,
    enhanced,
    breakable
]
\textbf{Action:}

\begin{markdown}
**Analysis of Reaction.png**

This image shows a **heterocyclic ring transformation reaction** - specifically the conversion of an **Isothiazole** to an **N-Alkyl Pyrazole**.

---

****Reaction Overview****

| Component | Description |
|-----------|-------------|
| **Starting Material** | **Isothiazole** - a 5-membered aromatic heterocycle containing N and S atoms |
| **Reagents** | + "NH" (nitrogen/amine source) + "O" (oxygen/oxidation) |
| **Product** | **N-Alkyl Pyrazole** - a 5-membered heterocycle with two adjacent nitrogen atoms (N-N) |
| **Pathway** | Via an **Intermediate Structure** |

---

****Structural Details****

**Isothiazole (Reactant):**
- 5-membered ring with N-S bond
- Contains modular substituent positions shown as colored circles:
  - [orange] Orange position
  - [blue] Blue position  
  - [black] Gray position

**N-Alkyl Pyrazole (Product):**
- 5-membered ring with N-N bond
- The same substituent positions are retained (modular assembly)
- An **R group** (alkyl) is attached to one nitrogen

---

****Key Chemical Transformation****
1. The **S (sulfur)** in isothiazole is replaced
2. A new **N-N bond** is formed (characteristic of pyrazole)
3. The ring skeleton is reorganized
4. An **N-alkyl group (R)** is introduced
5. The substituent positions (colored circles) are preserved during the transformation

---

****What would you like to do next?****

1. **Generate the structures** (Isothiazole and/or N-Alkyl Pyrazole) as XYZ files?
2. **View the TS.png** to see the transition state/intermediate structure?
3. **Build the intermediate structure** mentioned in the reaction pathway?
4. **Explore specific substituents** at the modular positions?

Let me know how you'd like to proceed!
\end{markdown}

\end{tcolorbox}

\setlength{\parindent}{5pt} \textbf{\textcolor{blue}{User:}}
\begin{tcolorbox}[
    colback=blue!10,
    colframe=blue,
    width=\textwidth,
    arc=2mm,
    boxrule=0.2mm,
    leftrule=0.2mm, rightrule=0.2mm,
    toprule=0.2mm, bottomrule=0.2mm,
    enhanced,
    breakable
]
\begin{markdown}
with the substituent be consistent before and after reaction, let's build substrate and product with the R on the C alpha to S as Me, the others as H. generate the structures of these two
\end{markdown}
\end{tcolorbox}
\setlength{\parindent}{5pt} \robot \hspace{2pt} \textbf{Estructural}

\begin{tcolorbox}[
    colback=matterbg2,
    colframe=mattergreen1,
    width=\textwidth,
    arc=2mm,
    boxrule=0.2mm,
    leftrule=0.2mm, rightrule=0.2mm,
    toprule=0.2mm, bottomrule=0.2mm,
    enhanced,
    breakable
]
\textbf{Action:}

\begin{markdown}
I'll generate both the substrate (isothiazole) and product (pyrazole) structures based on the reaction scheme:

**Substituent assignments:**
- **Orange position** (C alpha to S): **Me (methyl)**
- **Blue position**: **H**
- **Gray position**: **H**
- **R on pyrazole N**: **H** (making it 1H-pyrazole)

Let me generate both structures:
\end{markdown}

\textbf{Tool used:}

\setlength{\parindent}{5pt}\underline{\texttt{Tool Name:}} \texttt{organic\_molecules\_xyz\_generation}\par
\setlength{\parindent}{5pt}\underline{\texttt{Arguments:}}\par
\setlength{\parindent}{10pt}\texttt{smiles\_list = ["Cc1ccns1", "Cc1cc[nH]n1"]}\par
\setlength{\parindent}{10pt}\texttt{filenames = ["5-methylisothiazole\_substrate.xyz", "3-methyl-1H-pyrazole\_product.xyz"]}\par
\smallskip
\end{tcolorbox}

\setlength{\parindent}{5pt} \robot \hspace{2pt} \textbf{Estructural}

\begin{tcolorbox}[
    colback=matterbg2,
    colframe=mattergreen1,
    width=\textwidth,
    arc=2mm,
    boxrule=0.2mm,
    leftrule=0.2mm, rightrule=0.2mm,
    toprule=0.2mm, bottomrule=0.2mm,
    enhanced,
    breakable
]
\textbf{Action:}

\begin{markdown}
Both structures have been generated successfully. Let me visualize them to confirm they're correct:
\end{markdown}

\textbf{Tool used:}

\setlength{\parindent}{5pt}\underline{\texttt{Tool Name:}} \texttt{view\_molecule}\par
\setlength{\parindent}{5pt}\underline{\texttt{Arguments:}}\par
\setlength{\parindent}{10pt}\texttt{xyz\_file\_relative\_path = 5-methylisothiazole\_substrate.xyz}\par
\setlength{\parindent}{10pt}\texttt{left\_right\_deg = 0}\par
\setlength{\parindent}{10pt}\texttt{up\_down\_deg = 0}\par
\smallskip
\end{tcolorbox}

\setlength{\parindent}{5pt} \robot \hspace{2pt} \textbf{Estructural}

\begin{tcolorbox}[
    colback=matterbg2,
    colframe=mattergreen1,
    width=\textwidth,
    arc=2mm,
    boxrule=0.2mm,
    leftrule=0.2mm, rightrule=0.2mm,
    toprule=0.2mm, bottomrule=0.2mm,
    enhanced,
    breakable
]
\textbf{Action:}

\begin{markdown}
The **substrate (5-methylisothiazole)** looks correct. Now let me view the product:
\end{markdown}

\textbf{Tool used:}

\setlength{\parindent}{5pt}\underline{\texttt{Tool Name:}} \texttt{view\_molecule}\par
\setlength{\parindent}{5pt}\underline{\texttt{Arguments:}}\par
\setlength{\parindent}{10pt}\texttt{xyz\_file\_relative\_path = 3-methyl-1H-pyrazole\_product.xyz}\par
\setlength{\parindent}{10pt}\texttt{left\_right\_deg = 0}\par
\setlength{\parindent}{10pt}\texttt{up\_down\_deg = 0}\par
\smallskip
\end{tcolorbox}

\setlength{\parindent}{5pt} \robot \hspace{2pt} \textbf{Estructural}

\begin{tcolorbox}[
    colback=matterbg2,
    colframe=mattergreen1,
    width=\textwidth,
    arc=2mm,
    boxrule=0.2mm,
    leftrule=0.2mm, rightrule=0.2mm,
    toprule=0.2mm, bottomrule=0.2mm,
    enhanced,
    breakable
]
\textbf{Action:}

\begin{markdown}
Both structures have been successfully generated. Here's a summary:

---

****Structures Generated****

****1. Substrate: 5-Methylisothiazole****
**File:** `5-methylisothiazole_substrate.xyz`

| Feature | Details |
|---------|---------|
| **Ring** | 5-membered isothiazole (N-S heterocycle) |
| **S atom** | Index 5 |
| **N atom** | Index 4 |
| **Methyl group** | C:0 (with H:6, H:7, H:8) attached to C:1 |
| **C alpha to S** | C:1 (bonded to S:5) --- **has the Me substituent** $\checkmark$ |
| **Other positions** | H atoms (indices 9, 10) |

---

****2. Product: 3-Methyl-1H-pyrazole****
**File:** `3-methyl-1H-pyrazole_product.xyz`

| Feature | Details |
|---------|---------|
| **Ring** | 5-membered pyrazole (N-N heterocycle) |
| **N atoms** | N:4 and N:5 (adjacent, forming N-N bond) |
| **N-H** | H:11 attached to N:4 (1H-pyrazole) |
| **Methyl group** | C:0 (with H:6, H:7, H:8) attached to C:1 |
| **Equivalent position** | C:1 (adjacent to N:5) --- **Me preserved** $\checkmark$ |
| **Other positions** | H atoms (indices 9, 10) |

---

****Structural Correspondence****

| Isothiazole (Substrate) | Pyrazole (Product) | Substituent |
|------------------------|-------------------|-------------|
| S (index 5) | N (index 5) | --- |
| N (index 4) | N-H (index 4) | H on N |
| C alpha to S (C:1) | C alpha to N (C:1) | **Me** |
| Other C atoms | Other C atoms | **H** |

---

Both files are now available in your working directory:
- `5-methylisothiazole_substrate.xyz`
- `3-methyl-1H-pyrazole_product.xyz`

Would you like me to:
1. **View the TS.png** to analyze the transition state/intermediate?
2. **Build an intermediate structure** for this transformation?
3. **Perform any modifications** to these structures?
\end{markdown}

\end{tcolorbox}

\setlength{\parindent}{5pt} \textbf{\textcolor{blue}{User:}}
\begin{tcolorbox}[
    colback=blue!10,
    colframe=blue,
    width=\textwidth,
    arc=2mm,
    boxrule=0.2mm,
    leftrule=0.2mm, rightrule=0.2mm,
    toprule=0.2mm, bottomrule=0.2mm,
    enhanced,
    breakable
]
\begin{markdown}
Ahh your are suggesting the incoming "NH" replace the S atom. It is great. This is therefore a single atom editing reaction, Mark Levin style. TS.png contains the possible TS of one of the steps. Can you tell if it is the earlier or later step.
\end{markdown}
\end{tcolorbox}
\setlength{\parindent}{5pt} \robot \hspace{2pt} \textbf{Estructural}

\begin{tcolorbox}[
    colback=matterbg2,
    colframe=mattergreen1,
    width=\textwidth,
    arc=2mm,
    boxrule=0.2mm,
    leftrule=0.2mm, rightrule=0.2mm,
    toprule=0.2mm, bottomrule=0.2mm,
    enhanced,
    breakable
]
\textbf{Action:}

\begin{markdown}
Exactly! This is a beautiful example of **single-atom skeletal editing** (Mark Levin style) where the sulfur atom is replaced by nitrogen while preserving the rest of the molecular skeleton. Very elegant chemistry!

Let me examine the TS.png to determine which step of the mechanism it represents:
\end{markdown}

\textbf{Tool used:}

\setlength{\parindent}{5pt}\underline{\texttt{Tool Name:}} \texttt{view\_png\_file}\par
\setlength{\parindent}{5pt}\underline{\texttt{Arguments:}}\par
\setlength{\parindent}{10pt}\texttt{png\_file\_relative\_path = TS.png}\par
\smallskip
\end{tcolorbox}

\setlength{\parindent}{5pt} \robot \hspace{2pt} \textbf{Estructural}

\begin{tcolorbox}[
    colback=matterbg2,
    colframe=mattergreen1,
    width=\textwidth,
    arc=2mm,
    boxrule=0.2mm,
    leftrule=0.2mm, rightrule=0.2mm,
    toprule=0.2mm, bottomrule=0.2mm,
    enhanced,
    breakable
]
\textbf{Action:}

\begin{markdown}
Excellent question! This TS.png reveals crucial mechanistic information.

****Analysis of TS.png****

****What the image shows:****

| Component | Structure | Key Features |
|-----------|-----------|--------------|
| **Left (Intermediate)** | **NH TDSO** | S=O (sulfoxide), NH attached to S, ring N intact |
| **Right (Product)** | **N-Alkyl Pyrazole** | Final pyrazole with N-N bond, R on nitrogen |

---

****This is the LATER STEP** [search]**

**Evidence:**

1. **NH is already incorporated** - In the "NH TDSO" intermediate, the NH group is already bonded to sulfur. This means the NH addition step has already occurred.

2. **Sulfur is already oxidized** - The S=O (sulfoxide) is present, indicating the oxidation step ("+O") has already happened.

3. **What this TS represents** - The transition state for **sulfur extrusion** and **N-N bond formation** to give the final pyrazole.

---

****Proposed Mechanism Sequence:****

| Step | Transformation | Status |
|------|---------------|--------|
| **Step 1 (Earlier)** | Isothiazole + "NH" $\rightarrow$ NH incorporation onto S | [done] Already completed |
| **Step 2 (Earlier)** | Oxidation (+O) $\rightarrow$ S=O formation | [done] Already completed |
| **Step 3 (LATER - This TS)** | NH TDSO $\rightarrow$ **Pyrazole** + SO extrusion | [target] **This is the TS shown** |

---

****Mechanistic Interpretation:****

The "NH TDSO" intermediate (likely a **thiadiazole S-oxide** or similar) undergoes:
- **S-N bond cleavage** (breaking S from the ring)
- **N-N bond formation** (creating the pyrazole N-N linkage)  
- **SO extrusion** (sulfur monoxide leaves)

This is the **ring-contracting/sulfur-extrusion step** - the final key bond-forming event that delivers the pyrazole product.

---

Would you like me to:
1. **Build the NH TDSO intermediate structure** for computational study?
2. **Generate a TS geometry** for this sulfur extrusion step?
3. **Create the complete reaction coordinate** with all species?
\end{markdown}

\end{tcolorbox}

\setlength{\parindent}{5pt} \textbf{\textcolor{blue}{User:}}
\begin{tcolorbox}[
    colback=blue!10,
    colframe=blue,
    width=\textwidth,
    arc=2mm,
    boxrule=0.2mm,
    leftrule=0.2mm, rightrule=0.2mm,
    toprule=0.2mm, bottomrule=0.2mm,
    enhanced,
    breakable
]
\begin{markdown}
OK. You are suggesting a missing step involve amine addition for N-N bond formation then sulfur oxidation to S=O. Can you then generate the structures of NH TDSO and its pre-oxidized form as the key intermediates, and make sure they are consistent with the mechanism you are proposing in terms of skeleton connection and substituent pattern? Remember same colour atom represent same atom across reaction.
\end{markdown}
\end{tcolorbox}
\setlength{\parindent}{5pt} \robot \hspace{2pt} \textbf{Estructural}

\begin{tcolorbox}[
    colback=matterbg2,
    colframe=mattergreen1,
    width=\textwidth,
    arc=2mm,
    boxrule=0.2mm,
    leftrule=0.2mm, rightrule=0.2mm,
    toprule=0.2mm, bottomrule=0.2mm,
    enhanced,
    breakable
]
\textbf{Action:}

\begin{markdown}
You're right! Let me clarify the mechanism I'm proposing:

**Proposed Mechanism:**
1. **Step 1**: Isothiazole + NH $\rightarrow$ Ring expansion with N-N bond formation (pre-oxidized intermediate)
2. **Step 2**: Oxidation of S $\rightarrow$ S=O (forming NH TDSO)
3. **Step 3**: SO extrusion $\rightarrow$ Pyrazole (the TS shown in TS.png)

Now let me build the two key intermediates with the correct connectivity. Based on the image:
- **6-membered ring**: S-C(Me)-C-C-N-N(H) back to S
- **Me on C adjacent to S** (orange position)
- **N-N bond formed** (the new NH bonded to original N)
\end{markdown}

\textbf{Tool used:}

\setlength{\parindent}{5pt}\underline{\texttt{Tool Name:}} \texttt{organic\_molecules\_xyz\_generation}\par
\setlength{\parindent}{5pt}\underline{\texttt{Arguments:}}\par
\setlength{\parindent}{10pt}\texttt{smiles\_list = ["CC1=CC=N[NH]S1", "CC1=CC=N[NH][S]1=O"]}\par
\setlength{\parindent}{10pt}\texttt{filenames = ["pre-oxidized\_NH-thiadiazine.xyz", "NH\_TDSO\_intermediate.xyz"]}\par
\smallskip
\end{tcolorbox}

\setlength{\parindent}{5pt} \robot \hspace{2pt} \textbf{Estructural}

\begin{tcolorbox}[
    colback=matterbg2,
    colframe=mattergreen1,
    width=\textwidth,
    arc=2mm,
    boxrule=0.2mm,
    leftrule=0.2mm, rightrule=0.2mm,
    toprule=0.2mm, bottomrule=0.2mm,
    enhanced,
    breakable
]
\textbf{Action:}

\begin{markdown}
Both intermediates have been generated. Let me visualize them to verify the correct structure and connectivity:
\end{markdown}

\textbf{Tool used:}

\setlength{\parindent}{5pt}\underline{\texttt{Tool Name:}} \texttt{view\_molecule}\par
\setlength{\parindent}{5pt}\underline{\texttt{Arguments:}}\par
\setlength{\parindent}{10pt}\texttt{xyz\_file\_relative\_path = pre-oxidized\_NH-thiadiazine.xyz}\par
\setlength{\parindent}{10pt}\texttt{left\_right\_deg = 0}\par
\setlength{\parindent}{10pt}\texttt{up\_down\_deg = 0}\par
\smallskip
\end{tcolorbox}

\setlength{\parindent}{5pt} \robot \hspace{2pt} \textbf{Estructural}

\begin{tcolorbox}[
    colback=matterbg2,
    colframe=mattergreen1,
    width=\textwidth,
    arc=2mm,
    boxrule=0.2mm,
    leftrule=0.2mm, rightrule=0.2mm,
    toprule=0.2mm, bottomrule=0.2mm,
    enhanced,
    breakable
]
\textbf{Action:}

\begin{markdown}
Excellent! The **pre-oxidized intermediate** structure looks correct:
- **6-membered ring**: C:1 - C:2 - C:3 - N:4 - N:5 - S:6
- **Me (C:0)** attached to **C:1** which is adjacent to **S:6** $\checkmark$
- **N-N bond** present (N:4 - N:5) $\checkmark$
- **NH** is N:5 with H:12 attached $\checkmark$

Now let me view the oxidized NH TDSO intermediate:
\end{markdown}

\textbf{Tool used:}

\setlength{\parindent}{5pt}\underline{\texttt{Tool Name:}} \texttt{view\_molecule}\par
\setlength{\parindent}{5pt}\underline{\texttt{Arguments:}}\par
\setlength{\parindent}{10pt}\texttt{xyz\_file\_relative\_path = NH\_TDSO\_intermediate.xyz}\par
\setlength{\parindent}{10pt}\texttt{left\_right\_deg = 0}\par
\setlength{\parindent}{10pt}\texttt{up\_down\_deg = 0}\par
\smallskip
\end{tcolorbox}

\setlength{\parindent}{5pt} \robot \hspace{2pt} \textbf{Estructural}

\begin{tcolorbox}[
    colback=matterbg2,
    colframe=mattergreen1,
    width=\textwidth,
    arc=2mm,
    boxrule=0.2mm,
    leftrule=0.2mm, rightrule=0.2mm,
    toprule=0.2mm, bottomrule=0.2mm,
    enhanced,
    breakable
]
\textbf{Action:}

\begin{markdown}
The **NH TDSO intermediate** structure is correct:
- **6-membered ring**: C:1 - C:2 - C:3 - N:4 - N:5 - S:6
- **S=O** present: S:6 with O:7 (sulfoxide) $\checkmark$
- **Me (C:0)** attached to **C:1** adjacent to **S:6** $\checkmark$
- **N-N bond** present (N:4 - N:5) $\checkmark$
- **NH** is N:5 with H:13 attached $\checkmark$

---

****Complete Mechanism Summary****

All structures are now generated and consistent with the proposed single-atom skeletal editing mechanism:

| Step | Structure | File | Key Features |
|------|-----------|------|--------------|
| **Substrate** | 5-Methylisothiazole | `5-methylisothiazole_substrate.xyz` | 5-membered ring, S-N, Me on C($\alpha$ to S) |
| **Intermediate 1** | Pre-oxidized NH-thiadiazine | `pre-oxidized_NH-thiadiazine.xyz` | 6-membered ring, N-N bond formed, S not oxidized |
| **Intermediate 2** | NH TDSO | `NH_TDSO_intermediate.xyz` | 6-membered ring, N-N bond, **S=O** formed |
| **Product** | 3-Methyl-1H-pyrazole | `3-methyl-1H-pyrazole_product.xyz` | 5-membered ring, N-N, SO extruded |

---

****Mechanistic Pathway (Mark Levin-style Skeletal Editing)****

```
Isothiazole (5-membered)
       |
       | + NH (amine source)
       | Ring expansion + N-N bond formation
       [down]
Pre-oxidized NH-thiadiazine (6-membered)
       |
       | + O (oxidation)
       | S $\rightarrow$ S=O
       [down]
NH TDSO (6-membered, S-oxide)
       |
       | [TS shown in TS.png]
       | SO extrusion + ring contraction
       [down]
N-Alkyl Pyrazole (5-membered)
```

---

****Atom Correspondence (Color Coding)****

| Position | Substrate | Intermediate | Product |
|----------|-----------|--------------|---------|
| [orange] Orange (Me) | C:1 ($\alpha$ to S) | C:1 ($\alpha$ to S) | C:1 ($\alpha$ to N) |
| [blue] Blue (H) | C:3 | C:3 | C:3 |
| [black] Gray (H) | C:2 | C:2 | C:2 |
| Heteroatom | S | S ($\rightarrow$ S=O) | N (from NH) |

The skeletal connectivity and substituent pattern are preserved throughout the transformation! Would you like me to perform any further analysis or generate the transition state structure for the SO extrusion step?
\end{markdown}

\end{tcolorbox}

\setlength{\parindent}{5pt} \textbf{\textcolor{blue}{User:}}
\begin{tcolorbox}[
    colback=blue!10,
    colframe=blue,
    width=\textwidth,
    arc=2mm,
    boxrule=0.2mm,
    leftrule=0.2mm, rightrule=0.2mm,
    toprule=0.2mm, bottomrule=0.2mm,
    enhanced,
    breakable
]
\begin{markdown}
The "NH" suggest a pseudo NH source and the pre-oxidation NH TDSO is likely having "NH". If the N-alkylation happens after formation of NH TDSO and SO extrusion TS takes place with the N alkylated intermediate, as it is known diazine-like molecules could be alkylated on either N, can you generate the possible TS for either pathway? A side note the reaction is performed in solvent so proton exchange with solvent is possible.
\end{markdown}
\end{tcolorbox}
\setlength{\parindent}{5pt} \robot \hspace{2pt} \textbf{Estructural}

\begin{tcolorbox}[
    colback=matterbg2,
    colframe=mattergreen1,
    width=\textwidth,
    arc=2mm,
    boxrule=0.2mm,
    leftrule=0.2mm, rightrule=0.2mm,
    toprule=0.2mm, bottomrule=0.2mm,
    enhanced,
    breakable
]
\textbf{Action:}

\begin{markdown}
Excellent mechanistic insight! Let me revise the understanding:

**Updated Mechanism:**
1. Isothiazole + "NH" $\rightarrow$ Pre-oxidized NH-thiadiazine (NH form)
2. Oxidation $\rightarrow$ NH TDSO (still NH form)
3. **N-alkylation** $\rightarrow$ N-alkyl TDSO (can occur on either N)
4. **SO extrusion TS** $\rightarrow$ N-alkyl pyrazole

Since the diazine has two nitrogens that could be alkylated, there are **two possible pathways**:
- **Pathway A**: Alkylation on N:5 (the N adjacent to S, originally the NH)
- **Pathway B**: Alkylation on N:4 (the other N, away from S)

Let me first generate both N-methylated TDSO intermediates, then create TS geometries for SO extrusion:
\end{markdown}

\textbf{Tool used:}

\setlength{\parindent}{5pt}\underline{\texttt{Tool Name:}} \texttt{organic\_molecules\_xyz\_generation}\par
\setlength{\parindent}{5pt}\underline{\texttt{Arguments:}}\par
\setlength{\parindent}{10pt}\texttt{smiles\_list = ["CC1=CC=NN(C)[S]1=O", "CC1=CC=[N+](C)N[S]1=O"]}\par
\setlength{\parindent}{10pt}\texttt{filenames = ["N5-Me\_TDSO\_pathwayA.xyz", "N4-Me\_TDSO\_pathwayB.xyz"]}\par
\smallskip
\end{tcolorbox}

\setlength{\parindent}{5pt} \robot \hspace{2pt} \textbf{Estructural}

\begin{tcolorbox}[
    colback=matterbg2,
    colframe=mattergreen1,
    width=\textwidth,
    arc=2mm,
    boxrule=0.2mm,
    leftrule=0.2mm, rightrule=0.2mm,
    toprule=0.2mm, bottomrule=0.2mm,
    enhanced,
    breakable
]
\textbf{Action:}

\begin{markdown}
Both N-methylated intermediates generated. Let me visualize them to identify the correct atomic indices for TS generation:
\end{markdown}

\textbf{Tool used:}

\setlength{\parindent}{5pt}\underline{\texttt{Tool Name:}} \texttt{view\_molecule}\par
\setlength{\parindent}{5pt}\underline{\texttt{Arguments:}}\par
\setlength{\parindent}{10pt}\texttt{xyz\_file\_relative\_path = N5-Me\_TDSO\_pathwayA.xyz}\par
\setlength{\parindent}{10pt}\texttt{left\_right\_deg = 0}\par
\setlength{\parindent}{10pt}\texttt{up\_down\_deg = 0}\par
\smallskip
\end{tcolorbox}

\setlength{\parindent}{5pt} \robot \hspace{2pt} \textbf{Estructural}

\begin{tcolorbox}[
    colback=matterbg2,
    colframe=mattergreen1,
    width=\textwidth,
    arc=2mm,
    boxrule=0.2mm,
    leftrule=0.2mm, rightrule=0.2mm,
    toprule=0.2mm, bottomrule=0.2mm,
    enhanced,
    breakable
]
\textbf{Action:}

\begin{markdown}
**Pathway A (N5-Me TDSO)** structure verified:
- **Ring**: C:1 - C:2 - C:3 - N:4 - N:5 - S:7 (back to C:1)
- **Me on C:1** (C:0, adjacent to S) $\checkmark$
- **N-Me on N:5** (C:6, the N adjacent to S) $\checkmark$
- **S=O**: S:7 with O:8 $\checkmark$

For SO extrusion TS, bonds to elongate: **S:7-C:1** and **S:7-N:5**

Now let me view Pathway B:
\end{markdown}

\textbf{Tool used:}

\setlength{\parindent}{5pt}\underline{\texttt{Tool Name:}} \texttt{view\_molecule}\par
\setlength{\parindent}{5pt}\underline{\texttt{Arguments:}}\par
\setlength{\parindent}{10pt}\texttt{xyz\_file\_relative\_path = N4-Me\_TDSO\_pathwayB.xyz}\par
\setlength{\parindent}{10pt}\texttt{left\_right\_deg = 0}\par
\setlength{\parindent}{10pt}\texttt{up\_down\_deg = 0}\par
\smallskip
\end{tcolorbox}

\setlength{\parindent}{5pt} \robot \hspace{2pt} \textbf{Estructural}

\begin{tcolorbox}[
    colback=matterbg2,
    colframe=mattergreen1,
    width=\textwidth,
    arc=2mm,
    boxrule=0.2mm,
    leftrule=0.2mm, rightrule=0.2mm,
    toprule=0.2mm, bottomrule=0.2mm,
    enhanced,
    breakable
]
\textbf{Action:}

\begin{markdown}
**Pathway B (N4-Me TDSO)** structure verified:
- **Ring**: C:1 - C:2 - C:3 - N:4 - N:6 - S:7 (back to C:1)
- **Me on C:1** (C:0, adjacent to S) $\checkmark$
- **N-Me on N:4** (C:5, the N away from S) $\checkmark$
- **NH on N:6** (H:17, the N adjacent to S) $\checkmark$
- **S=O**: S:7 with O:8 $\checkmark$

For SO extrusion TS, bonds to elongate: **S:7-C:1** and **S:7-N:6**

Now let me generate TS initial geometries for both pathways by elongating the S-C and S-N bonds using constrained optimization:
\end{markdown}

\textbf{Tool used:}

\setlength{\parindent}{5pt}\underline{\texttt{Tool Name:}} \texttt{constraint\_xtb}\par
\setlength{\parindent}{5pt}\underline{\texttt{Arguments:}}\par
\setlength{\parindent}{10pt}\texttt{input\_xyz = N5-Me\_TDSO\_pathwayA.xyz}\par
\setlength{\parindent}{10pt}\texttt{output\_xyz = TS\_pathwayA\_SO\_extrusion.xyz}\par
\setlength{\parindent}{10pt}\texttt{distance\_constraints = [\{"atoms": [7, 1], "value": 2.3\}, \{"atoms": [7, 5], "value": 2.2\}]}\par
\setlength{\parindent}{10pt}\texttt{force\_constant = 0.8}\par
\setlength{\parindent}{10pt}\texttt{charge = 0}\par
\smallskip
\end{tcolorbox}

\setlength{\parindent}{5pt} \robot \hspace{2pt} \textbf{Estructural}

\begin{tcolorbox}[
    colback=matterbg2,
    colframe=mattergreen1,
    width=\textwidth,
    arc=2mm,
    boxrule=0.2mm,
    leftrule=0.2mm, rightrule=0.2mm,
    toprule=0.2mm, bottomrule=0.2mm,
    enhanced,
    breakable
]
\textbf{Action:}

\begin{markdown}
Pathway A TS generated successfully. Now let me generate the Pathway B TS:
\end{markdown}

\textbf{Tool used:}

\setlength{\parindent}{5pt}\underline{\texttt{Tool Name:}} \texttt{constraint\_xtb}\par
\setlength{\parindent}{5pt}\underline{\texttt{Arguments:}}\par
\setlength{\parindent}{10pt}\texttt{input\_xyz = N4-Me\_TDSO\_pathwayB.xyz}\par
\setlength{\parindent}{10pt}\texttt{output\_xyz = TS\_pathwayB\_SO\_extrusion.xyz}\par
\setlength{\parindent}{10pt}\texttt{distance\_constraints = [\{"atoms": [7, 1], "value": 2.3\}, \{"atoms": [7, 6], "value": 2.2\}]}\par
\setlength{\parindent}{10pt}\texttt{force\_constant = 0.8}\par
\setlength{\parindent}{10pt}\texttt{charge = 0}\par
\smallskip
\end{tcolorbox}

\setlength{\parindent}{5pt} \robot \hspace{2pt} \textbf{Estructural}

\begin{tcolorbox}[
    colback=matterbg2,
    colframe=mattergreen1,
    width=\textwidth,
    arc=2mm,
    boxrule=0.2mm,
    leftrule=0.2mm, rightrule=0.2mm,
    toprule=0.2mm, bottomrule=0.2mm,
    enhanced,
    breakable
]
\textbf{Action:}

\begin{markdown}
Both TS geometries generated successfully. Let me visualize and verify them:
\end{markdown}

\textbf{Tool used:}

\setlength{\parindent}{5pt}\underline{\texttt{Tool Name:}} \texttt{view\_molecule}\par
\setlength{\parindent}{5pt}\underline{\texttt{Arguments:}}\par
\setlength{\parindent}{10pt}\texttt{xyz\_file\_relative\_path = TS\_pathwayA\_SO\_extrusion.xyz}\par
\setlength{\parindent}{10pt}\texttt{left\_right\_deg = 0}\par
\setlength{\parindent}{10pt}\texttt{up\_down\_deg = 0}\par
\smallskip
\end{tcolorbox}

\setlength{\parindent}{5pt} \robot \hspace{2pt} \textbf{Estructural}

\begin{tcolorbox}[
    colback=matterbg2,
    colframe=mattergreen1,
    width=\textwidth,
    arc=2mm,
    boxrule=0.2mm,
    leftrule=0.2mm, rightrule=0.2mm,
    toprule=0.2mm, bottomrule=0.2mm,
    enhanced,
    breakable
]
\textbf{Action:}

\begin{markdown}
**Pathway A TS** looks great! The S=O group (S:7, O:8) is clearly being extruded with elongated S-C:1 and S-N:5 bonds. Let me verify the bond distances:
\end{markdown}

\textbf{Tool used:}

\setlength{\parindent}{5pt}\underline{\texttt{Tool Name:}} \texttt{get\_distance\_angle\_dihedral}\par
\setlength{\parindent}{5pt}\underline{\texttt{Arguments:}}\par
\setlength{\parindent}{10pt}\texttt{input\_path = TS\_pathwayA\_SO\_extrusion.xyz}\par
\setlength{\parindent}{10pt}\texttt{targets = [\{"atom": [7]\}, \{"atom": [1]\}]}\par
\smallskip
\end{tcolorbox}

\setlength{\parindent}{5pt} \robot \hspace{2pt} \textbf{Estructural}

\begin{tcolorbox}[
    colback=matterbg2,
    colframe=mattergreen1,
    width=\textwidth,
    arc=2mm,
    boxrule=0.2mm,
    leftrule=0.2mm, rightrule=0.2mm,
    toprule=0.2mm, bottomrule=0.2mm,
    enhanced,
    breakable
]
\textbf{Tool used:}

\setlength{\parindent}{5pt}\underline{\texttt{Tool Name:}} \texttt{get\_distance\_angle\_dihedral}\par
\setlength{\parindent}{5pt}\underline{\texttt{Arguments:}}\par
\setlength{\parindent}{10pt}\texttt{input\_path = TS\_pathwayA\_SO\_extrusion.xyz}\par
\setlength{\parindent}{10pt}\texttt{targets = [\{"atom": [7]\}, \{"atom": [5]\}]}\par
\smallskip
\end{tcolorbox}

\setlength{\parindent}{5pt} \robot \hspace{2pt} \textbf{Estructural}

\begin{tcolorbox}[
    colback=matterbg2,
    colframe=mattergreen1,
    width=\textwidth,
    arc=2mm,
    boxrule=0.2mm,
    leftrule=0.2mm, rightrule=0.2mm,
    toprule=0.2mm, bottomrule=0.2mm,
    enhanced,
    breakable
]
\textbf{Action:}

\begin{markdown}
**Pathway A TS bond distances verified:**
- S:7 - C:1 = **2.28 Å** (target: 2.3 Å) $\checkmark$
- S:7 - N:5 = **2.19 Å** (target: 2.2 Å) $\checkmark$

Now let me view Pathway B TS:
\end{markdown}

\textbf{Tool used:}

\setlength{\parindent}{5pt}\underline{\texttt{Tool Name:}} \texttt{view\_molecule}\par
\setlength{\parindent}{5pt}\underline{\texttt{Arguments:}}\par
\setlength{\parindent}{10pt}\texttt{xyz\_file\_relative\_path = TS\_pathwayB\_SO\_extrusion.xyz}\par
\setlength{\parindent}{10pt}\texttt{left\_right\_deg = 0}\par
\setlength{\parindent}{10pt}\texttt{up\_down\_deg = 0}\par
\smallskip
\end{tcolorbox}

\setlength{\parindent}{5pt} \robot \hspace{2pt} \textbf{Estructural}

\begin{tcolorbox}[
    colback=matterbg2,
    colframe=mattergreen1,
    width=\textwidth,
    arc=2mm,
    boxrule=0.2mm,
    leftrule=0.2mm, rightrule=0.2mm,
    toprule=0.2mm, bottomrule=0.2mm,
    enhanced,
    breakable
]
\textbf{Action:}

\begin{markdown}
**Pathway B TS** also shows clear SO extrusion geometry. Let me verify the bond distances:
\end{markdown}

\textbf{Tool used:}

\setlength{\parindent}{5pt}\underline{\texttt{Tool Name:}} \texttt{get\_distance\_angle\_dihedral}\par
\setlength{\parindent}{5pt}\underline{\texttt{Arguments:}}\par
\setlength{\parindent}{10pt}\texttt{input\_path = TS\_pathwayB\_SO\_extrusion.xyz}\par
\setlength{\parindent}{10pt}\texttt{targets = [\{"atom": [7]\}, \{"atom": [1]\}]}\par
\smallskip
\end{tcolorbox}

\setlength{\parindent}{5pt} \robot \hspace{2pt} \textbf{Estructural}

\begin{tcolorbox}[
    colback=matterbg2,
    colframe=mattergreen1,
    width=\textwidth,
    arc=2mm,
    boxrule=0.2mm,
    leftrule=0.2mm, rightrule=0.2mm,
    toprule=0.2mm, bottomrule=0.2mm,
    enhanced,
    breakable
]
\textbf{Tool used:}

\setlength{\parindent}{5pt}\underline{\texttt{Tool Name:}} \texttt{get\_distance\_angle\_dihedral}\par
\setlength{\parindent}{5pt}\underline{\texttt{Arguments:}}\par
\setlength{\parindent}{10pt}\texttt{input\_path = TS\_pathwayB\_SO\_extrusion.xyz}\par
\setlength{\parindent}{10pt}\texttt{targets = [\{"atom": [7]\}, \{"atom": [6]\}]}\par
\smallskip
\end{tcolorbox}

\setlength{\parindent}{5pt} \robot \hspace{2pt} \textbf{Estructural}

\begin{tcolorbox}[
    colback=matterbg2,
    colframe=mattergreen1,
    width=\textwidth,
    arc=2mm,
    boxrule=0.2mm,
    leftrule=0.2mm, rightrule=0.2mm,
    toprule=0.2mm, bottomrule=0.2mm,
    enhanced,
    breakable
]
\textbf{Action:}

\begin{markdown}
**Pathway B TS bond distances verified:**
- S:7 - C:1 = **2.28 Å** (target: 2.3 Å) $\checkmark$
- S:7 - N:6 = **2.19 Å** (target: 2.2 Å) $\checkmark$

---

****Complete Summary: Two Pathways for SO Extrusion****

Both transition state geometries have been successfully generated!

****Pathway A: N-Alkylation on N adjacent to S (N5-Me)****

| Structure | File | Description |
|-----------|------|-------------|
| Pre-TS intermediate | `N5-Me_TDSO_pathwayA.xyz` | N-Me on N:5 (adjacent to S) |
| **TS geometry** | `TS_pathwayA_SO_extrusion.xyz` | S-C: 2.28 Å, S-N: 2.19 Å |
| Product | $\rightarrow$ 1-methyl-3-methylpyrazole | Me on N next to C(Me) |

****Pathway B: N-Alkylation on N away from S (N4-Me)****

| Structure | File | Description |
|-----------|------|-------------|
| Pre-TS intermediate | `N4-Me_TDSO_pathwayB.xyz` | N-Me on N:4 (away from S), NH on N:6 |
| **TS geometry** | `TS_pathwayB_SO_extrusion.xyz` | S-C: 2.28 Å, S-N: 2.19 Å |
| Product | $\rightarrow$ 2-methyl-3-methylpyrazole | Me on N away from C(Me) |

---

****Key Mechanistic Differences****

| Feature | Pathway A | Pathway B |
|---------|-----------|-----------|
| **N-Alkylation site** | N:5 (adj. to S) | N:4 (away from S) |
| **NH position** | N:4 | N:6 (adj. to S) |
| **Pyrazole product** | 1,3-dimethylpyrazole | 2,3-dimethylpyrazole |
| **Regioselectivity** | N1-alkylated | N2-alkylated |

---

****TS Geometry Characteristics****

Both TS structures show:
- **Elongated S-C bond** (~2.28 Å vs ~1.8 Å equilibrium) - partial bond breaking
- **Elongated S-N bond** (~2.19 Å vs ~1.7 Å equilibrium) - partial bond breaking
- **S=O group departing** from the ring
- **N-N bond intact** - will form pyrazole core after SO extrusion

---

****Files Generated (Complete Set)****

```
Substrate:     5-methylisothiazole_substrate.xyz
Intermediate:  pre-oxidized_NH-thiadiazine.xyz
               NH_TDSO_intermediate.xyz
               
Pathway A:     N5-Me_TDSO_pathwayA.xyz
               TS_pathwayA_SO_extrusion.xyz

Pathway B:     N4-Me_TDSO_pathwayB.xyz
               TS_pathwayB_SO_extrusion.xyz

Product:       3-methyl-1H-pyrazole_product.xyz
```

Would you like me to:
1. **Generate the pyrazole products** for each pathway with correct N-alkylation patterns?
2. **Perform frequency calculations** on the TS geometries to verify they are true saddle points?
3. **Compare the two pathways** in terms of geometric strain or steric effects?
\end{markdown}

\end{tcolorbox}

\setlength{\parindent}{5pt} \textbf{\textcolor{blue}{User:}}
\begin{tcolorbox}[
    colback=blue!10,
    colframe=blue,
    width=\textwidth,
    arc=2mm,
    boxrule=0.2mm,
    leftrule=0.2mm, rightrule=0.2mm,
    toprule=0.2mm, bottomrule=0.2mm,
    enhanced,
    breakable
]
\begin{markdown}
Both S-C and S-N are reasonable but the C-N distance seems too long for a bond formation 6-membered ring shrinking to 5-membered ring TS, isn't it? Please revise after rethinking the distances between the S, C, N atoms that are crucial to forming the correct 5 membered ring.
\end{markdown}
\end{tcolorbox}
\setlength{\parindent}{5pt} \robot \hspace{2pt} \textbf{Estructural}

\begin{tcolorbox}[
    colback=matterbg2,
    colframe=mattergreen1,
    width=\textwidth,
    arc=2mm,
    boxrule=0.2mm,
    leftrule=0.2mm, rightrule=0.2mm,
    toprule=0.2mm, bottomrule=0.2mm,
    enhanced,
    breakable
]
\textbf{Action:}

\begin{markdown}
You're absolutely right! I apologize for the oversight. This is a **ring contraction** process, so there are THREE key distances in the TS:

1. **S-C bond BREAKING** (elongating)
2. **S-N bond BREAKING** (elongating)
3. **C-N bond FORMING** (shortening) $\leftarrow$ I missed this!

For the 6$\rightarrow$5 membered ring contraction, the C that was attached to S needs to form a NEW bond with the N that was attached to S. Let me first check the current C-N distance in my TS structures:
\end{markdown}

\textbf{Tool used:}

\setlength{\parindent}{5pt}\underline{\texttt{Tool Name:}} \texttt{get\_distance\_angle\_dihedral}\par
\setlength{\parindent}{5pt}\underline{\texttt{Arguments:}}\par
\setlength{\parindent}{10pt}\texttt{input\_path = TS\_pathwayA\_SO\_extrusion.xyz}\par
\setlength{\parindent}{10pt}\texttt{targets = [\{"atom": [1]\}, \{"atom": [5]\}]}\par
\smallskip
\end{tcolorbox}

\setlength{\parindent}{5pt} \robot \hspace{2pt} \textbf{Estructural}

\begin{tcolorbox}[
    colback=matterbg2,
    colframe=mattergreen1,
    width=\textwidth,
    arc=2mm,
    boxrule=0.2mm,
    leftrule=0.2mm, rightrule=0.2mm,
    toprule=0.2mm, bottomrule=0.2mm,
    enhanced,
    breakable
]
\textbf{Action:}

\begin{markdown}
The C:1-N:5 distance is **3.14 Å** - way too long for a forming bond! Let me check Pathway B as well:
\end{markdown}

\textbf{Tool used:}

\setlength{\parindent}{5pt}\underline{\texttt{Tool Name:}} \texttt{get\_distance\_angle\_dihedral}\par
\setlength{\parindent}{5pt}\underline{\texttt{Arguments:}}\par
\setlength{\parindent}{10pt}\texttt{input\_path = TS\_pathwayB\_SO\_extrusion.xyz}\par
\setlength{\parindent}{10pt}\texttt{targets = [\{"atom": [1]\}, \{"atom": [6]\}]}\par
\smallskip
\end{tcolorbox}

\setlength{\parindent}{5pt} \robot \hspace{2pt} \textbf{Estructural}

\begin{tcolorbox}[
    colback=matterbg2,
    colframe=mattergreen1,
    width=\textwidth,
    arc=2mm,
    boxrule=0.2mm,
    leftrule=0.2mm, rightrule=0.2mm,
    toprule=0.2mm, bottomrule=0.2mm,
    enhanced,
    breakable
]
\textbf{Action:}

\begin{markdown}
Pathway B C:1-N:6 distance is **2.81 Å** - also too long!

Now I understand the TS geometry better. The three key atoms (C, S, N) form a **triangle** where:
- **S-C breaking**: elongating from ~1.8 Å $\rightarrow$ ~2.1-2.2 Å
- **S-N breaking**: elongating from ~1.7 Å $\rightarrow$ ~2.0-2.1 Å  
- **C-N forming**: shortening toward ~1.4 Å $\rightarrow$ ~1.8-1.9 Å in TS

Let me regenerate both TS structures with all three constraints:
\end{markdown}

\textbf{Tool used:}

\setlength{\parindent}{5pt}\underline{\texttt{Tool Name:}} \texttt{constraint\_xtb}\par
\setlength{\parindent}{5pt}\underline{\texttt{Arguments:}}\par
\setlength{\parindent}{10pt}\texttt{input\_xyz = N5-Me\_TDSO\_pathwayA.xyz}\par
\setlength{\parindent}{10pt}\texttt{output\_xyz = TS\_pathwayA\_revised.xyz}\par
\setlength{\parindent}{10pt}\texttt{distance\_constraints = [\{"atoms": [7, 1], "value": 2.2\}, \{"atoms": [7, 5], "value": 2.1\}, \{"atoms": [1, 5], "value": 1.9\}]}\par
\setlength{\parindent}{10pt}\texttt{force\_constant = 1.0}\par
\setlength{\parindent}{10pt}\texttt{charge = 0}\par
\smallskip
\end{tcolorbox}

\setlength{\parindent}{5pt} \robot \hspace{2pt} \textbf{Estructural}

\begin{tcolorbox}[
    colback=matterbg2,
    colframe=mattergreen1,
    width=\textwidth,
    arc=2mm,
    boxrule=0.2mm,
    leftrule=0.2mm, rightrule=0.2mm,
    toprule=0.2mm, bottomrule=0.2mm,
    enhanced,
    breakable
]
\textbf{Action:}

\begin{markdown}
Now let me generate the revised Pathway B TS:
\end{markdown}

\textbf{Tool used:}

\setlength{\parindent}{5pt}\underline{\texttt{Tool Name:}} \texttt{constraint\_xtb}\par
\setlength{\parindent}{5pt}\underline{\texttt{Arguments:}}\par
\setlength{\parindent}{10pt}\texttt{input\_xyz = N4-Me\_TDSO\_pathwayB.xyz}\par
\setlength{\parindent}{10pt}\texttt{output\_xyz = TS\_pathwayB\_revised.xyz}\par
\setlength{\parindent}{10pt}\texttt{distance\_constraints = [\{"atoms": [7, 1], "value": 2.2\}, \{"atoms": [7, 6], "value": 2.1\}, \{"atoms": [1, 6], "value": 1.9\}]}\par
\setlength{\parindent}{10pt}\texttt{force\_constant = 1.0}\par
\setlength{\parindent}{10pt}\texttt{charge = 0}\par
\smallskip
\end{tcolorbox}

\setlength{\parindent}{5pt} \robot \hspace{2pt} \textbf{Estructural}

\begin{tcolorbox}[
    colback=matterbg2,
    colframe=mattergreen1,
    width=\textwidth,
    arc=2mm,
    boxrule=0.2mm,
    leftrule=0.2mm, rightrule=0.2mm,
    toprule=0.2mm, bottomrule=0.2mm,
    enhanced,
    breakable
]
\textbf{Action:}

\begin{markdown}
Both revised TS structures generated. Let me visualize and verify the distances:
\end{markdown}

\textbf{Tool used:}

\setlength{\parindent}{5pt}\underline{\texttt{Tool Name:}} \texttt{view\_molecule}\par
\setlength{\parindent}{5pt}\underline{\texttt{Arguments:}}\par
\setlength{\parindent}{10pt}\texttt{xyz\_file\_relative\_path = TS\_pathwayA\_revised.xyz}\par
\setlength{\parindent}{10pt}\texttt{left\_right\_deg = 0}\par
\setlength{\parindent}{10pt}\texttt{up\_down\_deg = 0}\par
\smallskip
\end{tcolorbox}

\setlength{\parindent}{5pt} \robot \hspace{2pt} \textbf{Estructural}

\begin{tcolorbox}[
    colback=matterbg2,
    colframe=mattergreen1,
    width=\textwidth,
    arc=2mm,
    boxrule=0.2mm,
    leftrule=0.2mm, rightrule=0.2mm,
    toprule=0.2mm, bottomrule=0.2mm,
    enhanced,
    breakable
]
\textbf{Action:}

\begin{markdown}
Excellent! The revised Pathway A TS shows much better geometry - you can clearly see the **triangular arrangement** of C:1, S:7, and N:5 with SO departing while C-N is forming! Let me verify the distances:
\end{markdown}

\textbf{Tool used:}

\setlength{\parindent}{5pt}\underline{\texttt{Tool Name:}} \texttt{get\_distance\_angle\_dihedral}\par
\setlength{\parindent}{5pt}\underline{\texttt{Arguments:}}\par
\setlength{\parindent}{10pt}\texttt{input\_path = TS\_pathwayA\_revised.xyz}\par
\setlength{\parindent}{10pt}\texttt{targets = [\{"atom": [7]\}, \{"atom": [1]\}]}\par
\smallskip
\end{tcolorbox}

\setlength{\parindent}{5pt} \robot \hspace{2pt} \textbf{Estructural}

\begin{tcolorbox}[
    colback=matterbg2,
    colframe=mattergreen1,
    width=\textwidth,
    arc=2mm,
    boxrule=0.2mm,
    leftrule=0.2mm, rightrule=0.2mm,
    toprule=0.2mm, bottomrule=0.2mm,
    enhanced,
    breakable
]
\textbf{Tool used:}

\setlength{\parindent}{5pt}\underline{\texttt{Tool Name:}} \texttt{get\_distance\_angle\_dihedral}\par
\setlength{\parindent}{5pt}\underline{\texttt{Arguments:}}\par
\setlength{\parindent}{10pt}\texttt{input\_path = TS\_pathwayA\_revised.xyz}\par
\setlength{\parindent}{10pt}\texttt{targets = [\{"atom": [7]\}, \{"atom": [5]\}]}\par
\smallskip
\end{tcolorbox}

\setlength{\parindent}{5pt} \robot \hspace{2pt} \textbf{Estructural}

\begin{tcolorbox}[
    colback=matterbg2,
    colframe=mattergreen1,
    width=\textwidth,
    arc=2mm,
    boxrule=0.2mm,
    leftrule=0.2mm, rightrule=0.2mm,
    toprule=0.2mm, bottomrule=0.2mm,
    enhanced,
    breakable
]
\textbf{Tool used:}

\setlength{\parindent}{5pt}\underline{\texttt{Tool Name:}} \texttt{get\_distance\_angle\_dihedral}\par
\setlength{\parindent}{5pt}\underline{\texttt{Arguments:}}\par
\setlength{\parindent}{10pt}\texttt{input\_path = TS\_pathwayA\_revised.xyz}\par
\setlength{\parindent}{10pt}\texttt{targets = [\{"atom": [1]\}, \{"atom": [5]\}]}\par
\smallskip
\end{tcolorbox}

\setlength{\parindent}{5pt} \robot \hspace{2pt} \textbf{Estructural}

\begin{tcolorbox}[
    colback=matterbg2,
    colframe=mattergreen1,
    width=\textwidth,
    arc=2mm,
    boxrule=0.2mm,
    leftrule=0.2mm, rightrule=0.2mm,
    toprule=0.2mm, bottomrule=0.2mm,
    enhanced,
    breakable
]
\textbf{Action:}

\begin{markdown}
**Pathway A Revised TS - All distances verified:**
- S:7-C:1 = **2.19 Å** (breaking) $\checkmark$
- S:7-N:5 = **2.10 Å** (breaking) $\checkmark$
- C:1-N:5 = **1.89 Å** (forming) $\checkmark$ $\leftarrow$ **Much improved from 3.14 Å!**

Now let me verify Pathway B:
\end{markdown}

\textbf{Tool used:}

\setlength{\parindent}{5pt}\underline{\texttt{Tool Name:}} \texttt{view\_molecule}\par
\setlength{\parindent}{5pt}\underline{\texttt{Arguments:}}\par
\setlength{\parindent}{10pt}\texttt{xyz\_file\_relative\_path = TS\_pathwayB\_revised.xyz}\par
\setlength{\parindent}{10pt}\texttt{left\_right\_deg = 0}\par
\setlength{\parindent}{10pt}\texttt{up\_down\_deg = 0}\par
\smallskip
\end{tcolorbox}

\setlength{\parindent}{5pt} \robot \hspace{2pt} \textbf{Estructural}

\begin{tcolorbox}[
    colback=matterbg2,
    colframe=mattergreen1,
    width=\textwidth,
    arc=2mm,
    boxrule=0.2mm,
    leftrule=0.2mm, rightrule=0.2mm,
    toprule=0.2mm, bottomrule=0.2mm,
    enhanced,
    breakable
]
\textbf{Action:}

\begin{markdown}
Pathway B TS also shows excellent geometry with the **triangular C-S-N arrangement**. Let me verify the distances:
\end{markdown}

\textbf{Tool used:}

\setlength{\parindent}{5pt}\underline{\texttt{Tool Name:}} \texttt{get\_distance\_angle\_dihedral}\par
\setlength{\parindent}{5pt}\underline{\texttt{Arguments:}}\par
\setlength{\parindent}{10pt}\texttt{input\_path = TS\_pathwayB\_revised.xyz}\par
\setlength{\parindent}{10pt}\texttt{targets = [\{"atom": [7]\}, \{"atom": [1]\}]}\par
\smallskip
\end{tcolorbox}

\setlength{\parindent}{5pt} \robot \hspace{2pt} \textbf{Estructural}

\begin{tcolorbox}[
    colback=matterbg2,
    colframe=mattergreen1,
    width=\textwidth,
    arc=2mm,
    boxrule=0.2mm,
    leftrule=0.2mm, rightrule=0.2mm,
    toprule=0.2mm, bottomrule=0.2mm,
    enhanced,
    breakable
]
\textbf{Tool used:}

\setlength{\parindent}{5pt}\underline{\texttt{Tool Name:}} \texttt{get\_distance\_angle\_dihedral}\par
\setlength{\parindent}{5pt}\underline{\texttt{Arguments:}}\par
\setlength{\parindent}{10pt}\texttt{input\_path = TS\_pathwayB\_revised.xyz}\par
\setlength{\parindent}{10pt}\texttt{targets = [\{"atom": [7]\}, \{"atom": [6]\}]}\par
\smallskip
\end{tcolorbox}

\setlength{\parindent}{5pt} \robot \hspace{2pt} \textbf{Estructural}

\begin{tcolorbox}[
    colback=matterbg2,
    colframe=mattergreen1,
    width=\textwidth,
    arc=2mm,
    boxrule=0.2mm,
    leftrule=0.2mm, rightrule=0.2mm,
    toprule=0.2mm, bottomrule=0.2mm,
    enhanced,
    breakable
]
\textbf{Tool used:}

\setlength{\parindent}{5pt}\underline{\texttt{Tool Name:}} \texttt{get\_distance\_angle\_dihedral}\par
\setlength{\parindent}{5pt}\underline{\texttt{Arguments:}}\par
\setlength{\parindent}{10pt}\texttt{input\_path = TS\_pathwayB\_revised.xyz}\par
\setlength{\parindent}{10pt}\texttt{targets = [\{"atom": [1]\}, \{"atom": [6]\}]}\par
\smallskip
\end{tcolorbox}

\setlength{\parindent}{5pt} \robot \hspace{2pt} \textbf{Estructural}

\begin{tcolorbox}[
    colback=matterbg2,
    colframe=mattergreen1,
    width=\textwidth,
    arc=2mm,
    boxrule=0.2mm,
    leftrule=0.2mm, rightrule=0.2mm,
    toprule=0.2mm, bottomrule=0.2mm,
    enhanced,
    breakable
]
\textbf{Action:}

\begin{markdown}
**Pathway B Revised TS - All distances verified:**
- S:7-C:1 = **2.19 Å** (breaking) $\checkmark$
- S:7-N:6 = **2.11 Å** (breaking) $\checkmark$
- C:1-N:6 = **1.89 Å** (forming) $\checkmark$ $\leftarrow$ **Much improved from 2.81 Å!**

---

****Revised TS Summary - Proper Ring Contraction Geometry****

****Key Insight: Three-Bond TS for 6$\rightarrow$5 Ring Contraction****

The SO extrusion involves a **concerted process** with:
- Two bonds **breaking** (S-C, S-N)
- One bond **forming** (C-N)

| Distance | Original TS | Revised TS | Description |
|----------|-------------|------------|-------------|
| **S-C** | ~2.28 Å | ~2.19 Å | Breaking (from ~1.8 Å) |
| **S-N** | ~2.19 Å | ~2.10 Å | Breaking (from ~1.7 Å) |
| **C-N** | **3.14 / 2.81 Å** | **1.89 Å** | **Forming (toward ~1.4 Å)** |

---

****Comparison: Original vs Revised TS Geometries****

| Pathway | Bond | Original | Revised | Improvement |
|---------|------|----------|---------|-------------|
| **A** | S:7-C:1 | 2.28 Å | 2.19 Å | $\checkmark$ |
| **A** | S:7-N:5 | 2.19 Å | 2.10 Å | $\checkmark$ |
| **A** | C:1-N:5 | **3.14 Å** | **1.89 Å** | **$-$1.25 Å** |
| **B** | S:7-C:1 | 2.28 Å | 2.19 Å | $\checkmark$ |
| **B** | S:7-N:6 | 2.19 Å | 2.11 Å | $\checkmark$ |
| **B** | C:1-N:6 | **2.81 Å** | **1.89 Å** | **$-$0.92 Å** |

---

****Revised Files Generated****

| Pathway | File | Key Features |
|---------|------|--------------|
| **A** | `TS_pathwayA_revised.xyz` | N-Me on N:5 (adj. to S), C-N forming at 1.89 Å |
| **B** | `TS_pathwayB_revised.xyz` | N-Me on N:4 (away from S), C-N forming at 1.89 Å |

---

****TS Geometry Interpretation****

The revised TS structures now correctly show:

```
        O
        ‖
        S $\leftarrow$ leaving group
       / \
      /   \  (both bonds elongating ~2.1-2.2 Å)
     C-----N  $\leftarrow$ new bond forming (~1.9 Å)
    / \   |
   Me  \  |
        Ring continues...
```

This represents a **synchronous** transition state where:
- SO departs "above" the plane
- C and N come together "below" to close the 5-membered pyrazole ring
- The three key atoms form a **triangular** arrangement characteristic of ring contraction TSs

Thank you for catching that important oversight! The revised TS geometries are now chemically reasonable for a 6$\rightarrow$5 ring contraction process with concurrent bond breaking and formation.
\end{markdown}

\end{tcolorbox}

\setlength{\parindent}{5pt} \textbf{\textcolor{blue}{User:}}
\begin{tcolorbox}[
    colback=blue!10,
    colframe=blue,
    width=\textwidth,
    arc=2mm,
    boxrule=0.2mm,
    leftrule=0.2mm, rightrule=0.2mm,
    toprule=0.2mm, bottomrule=0.2mm,
    enhanced,
    breakable
]
\begin{markdown}
TS\\textunderscore{}B seems has protonated N for bond breaking/forming, a hint is it can undergo proton transfer with solvent. With this in knowledge, relocate files to common, path\\textunderscore{}A, path\\textunderscore{}B, misc, and optimize crucial structures like key intermediates and both TS. Be careful on force constant when using xtb to run optimizations.
\end{markdown}
\end{tcolorbox}
\setlength{\parindent}{5pt} \robot \hspace{2pt} \textbf{Estructural}

\begin{tcolorbox}[
    colback=matterbg2,
    colframe=mattergreen1,
    width=\textwidth,
    arc=2mm,
    boxrule=0.2mm,
    leftrule=0.2mm, rightrule=0.2mm,
    toprule=0.2mm, bottomrule=0.2mm,
    enhanced,
    breakable
]
\textbf{Action:}

\begin{markdown}
Great point! In Pathway B, the N:6 (adjacent to S) is protonated with H:17, but for proper bond formation/breaking, it should be deprotonated (proton transferred to solvent). Let me:

1. Create directories and organize files
2. Create deprotonated Pathway B intermediate
3. Optimize all key structures

First, let me create the directory structure and move files:
\end{markdown}

\textbf{Tool used:}

\setlength{\parindent}{5pt}\underline{\texttt{Tool Name:}} \texttt{repl\_tool}\par
\setlength{\parindent}{5pt}\underline{\texttt{Arguments:}}\par
\setlength{\parindent}{10pt}\texttt{code =}\par
\begin{verbatim}

import os
import shutil

# Create directories
directories = ['common', 'path_A', 'path_B', 'misc']
for d in directories:
    os.makedirs(d, exist_ok=True)
    print(f"Created directory: {d}")

# Define file organization
common_files = [
    '5-methylisothiazole_substrate.xyz',
    '3-methyl-1H-pyrazole_product.xyz',
    'pre-oxidized_NH-thiadiazine.xyz',
    'NH_TDSO_intermediate.xyz'
]

path_A_files = [
    'N5-Me_TDSO_pathwayA.xyz',
    'TS_pathwayA_revised.xyz'
]

path_B_files = [
    'N4-Me_TDSO_pathwayB.xyz',  # Will be replaced with deprotonated version
    'TS_pathwayB_revised.xyz'   # Will be replaced with deprotonated version
]

misc_files = [
    'Reaction.png',
    'TS.png',
    'TS_pathwayA_SO_extrusion.xyz',
    'TS_pathwayA_SO_extrusion.log',
    'TS_pathwayB_SO_extrusion.xyz',
    'TS_pathwayB_SO_extrusion.log',
    'TS_pathwayA_revised.log',
    'TS_pathwayB_revised.log',
    'file_log.txt'
]

# Move files
for f in common_files:
    if os.path.exists(f):
        shutil.copy(f, f'common/{f}')
        print(f"Copied {f} -> common/")

for f in path_A_files:
    if os.path.exists(f):
        shutil.copy(f, f'path_A/{f}')
        print(f"Copied {f} -> path_A/")

for f in path_B_files:
    if os.path.exists(f):
        shutil.copy(f, f'path_B/{f}')
        print(f"Copied {f} -> path_B/")

for f in misc_files:
    if os.path.exists(f):
        shutil.move(f, f'misc/{f}')
        print(f"Moved {f} -> misc/")

print("
Directory organization complete!")

\end{verbatim}\par
\smallskip
\end{tcolorbox}

\setlength{\parindent}{5pt} \robot \hspace{2pt} \textbf{Estructural}

\begin{tcolorbox}[
    colback=matterbg2,
    colframe=mattergreen1,
    width=\textwidth,
    arc=2mm,
    boxrule=0.2mm,
    leftrule=0.2mm, rightrule=0.2mm,
    toprule=0.2mm, bottomrule=0.2mm,
    enhanced,
    breakable
]
\textbf{Action:}

\begin{markdown}
Directories organized. Now let me create the deprotonated Pathway B intermediate by removing H:17 from N:6:
\end{markdown}

\textbf{Tool used:}

\setlength{\parindent}{5pt}\underline{\texttt{Tool Name:}} \texttt{remove\_atoms}\par
\setlength{\parindent}{5pt}\underline{\texttt{Arguments:}}\par
\setlength{\parindent}{10pt}\texttt{input\_path = path\_B/N4-Me\_TDSO\_pathwayB.xyz}\par
\setlength{\parindent}{10pt}\texttt{atoms\_list = [17]}\par
\setlength{\parindent}{10pt}\texttt{output\_path = path\_B/N4-Me\_TDSO\_deprotonated.xyz}\par
\smallskip
\end{tcolorbox}

\setlength{\parindent}{5pt} \robot \hspace{2pt} \textbf{Estructural}

\begin{tcolorbox}[
    colback=matterbg2,
    colframe=mattergreen1,
    width=\textwidth,
    arc=2mm,
    boxrule=0.2mm,
    leftrule=0.2mm, rightrule=0.2mm,
    toprule=0.2mm, bottomrule=0.2mm,
    enhanced,
    breakable
]
\textbf{Action:}

\begin{markdown}
Deprotonated intermediate created. Let me verify the structure and check the new atomic indices:
\end{markdown}

\textbf{Tool used:}

\setlength{\parindent}{5pt}\underline{\texttt{Tool Name:}} \texttt{view\_molecule}\par
\setlength{\parindent}{5pt}\underline{\texttt{Arguments:}}\par
\setlength{\parindent}{10pt}\texttt{xyz\_file\_relative\_path = path\_B/N4-Me\_TDSO\_deprotonated.xyz}\par
\setlength{\parindent}{10pt}\texttt{left\_right\_deg = 0}\par
\setlength{\parindent}{10pt}\texttt{up\_down\_deg = 0}\par
\smallskip
\end{tcolorbox}

\setlength{\parindent}{5pt} \robot \hspace{2pt} \textbf{Estructural}

\begin{tcolorbox}[
    colback=matterbg2,
    colframe=mattergreen1,
    width=\textwidth,
    arc=2mm,
    boxrule=0.2mm,
    leftrule=0.2mm, rightrule=0.2mm,
    toprule=0.2mm, bottomrule=0.2mm,
    enhanced,
    breakable
]
\textbf{Action:}

\begin{markdown}
N:6 is now deprotonated (no H attached). The key indices remain:
- **C:1** (with Me) - adjacent to S
- **S:7** (with O:8) - SO leaving group  
- **N:6** - deprotonated, will form bond with C:1
- **N:4** (with N-Me/C:5)

Now let me optimize all crucial structures. Starting with **common structures**:
\end{markdown}

\textbf{Tool used:}

\setlength{\parindent}{5pt}\underline{\texttt{Tool Name:}} \texttt{constraint\_xtb}\par
\setlength{\parindent}{5pt}\underline{\texttt{Arguments:}}\par
\setlength{\parindent}{10pt}\texttt{input\_xyz = common/5-methylisothiazole\_substrate.xyz}\par
\setlength{\parindent}{10pt}\texttt{output\_xyz = common/5-methylisothiazole\_substrate\_opt.xyz}\par
\setlength{\parindent}{10pt}\texttt{charge = 0}\par
\smallskip
\end{tcolorbox}

\setlength{\parindent}{5pt} \robot \hspace{2pt} \textbf{Estructural}

\begin{tcolorbox}[
    colback=matterbg2,
    colframe=mattergreen1,
    width=\textwidth,
    arc=2mm,
    boxrule=0.2mm,
    leftrule=0.2mm, rightrule=0.2mm,
    toprule=0.2mm, bottomrule=0.2mm,
    enhanced,
    breakable
]
\textbf{Tool used:}

\setlength{\parindent}{5pt}\underline{\texttt{Tool Name:}} \texttt{constraint\_xtb}\par
\setlength{\parindent}{5pt}\underline{\texttt{Arguments:}}\par
\setlength{\parindent}{10pt}\texttt{input\_xyz = common/3-methyl-1H-pyrazole\_product.xyz}\par
\setlength{\parindent}{10pt}\texttt{output\_xyz = common/3-methyl-1H-pyrazole\_product\_opt.xyz}\par
\setlength{\parindent}{10pt}\texttt{charge = 0}\par
\smallskip
\end{tcolorbox}

\setlength{\parindent}{5pt} \robot \hspace{2pt} \textbf{Estructural}

\begin{tcolorbox}[
    colback=matterbg2,
    colframe=mattergreen1,
    width=\textwidth,
    arc=2mm,
    boxrule=0.2mm,
    leftrule=0.2mm, rightrule=0.2mm,
    toprule=0.2mm, bottomrule=0.2mm,
    enhanced,
    breakable
]
\textbf{Tool used:}

\setlength{\parindent}{5pt}\underline{\texttt{Tool Name:}} \texttt{constraint\_xtb}\par
\setlength{\parindent}{5pt}\underline{\texttt{Arguments:}}\par
\setlength{\parindent}{10pt}\texttt{input\_xyz = common/pre-oxidized\_NH-thiadiazine.xyz}\par
\setlength{\parindent}{10pt}\texttt{output\_xyz = common/pre-oxidized\_NH-thiadiazine\_opt.xyz}\par
\setlength{\parindent}{10pt}\texttt{charge = 0}\par
\smallskip
\end{tcolorbox}

\setlength{\parindent}{5pt} \robot \hspace{2pt} \textbf{Estructural}

\begin{tcolorbox}[
    colback=matterbg2,
    colframe=mattergreen1,
    width=\textwidth,
    arc=2mm,
    boxrule=0.2mm,
    leftrule=0.2mm, rightrule=0.2mm,
    toprule=0.2mm, bottomrule=0.2mm,
    enhanced,
    breakable
]
\textbf{Tool used:}

\setlength{\parindent}{5pt}\underline{\texttt{Tool Name:}} \texttt{constraint\_xtb}\par
\setlength{\parindent}{5pt}\underline{\texttt{Arguments:}}\par
\setlength{\parindent}{10pt}\texttt{input\_xyz = common/NH\_TDSO\_intermediate.xyz}\par
\setlength{\parindent}{10pt}\texttt{output\_xyz = common/NH\_TDSO\_intermediate\_opt.xyz}\par
\setlength{\parindent}{10pt}\texttt{charge = 0}\par
\smallskip
\end{tcolorbox}

\setlength{\parindent}{5pt} \robot \hspace{2pt} \textbf{Estructural}

\begin{tcolorbox}[
    colback=matterbg2,
    colframe=mattergreen1,
    width=\textwidth,
    arc=2mm,
    boxrule=0.2mm,
    leftrule=0.2mm, rightrule=0.2mm,
    toprule=0.2mm, bottomrule=0.2mm,
    enhanced,
    breakable
]
\textbf{Action:}

\begin{markdown}
Common structures optimized. Now **Pathway A** structures:
\end{markdown}

\textbf{Tool used:}

\setlength{\parindent}{5pt}\underline{\texttt{Tool Name:}} \texttt{constraint\_xtb}\par
\setlength{\parindent}{5pt}\underline{\texttt{Arguments:}}\par
\setlength{\parindent}{10pt}\texttt{input\_xyz = path\_A/N5-Me\_TDSO\_pathwayA.xyz}\par
\setlength{\parindent}{10pt}\texttt{output\_xyz = path\_A/N5-Me\_TDSO\_pathwayA\_opt.xyz}\par
\setlength{\parindent}{10pt}\texttt{charge = 0}\par
\smallskip
\end{tcolorbox}

\setlength{\parindent}{5pt} \robot \hspace{2pt} \textbf{Estructural}

\begin{tcolorbox}[
    colback=matterbg2,
    colframe=mattergreen1,
    width=\textwidth,
    arc=2mm,
    boxrule=0.2mm,
    leftrule=0.2mm, rightrule=0.2mm,
    toprule=0.2mm, bottomrule=0.2mm,
    enhanced,
    breakable
]
\textbf{Action:}

\begin{markdown}
Now let me check the optimized Pathway A intermediate to verify indices before TS optimization:
\end{markdown}

\textbf{Tool used:}

\setlength{\parindent}{5pt}\underline{\texttt{Tool Name:}} \texttt{view\_molecule}\par
\setlength{\parindent}{5pt}\underline{\texttt{Arguments:}}\par
\setlength{\parindent}{10pt}\texttt{xyz\_file\_relative\_path = path\_A/N5-Me\_TDSO\_pathwayA\_opt.xyz}\par
\setlength{\parindent}{10pt}\texttt{left\_right\_deg = 0}\par
\setlength{\parindent}{10pt}\texttt{up\_down\_deg = 0}\par
\smallskip
\end{tcolorbox}

\setlength{\parindent}{5pt} \robot \hspace{2pt} \textbf{Estructural}

\begin{tcolorbox}[
    colback=matterbg2,
    colframe=mattergreen1,
    width=\textwidth,
    arc=2mm,
    boxrule=0.2mm,
    leftrule=0.2mm, rightrule=0.2mm,
    toprule=0.2mm, bottomrule=0.2mm,
    enhanced,
    breakable
]
\textbf{Action:}

\begin{markdown}
Good, indices confirmed for Pathway A. Now let me generate the TS from the optimized intermediate with careful force constant:
\end{markdown}

\textbf{Tool used:}

\setlength{\parindent}{5pt}\underline{\texttt{Tool Name:}} \texttt{constraint\_xtb}\par
\setlength{\parindent}{5pt}\underline{\texttt{Arguments:}}\par
\setlength{\parindent}{10pt}\texttt{input\_xyz = path\_A/N5-Me\_TDSO\_pathwayA\_opt.xyz}\par
\setlength{\parindent}{10pt}\texttt{output\_xyz = path\_A/TS\_pathwayA\_opt.xyz}\par
\setlength{\parindent}{10pt}\texttt{distance\_constraints = [\{"atoms": [7, 1], "value": 2.2\}, \{"atoms": [7, 5], "value": 2.1\}, \{"atoms": [1, 5], "value": 1.9\}]}\par
\setlength{\parindent}{10pt}\texttt{force\_constant = 0.5}\par
\setlength{\parindent}{10pt}\texttt{charge = 0}\par
\smallskip
\end{tcolorbox}

\setlength{\parindent}{5pt} \robot \hspace{2pt} \textbf{Estructural}

\begin{tcolorbox}[
    colback=matterbg2,
    colframe=mattergreen1,
    width=\textwidth,
    arc=2mm,
    boxrule=0.2mm,
    leftrule=0.2mm, rightrule=0.2mm,
    toprule=0.2mm, bottomrule=0.2mm,
    enhanced,
    breakable
]
\textbf{Action:}

\begin{markdown}
Pathway A TS generated. Let me verify the distances:
\end{markdown}

\textbf{Tool used:}

\setlength{\parindent}{5pt}\underline{\texttt{Tool Name:}} \texttt{get\_distance\_angle\_dihedral}\par
\setlength{\parindent}{5pt}\underline{\texttt{Arguments:}}\par
\setlength{\parindent}{10pt}\texttt{input\_path = path\_A/TS\_pathwayA\_opt.xyz}\par
\setlength{\parindent}{10pt}\texttt{targets = [\{"atom": [7]\}, \{"atom": [1]\}]}\par
\smallskip
\end{tcolorbox}

\setlength{\parindent}{5pt} \robot \hspace{2pt} \textbf{Estructural}

\begin{tcolorbox}[
    colback=matterbg2,
    colframe=mattergreen1,
    width=\textwidth,
    arc=2mm,
    boxrule=0.2mm,
    leftrule=0.2mm, rightrule=0.2mm,
    toprule=0.2mm, bottomrule=0.2mm,
    enhanced,
    breakable
]
\textbf{Tool used:}

\setlength{\parindent}{5pt}\underline{\texttt{Tool Name:}} \texttt{get\_distance\_angle\_dihedral}\par
\setlength{\parindent}{5pt}\underline{\texttt{Arguments:}}\par
\setlength{\parindent}{10pt}\texttt{input\_path = path\_A/TS\_pathwayA\_opt.xyz}\par
\setlength{\parindent}{10pt}\texttt{targets = [\{"atom": [7]\}, \{"atom": [5]\}]}\par
\smallskip
\end{tcolorbox}

\setlength{\parindent}{5pt} \robot \hspace{2pt} \textbf{Estructural}

\begin{tcolorbox}[
    colback=matterbg2,
    colframe=mattergreen1,
    width=\textwidth,
    arc=2mm,
    boxrule=0.2mm,
    leftrule=0.2mm, rightrule=0.2mm,
    toprule=0.2mm, bottomrule=0.2mm,
    enhanced,
    breakable
]
\textbf{Tool used:}

\setlength{\parindent}{5pt}\underline{\texttt{Tool Name:}} \texttt{get\_distance\_angle\_dihedral}\par
\setlength{\parindent}{5pt}\underline{\texttt{Arguments:}}\par
\setlength{\parindent}{10pt}\texttt{input\_path = path\_A/TS\_pathwayA\_opt.xyz}\par
\setlength{\parindent}{10pt}\texttt{targets = [\{"atom": [1]\}, \{"atom": [5]\}]}\par
\smallskip
\end{tcolorbox}

\setlength{\parindent}{5pt} \robot \hspace{2pt} \textbf{Estructural}

\begin{tcolorbox}[
    colback=matterbg2,
    colframe=mattergreen1,
    width=\textwidth,
    arc=2mm,
    boxrule=0.2mm,
    leftrule=0.2mm, rightrule=0.2mm,
    toprule=0.2mm, bottomrule=0.2mm,
    enhanced,
    breakable
]
\textbf{Action:}

\begin{markdown}
Pathway A TS verified:
- S:7-C:1 = **2.19 Å** $\checkmark$
- S:7-N:5 = **2.09 Å** $\checkmark$
- C:1-N:5 = **1.88 Å** $\checkmark$

Now let me optimize **Pathway B** (deprotonated, charge=-1):
\end{markdown}

\textbf{Tool used:}

\setlength{\parindent}{5pt}\underline{\texttt{Tool Name:}} \texttt{constraint\_xtb}\par
\setlength{\parindent}{5pt}\underline{\texttt{Arguments:}}\par
\setlength{\parindent}{10pt}\texttt{input\_xyz = path\_B/N4-Me\_TDSO\_deprotonated.xyz}\par
\setlength{\parindent}{10pt}\texttt{output\_xyz = path\_B/N4-Me\_TDSO\_deprotonated\_opt.xyz}\par
\setlength{\parindent}{10pt}\texttt{charge = -1}\par
\smallskip
\end{tcolorbox}

\setlength{\parindent}{5pt} \robot \hspace{2pt} \textbf{Estructural}

\begin{tcolorbox}[
    colback=matterbg2,
    colframe=mattergreen1,
    width=\textwidth,
    arc=2mm,
    boxrule=0.2mm,
    leftrule=0.2mm, rightrule=0.2mm,
    toprule=0.2mm, bottomrule=0.2mm,
    enhanced,
    breakable
]
\textbf{Action:}

\begin{markdown}
Pathway B intermediate optimized. Let me verify the indices in the optimized deprotonated structure:
\end{markdown}

\textbf{Tool used:}

\setlength{\parindent}{5pt}\underline{\texttt{Tool Name:}} \texttt{view\_molecule}\par
\setlength{\parindent}{5pt}\underline{\texttt{Arguments:}}\par
\setlength{\parindent}{10pt}\texttt{xyz\_file\_relative\_path = path\_B/N4-Me\_TDSO\_deprotonated\_opt.xyz}\par
\setlength{\parindent}{10pt}\texttt{left\_right\_deg = 0}\par
\setlength{\parindent}{10pt}\texttt{up\_down\_deg = 0}\par
\smallskip
\end{tcolorbox}

\setlength{\parindent}{5pt} \robot \hspace{2pt} \textbf{Estructural}

\begin{tcolorbox}[
    colback=matterbg2,
    colframe=mattergreen1,
    width=\textwidth,
    arc=2mm,
    boxrule=0.2mm,
    leftrule=0.2mm, rightrule=0.2mm,
    toprule=0.2mm, bottomrule=0.2mm,
    enhanced,
    breakable
]
\textbf{Action:}

\begin{markdown}
Deprotonated structure verified:
- **N:6** is now deprotonated (no H attached) $\checkmark$
- **C:1** (with Me/C:0) adjacent to S
- **S:7** (with O:8) - SO leaving group
- **N:4** (with N-Me/C:5)

Now let me generate the Pathway B deprotonated TS (charge=-1):
\end{markdown}

\textbf{Tool used:}

\setlength{\parindent}{5pt}\underline{\texttt{Tool Name:}} \texttt{constraint\_xtb}\par
\setlength{\parindent}{5pt}\underline{\texttt{Arguments:}}\par
\setlength{\parindent}{10pt}\texttt{input\_xyz = path\_B/N4-Me\_TDSO\_deprotonated\_opt.xyz}\par
\setlength{\parindent}{10pt}\texttt{output\_xyz = path\_B/TS\_pathwayB\_deprotonated\_opt.xyz}\par
\setlength{\parindent}{10pt}\texttt{distance\_constraints = [\{"atoms": [7, 1], "value": 2.2\}, \{"atoms": [7, 6], "value": 2.1\}, \{"atoms": [1, 6], "value": 1.9\}]}\par
\setlength{\parindent}{10pt}\texttt{force\_constant = 0.5}\par
\setlength{\parindent}{10pt}\texttt{charge = -1}\par
\smallskip
\end{tcolorbox}

\setlength{\parindent}{5pt} \robot \hspace{2pt} \textbf{Estructural}

\begin{tcolorbox}[
    colback=matterbg2,
    colframe=mattergreen1,
    width=\textwidth,
    arc=2mm,
    boxrule=0.2mm,
    leftrule=0.2mm, rightrule=0.2mm,
    toprule=0.2mm, bottomrule=0.2mm,
    enhanced,
    breakable
]
\textbf{Action:}

\begin{markdown}
Pathway B TS generated. Let me verify the distances:
\end{markdown}

\textbf{Tool used:}

\setlength{\parindent}{5pt}\underline{\texttt{Tool Name:}} \texttt{get\_distance\_angle\_dihedral}\par
\setlength{\parindent}{5pt}\underline{\texttt{Arguments:}}\par
\setlength{\parindent}{10pt}\texttt{input\_path = path\_B/TS\_pathwayB\_deprotonated\_opt.xyz}\par
\setlength{\parindent}{10pt}\texttt{targets = [\{"atom": [7]\}, \{"atom": [1]\}]}\par
\smallskip
\end{tcolorbox}

\setlength{\parindent}{5pt} \robot \hspace{2pt} \textbf{Estructural}

\begin{tcolorbox}[
    colback=matterbg2,
    colframe=mattergreen1,
    width=\textwidth,
    arc=2mm,
    boxrule=0.2mm,
    leftrule=0.2mm, rightrule=0.2mm,
    toprule=0.2mm, bottomrule=0.2mm,
    enhanced,
    breakable
]
\textbf{Tool used:}

\setlength{\parindent}{5pt}\underline{\texttt{Tool Name:}} \texttt{get\_distance\_angle\_dihedral}\par
\setlength{\parindent}{5pt}\underline{\texttt{Arguments:}}\par
\setlength{\parindent}{10pt}\texttt{input\_path = path\_B/TS\_pathwayB\_deprotonated\_opt.xyz}\par
\setlength{\parindent}{10pt}\texttt{targets = [\{"atom": [7]\}, \{"atom": [6]\}]}\par
\smallskip
\end{tcolorbox}

\setlength{\parindent}{5pt} \robot \hspace{2pt} \textbf{Estructural}

\begin{tcolorbox}[
    colback=matterbg2,
    colframe=mattergreen1,
    width=\textwidth,
    arc=2mm,
    boxrule=0.2mm,
    leftrule=0.2mm, rightrule=0.2mm,
    toprule=0.2mm, bottomrule=0.2mm,
    enhanced,
    breakable
]
\textbf{Tool used:}

\setlength{\parindent}{5pt}\underline{\texttt{Tool Name:}} \texttt{get\_distance\_angle\_dihedral}\par
\setlength{\parindent}{5pt}\underline{\texttt{Arguments:}}\par
\setlength{\parindent}{10pt}\texttt{input\_path = path\_B/TS\_pathwayB\_deprotonated\_opt.xyz}\par
\setlength{\parindent}{10pt}\texttt{targets = [\{"atom": [1]\}, \{"atom": [6]\}]}\par
\smallskip
\end{tcolorbox}

\setlength{\parindent}{5pt} \robot \hspace{2pt} \textbf{Estructural}

\begin{tcolorbox}[
    colback=matterbg2,
    colframe=mattergreen1,
    width=\textwidth,
    arc=2mm,
    boxrule=0.2mm,
    leftrule=0.2mm, rightrule=0.2mm,
    toprule=0.2mm, bottomrule=0.2mm,
    enhanced,
    breakable
]
\textbf{Action:}

\begin{markdown}
Pathway B TS verified:
- S:7-C:1 = **2.20 Å** $\checkmark$
- S:7-N:6 = **2.09 Å** $\checkmark$  
- C:1-N:6 = **1.86 Å** $\checkmark$

Now let me clean up the remaining files in the root directory:
\end{markdown}

\textbf{Tool used:}

\setlength{\parindent}{5pt}\underline{\texttt{Tool Name:}} \texttt{repl\_tool}\par
\setlength{\parindent}{5pt}\underline{\texttt{Arguments:}}\par
\setlength{\parindent}{10pt}\texttt{code =}\par
\begin{verbatim}

import os
import shutil

# Files to move to misc (old/duplicate files in root)
root_files_to_misc = [
    '3-methyl-1H-pyrazole_product.xyz',
    '5-methylisothiazole_substrate.xyz',
    'N4-Me_TDSO_pathwayB.xyz',
    'N5-Me_TDSO_pathwayA.xyz',
    'NH_TDSO_intermediate.xyz',
    'TS_pathwayA_revised.xyz',
    'TS_pathwayB_revised.xyz',
    'pre-oxidized_NH-thiadiazine.xyz',
    'file_log.txt'
]

# Move remaining root files to misc
for f in root_files_to_misc:
    if os.path.exists(f):
        shutil.move(f, f'misc/{f}')
        print(f"Moved {f} -> misc/")

# Remove view json files from root (they're cached visualization files)
for f in os.listdir('.'):
    if f.endswith('.view.json'):
        os.remove(f)
        print(f"Removed cache file: {f}")

print("
=== Final Directory Structure ===")
for root, dirs, files in os.walk('.'):
    # Skip hidden directories
    dirs[:] = [d for d in dirs if not d.startswith('.')]
    level = root.replace('.', '').count(os.sep)
    indent = ' ' * 2 * level
    print(f'{indent}{os.path.basename(root)}/')
    subindent = ' ' * 2 * (level + 1)
    for file in sorted(files):
        if not file.startswith('.'):
            print(f'{subindent}{file}')

\end{verbatim}\par
\smallskip
\end{tcolorbox}

\setlength{\parindent}{5pt} \robot \hspace{2pt} \textbf{Estructural}

\begin{tcolorbox}[
    colback=matterbg2,
    colframe=mattergreen1,
    width=\textwidth,
    arc=2mm,
    boxrule=0.2mm,
    leftrule=0.2mm, rightrule=0.2mm,
    toprule=0.2mm, bottomrule=0.2mm,
    enhanced,
    breakable
]
\textbf{Action:}

\begin{markdown}
Files organized. Let me visualize the final Pathway B deprotonated TS structure:
\end{markdown}

\textbf{Tool used:}

\setlength{\parindent}{5pt}\underline{\texttt{Tool Name:}} \texttt{view\_molecule}\par
\setlength{\parindent}{5pt}\underline{\texttt{Arguments:}}\par
\setlength{\parindent}{10pt}\texttt{xyz\_file\_relative\_path = path\_B/TS\_pathwayB\_deprotonated\_opt.xyz}\par
\setlength{\parindent}{10pt}\texttt{left\_right\_deg = 0}\par
\setlength{\parindent}{10pt}\texttt{up\_down\_deg = 0}\par
\smallskip
\end{tcolorbox}

\setlength{\parindent}{5pt} \robot \hspace{2pt} \textbf{Estructural}

\begin{tcolorbox}[
    colback=matterbg2,
    colframe=mattergreen1,
    width=\textwidth,
    arc=2mm,
    boxrule=0.2mm,
    leftrule=0.2mm, rightrule=0.2mm,
    toprule=0.2mm, bottomrule=0.2mm,
    enhanced,
    breakable
]
\textbf{Action:}

\begin{markdown}
Excellent! The **Pathway B deprotonated TS** shows the proper geometry:
- **N:6 is deprotonated** (no H) - ready for nucleophilic attack on C:1
- **Triangular C:1-S:7-N:6** arrangement with SO departing
- **N:4 has N-Me** (C:5) - the alkylation away from S

---

****Final Summary: Organized File Structure \\& Optimized Structures****

****Directory Organization****

```
+-- common/                          # Shared structures
|   +-- 5-methylisothiazole_substrate_opt.xyz    $\leftarrow$ OPTIMIZED substrate
|   +-- 3-methyl-1H-pyrazole_product_opt.xyz     $\leftarrow$ OPTIMIZED product
|   +-- pre-oxidized_NH-thiadiazine_opt.xyz      $\leftarrow$ OPTIMIZED (before S oxidation)
|   +-- NH_TDSO_intermediate_opt.xyz             $\leftarrow$ OPTIMIZED (after S oxidation)
|
+-- path_A/                          # N-alkylation on N adjacent to S
|   +-- N5-Me_TDSO_pathwayA_opt.xyz              $\leftarrow$ OPTIMIZED intermediate
|   +-- TS_pathwayA_opt.xyz                      $\leftarrow$ OPTIMIZED TS (charge=0)
|
+-- path_B/                          # N-alkylation on N away from S
|   +-- N4-Me_TDSO_deprotonated_opt.xyz          $\leftarrow$ OPTIMIZED (N:6 deprotonated)
|   +-- TS_pathwayB_deprotonated_opt.xyz         $\leftarrow$ OPTIMIZED TS (charge=-1)
|
+-- misc/                            # Old files, images, logs
    +-- Reaction.png, TS.png
    +-- (old TS versions, unoptimized structures)
```

---

****Key Mechanistic Difference: Pathways A vs B****

| Feature | **Pathway A** | **Pathway B** |
|---------|---------------|---------------|
| **N-Me position** | N:5 (adjacent to S) | N:4 (away from S) |
| **Bond-forming N** | N:5 (methylated) | N:6 (deprotonated) |
| **Charge** | Neutral (0) | Anionic (-1) |
| **Proton transfer** | Not required | Required ($\rightarrow$ solvent) |
| **Product** | 1,3-dimethylpyrazole | 2,3-dimethylpyrazole |

---

****Optimized TS Geometries Verified****

| TS | S-C (breaking) | S-N (breaking) | C-N (forming) |
|----|----------------|----------------|---------------|
| **Pathway A** | 2.19 Å | 2.09 Å | 1.88 Å |
| **Pathway B** | 2.20 Å | 2.09 Å | 1.86 Å |

All distances are within target ranges with **force\\textunderscore{}constant = 0.5**.

---

****Complete Reaction Mechanism (Mark Levin-style Skeletal Editing)****

```
5-Methylisothiazole (common/...substrate_opt.xyz)
        |
        | + "NH" source
        [down]
Pre-oxidized NH-thiadiazine (common/pre-oxidized...opt.xyz)
        |
        | + O (oxidation)
        [down]
NH TDSO intermediate (common/NH_TDSO...opt.xyz)
        |
        +----------------------------------+
        |                                  |
        [down]                                  [down]
   N-alkylation on N5               N-alkylation on N4
   (path_A/N5-Me...opt.xyz)         + proton transfer to solvent
        |                           (path_B/N4-Me_deprotonated...opt.xyz)
        |                                  |
        [down]                                  [down]
   TS (path_A/TS...opt.xyz)         TS (path_B/TS_deprotonated...opt.xyz)
   [charge = 0]                     [charge = -1]
        |                                  |
        [down]                                  [down]
   1,3-dimethylpyrazole             2,3-dimethylpyrazole
```

All crucial structures are now optimized with proper charge states and TS geometries featuring the correct three-bond (2 breaking + 1 forming) ring contraction character!
\end{markdown}

\end{tcolorbox}

\setlength{\parindent}{5pt} \textbf{\textcolor{blue}{User:}}
\begin{tcolorbox}[
    colback=blue!10,
    colframe=blue,
    width=\textwidth,
    arc=2mm,
    boxrule=0.2mm,
    leftrule=0.2mm, rightrule=0.2mm,
    toprule=0.2mm, bottomrule=0.2mm,
    enhanced,
    breakable
]
\begin{markdown}
now please add and optimize the final product of each path, then plot the reaction energy profile of the SO extrusion step to compare two pathways.
\end{markdown}
\end{tcolorbox}
\setlength{\parindent}{5pt} \robot \hspace{2pt} \textbf{Estructural}

\begin{tcolorbox}[
    colback=matterbg2,
    colframe=mattergreen1,
    width=\textwidth,
    arc=2mm,
    boxrule=0.2mm,
    leftrule=0.2mm, rightrule=0.2mm,
    toprule=0.2mm, bottomrule=0.2mm,
    enhanced,
    breakable
]
\textbf{Action:}

\begin{markdown}
I'll generate and optimize the products for each pathway, then create an energy profile. 

For the products:
- **Pathway A**: 1,5-dimethyl-1H-pyrazole (N-Me adjacent to C-Me), neutral
- **Pathway B**: Pyrazolide anion initially (charge=-1), then protonated to give 1,3-dimethyl-1H-pyrazole

Let me first generate the products:
\end{markdown}

\textbf{Tool used:}

\setlength{\parindent}{5pt}\underline{\texttt{Tool Name:}} \texttt{organic\_molecules\_xyz\_generation}\par
\setlength{\parindent}{5pt}\underline{\texttt{Arguments:}}\par
\setlength{\parindent}{10pt}\texttt{smiles\_list = ["Cc1ccnn1C", "Cn1ccc(C)n1"]}\par
\setlength{\parindent}{10pt}\texttt{filenames = ["path\_A/product\_1-5-dimethylpyrazole.xyz", "path\_B/product\_1-3-dimethylpyrazole.xyz"]}\par
\smallskip
\end{tcolorbox}

\setlength{\parindent}{5pt} \robot \hspace{2pt} \textbf{Estructural}

\begin{tcolorbox}[
    colback=matterbg2,
    colframe=mattergreen1,
    width=\textwidth,
    arc=2mm,
    boxrule=0.2mm,
    leftrule=0.2mm, rightrule=0.2mm,
    toprule=0.2mm, bottomrule=0.2mm,
    enhanced,
    breakable
]
\textbf{Action:}

\begin{markdown}
Now let me optimize the products. For Pathway A (neutral) and Pathway B (need anionic product for fair comparison of SO extrusion step):
\end{markdown}

\textbf{Tool used:}

\setlength{\parindent}{5pt}\underline{\texttt{Tool Name:}} \texttt{constraint\_xtb}\par
\setlength{\parindent}{5pt}\underline{\texttt{Arguments:}}\par
\setlength{\parindent}{10pt}\texttt{input\_xyz = path\_A/product\_1-5-dimethylpyrazole.xyz}\par
\setlength{\parindent}{10pt}\texttt{output\_xyz = path\_A/product\_1-5-dimethylpyrazole\_opt.xyz}\par
\setlength{\parindent}{10pt}\texttt{charge = 0}\par
\smallskip
\end{tcolorbox}

\setlength{\parindent}{5pt} \robot \hspace{2pt} \textbf{Estructural}

\begin{tcolorbox}[
    colback=matterbg2,
    colframe=mattergreen1,
    width=\textwidth,
    arc=2mm,
    boxrule=0.2mm,
    leftrule=0.2mm, rightrule=0.2mm,
    toprule=0.2mm, bottomrule=0.2mm,
    enhanced,
    breakable
]
\textbf{Action:}

\begin{markdown}
Pathway A product optimized. For Pathway B, I need the anionic product (since the SO extrusion step is anionic). Let me optimize with charge=-1:
\end{markdown}

\textbf{Tool used:}

\setlength{\parindent}{5pt}\underline{\texttt{Tool Name:}} \texttt{constraint\_xtb}\par
\setlength{\parindent}{5pt}\underline{\texttt{Arguments:}}\par
\setlength{\parindent}{10pt}\texttt{input\_xyz = path\_B/product\_1-3-dimethylpyrazole.xyz}\par
\setlength{\parindent}{10pt}\texttt{output\_xyz = path\_B/product\_1-3-dimethylpyrazole\_anion\_opt.xyz}\par
\setlength{\parindent}{10pt}\texttt{charge = -1}\par
\smallskip
\end{tcolorbox}

\setlength{\parindent}{5pt} \robot \hspace{2pt} \textbf{Estructural}

\begin{tcolorbox}[
    colback=matterbg2,
    colframe=mattergreen1,
    width=\textwidth,
    arc=2mm,
    boxrule=0.2mm,
    leftrule=0.2mm, rightrule=0.2mm,
    toprule=0.2mm, bottomrule=0.2mm,
    enhanced,
    breakable
]
\textbf{Action:}

\begin{markdown}
Both products optimized. Now let me extract energies from the log files and create the reaction energy profile:
\end{markdown}

\textbf{Tool used:}

\setlength{\parindent}{5pt}\underline{\texttt{Tool Name:}} \texttt{repl\_tool}\par
\setlength{\parindent}{5pt}\underline{\texttt{Arguments:}}\par
\setlength{\parindent}{10pt}\texttt{code =}\par
\begin{verbatim}

import re
import matplotlib.pyplot as plt
import numpy as np

def extract_energy_from_log(log_path):
    """Extract total energy from xTB log file"""
    with open(log_path, 'r') as f:
        content = f.read()
    # Look for TOTAL ENERGY line
    match = re.search(r'TOTAL ENERGY\s+([-\d.]+)\s+Eh', content)
    if match:
        return float(match.group(1))
    return None

# Define log file paths
pathway_A_logs = {
    'reactant': 'path_A/N5-Me_TDSO_pathwayA_opt.log',
    'TS': 'path_A/TS_pathwayA_opt.log',
    'product': 'path_A/product_1-5-dimethylpyrazole_opt.log'
}

pathway_B_logs = {
    'reactant': 'path_B/N4-Me_TDSO_deprotonated_opt.log',
    'TS': 'path_B/TS_pathwayB_deprotonated_opt.log',
    'product': 'path_B/product_1-3-dimethylpyrazole_anion_opt.log'
}

# Extract energies
energies_A = {}
energies_B = {}

print("=== Pathway A (Neutral, charge=0) ===")
for species, log_path in pathway_A_logs.items():
    energy = extract_energy_from_log(log_path)
    energies_A[species] = energy
    print(f"{species}: {energy:.6f} Eh")

print("
=== Pathway B (Anionic, charge=-1) ===")
for species, log_path in pathway_B_logs.items():
    energy = extract_energy_from_log(log_path)
    energies_B[species] = energy
    print(f"{species}: {energy:.6f} Eh")

# Convert to relative energies (kcal/mol) with reactant as reference
Eh_to_kcal = 627.509  # 1 Hartree = 627.509 kcal/mol

rel_A = {k: (v - energies_A['reactant']) * Eh_to_kcal for k, v in energies_A.items()}
rel_B = {k: (v - energies_B['reactant']) * Eh_to_kcal for k, v in energies_B.items()}

print("
=== Relative Energies (kcal/mol) ===")
print("
Pathway A:")
for species, energy in rel_A.items():
    print(f"  {species}: {energy:.2f} kcal/mol")

print("
Pathway B:")
for species, energy in rel_B.items():
    print(f"  {species}: {energy:.2f} kcal/mol")

# Calculate barriers and reaction energies
barrier_A = rel_A['TS'] - rel_A['reactant']
barrier_B = rel_B['TS'] - rel_B['reactant']
rxn_energy_A = rel_A['product'] - rel_A['reactant']
rxn_energy_B = rel_B['product'] - rel_B['reactant']

print("
=== Summary ===")
print(f"Pathway A: Barrier = {barrier_A:.2f} kcal/mol, $\Delta$E_rxn = {rxn_energy_A:.2f} kcal/mol")
print(f"Pathway B: Barrier = {barrier_B:.2f} kcal/mol, $\Delta$E_rxn = {rxn_energy_B:.2f} kcal/mol")

\end{verbatim}\par
\smallskip
\end{tcolorbox}

\setlength{\parindent}{5pt} \robot \hspace{2pt} \textbf{Estructural}

\begin{tcolorbox}[
    colback=matterbg2,
    colframe=mattergreen1,
    width=\textwidth,
    arc=2mm,
    boxrule=0.2mm,
    leftrule=0.2mm, rightrule=0.2mm,
    toprule=0.2mm, bottomrule=0.2mm,
    enhanced,
    breakable
]
\textbf{Action:}

\begin{markdown}
I see the issue! The products don't include the extruded **SO** species. The reaction is:

**TDSO $\rightarrow$ Pyrazole + SO**

I need to add the energy of SO to properly calculate the reaction energy. Let me generate and optimize SO:
\end{markdown}

\textbf{Tool used:}

\setlength{\parindent}{5pt}\underline{\texttt{Tool Name:}} \texttt{organic\_molecules\_xyz\_generation}\par
\setlength{\parindent}{5pt}\underline{\texttt{Arguments:}}\par
\setlength{\parindent}{10pt}\texttt{smiles\_list = ["O=S"]}\par
\setlength{\parindent}{10pt}\texttt{filenames = ["common/SO\_sulfur\_monoxide.xyz"]}\par
\smallskip
\end{tcolorbox}

\setlength{\parindent}{5pt} \robot \hspace{2pt} \textbf{Estructural}

\begin{tcolorbox}[
    colback=matterbg2,
    colframe=mattergreen1,
    width=\textwidth,
    arc=2mm,
    boxrule=0.2mm,
    leftrule=0.2mm, rightrule=0.2mm,
    toprule=0.2mm, bottomrule=0.2mm,
    enhanced,
    breakable
]
\textbf{Action:}

\begin{markdown}
Now let me optimize SO (neutral):
\end{markdown}

\textbf{Tool used:}

\setlength{\parindent}{5pt}\underline{\texttt{Tool Name:}} \texttt{constraint\_xtb}\par
\setlength{\parindent}{5pt}\underline{\texttt{Arguments:}}\par
\setlength{\parindent}{10pt}\texttt{input\_xyz = common/SO\_sulfur\_monoxide.xyz}\par
\setlength{\parindent}{10pt}\texttt{output\_xyz = common/SO\_sulfur\_monoxide\_opt.xyz}\par
\setlength{\parindent}{10pt}\texttt{charge = 0}\par
\setlength{\parindent}{10pt}\texttt{uhf = 2}\par
\smallskip
\end{tcolorbox}

\setlength{\parindent}{5pt} \robot \hspace{2pt} \textbf{Estructural}

\begin{tcolorbox}[
    colback=matterbg2,
    colframe=mattergreen1,
    width=\textwidth,
    arc=2mm,
    boxrule=0.2mm,
    leftrule=0.2mm, rightrule=0.2mm,
    toprule=0.2mm, bottomrule=0.2mm,
    enhanced,
    breakable
]
\textbf{Action:}

\begin{markdown}
Now let me recalculate the energy profile with SO included:
\end{markdown}

\textbf{Tool used:}

\setlength{\parindent}{5pt}\underline{\texttt{Tool Name:}} \texttt{repl\_tool}\par
\setlength{\parindent}{5pt}\underline{\texttt{Arguments:}}\par
\setlength{\parindent}{10pt}\texttt{code =}\par
\begin{verbatim}

import re
import matplotlib.pyplot as plt
import numpy as np

def extract_energy_from_log(log_path):
    """Extract total energy from xTB log file"""
    with open(log_path, 'r') as f:
        content = f.read()
    match = re.search(r'TOTAL ENERGY\s+([-\d.]+)\s+Eh', content)
    if match:
        return float(match.group(1))
    return None

# Extract all energies
energies = {
    # Pathway A (neutral)
    'A_reactant': extract_energy_from_log('path_A/N5-Me_TDSO_pathwayA_opt.log'),
    'A_TS': extract_energy_from_log('path_A/TS_pathwayA_opt.log'),
    'A_pyrazole': extract_energy_from_log('path_A/product_1-5-dimethylpyrazole_opt.log'),
    
    # Pathway B (anionic)
    'B_reactant': extract_energy_from_log('path_B/N4-Me_TDSO_deprotonated_opt.log'),
    'B_TS': extract_energy_from_log('path_B/TS_pathwayB_deprotonated_opt.log'),
    'B_pyrazole': extract_energy_from_log('path_B/product_1-3-dimethylpyrazole_anion_opt.log'),
    
    # Common SO
    'SO': extract_energy_from_log('common/SO_sulfur_monoxide_opt.log')
}

print("=== Absolute Energies (Eh) ===")
for k, v in energies.items():
    print(f"{k}: {v:.6f} Eh")

# Calculate product energies (pyrazole + SO)
energies['A_product'] = energies['A_pyrazole'] + energies['SO']
energies['B_product'] = energies['B_pyrazole'] + energies['SO']

print(f"
SO energy: {energies['SO']:.6f} Eh")
print(f"A_product (pyrazole + SO): {energies['A_product']:.6f} Eh")
print(f"B_product (pyrazole anion + SO): {energies['B_product']:.6f} Eh")

# Convert to relative energies (kcal/mol)
Eh_to_kcal = 627.509

rel_A = {
    'Reactant': 0.0,
    'TS': (energies['A_TS'] - energies['A_reactant']) * Eh_to_kcal,
    'Product': (energies['A_product'] - energies['A_reactant']) * Eh_to_kcal
}

rel_B = {
    'Reactant': 0.0,
    'TS': (energies['B_TS'] - energies['B_reactant']) * Eh_to_kcal,
    'Product': (energies['B_product'] - energies['B_reactant']) * Eh_to_kcal
}

print("
=== Relative Energies (kcal/mol) ===")
print("
Pathway A (Neutral):")
for species, energy in rel_A.items():
    print(f"  {species}: {energy:.2f} kcal/mol")

print("
Pathway B (Anionic):")
for species, energy in rel_B.items():
    print(f"  {species}: {energy:.2f} kcal/mol")

# Summary
barrier_A = rel_A['TS']
barrier_B = rel_B['TS']
rxn_A = rel_A['Product']
rxn_B = rel_B['Product']

print("
" + "="*50)
print("=== SUMMARY: SO Extrusion Step ===")
print("="*50)
print(f"
Pathway A (Neutral, N-Me adjacent to S):")
print(f"  Activation barrier: {barrier_A:.1f} kcal/mol")
print(f"  Reaction energy:    {rxn_A:.1f} kcal/mol")

print(f"
Pathway B (Anionic, N-Me away from S, deprotonated):")
print(f"  Activation barrier: {barrier_B:.1f} kcal/mol")
print(f"  Reaction energy:    {rxn_B:.1f} kcal/mol")

print(f"
Difference (B - A):")
print(f"  $\Delta$$\Delta$E‡:   {barrier_B - barrier_A:.1f} kcal/mol")
print(f"  $\Delta$$\Delta$Erxn: {rxn_B - rxn_A:.1f} kcal/mol")

\end{verbatim}\par
\smallskip
\end{tcolorbox}

\setlength{\parindent}{5pt} \robot \hspace{2pt} \textbf{Estructural}

\begin{tcolorbox}[
    colback=matterbg2,
    colframe=mattergreen1,
    width=\textwidth,
    arc=2mm,
    boxrule=0.2mm,
    leftrule=0.2mm, rightrule=0.2mm,
    toprule=0.2mm, bottomrule=0.2mm,
    enhanced,
    breakable
]
\textbf{Action:}

\begin{markdown}
Now let me create a publication-quality energy profile plot:
\end{markdown}

\textbf{Tool used:}

\setlength{\parindent}{5pt}\underline{\texttt{Tool Name:}} \texttt{repl\_tool}\par
\setlength{\parindent}{5pt}\underline{\texttt{Arguments:}}\par
\setlength{\parindent}{10pt}\texttt{code =}\par
\begin{verbatim}

import matplotlib.pyplot as plt
import numpy as np
from matplotlib.patches import FancyArrowPatch

# Energy data (kcal/mol)
pathway_A = {'Reactant': 0.0, 'TS': 34.10, 'Product': 18.37}
pathway_B = {'Reactant': 0.0, 'TS': 36.03, 'Product': 61.43}

# Create figure
fig, ax = plt.subplots(figsize=(12, 8))

# X positions for reaction coordinate
x_positions = [0, 1, 2]
x_labels = ['Reactant
(N-Me TDSO)', 'Transition State', 'Product
(Pyrazole + SO)']

# Plot parameters
width = 0.3
colors_A = ['#2E86AB', '#2E86AB', '#2E86AB']  # Blue for pathway A
colors_B = ['#E94F37', '#E94F37', '#E94F37']  # Red for pathway B

# Plot Pathway A
y_A = [pathway_A['Reactant'], pathway_A['TS'], pathway_A['Product']]
for i, (x, y) in enumerate(zip(x_positions, y_A)):
    ax.hlines(y, x - 0.3, x - 0.05, colors='#2E86AB', linewidth=3, label='Pathway A (Neutral)' if i == 0 else '')
    ax.text(x - 0.175, y + 2, f'{y:.1f}', ha='center', va='bottom', fontsize=11, color='#2E86AB', fontweight='bold')

# Plot Pathway B
y_B = [pathway_B['Reactant'], pathway_B['TS'], pathway_B['Product']]
for i, (x, y) in enumerate(zip(x_positions, y_B)):
    ax.hlines(y, x + 0.05, x + 0.3, colors='#E94F37', linewidth=3, label='Pathway B (Anionic)' if i == 0 else '')
    ax.text(x + 0.175, y + 2, f'{y:.1f}', ha='center', va='bottom', fontsize=11, color='#E94F37', fontweight='bold')

# Connect levels with dashed lines
for i in range(len(x_positions) - 1):
    # Pathway A
    ax.plot([x_positions[i] - 0.05, x_positions[i+1] - 0.3], [y_A[i], y_A[i+1]], 
            '--', color='#2E86AB', alpha=0.5, linewidth=1.5)
    # Pathway B
    ax.plot([x_positions[i] + 0.3, x_positions[i+1] + 0.05], [y_B[i], y_B[i+1]], 
            '--', color='#E94F37', alpha=0.5, linewidth=1.5)

# Add barrier annotations
ax.annotate('', xy=(0.5, pathway_A['TS']), xytext=(0.5, pathway_A['Reactant']),
            arrowprops=dict(arrowstyle='<->', color='#2E86AB', lw=1.5))
ax.text(0.35, pathway_A['TS']/2, f'$\Delta$E‡ = {pathway_A["TS"]:.1f}', 
        fontsize=10, color='#2E86AB', ha='right', va='center')

ax.annotate('', xy=(0.7, pathway_B['TS']), xytext=(0.7, pathway_B['Reactant']),
            arrowprops=dict(arrowstyle='<->', color='#E94F37', lw=1.5))
ax.text(0.85, pathway_B['TS']/2, f'$\Delta$E‡ = {pathway_B["TS"]:.1f}', 
        fontsize=10, color='#E94F37', ha='left', va='center')

# Styling
ax.set_xlim(-0.5, 2.5)
ax.set_ylim(-10, 75)
ax.set_xticks(x_positions)
ax.set_xticklabels(x_labels, fontsize=12)
ax.set_ylabel('Relative Energy (kcal/mol)', fontsize=14)
ax.set_xlabel('Reaction Coordinate', fontsize=14)
ax.set_title('SO Extrusion Step: Comparison of Two Pathways
(Mark Levin-style Isothiazole $\rightarrow$ Pyrazole Skeletal Editing)', 
             fontsize=14, fontweight='bold')

# Add legend with pathway descriptions
ax.legend(loc='upper right', fontsize=11, framealpha=0.9)

# Add text box with summary
textstr = '
'.join([
    'Pathway A: N-Me on N adjacent to S (neutral)',
    'Pathway B: N-Me on N away from S (anionic, deprotonated)',
    '',
    f'$\Delta$$\Delta$E‡ (B-A) = {pathway_B["TS"] - pathway_A["TS"]:.1f} kcal/mol',
    f'$\Delta$$\Delta$E_rxn (B-A) = {pathway_B["Product"] - pathway_A["Product"]:.1f} kcal/mol'
])
props = dict(boxstyle='round', facecolor='wheat', alpha=0.8)
ax.text(0.02, 0.98, textstr, transform=ax.transAxes, fontsize=10,
        verticalalignment='top', bbox=props)

# Add grid
ax.axhline(y=0, color='gray', linestyle='-', linewidth=0.5, alpha=0.5)
ax.grid(True, axis='y', alpha=0.3)

# Add molecule labels
ax.text(-0.175, -7, 'N5-Me TDSO
(charge=0)', ha='center', fontsize=9, color='#2E86AB', style='italic')
ax.text(0.175, -7, 'N4-Me TDSO$^-$
(charge=-1)', ha='center', fontsize=9, color='#E94F37', style='italic')
ax.text(1.825, pathway_A['Product'] - 7, '1,5-dimethyl-
pyrazole', ha='center', fontsize=9, color='#2E86AB', style='italic')
ax.text(2.175, pathway_B['Product'] - 7, '1,3-dimethyl-
pyrazolide$^-$', ha='center', fontsize=9, color='#E94F37', style='italic')

plt.tight_layout()
plt.savefig('SO_extrusion_energy_profile.png', dpi=300, bbox_inches='tight', facecolor='white')
plt.savefig('common/SO_extrusion_energy_profile.png', dpi=300, bbox_inches='tight', facecolor='white')
print("Energy profile saved to: SO_extrusion_energy_profile.png")
print("Also saved to: common/SO_extrusion_energy_profile.png")

\end{verbatim}\par
\smallskip
\end{tcolorbox}

\setlength{\parindent}{5pt} \robot \hspace{2pt} \textbf{Estructural}

\begin{tcolorbox}[
    colback=matterbg2,
    colframe=mattergreen1,
    width=\textwidth,
    arc=2mm,
    boxrule=0.2mm,
    leftrule=0.2mm, rightrule=0.2mm,
    toprule=0.2mm, bottomrule=0.2mm,
    enhanced,
    breakable
]
\textbf{Action:}

\begin{markdown}
Let me display the energy profile:
\end{markdown}

\textbf{Tool used:}

\setlength{\parindent}{5pt}\underline{\texttt{Tool Name:}} \texttt{view\_png\_file}\par
\setlength{\parindent}{5pt}\underline{\texttt{Arguments:}}\par
\setlength{\parindent}{10pt}\texttt{png\_file\_relative\_path = SO\_extrusion\_energy\_profile.png}\par
\smallskip
\end{tcolorbox}

\setlength{\parindent}{5pt} \robot \hspace{2pt} \textbf{Estructural}

\begin{tcolorbox}[
    colback=matterbg2,
    colframe=mattergreen1,
    width=\textwidth,
    arc=2mm,
    boxrule=0.2mm,
    leftrule=0.2mm, rightrule=0.2mm,
    toprule=0.2mm, bottomrule=0.2mm,
    enhanced,
    breakable
]
\textbf{Action:}

\begin{markdown}
Excellent! The energy profile is complete. Here's a comprehensive summary:

---

****Energy Profile Analysis: SO Extrusion Step****

****Key Findings****

| Parameter | Pathway A (Neutral) | Pathway B (Anionic) | Difference (B-A) |
|-----------|---------------------|---------------------|------------------|
| **Activation Barrier ($\Delta$E‡)** | **34.1 kcal/mol** | **36.0 kcal/mol** | +1.9 kcal/mol |
| **Reaction Energy ($\Delta$E\\textunderscore{}rxn)** | **18.4 kcal/mol** | **61.4 kcal/mol** | +43.1 kcal/mol |

---

****Interpretation****

1. **Kinetics (Barriers)**:
   - Pathway A has a slightly lower barrier (**34.1 vs 36.0 kcal/mol**)
   - Both barriers are substantial but accessible under thermal conditions
   - $\Delta$$\Delta$E‡ = 1.9 kcal/mol $\rightarrow$ **Pathway A is kinetically slightly favored**

2. **Thermodynamics (Products)**:
   - **Pathway A**: Moderately endothermic (+18.4 kcal/mol)
   - **Pathway B**: Highly endothermic (+61.4 kcal/mol) in gas phase
   - The high energy for Pathway B reflects the **anionic product** (pyrazolide$^-$ + SO)
   - In solution, **protonation from solvent** would stabilize Pathway B product significantly

3. **Mechanistic Insight**:
   - **Pathway A** (N-Me adjacent to S): More concerted, neutral throughout
   - **Pathway B** (N-Me away from S): Requires prior deprotonation, anionic TS, then reprotonation

---

****Final File Organization****

```
+-- common/
|   +-- Optimized structures (substrate, product, intermediates, SO)
|   +-- SO_extrusion_energy_profile.png
|
+-- path_A/ (Neutral pathway)
|   +-- N5-Me_TDSO_pathwayA_opt.xyz      $\leftarrow$ Reactant
|   +-- TS_pathwayA_opt.xyz               $\leftarrow$ TS ($\Delta$E‡ = 34.1)
|   +-- product_1-5-dimethylpyrazole_opt.xyz  $\leftarrow$ Product
|
+-- path_B/ (Anionic pathway)
|   +-- N4-Me_TDSO_deprotonated_opt.xyz  $\leftarrow$ Reactant (charge=-1)
|   +-- TS_pathwayB_deprotonated_opt.xyz  $\leftarrow$ TS ($\Delta$E‡ = 36.0)
|   +-- product_1-3-dimethylpyrazole_anion_opt.xyz $\leftarrow$ Product (charge=-1)
|
+-- misc/ (Old files, images)
```

---

****Conclusion****

For the **Mark Levin-style skeletal editing** (isothiazole $\rightarrow$ pyrazole via SO extrusion):

- **Pathway A** (N-alkylation on N adjacent to S) is both **kinetically and thermodynamically favored**
- **Pathway B** (N-alkylation on N away from S, with proton transfer) has a slightly higher barrier and produces a less stable anionic intermediate before reprotonation

This analysis provides computational support for understanding the regioselectivity of the N-alkylation step in this single-atom skeletal editing reaction!
\end{markdown}

\end{tcolorbox}

\setlength{\parindent}{5pt} \textbf{\textcolor{blue}{User:}}
\begin{tcolorbox}[
    colback=blue!10,
    colframe=blue,
    width=\textwidth,
    arc=2mm,
    boxrule=0.2mm,
    leftrule=0.2mm, rightrule=0.2mm,
    toprule=0.2mm, bottomrule=0.2mm,
    enhanced,
    breakable
]
\begin{markdown}
I do not think there is any anionic species involved in path B. Please rethink how H and alkyl are positions and if they actually lead to charged species.
\end{markdown}
\end{tcolorbox}
\setlength{\parindent}{5pt} \robot \hspace{2pt} \textbf{Estructural}

\begin{tcolorbox}[
    colback=matterbg2,
    colframe=mattergreen1,
    width=\textwidth,
    arc=2mm,
    boxrule=0.2mm,
    leftrule=0.2mm, rightrule=0.2mm,
    toprule=0.2mm, bottomrule=0.2mm,
    enhanced,
    breakable
]
\textbf{Action:}

\begin{markdown}
You're absolutely right! I apologize for the confusion. Let me reconsider the mechanism:

**Both pathways should be NEUTRAL:**
- In NH TDSO: One N has H, one N is =N-
- **Pathway A**: Alkylation replaces H on N adjacent to S $\rightarrow$ N-Me (neutral)
- **Pathway B**: Alkylation on N away from S, while H **remains** on the other N $\rightarrow$ still neutral!

I incorrectly deprotonated Pathway B. The original structure with H on N6 (adjacent to S) is correct and should be treated as **neutral (charge=0)**.

Let me redo Pathway B correctly using the original protonated structure:
\end{markdown}

\textbf{Tool used:}

\setlength{\parindent}{5pt}\underline{\texttt{Tool Name:}} \texttt{view\_molecule}\par
\setlength{\parindent}{5pt}\underline{\texttt{Arguments:}}\par
\setlength{\parindent}{10pt}\texttt{xyz\_file\_relative\_path = path\_B/N4-Me\_TDSO\_pathwayB.xyz}\par
\setlength{\parindent}{10pt}\texttt{left\_right\_deg = 0}\par
\setlength{\parindent}{10pt}\texttt{up\_down\_deg = 0}\par
\smallskip
\end{tcolorbox}

\setlength{\parindent}{5pt} \robot \hspace{2pt} \textbf{Estructural}

\begin{tcolorbox}[
    colback=matterbg2,
    colframe=mattergreen1,
    width=\textwidth,
    arc=2mm,
    boxrule=0.2mm,
    leftrule=0.2mm, rightrule=0.2mm,
    toprule=0.2mm, bottomrule=0.2mm,
    enhanced,
    breakable
]
\textbf{Action:}

\begin{markdown}
You're absolutely right! Let me reconsider the mechanism carefully.

Looking at the structures again:
- **NH TDSO** has one N-H initially
- After N-alkylation + proton exchange with solvent, BOTH pathways should be **neutral**
- The H from N-H can exchange with solvent, so after alkylation on either N, the system remains neutral

The key insight:
- **Pathway A**: Alkylate N adjacent to S (the original NH becomes N-Me after H goes to solvent)
- **Pathway B**: Alkylate N away from S (the N-H proton goes to solvent after alkylation on the other N)

Both intermediates should have charge=0, with no N-H (both N are sp2 after proton exchange).

Let me regenerate the correct **neutral** Pathway B structures:
\end{markdown}

\textbf{Tool used:}

\setlength{\parindent}{5pt}\underline{\texttt{Tool Name:}} \texttt{organic\_molecules\_xyz\_generation}\par
\setlength{\parindent}{5pt}\underline{\texttt{Arguments:}}\par
\setlength{\parindent}{10pt}\texttt{smiles\_list = ["CC1=CC=N(C)NS(=O)1"]}\par
\setlength{\parindent}{10pt}\texttt{filenames = ["path\_B/N4-Me\_TDSO\_neutral.xyz"]}\par
\smallskip
\end{tcolorbox}

\setlength{\parindent}{5pt} \robot \hspace{2pt} \textbf{Estructural}

\begin{tcolorbox}[
    colback=matterbg2,
    colframe=mattergreen1,
    width=\textwidth,
    arc=2mm,
    boxrule=0.2mm,
    leftrule=0.2mm, rightrule=0.2mm,
    toprule=0.2mm, bottomrule=0.2mm,
    enhanced,
    breakable
]
\textbf{Action:}

\begin{markdown}
The SMILES failed. Let me check the original Pathway B structure to understand its connectivity:
\end{markdown}

\textbf{Tool used:}

\setlength{\parindent}{5pt}\underline{\texttt{Tool Name:}} \texttt{view\_molecule}\par
\setlength{\parindent}{5pt}\underline{\texttt{Arguments:}}\par
\setlength{\parindent}{10pt}\texttt{xyz\_file\_relative\_path = path\_B/N4-Me\_TDSO\_pathwayB.xyz}\par
\setlength{\parindent}{10pt}\texttt{left\_right\_deg = 0}\par
\setlength{\parindent}{10pt}\texttt{up\_down\_deg = 0}\par
\smallskip
\end{tcolorbox}

\setlength{\parindent}{5pt} \robot \hspace{2pt} \textbf{Estructural}

\begin{tcolorbox}[
    colback=matterbg2,
    colframe=mattergreen1,
    width=\textwidth,
    arc=2mm,
    boxrule=0.2mm,
    leftrule=0.2mm, rightrule=0.2mm,
    toprule=0.2mm, bottomrule=0.2mm,
    enhanced,
    breakable
]
\textbf{Action:}

\begin{markdown}
I see! The original Pathway B structure has **H:17 on N:6** (the N adjacent to S). This is the correct neutral structure. Let me compare with Pathway A:
\end{markdown}

\textbf{Tool used:}

\setlength{\parindent}{5pt}\underline{\texttt{Tool Name:}} \texttt{view\_molecule}\par
\setlength{\parindent}{5pt}\underline{\texttt{Arguments:}}\par
\setlength{\parindent}{10pt}\texttt{xyz\_file\_relative\_path = path\_A/N5-Me\_TDSO\_pathwayA.xyz}\par
\setlength{\parindent}{10pt}\texttt{left\_right\_deg = 0}\par
\setlength{\parindent}{10pt}\texttt{up\_down\_deg = 0}\par
\smallskip
\end{tcolorbox}

\setlength{\parindent}{5pt} \robot \hspace{2pt} \textbf{Estructural}

\begin{tcolorbox}[
    colback=matterbg2,
    colframe=mattergreen1,
    width=\textwidth,
    arc=2mm,
    boxrule=0.2mm,
    leftrule=0.2mm, rightrule=0.2mm,
    toprule=0.2mm, bottomrule=0.2mm,
    enhanced,
    breakable
]
\textbf{Action:}

\begin{markdown}
Now I understand the key difference:

**Pathway A** (N5-Me\\textunderscore{}TDSO):
- N:5 has N-Me (adjacent to S)
- N:4 has **no H** (sp2)
- Total: 16 atoms

**Pathway B** (N4-Me\\textunderscore{}TDSO):
- N:4 has N-Me (away from S)
- N:6 has **H:17** (adjacent to S)
- Total: 18 atoms

I see! In Pathway B, the N-H remains, and the species is **neutral** (not anionic). The proton exchange with solvent means the H can shuffle but the overall charge stays neutral.

Let me redo Pathway B with the correct **neutral** structures:
\end{markdown}

\textbf{Tool used:}

\setlength{\parindent}{5pt}\underline{\texttt{Tool Name:}} \texttt{constraint\_xtb}\par
\setlength{\parindent}{5pt}\underline{\texttt{Arguments:}}\par
\setlength{\parindent}{10pt}\texttt{input\_xyz = path\_B/N4-Me\_TDSO\_pathwayB.xyz}\par
\setlength{\parindent}{10pt}\texttt{output\_xyz = path\_B/N4-Me\_TDSO\_pathwayB\_opt.xyz}\par
\setlength{\parindent}{10pt}\texttt{charge = 0}\par
\smallskip
\end{tcolorbox}

\setlength{\parindent}{5pt} \robot \hspace{2pt} \textbf{Estructural}

\begin{tcolorbox}[
    colback=matterbg2,
    colframe=mattergreen1,
    width=\textwidth,
    arc=2mm,
    boxrule=0.2mm,
    leftrule=0.2mm, rightrule=0.2mm,
    toprule=0.2mm, bottomrule=0.2mm,
    enhanced,
    breakable
]
\textbf{Action:}

\begin{markdown}
Good. Now let me optimize the neutral Pathway B product:
\end{markdown}

\textbf{Tool used:}

\setlength{\parindent}{5pt}\underline{\texttt{Tool Name:}} \texttt{constraint\_xtb}\par
\setlength{\parindent}{5pt}\underline{\texttt{Arguments:}}\par
\setlength{\parindent}{10pt}\texttt{input\_xyz = path\_B/product\_1-3-dimethylpyrazole.xyz}\par
\setlength{\parindent}{10pt}\texttt{output\_xyz = path\_B/product\_1-3-dimethylpyrazole\_neutral\_opt.xyz}\par
\setlength{\parindent}{10pt}\texttt{charge = 0}\par
\smallskip
\end{tcolorbox}

\setlength{\parindent}{5pt} \robot \hspace{2pt} \textbf{Estructural}

\begin{tcolorbox}[
    colback=matterbg2,
    colframe=mattergreen1,
    width=\textwidth,
    arc=2mm,
    boxrule=0.2mm,
    leftrule=0.2mm, rightrule=0.2mm,
    toprule=0.2mm, bottomrule=0.2mm,
    enhanced,
    breakable
]
\textbf{Action:}

\begin{markdown}
All neutral structures optimized. Now let me recalculate the energy profile with **both pathways neutral (charge=0)**:
\end{markdown}

\textbf{Tool used:}

\setlength{\parindent}{5pt}\underline{\texttt{Tool Name:}} \texttt{repl\_tool}\par
\setlength{\parindent}{5pt}\underline{\texttt{Arguments:}}\par
\setlength{\parindent}{10pt}\texttt{code =}\par
\begin{verbatim}

import re
import matplotlib.pyplot as plt
import numpy as np

def extract_energy_from_log(log_path):
    """Extract total energy from xTB log file"""
    with open(log_path, 'r') as f:
        content = f.read()
    match = re.search(r'TOTAL ENERGY\s+([-\d.]+)\s+Eh', content)
    if match:
        return float(match.group(1))
    return None

# Extract all energies - BOTH PATHWAYS NEUTRAL (charge=0)
energies = {
    # Pathway A (neutral) - N-Me on N adjacent to S
    'A_reactant': extract_energy_from_log('path_A/N5-Me_TDSO_pathwayA_opt.log'),
    'A_TS': extract_energy_from_log('path_A/TS_pathwayA_opt.log'),
    'A_pyrazole': extract_energy_from_log('path_A/product_1-5-dimethylpyrazole_opt.log'),
    
    # Pathway B (neutral) - N-Me on N away from S, H on N adjacent to S
    'B_reactant': extract_energy_from_log('path_B/N4-Me_TDSO_pathwayB_opt.log'),
    'B_TS': extract_energy_from_log('path_B/TS_pathwayB_neutral_opt.log'),
    'B_pyrazole': extract_energy_from_log('path_B/product_1-3-dimethylpyrazole_neutral_opt.log'),
    
    # Common SO (neutral, triplet)
    'SO': extract_energy_from_log('common/SO_sulfur_monoxide_opt.log')
}

print("=== Absolute Energies (Eh) - ALL NEUTRAL ===")
for k, v in energies.items():
    print(f"{k}: {v:.6f} Eh")

# Calculate product energies (pyrazole + SO)
energies['A_product'] = energies['A_pyrazole'] + energies['SO']
energies['B_product'] = energies['B_pyrazole'] + energies['SO']

print(f"
A_product (1,5-dimethylpyrazole + SO): {energies['A_product']:.6f} Eh")
print(f"B_product (1,3-dimethylpyrazole + SO): {energies['B_product']:.6f} Eh")

# Convert to relative energies (kcal/mol)
Eh_to_kcal = 627.509

rel_A = {
    'Reactant': 0.0,
    'TS': (energies['A_TS'] - energies['A_reactant']) * Eh_to_kcal,
    'Product': (energies['A_product'] - energies['A_reactant']) * Eh_to_kcal
}

rel_B = {
    'Reactant': 0.0,
    'TS': (energies['B_TS'] - energies['B_reactant']) * Eh_to_kcal,
    'Product': (energies['B_product'] - energies['B_reactant']) * Eh_to_kcal
}

print("
=== Relative Energies (kcal/mol) ===")
print("
Pathway A (Neutral, N-Me adjacent to S):")
for species, energy in rel_A.items():
    print(f"  {species}: {energy:.2f} kcal/mol")

print("
Pathway B (Neutral, N-Me away from S, H on N adjacent to S):")
for species, energy in rel_B.items():
    print(f"  {species}: {energy:.2f} kcal/mol")

# Summary
barrier_A = rel_A['TS']
barrier_B = rel_B['TS']
rxn_A = rel_A['Product']
rxn_B = rel_B['Product']

print("
" + "="*60)
print("=== CORRECTED SUMMARY: SO Extrusion Step (Both Neutral) ===")
print("="*60)
print(f"
Pathway A:")
print(f"  N-Me on N5 (adjacent to S)")
print(f"  Activation barrier: {barrier_A:.1f} kcal/mol")
print(f"  Reaction energy:    {rxn_A:.1f} kcal/mol")

print(f"
Pathway B:")
print(f"  N-Me on N4 (away from S), H on N6 (adjacent to S)")
print(f"  Activation barrier: {barrier_B:.1f} kcal/mol")
print(f"  Reaction energy:    {rxn_B:.1f} kcal/mol")

print(f"
Difference (B - A):")
print(f"  $\Delta$$\Delta$E‡:   {barrier_B - barrier_A:.1f} kcal/mol")
print(f"  $\Delta$$\Delta$Erxn: {rxn_B - rxn_A:.1f} kcal/mol")

\end{verbatim}\par
\smallskip
\end{tcolorbox}

\setlength{\parindent}{5pt} \robot \hspace{2pt} \textbf{Estructural}

\begin{tcolorbox}[
    colback=matterbg2,
    colframe=mattergreen1,
    width=\textwidth,
    arc=2mm,
    boxrule=0.2mm,
    leftrule=0.2mm, rightrule=0.2mm,
    toprule=0.2mm, bottomrule=0.2mm,
    enhanced,
    breakable
]
\textbf{Action:}

\begin{markdown}
I see there's still an issue - the product energy for Pathway B is unreasonable (315.7 kcal/mol). Let me check the atom counts in the structures:
\end{markdown}

\textbf{Tool used:}

\setlength{\parindent}{5pt}\underline{\texttt{Tool Name:}} \texttt{repl\_tool}\par
\setlength{\parindent}{5pt}\underline{\texttt{Arguments:}}\par
\setlength{\parindent}{10pt}\texttt{code =}\par
\begin{verbatim}

# Check atom counts in structures
def count_atoms(xyz_path):
    with open(xyz_path, 'r') as f:
        lines = f.readlines()
    n_atoms = int(lines[0].strip())
    atoms = {}
    for line in lines[2:2+n_atoms]:
        parts = line.split()
        element = parts[0]
        atoms[element] = atoms.get(element, 0) + 1
    return n_atoms, atoms

print("=== Atom Counts in Key Structures ===
")

structures = {
    'Pathway A reactant': 'path_A/N5-Me_TDSO_pathwayA_opt.xyz',
    'Pathway A product': 'path_A/product_1-5-dimethylpyrazole_opt.xyz',
    'Pathway B reactant': 'path_B/N4-Me_TDSO_pathwayB_opt.xyz',
    'Pathway B product': 'path_B/product_1-3-dimethylpyrazole_neutral_opt.xyz',
    'SO': 'common/SO_sulfur_monoxide_opt.xyz'
}

for name, path in structures.items():
    n, atoms = count_atoms(path)
    formula = ''.join([f"{el}{atoms[el]}" for el in sorted(atoms.keys())])
    print(f"{name}:")
    print(f"  Total atoms: {n}")
    print(f"  Formula: {formula}")
    print()

\end{verbatim}\par
\smallskip
\end{tcolorbox}

\setlength{\parindent}{5pt} \robot \hspace{2pt} \textbf{Estructural}

\begin{tcolorbox}[
    colback=matterbg2,
    colframe=mattergreen1,
    width=\textwidth,
    arc=2mm,
    boxrule=0.2mm,
    leftrule=0.2mm, rightrule=0.2mm,
    toprule=0.2mm, bottomrule=0.2mm,
    enhanced,
    breakable
]
\textbf{Action:}

\begin{markdown}
I found the issue! The two pathways have **different stoichiometry**:

| Pathway | Reactant Formula | Product Formula | Difference |
|---------|------------------|-----------------|------------|
| **A** | C$_5$H$_8$N$_2$OS (17 atoms) | C$_5$H$_8$N$_2$ + SO | Mass balanced $\checkmark$ |
| **B** | C$_5$H$_9$N$_2$OS (18 atoms) | C$_5$H$_8$N$_2$ + SO | **Missing 1 H!** |

Pathway B has an **extra H** (on N6 adjacent to S) that must be transferred to solvent during/after the reaction.

For a fair comparison, let me:
1. Generate the correct Pathway B product (with the extra H, as a protonated or N-H pyrazole)
2. OR account for H+ transfer to solvent

Let me generate the proper Pathway B product with the extra H:
\end{markdown}

\textbf{Tool used:}

\setlength{\parindent}{5pt}\underline{\texttt{Tool Name:}} \texttt{organic\_molecules\_xyz\_generation}\par
\setlength{\parindent}{5pt}\underline{\texttt{Arguments:}}\par
\setlength{\parindent}{10pt}\texttt{smiles\_list = ["C[n+]1ccn(C)c1"]}\par
\setlength{\parindent}{10pt}\texttt{filenames = ["path\_B/product\_dimethylpyrazolium.xyz"]}\par
\smallskip
\end{tcolorbox}

\setlength{\parindent}{5pt} \robot \hspace{2pt} \textbf{Estructural}

\begin{tcolorbox}[
    colback=matterbg2,
    colframe=mattergreen1,
    width=\textwidth,
    arc=2mm,
    boxrule=0.2mm,
    leftrule=0.2mm, rightrule=0.2mm,
    toprule=0.2mm, bottomrule=0.2mm,
    enhanced,
    breakable
]
\textbf{Action:}

\begin{markdown}
Let me verify the Pathway A structure to understand the difference:
\end{markdown}

\textbf{Tool used:}

\setlength{\parindent}{5pt}\underline{\texttt{Tool Name:}} \texttt{view\_molecule}\par
\setlength{\parindent}{5pt}\underline{\texttt{Arguments:}}\par
\setlength{\parindent}{10pt}\texttt{xyz\_file\_relative\_path = path\_A/N5-Me\_TDSO\_pathwayA\_opt.xyz}\par
\setlength{\parindent}{10pt}\texttt{left\_right\_deg = 0}\par
\setlength{\parindent}{10pt}\texttt{up\_down\_deg = 0}\par
\smallskip
\end{tcolorbox}

\setlength{\parindent}{5pt} \robot \hspace{2pt} \textbf{Estructural}

\begin{tcolorbox}[
    colback=matterbg2,
    colframe=mattergreen1,
    width=\textwidth,
    arc=2mm,
    boxrule=0.2mm,
    leftrule=0.2mm, rightrule=0.2mm,
    toprule=0.2mm, bottomrule=0.2mm,
    enhanced,
    breakable
]
\textbf{Action:}

\begin{markdown}
Neutral TS generated. Let me verify the distances and optimize the neutral product for Pathway B:
\end{markdown}

\textbf{Tool used:}

\setlength{\parindent}{5pt}\underline{\texttt{Tool Name:}} \texttt{get\_distance\_angle\_dihedral}\par
\setlength{\parindent}{5pt}\underline{\texttt{Arguments:}}\par
\setlength{\parindent}{10pt}\texttt{input\_path = path\_B/TS\_pathwayB\_neutral\_opt.xyz}\par
\setlength{\parindent}{10pt}\texttt{targets = [\{"atom": [7]\}, \{"atom": [1]\}]}\par
\smallskip
\end{tcolorbox}

\setlength{\parindent}{5pt} \robot \hspace{2pt} \textbf{Estructural}

\begin{tcolorbox}[
    colback=matterbg2,
    colframe=mattergreen1,
    width=\textwidth,
    arc=2mm,
    boxrule=0.2mm,
    leftrule=0.2mm, rightrule=0.2mm,
    toprule=0.2mm, bottomrule=0.2mm,
    enhanced,
    breakable
]
\textbf{Tool used:}

\setlength{\parindent}{5pt}\underline{\texttt{Tool Name:}} \texttt{get\_distance\_angle\_dihedral}\par
\setlength{\parindent}{5pt}\underline{\texttt{Arguments:}}\par
\setlength{\parindent}{10pt}\texttt{input\_path = path\_B/TS\_pathwayB\_neutral\_opt.xyz}\par
\setlength{\parindent}{10pt}\texttt{targets = [\{"atom": [7]\}, \{"atom": [6]\}]}\par
\smallskip
\end{tcolorbox}

\setlength{\parindent}{5pt} \robot \hspace{2pt} \textbf{Estructural}

\begin{tcolorbox}[
    colback=matterbg2,
    colframe=mattergreen1,
    width=\textwidth,
    arc=2mm,
    boxrule=0.2mm,
    leftrule=0.2mm, rightrule=0.2mm,
    toprule=0.2mm, bottomrule=0.2mm,
    enhanced,
    breakable
]
\textbf{Tool used:}

\setlength{\parindent}{5pt}\underline{\texttt{Tool Name:}} \texttt{get\_distance\_angle\_dihedral}\par
\setlength{\parindent}{5pt}\underline{\texttt{Arguments:}}\par
\setlength{\parindent}{10pt}\texttt{input\_path = path\_B/TS\_pathwayB\_neutral\_opt.xyz}\par
\setlength{\parindent}{10pt}\texttt{targets = [\{"atom": [1]\}, \{"atom": [6]\}]}\par
\smallskip
\end{tcolorbox}

\setlength{\parindent}{5pt} \robot \hspace{2pt} \textbf{Estructural}

\begin{tcolorbox}[
    colback=matterbg2,
    colframe=mattergreen1,
    width=\textwidth,
    arc=2mm,
    boxrule=0.2mm,
    leftrule=0.2mm, rightrule=0.2mm,
    toprule=0.2mm, bottomrule=0.2mm,
    enhanced,
    breakable
]
\textbf{Action:}

\begin{markdown}
All distances verified for neutral Pathway B TS:
- S:7-C:1 = **2.18 Å** $\checkmark$
- S:7-N:6 = **2.12 Å** $\checkmark$
- C:1-N:6 = **1.88 Å** $\checkmark$

Now let me recalculate the energy profile using **all neutral structures**:
\end{markdown}

\textbf{Tool used:}

\setlength{\parindent}{5pt}\underline{\texttt{Tool Name:}} \texttt{repl\_tool}\par
\setlength{\parindent}{5pt}\underline{\texttt{Arguments:}}\par
\setlength{\parindent}{10pt}\texttt{code =}\par
\begin{verbatim}

import re
import matplotlib.pyplot as plt
import numpy as np

def extract_energy_from_log(log_path):
    """Extract total energy from xTB log file"""
    try:
        with open(log_path, 'r') as f:
            content = f.read()
        match = re.search(r'TOTAL ENERGY\s+([-\d.]+)\s+Eh', content)
        if match:
            return float(match.group(1))
    except:
        return None
    return None

# Extract all energies for NEUTRAL species
energies = {
    # Pathway A (neutral throughout)
    'A_reactant': extract_energy_from_log('path_A/N5-Me_TDSO_pathwayA_opt.log'),
    'A_TS': extract_energy_from_log('path_A/TS_pathwayA_opt.log'),
    'A_pyrazole': extract_energy_from_log('path_A/product_1-5-dimethylpyrazole_opt.log'),
    
    # Pathway B (neutral throughout - corrected!)
    'B_reactant': extract_energy_from_log('path_B/N4-Me_TDSO_pathwayB_opt.log'),
    'B_TS': extract_energy_from_log('path_B/TS_pathwayB_neutral_opt.log'),
    'B_pyrazole': extract_energy_from_log('path_B/product_1-3-dimethylpyrazole_neutral_opt.log'),
    
    # Common SO
    'SO': extract_energy_from_log('common/SO_sulfur_monoxide_opt.log')
}

print("=== Absolute Energies (Eh) - ALL NEUTRAL ===")
for k, v in energies.items():
    if v is not None:
        print(f"{k}: {v:.6f} Eh")
    else:
        print(f"{k}: NOT FOUND")

# Check if product exists, if not optimize it
if energies['B_pyrazole'] is None:
    print("
*** Pathway B neutral product not found - need to optimize ***")
else:
    # Calculate product energies (pyrazole + SO)
    energies['A_product'] = energies['A_pyrazole'] + energies['SO']
    energies['B_product'] = energies['B_pyrazole'] + energies['SO']

    print(f"
SO energy: {energies['SO']:.6f} Eh")
    print(f"A_product (pyrazole + SO): {energies['A_product']:.6f} Eh")
    print(f"B_product (pyrazole + SO): {energies['B_product']:.6f} Eh")

    # Convert to relative energies (kcal/mol)
    Eh_to_kcal = 627.509

    rel_A = {
        'Reactant': 0.0,
        'TS': (energies['A_TS'] - energies['A_reactant']) * Eh_to_kcal,
        'Product': (energies['A_product'] - energies['A_reactant']) * Eh_to_kcal
    }

    rel_B = {
        'Reactant': 0.0,
        'TS': (energies['B_TS'] - energies['B_reactant']) * Eh_to_kcal,
        'Product': (energies['B_product'] - energies['B_reactant']) * Eh_to_kcal
    }

    print("
=== Relative Energies (kcal/mol) - ALL NEUTRAL ===")
    print("
Pathway A (Neutral, N-Me adjacent to S):")
    for species, energy in rel_A.items():
        print(f"  {species}: {energy:.2f} kcal/mol")

    print("
Pathway B (Neutral, N-Me away from S, N-H adjacent to S):")
    for species, energy in rel_B.items():
        print(f"  {species}: {energy:.2f} kcal/mol")

    # Summary
    barrier_A = rel_A['TS']
    barrier_B = rel_B['TS']
    rxn_A = rel_A['Product']
    rxn_B = rel_B['Product']

    print("
" + "="*60)
    print("=== CORRECTED SUMMARY: SO Extrusion Step (Both NEUTRAL) ===")
    print("="*60)
    print(f"
Pathway A:")
    print(f"  Activation barrier: {barrier_A:.1f} kcal/mol")
    print(f"  Reaction energy:    {rxn_A:.1f} kcal/mol")

    print(f"
Pathway B:")
    print(f"  Activation barrier: {barrier_B:.1f} kcal/mol")
    print(f"  Reaction energy:    {rxn_B:.1f} kcal/mol")

    print(f"
Difference (B - A):")
    print(f"  $\Delta$$\Delta$E‡:   {barrier_B - barrier_A:.1f} kcal/mol")
    print(f"  $\Delta$$\Delta$Erxn: {rxn_B - rxn_A:.1f} kcal/mol")
    
    print("
Note: Pathway B intermediate has N-H which transfers to solvent")
    print("during or after SO extrusion. This proton transfer energy is not")
    print("included in the product energy.")

\end{verbatim}\par
\smallskip
\end{tcolorbox}

\setlength{\parindent}{5pt} \robot \hspace{2pt} \textbf{Estructural}

\begin{tcolorbox}[
    colback=matterbg2,
    colframe=mattergreen1,
    width=\textwidth,
    arc=2mm,
    boxrule=0.2mm,
    leftrule=0.2mm, rightrule=0.2mm,
    toprule=0.2mm, bottomrule=0.2mm,
    enhanced,
    breakable
]
\textbf{Action:}

\begin{markdown}
Now I see the key difference clearly:

**Pathway A** (N5-Me TDSO):
- N:4 = **sp$^2$ nitrogen** (=N-, no H)
- N:5 = **sp$^3$ nitrogen** with Me (N-Me)
- Formula: C$_5$H$_8$N$_2$OS
- **The original N-H was replaced by N-Me (H left as HX during alkylation)**

**Pathway B** (N4-Me TDSO):
- N:4 = N with Me 
- N:6 = N with H
- Formula: C$_5$H$_9$N$_2$OS
- **Both H and Me are present (different alkylation mechanism)**

The stoichiometry difference arises because in **Pathway A**, alkylation replaces H, while in **Pathway B**, alkylation adds Me while keeping H.

For a fair comparison, I should include **H$^+$ (solvated proton)** in Pathway B products to balance mass. Let me recalculate properly:
\end{markdown}

\textbf{Tool used:}

\setlength{\parindent}{5pt}\underline{\texttt{Tool Name:}} \texttt{repl\_tool}\par
\setlength{\parindent}{5pt}\underline{\texttt{Arguments:}}\par
\setlength{\parindent}{10pt}\texttt{code =}\par
\begin{verbatim}

import re
import matplotlib.pyplot as plt
import numpy as np

def extract_energy_from_log(log_path):
    """Extract total energy from xTB log file"""
    with open(log_path, 'r') as f:
        content = f.read()
    match = re.search(r'TOTAL ENERGY\s+([-\d.]+)\s+Eh', content)
    if match:
        return float(match.group(1))
    return None

# Energies
energies = {
    'A_reactant': extract_energy_from_log('path_A/N5-Me_TDSO_pathwayA_opt.log'),
    'A_TS': extract_energy_from_log('path_A/TS_pathwayA_opt.log'),
    'A_pyrazole': extract_energy_from_log('path_A/product_1-5-dimethylpyrazole_opt.log'),
    'B_reactant': extract_energy_from_log('path_B/N4-Me_TDSO_pathwayB_opt.log'),
    'B_TS': extract_energy_from_log('path_B/TS_pathwayB_neutral_opt.log'),
    'B_pyrazole': extract_energy_from_log('path_B/product_1-3-dimethylpyrazole_neutral_opt.log'),
    'SO': extract_energy_from_log('common/SO_sulfur_monoxide_opt.log')
}

Eh_to_kcal = 627.509

# For Pathway B: Product = Pyrazole + SO + H+ (to solvent)
# Approximate solvated H+ energy contribution: ~-0.5 Eh (rough estimate for aqueous)
# Actually, let's just compare BARRIERS since they're well-defined

# Calculate relative energies for BARRIERS only
barrier_A = (energies['A_TS'] - energies['A_reactant']) * Eh_to_kcal
barrier_B = (energies['B_TS'] - energies['B_reactant']) * Eh_to_kcal

print("="*60)
print("CORRECTED COMPARISON: Both Pathways Neutral")
print("="*60)
print(f"
Pathway A (N-Me on N adjacent to S, C$_5$H$_8$N$_2$OS):")
print(f"  Structure: Alkylation replaced N-H $\rightarrow$ N-Me")
print(f"  Activation Barrier: {barrier_A:.1f} kcal/mol")

print(f"
Pathway B (N-Me on N away from S, C$_5$H$_9$N$_2$OS):")
print(f"  Structure: Alkylation added Me, kept N-H")
print(f"  Activation Barrier: {barrier_B:.1f} kcal/mol")

print(f"
*** Key Finding ***")
print(f"$\Delta$$\Delta$E‡ (B - A) = {barrier_B - barrier_A:.1f} kcal/mol")
print(f"Pathway A is kinetically favored by {barrier_B - barrier_A:.1f} kcal/mol")

# For products, note the mass imbalance
print(f"
*** Product Mass Balance ***")
print(f"Pathway A: TDSO(C$_5$H$_8$N$_2$OS) $\rightarrow$ Pyrazole(C$_5$H$_8$N$_2$) + SO $\checkmark$")
print(f"Pathway B: TDSO(C$_5$H$_9$N$_2$OS) $\rightarrow$ Pyrazole(C$_5$H$_8$N$_2$) + SO + H$^+$(solvent)")
print(f"  Note: Extra H in Path B transfers to solvent during/after SO extrusion")

# Create the energy profile plot focusing on barriers
fig, ax = plt.subplots(figsize=(12, 8))

# X positions
x = [0, 1, 2]
labels = ['Reactant
(N-Me TDSO)', 'Transition State
(SO Extrusion)', 'Product
(Pyrazole + SO)']

# Pathway A (complete energy profile)
rel_A = [0, barrier_A, (energies['A_pyrazole'] + energies['SO'] - energies['A_reactant']) * Eh_to_kcal]

# Pathway B (barrier only, product shown as dashed since H+ goes to solvent)
rel_B = [0, barrier_B, None]  # Product not directly comparable

# Plot Pathway A
for i, (xi, yi) in enumerate(zip(x, rel_A)):
    ax.hlines(yi, xi - 0.25, xi - 0.02, colors='#2E86AB', linewidth=4)
    ax.text(xi - 0.135, yi + 2, f'{yi:.1f}', ha='center', va='bottom', 
            fontsize=12, color='#2E86AB', fontweight='bold')

# Connect A levels
ax.plot([x[0] - 0.02, x[1] - 0.25], [rel_A[0], rel_A[1]], '--', color='#2E86AB', alpha=0.5, lw=2)
ax.plot([x[1] - 0.02, x[2] - 0.25], [rel_A[1], rel_A[2]], '--', color='#2E86AB', alpha=0.5, lw=2)

# Plot Pathway B (reactant and TS)
for i in [0, 1]:
    yi = [0, barrier_B][i]
    ax.hlines(yi, x[i] + 0.02, x[i] + 0.25, colors='#E94F37', linewidth=4)
    ax.text(x[i] + 0.135, yi + 2, f'{yi:.1f}', ha='center', va='bottom', 
            fontsize=12, color='#E94F37', fontweight='bold')

# Connect B levels (reactant to TS)
ax.plot([x[0] + 0.25, x[1] + 0.02], [0, barrier_B], '--', color='#E94F37', alpha=0.5, lw=2)

# Add dashed line for B product (indicating H+ transfer to solvent)
ax.hlines(rel_A[2], x[2] + 0.02, x[2] + 0.25, colors='#E94F37', linewidth=2, linestyles='dashed')
ax.text(x[2] + 0.135, rel_A[2] - 5, '+ H$^+$$\rightarrow$solv', ha='center', va='top', 
        fontsize=10, color='#E94F37', style='italic')

ax.plot([x[1] + 0.25, x[2] + 0.02], [barrier_B, rel_A[2]], ':', color='#E94F37', alpha=0.5, lw=2)

# Barrier arrows
ax.annotate('', xy=(0.5, barrier_A), xytext=(0.5, 0),
            arrowprops=dict(arrowstyle='<->', color='#2E86AB', lw=2))
ax.text(0.35, barrier_A/2, f'$\Delta$E‡={barrier_A:.1f}', fontsize=11, color='#2E86AB', 
        ha='right', va='center', fontweight='bold')

ax.annotate('', xy=(0.65, barrier_B), xytext=(0.65, 0),
            arrowprops=dict(arrowstyle='<->', color='#E94F37', lw=2))
ax.text(0.8, barrier_B/2, f'$\Delta$E‡={barrier_B:.1f}', fontsize=11, color='#E94F37', 
        ha='left', va='center', fontweight='bold')

# Styling
ax.set_xlim(-0.4, 2.5)
ax.set_ylim(-10, 55)
ax.set_xticks(x)
ax.set_xticklabels(labels, fontsize=11)
ax.set_ylabel('Relative Energy (kcal/mol)', fontsize=14)
ax.set_title('SO Extrusion Step: Comparison of Two N-Alkylation Pathways
(Isothiazole $\rightarrow$ Pyrazole Skeletal Editing)', 
             fontsize=14, fontweight='bold')

# Legend
ax.plot([], [], '-', color='#2E86AB', linewidth=4, label='Path A: N-Me adj. to S (C$_5$H$_8$N$_2$OS)')
ax.plot([], [], '-', color='#E94F37', linewidth=4, label='Path B: N-Me away from S (C$_5$H$_9$N$_2$OS)')
ax.legend(loc='upper right', fontsize=11)

# Info box
textstr = '
'.join([
    'Path A: N-H replaced by N-Me',
    'Path B: N-Me added, N-H retained',
    '',
    f'$\Delta$$\Delta$E‡ (B-A) = +{barrier_B - barrier_A:.1f} kcal/mol',
    '$\rightarrow$ Pathway A kinetically favored'
])
props = dict(boxstyle='round', facecolor='lightyellow', alpha=0.9)
ax.text(0.02, 0.98, textstr, transform=ax.transAxes, fontsize=11,
        verticalalignment='top', bbox=props)

ax.axhline(y=0, color='gray', linestyle='-', linewidth=0.5)
ax.grid(True, axis='y', alpha=0.3)

plt.tight_layout()
plt.savefig('SO_extrusion_energy_profile_corrected.png', dpi=300, bbox_inches='tight', facecolor='white')
print("
Plot saved to: SO_extrusion_energy_profile_corrected.png")

\end{verbatim}\par
\smallskip
\end{tcolorbox}

\setlength{\parindent}{5pt} \robot \hspace{2pt} \textbf{Estructural}

\begin{tcolorbox}[
    colback=matterbg2,
    colframe=mattergreen1,
    width=\textwidth,
    arc=2mm,
    boxrule=0.2mm,
    leftrule=0.2mm, rightrule=0.2mm,
    toprule=0.2mm, bottomrule=0.2mm,
    enhanced,
    breakable
]
\textbf{Action:}

\begin{markdown}
Let me display the corrected energy profile:
\end{markdown}

\textbf{Tool used:}

\setlength{\parindent}{5pt}\underline{\texttt{Tool Name:}} \texttt{view\_png\_file}\par
\setlength{\parindent}{5pt}\underline{\texttt{Arguments:}}\par
\setlength{\parindent}{10pt}\texttt{png\_file\_relative\_path = SO\_extrusion\_energy\_profile\_corrected.png}\par
\smallskip
\end{tcolorbox}

\setlength{\parindent}{5pt} \robot \hspace{2pt} \textbf{Estructural}

\begin{tcolorbox}[
    colback=matterbg2,
    colframe=mattergreen1,
    width=\textwidth,
    arc=2mm,
    boxrule=0.2mm,
    leftrule=0.2mm, rightrule=0.2mm,
    toprule=0.2mm, bottomrule=0.2mm,
    enhanced,
    breakable
]
\textbf{Action:}

\begin{markdown}
I see the issue! The **reaction energy for Pathway B is very high (315.7 kcal/mol)** because:
- Pathway B intermediate has **N-H** (extra H atom)
- The product is neutral pyrazole (no N-H)
- The H+ goes to solvent, but we're not accounting for the solvation energy!

The **barrier comparison is valid** (both species have same H count up to TS), but the **product energies are not directly comparable** due to different atom counts.

Let me create an updated energy profile that properly shows this:
\end{markdown}

\textbf{Tool used:}

\setlength{\parindent}{5pt}\underline{\texttt{Tool Name:}} \texttt{repl\_tool}\par
\setlength{\parindent}{5pt}\underline{\texttt{Arguments:}}\par
\setlength{\parindent}{10pt}\texttt{code =}\par
\begin{verbatim}

import matplotlib.pyplot as plt
import numpy as np

# Energy data (kcal/mol) - ALL NEUTRAL
pathway_A = {'Reactant': 0.0, 'TS': 34.10, 'Product': 18.37}
pathway_B = {'Reactant': 0.0, 'TS': 40.57, 'Product': None}  # Product not comparable

# For Pathway B product, we estimate with proton solvation
# H+ solvation energy is approximately -270 kcal/mol (very rough estimate)
# This would make Pathway B product roughly: 315.7 - 270 = ~45 kcal/mol
# But this is very dependent on solvent, so we'll show it as uncertain

# Create figure
fig, ax = plt.subplots(figsize=(12, 8))

# X positions
x_positions = [0, 1, 2]

# Plot Pathway A (complete)
y_A = [pathway_A['Reactant'], pathway_A['TS'], pathway_A['Product']]
for i, (x, y) in enumerate(zip(x_positions, y_A)):
    ax.hlines(y, x - 0.3, x - 0.05, colors='#2E86AB', linewidth=3, 
              label='Pathway A (N-Me adj. to S)' if i == 0 else '')
    ax.text(x - 0.175, y + 2, f'{y:.1f}', ha='center', va='bottom', 
            fontsize=11, color='#2E86AB', fontweight='bold')

# Plot Pathway B (TS only, product uncertain)
y_B_partial = [pathway_B['Reactant'], pathway_B['TS']]
for i, (x, y) in enumerate(zip(x_positions[:2], y_B_partial)):
    ax.hlines(y, x + 0.05, x + 0.3, colors='#E94F37', linewidth=3,
              label='Pathway B (N-Me away from S)' if i == 0 else '')
    ax.text(x + 0.175, y + 2, f'{y:.1f}', ha='center', va='bottom', 
            fontsize=11, color='#E94F37', fontweight='bold')

# Show uncertain product for Pathway B (with dashed box)
ax.hlines(45, 1.75, 2.3, colors='#E94F37', linewidth=2, linestyle='--', alpha=0.5)
ax.text(2.025, 48, '~45?', ha='center', va='bottom', fontsize=10, 
        color='#E94F37', alpha=0.7, style='italic')
ax.text(2.025, 38, '(after H$^+$
solvation)', ha='center', va='top', 
        fontsize=8, color='#E94F37', alpha=0.7)

# Connect levels with dashed lines
# Pathway A
ax.plot([x_positions[0] - 0.05, x_positions[1] - 0.3], [y_A[0], y_A[1]], 
        '--', color='#2E86AB', alpha=0.5, linewidth=1.5)
ax.plot([x_positions[1] - 0.05, x_positions[2] - 0.3], [y_A[1], y_A[2]], 
        '--', color='#2E86AB', alpha=0.5, linewidth=1.5)
# Pathway B (partial)
ax.plot([x_positions[0] + 0.3, x_positions[1] + 0.05], [y_B_partial[0], y_B_partial[1]], 
        '--', color='#E94F37', alpha=0.5, linewidth=1.5)
ax.plot([x_positions[1] + 0.3, 1.75], [y_B_partial[1], 45], 
        '--', color='#E94F37', alpha=0.3, linewidth=1.5)

# Add barrier annotations
ax.annotate('', xy=(0.5, pathway_A['TS']), xytext=(0.5, pathway_A['Reactant']),
            arrowprops=dict(arrowstyle='<->', color='#2E86AB', lw=1.5))
ax.text(0.35, pathway_A['TS']/2, f'$\Delta$E‡ = {pathway_A["TS"]:.1f}', 
        fontsize=10, color='#2E86AB', ha='right', va='center')

ax.annotate('', xy=(0.7, pathway_B['TS']), xytext=(0.7, pathway_B['Reactant']),
            arrowprops=dict(arrowstyle='<->', color='#E94F37', lw=1.5))
ax.text(0.85, pathway_B['TS']/2, f'$\Delta$E‡ = {pathway_B["TS"]:.1f}', 
        fontsize=10, color='#E94F37', ha='left', va='center')

# Add $\Delta$$\Delta$E‡ annotation
ax.annotate('', xy=(1.15, pathway_B['TS']), xytext=(1.15, pathway_A['TS']),
            arrowprops=dict(arrowstyle='<->', color='green', lw=2))
ax.text(1.25, (pathway_A['TS'] + pathway_B['TS'])/2, 
        f'$\Delta$$\Delta$E‡ = {pathway_B["TS"] - pathway_A["TS"]:.1f}', 
        fontsize=11, color='green', ha='left', va='center', fontweight='bold')

# Styling
ax.set_xlim(-0.5, 2.6)
ax.set_ylim(-10, 60)
ax.set_xticks(x_positions)
ax.set_xticklabels(['Reactant
(N-Me TDSO)', 'Transition State', 'Product
(Pyrazole + SO)'], fontsize=12)
ax.set_ylabel('Relative Energy (kcal/mol)', fontsize=14)
ax.set_xlabel('Reaction Coordinate', fontsize=14)
ax.set_title('SO Extrusion Step: Comparison of Two Pathways (NEUTRAL)
(Isothiazole $\rightarrow$ Pyrazole Single-Atom Skeletal Editing)', 
             fontsize=14, fontweight='bold')

ax.legend(loc='upper right', fontsize=11, framealpha=0.9)

# Add text box with summary
textstr = '
'.join([
    'Key Difference in Intermediates:',
    '• Pathway A: No N-H (16 atoms)',
    '• Pathway B: Has N-H (18 atoms)',
    '',
    'Barrier Comparison (VALID):',
    f'  Pathway A: $\Delta$E‡ = {pathway_A["TS"]:.1f} kcal/mol',
    f'  Pathway B: $\Delta$E‡ = {pathway_B["TS"]:.1f} kcal/mol',
    f'  $\rightarrow$ Pathway A favored by {pathway_B["TS"] - pathway_A["TS"]:.1f} kcal/mol',
    '',
    'Product Comparison:',
    '  Pathway B loses H$^+$ to solvent',
    '  (requires solvation correction)'
])
props = dict(boxstyle='round', facecolor='wheat', alpha=0.9)
ax.text(0.02, 0.98, textstr, transform=ax.transAxes, fontsize=9,
        verticalalignment='top', bbox=props)

# Add grid
ax.axhline(y=0, color='gray', linestyle='-', linewidth=0.5, alpha=0.5)
ax.grid(True, axis='y', alpha=0.3)

# Add molecule labels
ax.text(-0.175, -7, 'N5-Me TDSO
(no N-H)', ha='center', fontsize=9, color='#2E86AB', style='italic')
ax.text(0.175, -7, 'N4-Me TDSO
(has N-H)', ha='center', fontsize=9, color='#E94F37', style='italic')

plt.tight_layout()
plt.savefig('SO_extrusion_energy_profile_corrected.png', dpi=300, bbox_inches='tight', facecolor='white')
plt.savefig('common/SO_extrusion_energy_profile_corrected.png', dpi=300, bbox_inches='tight', facecolor='white')
print("Corrected energy profile saved!")

print("
" + "="*60)
print("=== FINAL SUMMARY: SO Extrusion Step (Both NEUTRAL) ===")
print("="*60)
print(f"""
Pathway A (N-Me adjacent to S, no N-H):
  • Intermediate: N5-Me TDSO (16 atoms)
  • Activation barrier: {pathway_A['TS']:.1f} kcal/mol
  • Product: 1,5-dimethylpyrazole + SO
  • Reaction energy: {pathway_A['Product']:.1f} kcal/mol

Pathway B (N-Me away from S, has N-H):
  • Intermediate: N4-Me TDSO (18 atoms, includes N-H)
  • Activation barrier: {pathway_B['TS']:.1f} kcal/mol
  • Product: 1,3-dimethylpyrazole + SO + H$^+$(solvent)
  • Reaction energy: requires H$^+$ solvation correction

KEY RESULT:
  $\Delta$$\Delta$E‡ = {pathway_B['TS'] - pathway_A['TS']:.1f} kcal/mol
  $\rightarrow$ Pathway A is kinetically FAVORED

Note: Both pathways are NEUTRAL throughout (no anionic species).
The N-H in Pathway B transfers to solvent during/after SO extrusion.
""")

\end{verbatim}\par
\smallskip
\end{tcolorbox}

\setlength{\parindent}{5pt} \robot \hspace{2pt} \textbf{Estructural}

\begin{tcolorbox}[
    colback=matterbg2,
    colframe=mattergreen1,
    width=\textwidth,
    arc=2mm,
    boxrule=0.2mm,
    leftrule=0.2mm, rightrule=0.2mm,
    toprule=0.2mm, bottomrule=0.2mm,
    enhanced,
    breakable
]
\textbf{Action:}

\begin{markdown}
Let me display the corrected energy profile:
\end{markdown}

\textbf{Tool used:}

\setlength{\parindent}{5pt}\underline{\texttt{Tool Name:}} \texttt{view\_png\_file}\par
\setlength{\parindent}{5pt}\underline{\texttt{Arguments:}}\par
\setlength{\parindent}{10pt}\texttt{png\_file\_relative\_path = SO\_extrusion\_energy\_profile\_corrected.png}\par
\smallskip
\end{tcolorbox}

\setlength{\parindent}{5pt} \robot \hspace{2pt} \textbf{Estructural}

\begin{tcolorbox}[
    colback=matterbg2,
    colframe=mattergreen1,
    width=\textwidth,
    arc=2mm,
    boxrule=0.2mm,
    leftrule=0.2mm, rightrule=0.2mm,
    toprule=0.2mm, bottomrule=0.2mm,
    enhanced,
    breakable
]
\textbf{Action:}

\begin{markdown}
Excellent! Here's the **corrected and complete summary**:

---

****Final Summary: SO Extrusion Step - BOTH PATHWAYS NEUTRAL****

****Key Correction****
You were absolutely right - **there are NO anionic species** in either pathway! Both pathways are neutral throughout:

| Feature | Pathway A | Pathway B |
|---------|-----------|-----------|
| **N-Me position** | Adjacent to S (N5) | Away from S (N4) |
| **N-H in intermediate** | **No** | **Yes** (on N6, adjacent to S) |
| **Charge** | Neutral (0) | Neutral (0) |
| **Atoms in intermediate** | 16 | 18 (extra H) |

---

****Energy Profile Results (Corrected)****

| Parameter | Pathway A | Pathway B |
|-----------|-----------|-----------|
| **Activation Barrier ($\Delta$E‡)** | **34.1 kcal/mol** | **40.6 kcal/mol** |
| **$\Delta$$\Delta$E‡ (B - A)** | --- | **+6.5 kcal/mol** |
| **Product Energy** | 18.4 kcal/mol | ~45? (needs H$^+$ solvation) |

****Key Result****
> **Pathway A is kinetically favored by 6.5 kcal/mol**

---

****Mechanistic Understanding****

```
Pathway A:                           Pathway B:
N5-Me TDSO (no N-H)                  N4-Me TDSO (has N-H)
    |                                    |
    | $\Delta$E‡ = 34.1 kcal/mol                | $\Delta$E‡ = 40.6 kcal/mol
    [down]                                    [down]
    TS                                   TS
    |                                    |
    [down]                                    [down]
1,5-dimethylpyrazole + SO            1,3-dimethylpyrazole + SO + H$^+$(solv)
```

The **N-H in Pathway B** transfers to solvent during/after SO extrusion (proton exchange with solvent), keeping everything neutral but adding complexity to the product energy comparison.

---

****Final File Organization****

```
+-- common/          $\leftarrow$ Shared structures & energy profiles
+-- path_A/          $\leftarrow$ Pathway A: N-Me adj. to S (FAVORED)
|   +-- N5-Me_TDSO_pathwayA_opt.xyz
|   +-- TS_pathwayA_opt.xyz
|   +-- product_1-5-dimethylpyrazole_opt.xyz
+-- path_B/          $\leftarrow$ Pathway B: N-Me away from S, N-H adj. to S
|   +-- N4-Me_TDSO_pathwayB_opt.xyz (neutral, with N-H)
|   +-- TS_pathwayB_neutral_opt.xyz
|   +-- product_1-3-dimethylpyrazole_neutral_opt.xyz
+-- misc/            $\leftarrow$ Old files and images
```

Thank you for the correction! The key insight is that proton exchange with solvent allows both pathways to remain neutral while still having different H atom distributions in their intermediates.
\end{markdown}

\end{tcolorbox}

\setlength{\parindent}{5pt} \textbf{\textcolor{blue}{User:}}
\begin{tcolorbox}[
    colback=blue!10,
    colframe=blue,
    width=\textwidth,
    arc=2mm,
    boxrule=0.2mm,
    leftrule=0.2mm, rightrule=0.2mm,
    toprule=0.2mm, bottomrule=0.2mm,
    enhanced,
    breakable
]
\begin{markdown}
Let me correct myself, there should not be any charged species, as alkylation removes H with R and end up with neutral.
\end{markdown}
\end{tcolorbox}
\setlength{\parindent}{5pt} \robot \hspace{2pt} \textbf{Estructural}

\begin{tcolorbox}[
    colback=matterbg2,
    colframe=mattergreen1,
    width=\textwidth,
    arc=2mm,
    boxrule=0.2mm,
    leftrule=0.2mm, rightrule=0.2mm,
    toprule=0.2mm, bottomrule=0.2mm,
    enhanced,
    breakable
]
\textbf{Action:}

\begin{markdown}
Now I understand! The N-alkylation is a **substitution** where H leaves with R (like R-X + N-H $\rightarrow$ N-R + HX). So:

- **Both pathways should have the SAME number of atoms**
- **No N-H in either intermediate after alkylation**
- **Both are neutral with identical molecular formula**

The difference is just which N gets alkylated:
- **Pathway A**: N-Me on N adjacent to S
- **Pathway B**: N-Me on N away from S (H was removed during alkylation, not retained!)

Let me generate the CORRECT Pathway B intermediate (without N-H):
\end{markdown}

\textbf{Tool used:}

\setlength{\parindent}{5pt}\underline{\texttt{Tool Name:}} \texttt{organic\_molecules\_xyz\_generation}\par
\setlength{\parindent}{5pt}\underline{\texttt{Arguments:}}\par
\setlength{\parindent}{10pt}\texttt{smiles\_list = ["CC1=CC=N(C)NS(=O)1"]}\par
\setlength{\parindent}{10pt}\texttt{filenames = ["path\_B/N4-Me\_TDSO\_correct.xyz"]}\par
\smallskip
\end{tcolorbox}

\setlength{\parindent}{5pt} \robot \hspace{2pt} \textbf{Estructural}

\begin{tcolorbox}[
    colback=matterbg2,
    colframe=mattergreen1,
    width=\textwidth,
    arc=2mm,
    boxrule=0.2mm,
    leftrule=0.2mm, rightrule=0.2mm,
    toprule=0.2mm, bottomrule=0.2mm,
    enhanced,
    breakable
]
\textbf{Action:}

\begin{markdown}
The SMILES failed. But wait - the **"deprotonated" structure I created earlier is actually CORRECT!** It has:
- N-Me on N4 (away from S)  
- No N-H (H was removed during alkylation)
- Same atom count as Pathway A

I just need to optimize it with **charge=0** (neutral), not -1. Let me fix this:
\end{markdown}

\textbf{Tool used:}

\setlength{\parindent}{5pt}\underline{\texttt{Tool Name:}} \texttt{constraint\_xtb}\par
\setlength{\parindent}{5pt}\underline{\texttt{Arguments:}}\par
\setlength{\parindent}{10pt}\texttt{input\_xyz = path\_B/N4-Me\_TDSO\_deprotonated.xyz}\par
\setlength{\parindent}{10pt}\texttt{output\_xyz = path\_B/N4-Me\_TDSO\_correct\_opt.xyz}\par
\setlength{\parindent}{10pt}\texttt{charge = 0}\par
\smallskip
\end{tcolorbox}

\setlength{\parindent}{5pt} \robot \hspace{2pt} \textbf{Estructural}

\begin{tcolorbox}[
    colback=matterbg2,
    colframe=mattergreen1,
    width=\textwidth,
    arc=2mm,
    boxrule=0.2mm,
    leftrule=0.2mm, rightrule=0.2mm,
    toprule=0.2mm, bottomrule=0.2mm,
    enhanced,
    breakable
]
\textbf{Action:}

\begin{markdown}
Now let me verify the correct Pathway B intermediate structure:
\end{markdown}

\textbf{Tool used:}

\setlength{\parindent}{5pt}\underline{\texttt{Tool Name:}} \texttt{view\_molecule}\par
\setlength{\parindent}{5pt}\underline{\texttt{Arguments:}}\par
\setlength{\parindent}{10pt}\texttt{xyz\_file\_relative\_path = path\_B/N4-Me\_TDSO\_correct\_opt.xyz}\par
\setlength{\parindent}{10pt}\texttt{left\_right\_deg = 0}\par
\setlength{\parindent}{10pt}\texttt{up\_down\_deg = 0}\par
\smallskip
\end{tcolorbox}

\setlength{\parindent}{5pt} \robot \hspace{2pt} \textbf{Estructural}

\begin{tcolorbox}[
    colback=matterbg2,
    colframe=mattergreen1,
    width=\textwidth,
    arc=2mm,
    boxrule=0.2mm,
    leftrule=0.2mm, rightrule=0.2mm,
    toprule=0.2mm, bottomrule=0.2mm,
    enhanced,
    breakable
]
\textbf{Action:}

\begin{markdown}
Now the structure is correct:
- **N:4 has N-Me** (C:5) - away from S $\checkmark$
- **N:6 has NO H** - just sp2 nitrogen adjacent to S $\checkmark$
- **Same atom count as Pathway A** (16 atoms) $\checkmark$
- **Neutral (charge=0)** $\checkmark$

Now let me generate the correct TS for Pathway B:
\end{markdown}

\textbf{Tool used:}

\setlength{\parindent}{5pt}\underline{\texttt{Tool Name:}} \texttt{constraint\_xtb}\par
\setlength{\parindent}{5pt}\underline{\texttt{Arguments:}}\par
\setlength{\parindent}{10pt}\texttt{input\_xyz = path\_B/N4-Me\_TDSO\_correct\_opt.xyz}\par
\setlength{\parindent}{10pt}\texttt{output\_xyz = path\_B/TS\_pathwayB\_correct\_opt.xyz}\par
\setlength{\parindent}{10pt}\texttt{distance\_constraints = [\{"atoms": [7, 1], "value": 2.2\}, \{"atoms": [7, 6], "value": 2.1\}, \{"atoms": [1, 6], "value": 1.9\}]}\par
\setlength{\parindent}{10pt}\texttt{force\_constant = 0.5}\par
\setlength{\parindent}{10pt}\texttt{charge = 0}\par
\smallskip
\end{tcolorbox}

\setlength{\parindent}{5pt} \robot \hspace{2pt} \textbf{Estructural}

\begin{tcolorbox}[
    colback=matterbg2,
    colframe=mattergreen1,
    width=\textwidth,
    arc=2mm,
    boxrule=0.2mm,
    leftrule=0.2mm, rightrule=0.2mm,
    toprule=0.2mm, bottomrule=0.2mm,
    enhanced,
    breakable
]
\textbf{Action:}

\begin{markdown}
TS generated. Now let me verify the distances and recalculate the energy profile with **identical atom counts** for both pathways:
\end{markdown}

\textbf{Tool used:}

\setlength{\parindent}{5pt}\underline{\texttt{Tool Name:}} \texttt{get\_distance\_angle\_dihedral}\par
\setlength{\parindent}{5pt}\underline{\texttt{Arguments:}}\par
\setlength{\parindent}{10pt}\texttt{input\_path = path\_B/TS\_pathwayB\_correct\_opt.xyz}\par
\setlength{\parindent}{10pt}\texttt{targets = [\{"atom": [1]\}, \{"atom": [6]\}]}\par
\smallskip
\end{tcolorbox}

\setlength{\parindent}{5pt} \robot \hspace{2pt} \textbf{Estructural}

\begin{tcolorbox}[
    colback=matterbg2,
    colframe=mattergreen1,
    width=\textwidth,
    arc=2mm,
    boxrule=0.2mm,
    leftrule=0.2mm, rightrule=0.2mm,
    toprule=0.2mm, bottomrule=0.2mm,
    enhanced,
    breakable
]
\textbf{Action:}

\begin{markdown}
C:1-N:6 forming bond = **1.86 Å** $\checkmark$

Now let me recalculate the energy profile with **CORRECT structures** (same atom count, both neutral):
\end{markdown}

\textbf{Tool used:}

\setlength{\parindent}{5pt}\underline{\texttt{Tool Name:}} \texttt{repl\_tool}\par
\setlength{\parindent}{5pt}\underline{\texttt{Arguments:}}\par
\setlength{\parindent}{10pt}\texttt{code =}\par
\begin{verbatim}

import re
import matplotlib.pyplot as plt
import numpy as np

def extract_energy_from_log(log_path):
    """Extract total energy from xTB log file"""
    try:
        with open(log_path, 'r') as f:
            content = f.read()
        match = re.search(r'TOTAL ENERGY\s+([-\d.]+)\s+Eh', content)
        if match:
            return float(match.group(1))
    except:
        return None
    return None

# Extract all energies for CORRECT neutral species (same atom count!)
energies = {
    # Pathway A (neutral, N-Me adjacent to S)
    'A_reactant': extract_energy_from_log('path_A/N5-Me_TDSO_pathwayA_opt.log'),
    'A_TS': extract_energy_from_log('path_A/TS_pathwayA_opt.log'),
    'A_pyrazole': extract_energy_from_log('path_A/product_1-5-dimethylpyrazole_opt.log'),
    
    # Pathway B CORRECTED (neutral, N-Me away from S, NO N-H!)
    'B_reactant': extract_energy_from_log('path_B/N4-Me_TDSO_correct_opt.log'),
    'B_TS': extract_energy_from_log('path_B/TS_pathwayB_correct_opt.log'),
    'B_pyrazole': extract_energy_from_log('path_B/product_1-3-dimethylpyrazole_neutral_opt.log'),
    
    # Common SO
    'SO': extract_energy_from_log('common/SO_sulfur_monoxide_opt.log')
}

print("=== Absolute Energies (Eh) - BOTH NEUTRAL, SAME ATOM COUNT ===")
for k, v in energies.items():
    if v is not None:
        print(f"{k}: {v:.6f} Eh")
    else:
        print(f"{k}: NOT FOUND")

# Calculate product energies (pyrazole + SO)
energies['A_product'] = energies['A_pyrazole'] + energies['SO']
energies['B_product'] = energies['B_pyrazole'] + energies['SO']

print(f"
SO energy: {energies['SO']:.6f} Eh")
print(f"A_product (1,5-dimethylpyrazole + SO): {energies['A_product']:.6f} Eh")
print(f"B_product (1,3-dimethylpyrazole + SO): {energies['B_product']:.6f} Eh")

# Convert to relative energies (kcal/mol)
Eh_to_kcal = 627.509

rel_A = {
    'Reactant': 0.0,
    'TS': (energies['A_TS'] - energies['A_reactant']) * Eh_to_kcal,
    'Product': (energies['A_product'] - energies['A_reactant']) * Eh_to_kcal
}

rel_B = {
    'Reactant': 0.0,
    'TS': (energies['B_TS'] - energies['B_reactant']) * Eh_to_kcal,
    'Product': (energies['B_product'] - energies['B_reactant']) * Eh_to_kcal
}

print("
=== Relative Energies (kcal/mol) ===")
print("
Pathway A (N-Me adjacent to S):")
for species, energy in rel_A.items():
    print(f"  {species}: {energy:.2f} kcal/mol")

print("
Pathway B (N-Me away from S):")
for species, energy in rel_B.items():
    print(f"  {species}: {energy:.2f} kcal/mol")

# Summary
barrier_A = rel_A['TS']
barrier_B = rel_B['TS']
rxn_A = rel_A['Product']
rxn_B = rel_B['Product']

print("
" + "="*60)
print("=== FINAL CORRECTED SUMMARY ===")
print("=== Both Neutral, Same Atom Count, Direct Comparison Valid ===")
print("="*60)
print(f"
Pathway A (N-Me adjacent to S):")
print(f"  Activation barrier ($\Delta$E‡): {barrier_A:.1f} kcal/mol")
print(f"  Reaction energy ($\Delta$E_rxn): {rxn_A:.1f} kcal/mol")

print(f"
Pathway B (N-Me away from S):")
print(f"  Activation barrier ($\Delta$E‡): {barrier_B:.1f} kcal/mol")
print(f"  Reaction energy ($\Delta$E_rxn): {rxn_B:.1f} kcal/mol")

print(f"
*** Comparison (B - A) ***")
print(f"  $\Delta$$\Delta$E‡ (barrier):  {barrier_B - barrier_A:+.1f} kcal/mol")
print(f"  $\Delta$$\Delta$E_rxn:         {rxn_B - rxn_A:+.1f} kcal/mol")

if barrier_A < barrier_B:
    print(f"
$\rightarrow$ Pathway A is kinetically FAVORED by {barrier_B - barrier_A:.1f} kcal/mol")
else:
    print(f"
$\rightarrow$ Pathway B is kinetically FAVORED by {barrier_A - barrier_B:.1f} kcal/mol")

\end{verbatim}\par
\smallskip
\end{tcolorbox}

\setlength{\parindent}{5pt} \robot \hspace{2pt} \textbf{Estructural}

\begin{tcolorbox}[
    colback=matterbg2,
    colframe=mattergreen1,
    width=\textwidth,
    arc=2mm,
    boxrule=0.2mm,
    leftrule=0.2mm, rightrule=0.2mm,
    toprule=0.2mm, bottomrule=0.2mm,
    enhanced,
    breakable
]
\textbf{Action:}

\begin{markdown}
**WOW!** The results are completely different with the correct structures!

****CORRECTED RESULTS (Both Neutral, Same Atom Count)****

| Parameter | Pathway A | Pathway B | Difference (B-A) |
|-----------|-----------|-----------|------------------|
| **$\Delta$E‡ (barrier)** | 34.1 kcal/mol | **22.6 kcal/mol** | **-11.5 kcal/mol** |
| **$\Delta$E\\textunderscore{}rxn** | 18.4 kcal/mol | **9.0 kcal/mol** | **-9.4 kcal/mol** |

****Pathway B is now kinetically FAVORED by 11.5 kcal/mol!****

This is a complete reversal from the earlier (incorrect) analysis. Let me create the corrected energy profile:
\end{markdown}

\textbf{Tool used:}

\setlength{\parindent}{5pt}\underline{\texttt{Tool Name:}} \texttt{repl\_tool}\par
\setlength{\parindent}{5pt}\underline{\texttt{Arguments:}}\par
\setlength{\parindent}{10pt}\texttt{code =}\par
\begin{verbatim}

import matplotlib.pyplot as plt
import numpy as np

# CORRECTED Energy data (kcal/mol) - Both Neutral, Same Atom Count
pathway_A = {'Reactant': 0.0, 'TS': 34.10, 'Product': 18.37}
pathway_B = {'Reactant': 0.0, 'TS': 22.56, 'Product': 8.95}

# Create figure
fig, ax = plt.subplots(figsize=(12, 8))

# X positions
x_positions = [0, 1, 2]

# Plot Pathway A
y_A = [pathway_A['Reactant'], pathway_A['TS'], pathway_A['Product']]
for i, (x, y) in enumerate(zip(x_positions, y_A)):
    ax.hlines(y, x - 0.3, x - 0.05, colors='#2E86AB', linewidth=3, 
              label='Pathway A (N-Me adj. to S)' if i == 0 else '')
    ax.text(x - 0.175, y + 1.5, f'{y:.1f}', ha='center', va='bottom', 
            fontsize=11, color='#2E86AB', fontweight='bold')

# Plot Pathway B
y_B = [pathway_B['Reactant'], pathway_B['TS'], pathway_B['Product']]
for i, (x, y) in enumerate(zip(x_positions, y_B)):
    ax.hlines(y, x + 0.05, x + 0.3, colors='#E94F37', linewidth=3,
              label='Pathway B (N-Me away from S)' if i == 0 else '')
    ax.text(x + 0.175, y + 1.5, f'{y:.1f}', ha='center', va='bottom', 
            fontsize=11, color='#E94F37', fontweight='bold')

# Connect levels with dashed lines
for i in range(len(x_positions) - 1):
    ax.plot([x_positions[i] - 0.05, x_positions[i+1] - 0.3], [y_A[i], y_A[i+1]], 
            '--', color='#2E86AB', alpha=0.5, linewidth=1.5)
    ax.plot([x_positions[i] + 0.3, x_positions[i+1] + 0.05], [y_B[i], y_B[i+1]], 
            '--', color='#E94F37', alpha=0.5, linewidth=1.5)

# Add barrier annotations
ax.annotate('', xy=(0.5, pathway_A['TS']), xytext=(0.5, pathway_A['Reactant']),
            arrowprops=dict(arrowstyle='<->', color='#2E86AB', lw=1.5))
ax.text(0.35, pathway_A['TS']/2, f'$\Delta$E‡ = {pathway_A["TS"]:.1f}', 
        fontsize=10, color='#2E86AB', ha='right', va='center')

ax.annotate('', xy=(0.7, pathway_B['TS']), xytext=(0.7, pathway_B['Reactant']),
            arrowprops=dict(arrowstyle='<->', color='#E94F37', lw=1.5))
ax.text(0.85, pathway_B['TS']/2, f'$\Delta$E‡ = {pathway_B["TS"]:.1f}', 
        fontsize=10, color='#E94F37', ha='left', va='center')

# Add $\Delta$$\Delta$E‡ annotation (highlight the key result!)
ax.annotate('', xy=(1.15, pathway_A['TS']), xytext=(1.15, pathway_B['TS']),
            arrowprops=dict(arrowstyle='<->', color='green', lw=2.5))
ax.text(1.25, (pathway_A['TS'] + pathway_B['TS'])/2, 
        f'$\Delta$$\Delta$E‡ = {pathway_B["TS"] - pathway_A["TS"]:.1f}
kcal/mol', 
        fontsize=12, color='green', ha='left', va='center', fontweight='bold')

# Styling
ax.set_xlim(-0.5, 2.5)
ax.set_ylim(-5, 45)
ax.set_xticks(x_positions)
ax.set_xticklabels(['Reactant
(N-Me TDSO)', 'Transition State', 'Product
(Dimethylpyrazole + SO)'], fontsize=12)
ax.set_ylabel('Relative Energy (kcal/mol)', fontsize=14)
ax.set_xlabel('Reaction Coordinate', fontsize=14)
ax.set_title('SO Extrusion Step: CORRECTED Energy Profile
(Both Pathways Neutral, Same Atom Count)', 
             fontsize=14, fontweight='bold')

ax.legend(loc='upper right', fontsize=11, framealpha=0.9)

# Add text box with summary
textstr = '
'.join([
    'CORRECTED ANALYSIS:',
    '• Both pathways: Neutral (charge=0)',
    '• Same atom count (16 atoms)',
    '• Direct comparison VALID',
    '',
    'RESULTS:',
    f'  Pathway A: $\Delta$E‡ = {pathway_A["TS"]:.1f} kcal/mol',
    f'  Pathway B: $\Delta$E‡ = {pathway_B["TS"]:.1f} kcal/mol',
    '',
    '$\star$ Pathway B FAVORED',
    f'   by {pathway_A["TS"] - pathway_B["TS"]:.1f} kcal/mol $\star$'
])
props = dict(boxstyle='round', facecolor='lightgreen', alpha=0.9)
ax.text(0.02, 0.98, textstr, transform=ax.transAxes, fontsize=10,
        verticalalignment='top', bbox=props)

# Add molecule labels
ax.text(-0.175, -3, '1,5-dimethyl
position', ha='center', fontsize=9, color='#2E86AB', style='italic')
ax.text(0.175, -3, '1,3-dimethyl
position', ha='center', fontsize=9, color='#E94F37', style='italic')

# Add grid
ax.axhline(y=0, color='gray', linestyle='-', linewidth=0.5, alpha=0.5)
ax.grid(True, axis='y', alpha=0.3)

plt.tight_layout()
plt.savefig('SO_extrusion_FINAL_corrected.png', dpi=300, bbox_inches='tight', facecolor='white')
plt.savefig('common/SO_extrusion_FINAL_corrected.png', dpi=300, bbox_inches='tight', facecolor='white')
print("Final corrected energy profile saved!")

\end{verbatim}\par
\smallskip
\end{tcolorbox}

\setlength{\parindent}{5pt} \robot \hspace{2pt} \textbf{Estructural}

\begin{tcolorbox}[
    colback=matterbg2,
    colframe=mattergreen1,
    width=\textwidth,
    arc=2mm,
    boxrule=0.2mm,
    leftrule=0.2mm, rightrule=0.2mm,
    toprule=0.2mm, bottomrule=0.2mm,
    enhanced,
    breakable
]
\textbf{Action:}

\begin{markdown}
Let me display the final corrected energy profile:
\end{markdown}

\textbf{Tool used:}

\setlength{\parindent}{5pt}\underline{\texttt{Tool Name:}} \texttt{view\_png\_file}\par
\setlength{\parindent}{5pt}\underline{\texttt{Arguments:}}\par
\setlength{\parindent}{10pt}\texttt{png\_file\_relative\_path = SO\_extrusion\_FINAL\_corrected.png}\par
\smallskip
\end{tcolorbox}

\setlength{\parindent}{5pt} \robot \hspace{2pt} \textbf{Estructural}

\begin{tcolorbox}[
    colback=matterbg2,
    colframe=mattergreen1,
    width=\textwidth,
    arc=2mm,
    boxrule=0.2mm,
    leftrule=0.2mm, rightrule=0.2mm,
    toprule=0.2mm, bottomrule=0.2mm,
    enhanced,
    breakable
]
\textbf{Action:}

\begin{markdown}
---

****FINAL CORRECTED Summary****

Thank you for the crucial correction! With **N-alkylation removing H with R** (neutral throughout), here are the correct results:

---

****Key Corrections Applied****
| Issue | Before | After (Corrected) |
|-------|--------|-------------------|
| **Pathway B intermediate** | Had N-H (18 atoms) | No N-H (16 atoms) |
| **Comparison validity** | Different atom counts | Same atom counts $\checkmark$ |
| **Charge states** | Some anionic species | All neutral (charge=0) $\checkmark$ |

---

****FINAL RESULTS (Both Neutral, Same Atom Count)****

| Parameter | Pathway A | Pathway B | $\Delta$(B-A) |
|-----------|-----------|-----------|--------|
| **N-Me position** | Adjacent to S | Away from S | --- |
| **$\Delta$E‡ (barrier)** | 34.1 kcal/mol | **22.6 kcal/mol** | **-11.5** |
| **$\Delta$E\\textunderscore{}rxn** | 18.4 kcal/mol | **9.0 kcal/mol** | **-9.4** |

**$\star$ **Pathway B is FAVORED by 11.5 kcal/mol** $\star$**

---

****Chemical Interpretation****

When **N-Me is positioned AWAY from S** (Pathway B):
- **Lower activation barrier** (22.6 vs 34.1 kcal/mol)
- **More exothermic** (or less endothermic) reaction
- Likely due to **reduced steric/electronic repulsion** during SO extrusion

---

****Final Correct File Structure****

```
+-- path_A/  (N-Me adjacent to S)
|   +-- N5-Me_TDSO_pathwayA_opt.xyz     $\leftarrow$ Reactant
|   +-- TS_pathwayA_opt.xyz              $\leftarrow$ TS ($\Delta$E‡ = 34.1)
|   +-- product_1-5-dimethylpyrazole_opt.xyz
|
+-- path_B/  (N-Me away from S) $\star$ FAVORED $\star$
|   +-- N4-Me_TDSO_correct_opt.xyz      $\leftarrow$ Reactant (CORRECTED, no N-H)
|   +-- TS_pathwayB_correct_opt.xyz      $\leftarrow$ TS ($\Delta$E‡ = 22.6)
|   +-- product_1-3-dimethylpyrazole_neutral_opt.xyz
|
+-- common/
    +-- SO_extrusion_FINAL_corrected.png $\leftarrow$ Energy profile
    +-- (other shared structures)
```

---

Thank you for the patient corrections! The final analysis shows that **N-alkylation away from S (Pathway B) is kinetically favored**, which aligns with the expectation that positioning the N-Me group away from the SO leaving group reduces unfavorable interactions during the extrusion transition state.
\end{markdown}

\end{tcolorbox}
