# Supplementary material for: El Agente Estructural: An Artificially Intelligent Molecular Editor
Source: arXiv:2602.04849 source file (2026-11-30)
Supplement: Supplementary file 3 [file ethylene.tex]

\setlength{\parindent}{5pt} \textbf{\textcolor{blue}{User:}}
\begin{tcolorbox}[
    colback=blue!10,
    colframe=blue,
    width=\textwidth,
    arc=2mm,
    boxrule=0.2mm,
    leftrule=0.2mm, rightrule=0.2mm,
    toprule=0.2mm, bottomrule=0.2mm,
    enhanced,
    breakable
]
\begin{markdown}
You are given an image file, mechanism.png, which depicts a chemical reaction mechanism. Based solely on the information shown in the image, generate three-dimensional molecular structures corresponding to each reaction intermediate and transition state depicted in the mechanism. Generate and save a separate XYZ file for each reaction intermediate and transition state.
\end{markdown}
\end{tcolorbox}
\setlength{\parindent}{5pt} \robot \hspace{2pt} \textbf{Estructural}

\begin{tcolorbox}[
    colback=matterbg2,
    colframe=mattergreen1,
    width=\textwidth,
    arc=2mm,
    boxrule=0.2mm,
    leftrule=0.2mm, rightrule=0.2mm,
    toprule=0.2mm, bottomrule=0.2mm,
    enhanced,
    breakable
]
\textbf{Action:}

\begin{markdown}
I'll start by viewing the mechanism.png image to understand the chemical reaction mechanism depicted and identify all the intermediates and transition states that need to be generated.
\end{markdown}

\textbf{Tool used:}

\setlength{\parindent}{5pt}\underline{\texttt{Tool Name:}} \texttt{view\_png\_file}\par
\setlength{\parindent}{5pt}\underline{\texttt{Arguments:}}\par
\setlength{\parindent}{10pt}\texttt{png\_file\_relative\_path = mechanism.png}\par
\smallskip
\end{tcolorbox}

\setlength{\parindent}{5pt} \robot \hspace{2pt} \textbf{Estructural}

\begin{tcolorbox}[
    colback=matterbg2,
    colframe=mattergreen1,
    width=\textwidth,
    arc=2mm,
    boxrule=0.2mm,
    leftrule=0.2mm, rightrule=0.2mm,
    toprule=0.2mm, bottomrule=0.2mm,
    enhanced,
    breakable
]
\textbf{Action:}

\begin{markdown}
Excellent! I can see this is a **migratory insertion mechanism** involving a zirconocene complex. The mechanism shows:

1. **Intermediate 1 (Left)**: Cp$_2$Zr$^+$(CH$_3$)($\eta$$^2$-ethylene) - Zirconocene cation with a methyl group and coordinated ethylene
2. **Transition State (Middle)**: 4-membered ring transition state showing the migratory insertion process with dashed bonds
3. **Intermediate 2 (Right)**: Cp$_2$Zr$^+$(n-propyl) - Zirconocene cation with a propyl group (product of insertion)

Let me start building these structures. First, let me check what predefined templates and fragments are available for zirconocene complexes.
\end{markdown}

\textbf{Tool used:}

\setlength{\parindent}{5pt}\underline{\texttt{Tool Name:}} \texttt{find\_available\_fragments}\par
\setlength{\parindent}{5pt}\underline{\texttt{Arguments:}}\par
\setlength{\parindent}{10pt}\texttt{type = predefined\_organometallics}\par
\smallskip
\end{tcolorbox}

\setlength{\parindent}{5pt} \robot \hspace{2pt} \textbf{Estructural}

\begin{tcolorbox}[
    colback=matterbg2,
    colframe=mattergreen1,
    width=\textwidth,
    arc=2mm,
    boxrule=0.2mm,
    leftrule=0.2mm, rightrule=0.2mm,
    toprule=0.2mm, bottomrule=0.2mm,
    enhanced,
    breakable
]
\textbf{Action:}

\begin{markdown}
Let me check for available ligands, specifically the cyclopentadienyl (Cp) ligand and other necessary fragments:
\end{markdown}

\textbf{Tool used:}

\setlength{\parindent}{5pt}\underline{\texttt{Tool Name:}} \texttt{find\_available\_fragments}\par
\setlength{\parindent}{5pt}\underline{\texttt{Arguments:}}\par
\setlength{\parindent}{10pt}\texttt{name = Cp}\par
\smallskip
\end{tcolorbox}

\setlength{\parindent}{5pt} \robot \hspace{2pt} \textbf{Estructural}

\begin{tcolorbox}[
    colback=matterbg2,
    colframe=mattergreen1,
    width=\textwidth,
    arc=2mm,
    boxrule=0.2mm,
    leftrule=0.2mm, rightrule=0.2mm,
    toprule=0.2mm, bottomrule=0.2mm,
    enhanced,
    breakable
]
\textbf{Tool used:}

\setlength{\parindent}{5pt}\underline{\texttt{Tool Name:}} \texttt{find\_available\_fragments}\par
\setlength{\parindent}{5pt}\underline{\texttt{Arguments:}}\par
\setlength{\parindent}{10pt}\texttt{name = ethylene}\par
\smallskip
\end{tcolorbox}

\setlength{\parindent}{5pt} \robot \hspace{2pt} \textbf{Estructural}

\begin{tcolorbox}[
    colback=matterbg2,
    colframe=mattergreen1,
    width=\textwidth,
    arc=2mm,
    boxrule=0.2mm,
    leftrule=0.2mm, rightrule=0.2mm,
    toprule=0.2mm, bottomrule=0.2mm,
    enhanced,
    breakable
]
\textbf{Tool used:}

\setlength{\parindent}{5pt}\underline{\texttt{Tool Name:}} \texttt{find\_available\_fragments}\par
\setlength{\parindent}{5pt}\underline{\texttt{Arguments:}}\par
\setlength{\parindent}{10pt}\texttt{name = Me}\par
\smallskip
\end{tcolorbox}

\setlength{\parindent}{5pt} \robot \hspace{2pt} \textbf{Estructural}

\begin{tcolorbox}[
    colback=matterbg2,
    colframe=mattergreen1,
    width=\textwidth,
    arc=2mm,
    boxrule=0.2mm,
    leftrule=0.2mm, rightrule=0.2mm,
    toprule=0.2mm, bottomrule=0.2mm,
    enhanced,
    breakable
]
\textbf{Action:}

\begin{markdown}
Now I have all the information I need. Let me build the three structures systematically.

**Building the structures:**

**Structure 1 - Intermediate 1**: Cp$_2$Zr(CH$_3$)($\eta$$^2$-ethylene)$^+$
**Structure 2 - Transition State**: 4-membered ring TS
**Structure 3 - Intermediate 2**: Cp$_2$Zr(n-propyl)$^+$

Let me start by building **Intermediate 1** using the tetrahedral template with two Cp rings, a methyl group, and an ethylene ligand:
\end{markdown}

\textbf{Tool used:}

\setlength{\parindent}{5pt}\underline{\texttt{Tool Name:}} \texttt{build\_tm\_complex\_from\_template}\par
\setlength{\parindent}{5pt}\underline{\texttt{Arguments:}}\par
\setlength{\parindent}{10pt}\texttt{coordination\_geometry = tetrahedral}\par
\setlength{\parindent}{10pt}\texttt{metal = Zr}\par
\setlength{\parindent}{10pt}\texttt{ligand\_bindings = [\{"Cp": [1, 2]\}, \{"CH3": [3]\}, \{"ethylene": [4]\}]}\par
\setlength{\parindent}{10pt}\texttt{output\_path = intermediate\_1\_Cp2Zr\_CH3\_ethylene.xyz}\par
\smallskip
\end{tcolorbox}

\setlength{\parindent}{5pt} \robot \hspace{2pt} \textbf{Estructural}

\begin{tcolorbox}[
    colback=matterbg2,
    colframe=mattergreen1,
    width=\textwidth,
    arc=2mm,
    boxrule=0.2mm,
    leftrule=0.2mm, rightrule=0.2mm,
    toprule=0.2mm, bottomrule=0.2mm,
    enhanced,
    breakable
]
\textbf{Action:}

\begin{markdown}
Intermediate 1 has been created. Let me visualize it to verify the structure:
\end{markdown}

\textbf{Tool used:}

\setlength{\parindent}{5pt}\underline{\texttt{Tool Name:}} \texttt{view\_molecule}\par
\setlength{\parindent}{5pt}\underline{\texttt{Arguments:}}\par
\setlength{\parindent}{10pt}\texttt{xyz\_file\_relative\_path = intermediate\_1\_Cp2Zr\_CH3\_ethylene.xyz}\par
\setlength{\parindent}{10pt}\texttt{left\_right\_deg = 20}\par
\setlength{\parindent}{10pt}\texttt{up\_down\_deg = 15}\par
\smallskip
\end{tcolorbox}

\setlength{\parindent}{5pt} \robot \hspace{2pt} \textbf{Estructural}

\begin{tcolorbox}[
    colback=matterbg2,
    colframe=mattergreen1,
    width=\textwidth,
    arc=2mm,
    boxrule=0.2mm,
    leftrule=0.2mm, rightrule=0.2mm,
    toprule=0.2mm, bottomrule=0.2mm,
    enhanced,
    breakable
]
\textbf{Action:}

\begin{markdown}
I can see Intermediate 1 with:
- Zr center (index 0)
- Two Cp rings (indices 2-11 and 12-21)
- Methyl group
- Ethylene ligand (C:25, C:26 at top)

Now let me build **Intermediate 2** (the product with propyl group). First, let me check if propyl is available in the fragment library:
\end{markdown}

\textbf{Tool used:}

\setlength{\parindent}{5pt}\underline{\texttt{Tool Name:}} \texttt{find\_available\_fragments}\par
\setlength{\parindent}{5pt}\underline{\texttt{Arguments:}}\par
\setlength{\parindent}{10pt}\texttt{name = propyl}\par
\smallskip
\end{tcolorbox}

\setlength{\parindent}{5pt} \robot \hspace{2pt} \textbf{Estructural}

\begin{tcolorbox}[
    colback=matterbg2,
    colframe=mattergreen1,
    width=\textwidth,
    arc=2mm,
    boxrule=0.2mm,
    leftrule=0.2mm, rightrule=0.2mm,
    toprule=0.2mm, bottomrule=0.2mm,
    enhanced,
    breakable
]
\textbf{Action:}

\begin{markdown}
Excellent! I found the propyl group (nPr). Now let me build **Intermediate 2** (Cp$_2$Zr-propyl):
\end{markdown}

\textbf{Tool used:}

\setlength{\parindent}{5pt}\underline{\texttt{Tool Name:}} \texttt{build\_tm\_complex\_from\_template}\par
\setlength{\parindent}{5pt}\underline{\texttt{Arguments:}}\par
\setlength{\parindent}{10pt}\texttt{coordination\_geometry = trigonal\_planar}\par
\setlength{\parindent}{10pt}\texttt{ligand\_bindings = [\{"Cp": [1, 2]\}, \{"nPr": [3]\}]}\par
\setlength{\parindent}{10pt}\texttt{metal = Zr}\par
\setlength{\parindent}{10pt}\texttt{output\_path = intermediate\_2\_Cp2Zr\_propyl.xyz}\par
\smallskip
\end{tcolorbox}

\setlength{\parindent}{5pt} \robot \hspace{2pt} \textbf{Estructural}

\begin{tcolorbox}[
    colback=matterbg2,
    colframe=mattergreen1,
    width=\textwidth,
    arc=2mm,
    boxrule=0.2mm,
    leftrule=0.2mm, rightrule=0.2mm,
    toprule=0.2mm, bottomrule=0.2mm,
    enhanced,
    breakable
]
\textbf{Action:}

\begin{markdown}
Let me visualize Intermediate 2 to verify it:
\end{markdown}

\textbf{Tool used:}

\setlength{\parindent}{5pt}\underline{\texttt{Tool Name:}} \texttt{view\_molecule}\par
\setlength{\parindent}{5pt}\underline{\texttt{Arguments:}}\par
\setlength{\parindent}{10pt}\texttt{left\_right\_deg = 20}\par
\setlength{\parindent}{10pt}\texttt{up\_down\_deg = 15}\par
\setlength{\parindent}{10pt}\texttt{xyz\_file\_relative\_path = intermediate\_2\_Cp2Zr\_propyl.xyz}\par
\smallskip
\end{tcolorbox}

\setlength{\parindent}{5pt} \robot \hspace{2pt} \textbf{Estructural}

\begin{tcolorbox}[
    colback=matterbg2,
    colframe=mattergreen1,
    width=\textwidth,
    arc=2mm,
    boxrule=0.2mm,
    leftrule=0.2mm, rightrule=0.2mm,
    toprule=0.2mm, bottomrule=0.2mm,
    enhanced,
    breakable
]
\textbf{Action:}

\begin{markdown}
I can see Intermediate 2 with:
- Zr:0 at center
- Two Cp rings (C:2-6 and C:12-16 with their H atoms)
- Propyl group (C:1, C:23, C:24 chain with H atoms)

The propyl appears disconnected visually, but this is common for metal-organic bonds in the viewer. Let me verify the Zr-C bond distance:
\end{markdown}

\textbf{Tool used:}

\setlength{\parindent}{5pt}\underline{\texttt{Tool Name:}} \texttt{get\_distance\_angle\_dihedral}\par
\setlength{\parindent}{5pt}\underline{\texttt{Arguments:}}\par
\setlength{\parindent}{10pt}\texttt{input\_path = intermediate\_2\_Cp2Zr\_propyl.xyz}\par
\setlength{\parindent}{10pt}\texttt{targets = [\{"atom": [0]\}, \{"atom": [1]\}]}\par
\smallskip
\end{tcolorbox}

\setlength{\parindent}{5pt} \robot \hspace{2pt} \textbf{Estructural}

\begin{tcolorbox}[
    colback=matterbg2,
    colframe=mattergreen1,
    width=\textwidth,
    arc=2mm,
    boxrule=0.2mm,
    leftrule=0.2mm, rightrule=0.2mm,
    toprule=0.2mm, bottomrule=0.2mm,
    enhanced,
    breakable
]
\textbf{Action:}

\begin{markdown}
The Zr-C distance is 2.475 Å, which is appropriate for a Zr-C bond. The structure is valid.

Now I need to construct the **Transition State** for the migratory insertion. Let me first analyze the atom connectivity in Intermediate 1 to understand the key atoms involved:
\end{markdown}

\textbf{Tool used:}

\setlength{\parindent}{5pt}\underline{\texttt{Tool Name:}} \texttt{get\_atomic\_neighbors}\par
\setlength{\parindent}{5pt}\underline{\texttt{Arguments:}}\par
\setlength{\parindent}{10pt}\texttt{file\_path = intermediate\_1\_Cp2Zr\_CH3\_ethylene.xyz}\par
\setlength{\parindent}{10pt}\texttt{target = 0}\par
\smallskip
\end{tcolorbox}

\setlength{\parindent}{5pt} \robot \hspace{2pt} \textbf{Estructural}

\begin{tcolorbox}[
    colback=matterbg2,
    colframe=mattergreen1,
    width=\textwidth,
    arc=2mm,
    boxrule=0.2mm,
    leftrule=0.2mm, rightrule=0.2mm,
    toprule=0.2mm, bottomrule=0.2mm,
    enhanced,
    breakable
]
\textbf{Action:}

\begin{markdown}
Let me check the neighbors of the methyl carbon (which should be index 1 based on the bond pair info):
\end{markdown}

\textbf{Tool used:}

\setlength{\parindent}{5pt}\underline{\texttt{Tool Name:}} \texttt{get\_atomic\_neighbors}\par
\setlength{\parindent}{5pt}\underline{\texttt{Arguments:}}\par
\setlength{\parindent}{10pt}\texttt{file\_path = intermediate\_1\_Cp2Zr\_CH3\_ethylene.xyz}\par
\setlength{\parindent}{10pt}\texttt{target = 1}\par
\smallskip
\end{tcolorbox}

\setlength{\parindent}{5pt} \robot \hspace{2pt} \textbf{Estructural}

\begin{tcolorbox}[
    colback=matterbg2,
    colframe=mattergreen1,
    width=\textwidth,
    arc=2mm,
    boxrule=0.2mm,
    leftrule=0.2mm, rightrule=0.2mm,
    toprule=0.2mm, bottomrule=0.2mm,
    enhanced,
    breakable
]
\textbf{Action:}

\begin{markdown}
Now I understand the structure:
- C:1 is the methyl carbon (bonded to Zr:0, H:22, H:23, H:24)
- C:25 and C:26 are the ethylene carbons

Let me check the ethylene carbon neighbors:
\end{markdown}

\textbf{Tool used:}

\setlength{\parindent}{5pt}\underline{\texttt{Tool Name:}} \texttt{get\_atomic\_neighbors}\par
\setlength{\parindent}{5pt}\underline{\texttt{Arguments:}}\par
\setlength{\parindent}{10pt}\texttt{file\_path = intermediate\_1\_Cp2Zr\_CH3\_ethylene.xyz}\par
\setlength{\parindent}{10pt}\texttt{target = 25}\par
\smallskip
\end{tcolorbox}

\setlength{\parindent}{5pt} \robot \hspace{2pt} \textbf{Estructural}

\begin{tcolorbox}[
    colback=matterbg2,
    colframe=mattergreen1,
    width=\textwidth,
    arc=2mm,
    boxrule=0.2mm,
    leftrule=0.2mm, rightrule=0.2mm,
    toprule=0.2mm, bottomrule=0.2mm,
    enhanced,
    breakable
]
\textbf{Tool used:}

\setlength{\parindent}{5pt}\underline{\texttt{Tool Name:}} \texttt{get\_atomic\_neighbors}\par
\setlength{\parindent}{5pt}\underline{\texttt{Arguments:}}\par
\setlength{\parindent}{10pt}\texttt{file\_path = intermediate\_1\_Cp2Zr\_CH3\_ethylene.xyz}\par
\setlength{\parindent}{10pt}\texttt{target = 26}\par
\smallskip
\end{tcolorbox}

\setlength{\parindent}{5pt} \robot \hspace{2pt} \textbf{Estructural}

\begin{tcolorbox}[
    colback=matterbg2,
    colframe=mattergreen1,
    width=\textwidth,
    arc=2mm,
    boxrule=0.2mm,
    leftrule=0.2mm, rightrule=0.2mm,
    toprule=0.2mm, bottomrule=0.2mm,
    enhanced,
    breakable
]
\textbf{Action:}

\begin{markdown}
Now I have a clear picture of the structure:
- C:1 = methyl carbon (bonded to Zr:0)
- C:25 = ethylene carbon 1 (bonded to C:26, H:29, H:30, Zr:0)
- C:26 = ethylene carbon 2 (bonded to C:25, H:27, H:28, Zr:0)

For the **transition state**, I need to create a 4-membered ring: Zr-C25-C26-C1 (or similar). Let me get the current distances to plan the TS geometry:
\end{markdown}

\textbf{Tool used:}

\setlength{\parindent}{5pt}\underline{\texttt{Tool Name:}} \texttt{repl\_tool}\par
\setlength{\parindent}{5pt}\underline{\texttt{Arguments:}}\par
\setlength{\parindent}{10pt}\texttt{code =}\par
\begin{verbatim}

# Get key distances in intermediate_1 for planning the TS
import subprocess

# Read the xyz file to understand the geometry
with open('intermediate_1_Cp2Zr_CH3_ethylene.xyz', 'r') as f:
    content = f.read()
print("Intermediate 1 structure:")
print(content[:2000])

\end{verbatim}\par
\smallskip
\end{tcolorbox}

\setlength{\parindent}{5pt} \robot \hspace{2pt} \textbf{Estructural}

\begin{tcolorbox}[
    colback=matterbg2,
    colframe=mattergreen1,
    width=\textwidth,
    arc=2mm,
    boxrule=0.2mm,
    leftrule=0.2mm, rightrule=0.2mm,
    toprule=0.2mm, bottomrule=0.2mm,
    enhanced,
    breakable
]
\textbf{Action:}

\begin{markdown}
Now let me measure the key distances needed for the TS geometry:
\end{markdown}

\textbf{Tool used:}

\setlength{\parindent}{5pt}\underline{\texttt{Tool Name:}} \texttt{get\_distance\_angle\_dihedral}\par
\setlength{\parindent}{5pt}\underline{\texttt{Arguments:}}\par
\setlength{\parindent}{10pt}\texttt{input\_path = intermediate\_1\_Cp2Zr\_CH3\_ethylene.xyz}\par
\setlength{\parindent}{10pt}\texttt{targets = [\{"atom": [0]\}, \{"atom": [1]\}]}\par
\smallskip
\end{tcolorbox}

\setlength{\parindent}{5pt} \robot \hspace{2pt} \textbf{Estructural}

\begin{tcolorbox}[
    colback=matterbg2,
    colframe=mattergreen1,
    width=\textwidth,
    arc=2mm,
    boxrule=0.2mm,
    leftrule=0.2mm, rightrule=0.2mm,
    toprule=0.2mm, bottomrule=0.2mm,
    enhanced,
    breakable
]
\textbf{Tool used:}

\setlength{\parindent}{5pt}\underline{\texttt{Tool Name:}} \texttt{get\_distance\_angle\_dihedral}\par
\setlength{\parindent}{5pt}\underline{\texttt{Arguments:}}\par
\setlength{\parindent}{10pt}\texttt{input\_path = intermediate\_1\_Cp2Zr\_CH3\_ethylene.xyz}\par
\setlength{\parindent}{10pt}\texttt{targets = [\{"atom": [1]\}, \{"atom": [25]\}]}\par
\smallskip
\end{tcolorbox}

\setlength{\parindent}{5pt} \robot \hspace{2pt} \textbf{Estructural}

\begin{tcolorbox}[
    colback=matterbg2,
    colframe=mattergreen1,
    width=\textwidth,
    arc=2mm,
    boxrule=0.2mm,
    leftrule=0.2mm, rightrule=0.2mm,
    toprule=0.2mm, bottomrule=0.2mm,
    enhanced,
    breakable
]
\textbf{Tool used:}

\setlength{\parindent}{5pt}\underline{\texttt{Tool Name:}} \texttt{get\_distance\_angle\_dihedral}\par
\setlength{\parindent}{5pt}\underline{\texttt{Arguments:}}\par
\setlength{\parindent}{10pt}\texttt{input\_path = intermediate\_1\_Cp2Zr\_CH3\_ethylene.xyz}\par
\setlength{\parindent}{10pt}\texttt{targets = [\{"atom": [1]\}, \{"atom": [26]\}]}\par
\smallskip
\end{tcolorbox}

\setlength{\parindent}{5pt} \robot \hspace{2pt} \textbf{Estructural}

\begin{tcolorbox}[
    colback=matterbg2,
    colframe=mattergreen1,
    width=\textwidth,
    arc=2mm,
    boxrule=0.2mm,
    leftrule=0.2mm, rightrule=0.2mm,
    toprule=0.2mm, bottomrule=0.2mm,
    enhanced,
    breakable
]
\textbf{Tool used:}

\setlength{\parindent}{5pt}\underline{\texttt{Tool Name:}} \texttt{get\_distance\_angle\_dihedral}\par
\setlength{\parindent}{5pt}\underline{\texttt{Arguments:}}\par
\setlength{\parindent}{10pt}\texttt{input\_path = intermediate\_1\_Cp2Zr\_CH3\_ethylene.xyz}\par
\setlength{\parindent}{10pt}\texttt{targets = [\{"atom": [25]\}, \{"atom": [26]\}]}\par
\smallskip
\end{tcolorbox}

\setlength{\parindent}{5pt} \robot \hspace{2pt} \textbf{Estructural}

\begin{tcolorbox}[
    colback=matterbg2,
    colframe=mattergreen1,
    width=\textwidth,
    arc=2mm,
    boxrule=0.2mm,
    leftrule=0.2mm, rightrule=0.2mm,
    toprule=0.2mm, bottomrule=0.2mm,
    enhanced,
    breakable
]
\textbf{Action:}

\begin{markdown}
Now I have all the key distances:
- Zr-C1 (methyl): 2.475 Å
- C1-C25: 4.28 Å
- C1-C26: 3.90 Å  
- C25-C26 (ethylene C=C): 1.33 Å

For the **transition state**, I need to bring the methyl carbon (C1) close to one of the ethylene carbons (C26) while allowing the rest of the structure to relax. I'll use constrained xTB optimization with a C1-C26 distance constraint of ~2.1 Å (typical for a forming C-C bond in TS):
\end{markdown}

\textbf{Tool used:}

\setlength{\parindent}{5pt}\underline{\texttt{Tool Name:}} \texttt{constraint\_xtb}\par
\setlength{\parindent}{5pt}\underline{\texttt{Arguments:}}\par
\setlength{\parindent}{10pt}\texttt{input\_xyz = intermediate\_1\_Cp2Zr\_CH3\_ethylene.xyz}\par
\setlength{\parindent}{10pt}\texttt{output\_xyz = transition\_state\_migratory\_insertion.xyz}\par
\setlength{\parindent}{10pt}\texttt{distance\_constraints = [\{"atoms": [1, 26], "value": 2.1\}]}\par
\setlength{\parindent}{10pt}\texttt{force\_constant = 1.0}\par
\setlength{\parindent}{10pt}\texttt{charge = 1}\par
\setlength{\parindent}{10pt}\texttt{gfn\_method = gfn2}\par
\smallskip
\end{tcolorbox}

\setlength{\parindent}{5pt} \robot \hspace{2pt} \textbf{Estructural}

\begin{tcolorbox}[
    colback=matterbg2,
    colframe=mattergreen1,
    width=\textwidth,
    arc=2mm,
    boxrule=0.2mm,
    leftrule=0.2mm, rightrule=0.2mm,
    toprule=0.2mm, bottomrule=0.2mm,
    enhanced,
    breakable
]
\textbf{Action:}

\begin{markdown}
The transition state structure has been generated. Let me visualize it to verify the 4-membered ring geometry:
\end{markdown}

\textbf{Tool used:}

\setlength{\parindent}{5pt}\underline{\texttt{Tool Name:}} \texttt{view\_molecule}\par
\setlength{\parindent}{5pt}\underline{\texttt{Arguments:}}\par
\setlength{\parindent}{10pt}\texttt{left\_right\_deg = 15}\par
\setlength{\parindent}{10pt}\texttt{up\_down\_deg = 20}\par
\setlength{\parindent}{10pt}\texttt{xyz\_file\_relative\_path = transition\_state\_migratory\_insertion.xyz}\par
\smallskip
\end{tcolorbox}

\setlength{\parindent}{5pt} \robot \hspace{2pt} \textbf{Estructural}

\begin{tcolorbox}[
    colback=matterbg2,
    colframe=mattergreen1,
    width=\textwidth,
    arc=2mm,
    boxrule=0.2mm,
    leftrule=0.2mm, rightrule=0.2mm,
    toprule=0.2mm, bottomrule=0.2mm,
    enhanced,
    breakable
]
\textbf{Action:}

\begin{markdown}
Excellent! The transition state structure shows the characteristic 4-membered ring geometry! I can see:
- Zr:0 at center
- Two Cp rings (top and right)
- The 4-membered ring on the left: C:1 (methyl) - C:26 - C:25 forming the insertion geometry

Let me verify the key distances in the transition state:
\end{markdown}

\textbf{Tool used:}

\setlength{\parindent}{5pt}\underline{\texttt{Tool Name:}} \texttt{get\_distance\_angle\_dihedral}\par
\setlength{\parindent}{5pt}\underline{\texttt{Arguments:}}\par
\setlength{\parindent}{10pt}\texttt{input\_path = transition\_state\_migratory\_insertion.xyz}\par
\setlength{\parindent}{10pt}\texttt{targets = [\{"atom": [1]\}, \{"atom": [26]\}]}\par
\smallskip
\end{tcolorbox}

\setlength{\parindent}{5pt} \robot \hspace{2pt} \textbf{Estructural}

\begin{tcolorbox}[
    colback=matterbg2,
    colframe=mattergreen1,
    width=\textwidth,
    arc=2mm,
    boxrule=0.2mm,
    leftrule=0.2mm, rightrule=0.2mm,
    toprule=0.2mm, bottomrule=0.2mm,
    enhanced,
    breakable
]
\textbf{Action:}

\begin{markdown}
The C1-C26 distance is now 2.09 Å (forming C-C bond). Let me also check the Zr-C distances:
\end{markdown}

\textbf{Tool used:}

\setlength{\parindent}{5pt}\underline{\texttt{Tool Name:}} \texttt{get\_distance\_angle\_dihedral}\par
\setlength{\parindent}{5pt}\underline{\texttt{Arguments:}}\par
\setlength{\parindent}{10pt}\texttt{input\_path = transition\_state\_migratory\_insertion.xyz}\par
\setlength{\parindent}{10pt}\texttt{targets = [\{"atom": [0]\}, \{"atom": [1]\}]}\par
\smallskip
\end{tcolorbox}

\setlength{\parindent}{5pt} \robot \hspace{2pt} \textbf{Estructural}

\begin{tcolorbox}[
    colback=matterbg2,
    colframe=mattergreen1,
    width=\textwidth,
    arc=2mm,
    boxrule=0.2mm,
    leftrule=0.2mm, rightrule=0.2mm,
    toprule=0.2mm, bottomrule=0.2mm,
    enhanced,
    breakable
]
\textbf{Tool used:}

\setlength{\parindent}{5pt}\underline{\texttt{Tool Name:}} \texttt{get\_distance\_angle\_dihedral}\par
\setlength{\parindent}{5pt}\underline{\texttt{Arguments:}}\par
\setlength{\parindent}{10pt}\texttt{input\_path = transition\_state\_migratory\_insertion.xyz}\par
\setlength{\parindent}{10pt}\texttt{targets = [\{"atom": [0]\}, \{"atom": [25]\}]}\par
\smallskip
\end{tcolorbox}

\setlength{\parindent}{5pt} \robot \hspace{2pt} \textbf{Estructural}

\begin{tcolorbox}[
    colback=matterbg2,
    colframe=mattergreen1,
    width=\textwidth,
    arc=2mm,
    boxrule=0.2mm,
    leftrule=0.2mm, rightrule=0.2mm,
    toprule=0.2mm, bottomrule=0.2mm,
    enhanced,
    breakable
]
\textbf{Action:}

\begin{markdown}
The Zr-C25 distance is 2.24 Å (forming new $\sigma$-bond to ethylene carbon).

The transition state shows excellent geometry for migratory insertion:
- **C1-C26**: 2.09 Å (forming C-C bond)
- **Zr-C1**: 2.43 Å (partially breaking Zr-methyl bond)
- **Zr-C25**: 2.24 Å (forming new Zr-C $\sigma$-bond)

Now let me view Intermediate 2 from a better angle to confirm the propyl structure:
\end{markdown}

\textbf{Tool used:}

\setlength{\parindent}{5pt}\underline{\texttt{Tool Name:}} \texttt{view\_molecule}\par
\setlength{\parindent}{5pt}\underline{\texttt{Arguments:}}\par
\setlength{\parindent}{10pt}\texttt{left\_right\_deg = -30}\par
\setlength{\parindent}{10pt}\texttt{up\_down\_deg = 10}\par
\setlength{\parindent}{10pt}\texttt{xyz\_file\_relative\_path = intermediate\_2\_Cp2Zr\_propyl.xyz}\par
\smallskip
\end{tcolorbox}

\setlength{\parindent}{5pt} \robot \hspace{2pt} \textbf{Estructural}

\begin{tcolorbox}[
    colback=matterbg2,
    colframe=mattergreen1,
    width=\textwidth,
    arc=2mm,
    boxrule=0.2mm,
    leftrule=0.2mm, rightrule=0.2mm,
    toprule=0.2mm, bottomrule=0.2mm,
    enhanced,
    breakable
]
\textbf{Action:}

\begin{markdown}
I can clearly see Intermediate 2 with:
- Zr:0 at center
- Two Cp rings (C:12-16 and C:2-6)
- Propyl chain: C:1 (bonded to Zr) $\rightarrow$ C:24 $\rightarrow$ C:27 (terminal CH$_3$)

---

**Summary: Generated XYZ Files for Migratory Insertion Mechanism**

Based on the mechanism image showing olefin insertion into a Zr-C bond, I have successfully generated three 3D molecular structures:

**1. **Intermediate 1** (`intermediate_1_Cp2Zr_CH3_ethylene.xyz`)**
- **Structure**: Cp$_2$Zr$^+$(CH$_3$)($\eta$$^2$-C$_2$H$_4$)
- **Description**: Zirconocene cation with methyl ligand and side-on coordinated ethylene
- **Key features**:
  - Zr-CH$_3$ bond: 2.48 Å
  - $\eta$$^2$-ethylene coordination (both ethylene carbons bonded to Zr)
  - Tetrahedral-like geometry around Zr center

**2. **Transition State** (`transition_state_migratory_insertion.xyz`)**
- **Structure**: 4-membered ring TS for migratory insertion
- **Description**: The methyl group migrates to ethylene while Zr forms a $\sigma$-bond
- **Key TS distances**:
  - C(methyl)-C(ethylene) forming bond: **2.09 Å**
  - Zr-C(methyl) elongating bond: **2.43 Å**
  - Zr-C(ethylene) forming $\sigma$-bond: **2.24 Å**

**3. **Intermediate 2** (`intermediate_2_Cp2Zr_propyl.xyz`)**
- **Structure**: Cp$_2$Zr$^+$(n-C$_3$H$_7$)
- **Description**: Zirconocene cation with n-propyl ligand (product of ethylene insertion)
- **Key features**:
  - Zr-C(propyl) bond: 2.48 Å
  - Propyl chain: -CH$_2$-CH$_2$-CH$_3$ attached to Zr

All three XYZ files have been saved and represent the complete migratory insertion mechanism as depicted in the mechanism.png image.
\end{markdown}

\end{tcolorbox}
