# Supplementary material for: El Agente Estructural: An Artificially Intelligent Molecular Editor
Source: arXiv:2602.04849 source file (2026-11-30)
Supplement: Supplementary file 4 [file ferrocene_scan.tex]

\setlength{\parindent}{5pt} \textbf{\textcolor{blue}{User:}}
\begin{tcolorbox}[
    colback=blue!10,
    colframe=blue,
    width=\textwidth,
    arc=2mm,
    boxrule=0.2mm,
    leftrule=0.2mm, rightrule=0.2mm,
    toprule=0.2mm, bottomrule=0.2mm,
    enhanced,
    breakable
]
\begin{markdown}
Generate an XYZ file for ferrocene. 
Then create and save separate XYZ files for the following structural modifications:
1. Stretch the distance between the Fe atom and one Cp ring from 1.5 Å to 2.5 Å in increments of 0.1 Å, while keeping the other Cp ring fixed.
2. Change the Cp--Fe--Cp angle from 120$^{\circ}$ to 180$^{\circ}$ in increments of 10$^{\circ}$, saving a separate XYZ file for each angle.
\end{markdown}
\end{tcolorbox}
\setlength{\parindent}{5pt} \robot \hspace{2pt} \textbf{Estructural}

\begin{tcolorbox}[
    colback=matterbg2,
    colframe=mattergreen1,
    width=\textwidth,
    arc=2mm,
    boxrule=0.2mm,
    leftrule=0.2mm, rightrule=0.2mm,
    toprule=0.2mm, bottomrule=0.2mm,
    enhanced,
    breakable
]
\textbf{Tool used:}

\setlength{\parindent}{5pt}\underline{\texttt{Tool Name:}} \texttt{find\_available\_fragments}\par
\setlength{\parindent}{5pt}\underline{\texttt{Arguments:}}\par
\setlength{\parindent}{10pt}\texttt{type = predefined\_organometallics}\par
\setlength{\parindent}{10pt}\texttt{name = ferrocene}\par
\smallskip
\end{tcolorbox}

\setlength{\parindent}{5pt} \robot \hspace{2pt} \textbf{Estructural}

\begin{tcolorbox}[
    colback=matterbg2,
    colframe=mattergreen1,
    width=\textwidth,
    arc=2mm,
    boxrule=0.2mm,
    leftrule=0.2mm, rightrule=0.2mm,
    toprule=0.2mm, bottomrule=0.2mm,
    enhanced,
    breakable
]
\textbf{Tool used:}

\setlength{\parindent}{5pt}\underline{\texttt{Tool Name:}} \texttt{build\_tm\_complex\_from\_template}\par
\setlength{\parindent}{5pt}\underline{\texttt{Arguments:}}\par
\setlength{\parindent}{10pt}\texttt{ligand\_bindings = [\{"Cp": [1, 2]\}]}\par
\setlength{\parindent}{10pt}\texttt{metal = Fe}\par
\setlength{\parindent}{10pt}\texttt{coordination\_geometry = linear}\par
\setlength{\parindent}{10pt}\texttt{output\_path = ferrocene\_project/ferrocene.xyz}\par
\smallskip
\end{tcolorbox}

\setlength{\parindent}{5pt} \robot \hspace{2pt} \textbf{Estructural}

\begin{tcolorbox}[
    colback=matterbg2,
    colframe=mattergreen1,
    width=\textwidth,
    arc=2mm,
    boxrule=0.2mm,
    leftrule=0.2mm, rightrule=0.2mm,
    toprule=0.2mm, bottomrule=0.2mm,
    enhanced,
    breakable
]
\textbf{Tool used:}

\setlength{\parindent}{5pt}\underline{\texttt{Tool Name:}} \texttt{repl\_tool}\par
\setlength{\parindent}{5pt}\underline{\texttt{Arguments:}}\par
\setlength{\parindent}{10pt}\texttt{code =}\par
\begin{verbatim}
import os
os.makedirs('ferrocene_project', exist_ok=True)
print('Created directory: ferrocene_project')
\end{verbatim}\par
\smallskip
\end{tcolorbox}

\setlength{\parindent}{5pt} \robot \hspace{2pt} \textbf{Estructural}

\begin{tcolorbox}[
    colback=matterbg2,
    colframe=mattergreen1,
    width=\textwidth,
    arc=2mm,
    boxrule=0.2mm,
    leftrule=0.2mm, rightrule=0.2mm,
    toprule=0.2mm, bottomrule=0.2mm,
    enhanced,
    breakable
]
\textbf{Tool used:}

\setlength{\parindent}{5pt}\underline{\texttt{Tool Name:}} \texttt{build\_tm\_complex\_from\_template}\par
\setlength{\parindent}{5pt}\underline{\texttt{Arguments:}}\par
\setlength{\parindent}{10pt}\texttt{ligand\_bindings = [\{"Cp": [1, 2]\}]}\par
\setlength{\parindent}{10pt}\texttt{metal = Fe}\par
\setlength{\parindent}{10pt}\texttt{coordination\_geometry = linear}\par
\setlength{\parindent}{10pt}\texttt{output\_path = ferrocene\_project/ferrocene.xyz}\par
\smallskip
\end{tcolorbox}

\setlength{\parindent}{5pt} \robot \hspace{2pt} \textbf{Estructural}

\begin{tcolorbox}[
    colback=matterbg2,
    colframe=mattergreen1,
    width=\textwidth,
    arc=2mm,
    boxrule=0.2mm,
    leftrule=0.2mm, rightrule=0.2mm,
    toprule=0.2mm, bottomrule=0.2mm,
    enhanced,
    breakable
]
\textbf{Tool used:}

\setlength{\parindent}{5pt}\underline{\texttt{Tool Name:}} \texttt{repl\_tool}\par
\setlength{\parindent}{5pt}\underline{\texttt{Arguments:}}\par
\setlength{\parindent}{10pt}\texttt{code =}\par
\begin{verbatim}
with open('ferrocene_project/ferrocene.xyz', 'r') as f:
    lines = f.readlines()
    # Skip header (2 lines)
    atoms = lines[2:]
    for i, line in enumerate(atoms):
        print(f"{i}: {line.split()[0]}")
\end{verbatim}\par
\smallskip
\end{tcolorbox}

\setlength{\parindent}{5pt} \robot \hspace{2pt} \textbf{Estructural}

\begin{tcolorbox}[
    colback=matterbg2,
    colframe=mattergreen1,
    width=\textwidth,
    arc=2mm,
    boxrule=0.2mm,
    leftrule=0.2mm, rightrule=0.2mm,
    toprule=0.2mm, bottomrule=0.2mm,
    enhanced,
    breakable
]
\textbf{Tool used:}

\setlength{\parindent}{5pt}\underline{\texttt{Tool Name:}} \texttt{repl\_tool}\par
\setlength{\parindent}{5pt}\underline{\texttt{Arguments:}}\par
\setlength{\parindent}{10pt}\texttt{code =}\par
\begin{verbatim}
import math
import os

def read_xyz(path):
    with open(path, 'r') as f:
        lines = f.readlines()
    atoms = []
    for line in lines[2:]:
        parts = line.split()
        if len(parts) >= 4:
            atoms.append({
                'el': parts[0],
                'x': float(parts[1]),
                'y': float(parts[2]),
                'z': float(parts[3])
            })
    return atoms

def write_xyz(path, atoms):
    with open(path, 'w') as f:
        f.write(str(len(atoms)) + "
")
        f.write("Generated by Agent
")
        for atom in atoms:
            f.write(f"{atom['el']} {atom['x']:.6f} {atom['y']:.6f} {atom['z']:.6f}
")

def get_centroid(atoms, indices):
    cx, cy, cz = 0.0, 0.0, 0.0
    for idx in indices:
        cx += atoms[idx]['x']
        cy += atoms[idx]['y']
        cz += atoms[idx]['z']
    n = len(indices)
    return cx/n, cy/n, cz/n

def vec_sub(a, b): 
    return (a[0]-b[0], a[1]-b[1], a[2]-b[2])

def vec_add(a, b):
    return (a[0]+b[0], a[1]+b[1], a[2]+b[2])

def vec_scale(v, s):
    return (v[0]*s, v[1]*s, v[2]*s)

def vec_norm(v):
    return math.sqrt(v[0]**2 + v[1]**2 + v[2]**2)

def vec_normalize(v):
    n = vec_norm(v)
    if n == 0: return (0,0,0)
    return (v[0]/n, v[1]/n, v[2]/n)

def cross_product(a, b):
    return (a[1]*b[2] - a[2]*b[1],
            a[2]*b[0] - a[0]*b[2],
            a[0]*b[1] - a[1]*b[0])

def rotate_point(point, axis, angle_rad, origin):
    x = point[0] - origin[0]
    y = point[1] - origin[1]
    z = point[2] - origin[2]
    u, v, w = axis
    c = math.cos(angle_rad)
    s = math.sin(angle_rad)
    k_dot_v = u*x + v*y + w*z
    k_cross_v_x = v*z - w*y
    k_cross_v_y = w*x - u*z
    k_cross_v_z = u*y - v*x
    rx = x*c + k_cross_v_x*s + u*k_dot_v*(1-c)
    ry = y*c + k_cross_v_y*s + v*k_dot_v*(1-c)
    rz = z*c + k_cross_v_z*s + w*k_dot_v*(1-c)
    return rx + origin[0], ry + origin[1], rz + origin[2]

base_path = 'ferrocene_project/ferrocene.xyz'
atoms = read_xyz(base_path)

idx_fe = 0
idx_cp1_ring = [1, 2, 3, 4, 5]
idx_cp1_all = list(range(1, 11))
idx_cp2_ring = [11, 12, 13, 14, 15]
idx_cp2_all = list(range(11, 21))

fe_pos = (atoms[idx_fe]['x'], atoms[idx_fe]['y'], atoms[idx_fe]['z'])

# 1. Distance Modification
c1 = get_centroid(atoms, idx_cp1_ring)
v1 = vec_sub(c1, fe_pos)
current_dist = vec_norm(v1)
dir_v1 = vec_normalize(v1)

print(f"Initial Fe-Cp1 Distance: {current_dist:.4f}")

for d_int in range(15, 26):
    d = d_int / 10.0
    shift_val = d - current_dist
    shift_vec = vec_scale(dir_v1, shift_val)
    new_atoms = [a.copy() for a in atoms]
    for idx in idx_cp1_all:
        new_atoms[idx]['x'] += shift_vec[0]
        new_atoms[idx]['y'] += shift_vec[1]
        new_atoms[idx]['z'] += shift_vec[2]
    write_xyz(f'ferrocene_project/ferrocene_dist_{d:.1f}.xyz', new_atoms)
    print(f"Saved dist {d:.1f}")

# 2. Angle Modification
c2 = get_centroid(atoms, idx_cp2_ring)
v2 = vec_sub(c2, fe_pos)
arbitrary = (1.0, 0.0, 0.0)
if abs(vec_normalize(v2)[0]) > 0.9:
    arbitrary = (0.0, 1.0, 0.0)
rot_axis = cross_product(vec_normalize(v2), arbitrary)
rot_axis = vec_normalize(rot_axis)

for angle in range(120, 181, 10):
    rot_rad = math.radians(180 - angle)
    new_atoms = [a.copy() for a in atoms]
    for idx in idx_cp2_all:
        p = (atoms[idx]['x'], atoms[idx]['y'], atoms[idx]['z'])
        np = rotate_point(p, rot_axis, rot_rad, fe_pos)
        new_atoms[idx]['x'] = np[0]
        new_atoms[idx]['y'] = np[1]
        new_atoms[idx]['z'] = np[2]
    write_xyz(f'ferrocene_project/ferrocene_angle_{angle}.xyz', new_atoms)
    print(f"Saved angle {angle}")

\end{verbatim}\par
\smallskip
\end{tcolorbox}

\setlength{\parindent}{5pt} \robot \hspace{2pt} \textbf{Estructural}

\begin{tcolorbox}[
    colback=matterbg2,
    colframe=mattergreen1,
    width=\textwidth,
    arc=2mm,
    boxrule=0.2mm,
    leftrule=0.2mm, rightrule=0.2mm,
    toprule=0.2mm, bottomrule=0.2mm,
    enhanced,
    breakable
]
\textbf{Action:}

\begin{markdown}
The XYZ file for ferrocene has been generated, and the requested structural modifications have been performed. All files are saved in the `ferrocene_project` folder.

****Summary of Actions****

1.  **Ferrocene Generation**:
    *   Constructed the base ferrocene structure (Fe(Cp)$_2$) using a linear template with two cyclopentadienyl (Cp) ligands.
    *   **File**: `ferrocene_project/ferrocene.xyz`
    *   **Identified Indices**: Fe (0), Cp Ring 1 (1--10), Cp Ring 2 (11--20).

2.  **Modification 1: Fe--Cp Distance Scan**
    *   Stretched the distance between the Fe atom and the centroid of one Cp ring from **1.5 Å to 2.5 Å** (increment: 0.1 Å).
    *   **Files**: `ferrocene_dist_1.5.xyz` through `ferrocene_dist_2.5.xyz`.

3.  **Modification 2: Cp--Fe--Cp Angle Scan**
    *   Varied the angle between the two Cp ring centroids and the Fe atom from **120$^{\circ}$ to 180$^{\circ}$** (increment: 10$^{\circ}$).
    *   **Files**: `ferrocene_angle_120.xyz` through `ferrocene_angle_180.xyz`.

All structures are available in the `ferrocene_project` directory.
\end{markdown}

\end{tcolorbox}

\setlength{\parindent}{5pt} \textbf{\textcolor{blue}{User:}}
\begin{tcolorbox}[
    colback=blue!10,
    colframe=blue,
    width=\textwidth,
    arc=2mm,
    boxrule=0.2mm,
    leftrule=0.2mm, rightrule=0.2mm,
    toprule=0.2mm, bottomrule=0.2mm,
    enhanced,
    breakable
]
\begin{markdown}
Why don't you use set\\textunderscore{}distance\\textunderscore{}between\\textunderscore{}fragments or set\\textunderscore{}angle\\textunderscore{}between\\textunderscore{}fragments?
\end{markdown}
\end{tcolorbox}
\setlength{\parindent}{5pt} \robot \hspace{2pt} \textbf{Estructural}

\begin{tcolorbox}[
    colback=matterbg2,
    colframe=mattergreen1,
    width=\textwidth,
    arc=2mm,
    boxrule=0.2mm,
    leftrule=0.2mm, rightrule=0.2mm,
    toprule=0.2mm, bottomrule=0.2mm,
    enhanced,
    breakable
]
\textbf{Action:}

\begin{markdown}
Reasoning: The decision to use a custom Python script via `repl_tool` instead of the specific `set_distance_between_fragments` and `set_angle_between_fragments` tools was driven by **batch processing efficiency** and **environment constraints**.

1.  **Batch Efficiency**: The task required generating a total of 18 distinct XYZ files (11 distance steps and 7 angle steps). The specific geometry tools are designed for single-structure modifications. Using them would have required 18 separate, sequential tool calls (and conversation turns), which is significantly slower and less efficient than a single loop.
2.  **Environment Constraints**: The `repl_tool` allows me to write a Python loop to generate all files in one go, but it **cannot call other agent tools** (like `set_distance...`) from within its code. Therefore, I had to implement the vector mathematics (translation and rotation) directly in the Python script to achieve the "scan" functionality within a single action.
3.  **Simplicity of System**: Ferrocene has a very predictable indexing structure (Fe at 0, Ligands at 1-10 and 11-20). This made it safe to manually define the atom groups in the script. For more complex or unknown molecules where "fragment detection" is difficult, using `set_distance_between_fragments` with `fragment_mode='auto'` would indeed be the safer and preferred choice.

The requested XYZ files were successfully generated in the `ferrocene_project` directory in the previous step using this optimized batch method.

If you would like, I can demonstrate how to use `set_distance_between_fragments` for a single specific adjustment to compare the results.
\end{markdown}

\end{tcolorbox}
