# Supplementary material for: El Agente Estructural: An Artificially Intelligent Molecular Editor
Source: arXiv:2602.04849 source file (2026-11-30)
Supplement: Supplementary file 5 [file heme_analysis.tex]

\setlength{\parindent}{5pt} \textbf{\textcolor{blue}{User:}}
\begin{tcolorbox}[
    colback=blue!10,
    colframe=blue,
    width=\textwidth,
    arc=2mm,
    boxrule=0.2mm,
    leftrule=0.2mm, rightrule=0.2mm,
    toprule=0.2mm, bottomrule=0.2mm,
    enhanced,
    breakable
]
\begin{markdown}
The provided PDB-code-2FRJ.xyz file contains six distinct fragments. 
Identify which atoms belong to each fragment (heme group, lysine, histidine, water, NO ligand, and the histidine fragment coordinated to the heme iron). 
For each fragment, list each atom with its atomic species and atomic index explicitly paired.
\end{markdown}
\end{tcolorbox}
\setlength{\parindent}{5pt} \robot \hspace{2pt} \textbf{Estructural}

\begin{tcolorbox}[
    colback=matterbg2,
    colframe=mattergreen1,
    width=\textwidth,
    arc=2mm,
    boxrule=0.2mm,
    leftrule=0.2mm, rightrule=0.2mm,
    toprule=0.2mm, bottomrule=0.2mm,
    enhanced,
    breakable
]
\textbf{Tool used:}

\setlength{\parindent}{5pt}\underline{\texttt{Tool Name:}} \texttt{repl\_tool}\par
\setlength{\parindent}{5pt}\underline{\texttt{Arguments:}}\par
\setlength{\parindent}{10pt}\texttt{code =}\par
\begin{verbatim}
import os
import shutil
import numpy as np

# 1. Setup Directory
project_dir = "fragment_identification_project"
if not os.path.exists(project_dir):
    os.makedirs(project_dir)

src = "PDB-code-2FRJ.xyz"
dst = os.path.join(project_dir, "PDB-code-2FRJ.xyz")
if os.path.exists(src):
    shutil.copy(src, dst)

# 2. Read XYZ
def read_xyz(filepath):
    atoms = []
    with open(filepath, 'r') as f:
        lines = f.readlines()
        # Skip header if present (standard XYZ has count, then comment)
        start_idx = 2
        try:
            int(lines[0].split()[0])
        except:
            start_idx = 0 # No header?
        
        for i, line in enumerate(lines[start_idx:]):
            parts = line.split()
            if len(parts) >= 4:
                atoms.append({
                    'index': i,
                    'element': parts[0],
                    'coord': np.array([float(x) for x in parts[1:4]])
                })
    return atoms

atoms = read_xyz(dst)

# 3. Connectivity Analysis
# Radii for heuristics (Angstrom) - standard covalent radii approx
radii = {'H': 0.35, 'C': 0.76, 'N': 0.71, 'O': 0.66, 'S': 1.05, 'Fe': 1.32, 'P': 1.07}

def get_radius(el):
    return radii.get(el, 1.0) # default

def is_bonded(a1, a2):
    dist = np.linalg.norm(a1['coord'] - a2['coord'])
    limit = 1.3 * (get_radius(a1['element']) + get_radius(a2['element']))
    return dist < limit

# Build Adjacency List (Excluding Fe to separate ligands)
adj = {i: [] for i in range(len(atoms))}
fe_index = -1

for i in range(len(atoms)):
    if atoms[i]['element'] == 'Fe':
        fe_index = i
        continue # Skip Fe bonds for now
    for j in range(i + 1, len(atoms)):
        if atoms[j]['element'] == 'Fe':
            continue
        if is_bonded(atoms[i], atoms[j]):
            adj[i].append(j)
            adj[j].append(i)

# Find Connected Components (Fragments)
visited = set()
fragments = []

def get_fragment(start_node):
    component = []
    stack = [start_node]
    while stack:
        node = stack.pop()
        if node in visited:
            continue
        visited.add(node)
        component.append(node)
        for neighbor in adj[node]:
            if neighbor not in visited:
                stack.append(neighbor)
    return component

# Iterate
for i in range(len(atoms)):
    if i == fe_index:
        continue # Handle Fe separately
    if i not in visited:
        frag_indices = get_fragment(i)
        fragments.append(frag_indices)

# Analyze Fragments
results = []
for frag in fragments:
    # Get composition
    comp = {}
    atom_list = []
    for idx in frag:
        el = atoms[idx]['element']
        comp[el] = comp.get(el, 0) + 1
        atom_list.append((idx, el))
    
    # Heuristics for identification
    label = "Unknown"
    
    # Heme Porphyrin part: Many C, 4 N. (C20H12N4 approx core)
    if comp.get('N', 0) == 4 and comp.get('C', 0) > 15:
        label = "Heme_Porphyrin_Ring"
    
    # Water: 1 O, maybe 2 H
    elif comp.get('O', 0) >= 1 and sum(comp.values()) <= 3 and comp.get('C', 0) == 0:
        label = "Water"
        
    # NO: 1 N, 1 O
    elif comp.get('N', 0) == 1 and comp.get('O', 0) == 1 and sum(comp.values()) == 2:
        label = "NO_Ligand"
        
    # Amino Acids
    elif comp.get('N', 0) >= 1 and comp.get('C', 0) > 1:
        # Histidine: Imidazole ring (3 C, 2 N in ring) + backbone. Total N approx 3.
        # Lysine: Long chain, 2 N total (backbone + sidechain).
        if comp.get('N', 0) >= 3: # Likely His
             # Check if coordinated to Fe (Distance check)
             # Find closest atom in this fragment to Fe
             min_dist = 100
             if fe_index != -1:
                 fe_pos = atoms[fe_index]['coord']
                 for idx in frag:
                     d = np.linalg.norm(atoms[idx]['coord'] - fe_pos)
                     if d < min_dist:
                         min_dist = d
             
             if min_dist < 2.5: # Typical coordination bond
                 label = "Coordinated_Histidine"
             else:
                 label = "Histidine"
        elif comp.get('N', 0) == 2: # Likely Lysine (or His fragment?)
             # Lysine has long alkyl chain
             label = "Lysine" # Assumption
        else:
             label = "Other_Amino_Acid"
    
    results.append({'label': label, 'indices': frag, 'atoms': atom_list})

# Add Fe to Heme Group
if fe_index != -1:
    # Find the Heme_Porphyrin_Ring fragment
    for res in results:
        if res['label'] == "Heme_Porphyrin_Ring":
            res['indices'].append(fe_index)
            res['atoms'].append((fe_index, 'Fe'))
            res['label'] = "Heme_Group"
            break

# Sort or Organize Output
print(f"Found {len(results)} fragments (excluding Fe initially).")
for r in results:
    print(f"Fragment: {r['label']}")
    # print(f"  Indices: {r['indices']}")
    print(f"  Composition: {str([atoms[i]['element'] for i in r['indices'][:5]])} ... (Total {len(r['indices'])})")

    # Print explicit details for small ones or first few of large ones to confirm
    sorted_atoms = sorted(r['atoms'], key=lambda x: x[0])
    print(f"  Atoms: {sorted_atoms}")

\end{verbatim}\par
\smallskip
\end{tcolorbox}

\setlength{\parindent}{5pt} \robot \hspace{2pt} \textbf{Estructural}

\begin{tcolorbox}[
    colback=matterbg2,
    colframe=mattergreen1,
    width=\textwidth,
    arc=2mm,
    boxrule=0.2mm,
    leftrule=0.2mm, rightrule=0.2mm,
    toprule=0.2mm, bottomrule=0.2mm,
    enhanced,
    breakable
]
\textbf{Tool used:}

\setlength{\parindent}{5pt}\underline{\texttt{Tool Name:}} \texttt{repl\_tool}\par
\setlength{\parindent}{5pt}\underline{\texttt{Arguments:}}\par
\setlength{\parindent}{10pt}\texttt{code =}\par
\begin{verbatim}
import numpy as np

# Data from previous step (manual transcription of indices to be safe, or re-read)
# Indices from previous output:
frag2_indices = [3, 6, 19, 20, 21, 22, 60, 61, 62, 63, 64, 65]
frag3_indices = [4, 5, 15, 16, 17, 18, 44, 45, 46, 47, 48, 49]
fe_index = 0

def read_xyz_simple(filepath):
    coords = {}
    with open(filepath, 'r') as f:
        lines = f.readlines()
        start = 2
        try:
            int(lines[0].split()[0])
        except:
            start=0
        for i, line in enumerate(lines[start:]):
            parts = line.split()
            if len(parts) >= 4:
                coords[i] = np.array([float(x) for x in parts[1:4]])
    return coords

coords = read_xyz_simple("fragment_identification_project/PDB-code-2FRJ.xyz")

fe_pos = coords[fe_index]

def get_min_dist(indices, target_pos):
    dists = []
    for idx in indices:
        d = np.linalg.norm(coords[idx] - target_pos)
        dists.append(d)
    return min(dists)

d2 = get_min_dist(frag2_indices, fe_pos)
d3 = get_min_dist(frag3_indices, fe_pos)

print(f"Distance Frag 2 to Fe: {d2}")
print(f"Distance Frag 3 to Fe: {d3}")

\end{verbatim}\par
\smallskip
\end{tcolorbox}

\setlength{\parindent}{5pt} \robot \hspace{2pt} \textbf{Estructural}

\begin{tcolorbox}[
    colback=matterbg2,
    colframe=mattergreen1,
    width=\textwidth,
    arc=2mm,
    boxrule=0.2mm,
    leftrule=0.2mm, rightrule=0.2mm,
    toprule=0.2mm, bottomrule=0.2mm,
    enhanced,
    breakable
]
\textbf{Action:}

\begin{markdown}
Based on the structural analysis of the `PDB-code-2FRJ.xyz` file, the six distinct fragments have been identified and their constituent atoms are listed below.

The fragments were separated based on connectivity and their chemical identities were confirmed by analyzing their composition and proximity to the iron center.
*   **Heme Group**: Identified as the large porphyrin ring containing the central Iron (Fe) atom.
*   **NO Ligand**: Identified as the diatomic Nitrogen-Oxygen molecule.
*   **Coordinated Histidine**: Identified as the histidine sidechain (imidazole group) positioned within coordination distance (2.18 Å) of the Iron atom.
*   **Histidine**: Identified as the second histidine sidechain, located further (4.36 Å) from the Iron atom.
*   **Lysine**: Identified as the propyl-amine chain fragment.
*   **Water**: Identified as the isolated H2O molecule.

**Fragment Composition List**

**1. Heme Group**
*   **Fe**: 0
*   **N**: 7, 8, 9, 10
*   **C**: 23, 24, 25, 26, 27, 28, 29, 30, 31, 32, 33, 34, 35, 36, 37, 38, 39, 40, 41, 42
*   **H**: 66, 67, 68, 69, 70, 71, 72, 73, 74, 75, 76, 77

**2. NO Ligand**
*   **N**: 1
*   **O**: 2

**3. Histidine Fragment Coordinated to the Heme Iron**
*   **N**: 3, 6
*   **C**: 19, 20, 21, 22
*   **H**: 60, 61, 62, 63, 64, 65

**4. Histidine (Uncoordinated)**
*   **N**: 4, 5
*   **C**: 15, 16, 17, 18
*   **H**: 44, 45, 46, 47, 48, 49

**5. Lysine**
*   **N**: 11
*   **C**: 12, 13, 14
*   **H**: 51, 52, 53, 54, 55, 56, 57, 58, 59, 79

**6. Water**
*   **O**: 43
*   **H**: 50, 78
\end{markdown}

\end{tcolorbox}

\setlength{\parindent}{5pt} \textbf{\textcolor{blue}{User:}}
\begin{tcolorbox}[
    colback=blue!10,
    colframe=blue,
    width=\textwidth,
    arc=2mm,
    boxrule=0.2mm,
    leftrule=0.2mm, rightrule=0.2mm,
    toprule=0.2mm, bottomrule=0.2mm,
    enhanced,
    breakable
]
\begin{markdown}
Which tools do you use? Why don't you use match\\textunderscore{}smarts\\textunderscore{}in\\textunderscore{}xyz or get\\textunderscore{}atomic\\textunderscore{}neighbors? Can you solve the same query by using them?
\end{markdown}
\end{tcolorbox}
\setlength{\parindent}{5pt} \robot \hspace{2pt} \textbf{Estructural}

\begin{tcolorbox}[
    colback=matterbg2,
    colframe=mattergreen1,
    width=\textwidth,
    arc=2mm,
    boxrule=0.2mm,
    leftrule=0.2mm, rightrule=0.2mm,
    toprule=0.2mm, bottomrule=0.2mm,
    enhanced,
    breakable
]
\textbf{Tool used:}

\setlength{\parindent}{5pt}\underline{\texttt{Tool Name:}} \texttt{match\_smarts\_in\_xyz}\par
\setlength{\parindent}{5pt}\underline{\texttt{Arguments:}}\par
\setlength{\parindent}{10pt}\texttt{file\_path = fragment\_identification\_project/PDB-code-2FRJ.xyz}\par
\setlength{\parindent}{10pt}\texttt{smarts = [OH2]}\par
\smallskip
\setlength{\parindent}{5pt}\underline{\texttt{Tool Name:}} \texttt{match\_smarts\_in\_xyz}\par
\setlength{\parindent}{5pt}\underline{\texttt{Arguments:}}\par
\setlength{\parindent}{10pt}\texttt{smarts = N=O}\par
\setlength{\parindent}{10pt}\texttt{file\_path = fragment\_identification\_project/PDB-code-2FRJ.xyz}\par
\smallskip
\setlength{\parindent}{5pt}\underline{\texttt{Tool Name:}} \texttt{match\_smarts\_in\_xyz}\par
\setlength{\parindent}{5pt}\underline{\texttt{Arguments:}}\par
\setlength{\parindent}{10pt}\texttt{smarts = c1ncn[c]1}\par
\setlength{\parindent}{10pt}\texttt{file\_path = fragment\_identification\_project/PDB-code-2FRJ.xyz}\par
\smallskip
\setlength{\parindent}{5pt}\underline{\texttt{Tool Name:}} \texttt{match\_smarts\_in\_xyz}\par
\setlength{\parindent}{5pt}\underline{\texttt{Arguments:}}\par
\setlength{\parindent}{10pt}\texttt{file\_path = fragment\_identification\_project/PDB-code-2FRJ.xyz}\par
\setlength{\parindent}{10pt}\texttt{smarts = n1cccc1}\par
\smallskip
\setlength{\parindent}{5pt}\underline{\texttt{Tool Name:}} \texttt{get\_atomic\_neighbors}\par
\setlength{\parindent}{5pt}\underline{\texttt{Arguments:}}\par
\setlength{\parindent}{10pt}\texttt{target = Fe}\par
\setlength{\parindent}{10pt}\texttt{file\_path = fragment\_identification\_project/PDB-code-2FRJ.xyz}\par
\smallskip
\end{tcolorbox}

\setlength{\parindent}{5pt} \robot \hspace{2pt} \textbf{Estructural}

\begin{tcolorbox}[
    colback=matterbg2,
    colframe=mattergreen1,
    width=\textwidth,
    arc=2mm,
    boxrule=0.2mm,
    leftrule=0.2mm, rightrule=0.2mm,
    toprule=0.2mm, bottomrule=0.2mm,
    enhanced,
    breakable
]
\textbf{Action:}

\begin{markdown}
My primary tool choice was the **Python REPL** to write a **Connectivity-Based Partitioning script**.

I did not use `match_smarts_in_xyz` or `get_atomic_neighbors` as the primary method for the following reasons:

**1. Robustness for Metal Complexes**
**`match_smarts_in_xyz`** relies on OpenBabel to perceive bond orders and aromaticity from raw XYZ coordinates. In transition metal complexes (like Heme), this perception is often fragile:
*   **The Problem:** As demonstrated in my internal test, searching for an imidazole ring (`c1ncn[cH]1`) identified the *uncoordinated* Histidine but **missed** the *coordinated* Histidine. The coordination to Iron changes the bond geometry/perception, causing the standard aromatic pattern to fail.
*   **The Heme Issue:** Similarly, a pyrrole search (`n1cccc1`) only identified 2 of the 4 rings in the porphyrin core due to the delocalized bonding, which OpenBabel often interprets as alternating pyrrole (NH) and pyrrolenine (=N) forms.

**2. "Fragments" vs. "Substructures"**
*   **The Goal:** The task was to **partition** the entire molecule into disjoint fragments (sets of atoms).
*   **The Tool Limitation:** `match_smarts_in_xyz` finds **substructures**.
    *   It would find the "ring" of the histidine but *not* the attached backbone or side chain atoms.
    *   It would find the "core" of the heme but *not* the peripheral substituents.
    *   You would still need a traversal algorithm to "grow" the selection from the matched substructure to the rest of the molecule.

**3. Efficiency**
*   **`get_atomic_neighbors`**: This tool is the functional equivalent of my script's logic (checking connectivity). However, using it via tool calls is inefficient. To identify fragments in a 60+ atom molecule, I would need to call this tool iteratively dozens of times (traversing atom-by-atom), whereas a single Python script can process the entire adjacency matrix in milliseconds.

---

**Can you solve the same query by using them?**
**Yes, but it is much harder and prone to errors.**

You would need a hybrid approach:
1.  **Use `get_atomic_neighbors` on the Metal (Fe)**:
    *   Result: `N:1, N:3, N:7, N:8, N:9, N:10`
    *   This tells us **N:1** is the NO ligand base, **N:3** is the coordinated Histidine base, and **N:7-10** are the Heme bases.
2.  **Use `match_smarts_in_xyz` for isolated fragments**:
    *   `[OH2]` -> Finds Water (O:43).
    *   `N=O` -> Finds NO (N:1, O:2).
    *   `c1ncn[cH]1` -> Finds the uncoordinated Histidine ring.
3.  **Manual Traversal (The "Hard" Part)**:
    *   For the Heme and Coordinated Histidine (which SMARTS missed), you would have to manually call `get_atomic_neighbors` on the atoms found in Step 1 (e.g., neighbors of N:3) and recursively expand until you hit the fragment boundaries.

**Conclusion:** The Python script is the superior method for *blindly* identifying distinct chemical fragments in a complex system, while `match_smarts_in_xyz` is better suited for finding specific, well-defined functional groups in standard organic molecules.
\end{markdown}

\end{tcolorbox}
