# Supplementary material for: El Agente Estructural: An Artificially Intelligent Molecular Editor
Source: arXiv:2602.04849 source file (2026-11-30)
Supplement: Supplementary file 6 [file inorganic_isomer_generation.tex]

\setlength{\parindent}{5pt} \textbf{\textcolor{blue}{User:}}
\begin{tcolorbox}[
    colback=blue!10,
    colframe=blue,
    width=\textwidth,
    arc=2mm,
    boxrule=0.2mm,
    leftrule=0.2mm, rightrule=0.2mm,
    toprule=0.2mm, bottomrule=0.2mm,
    enhanced,
    breakable
]
\begin{markdown}
Generate the following structures with their respective isomers: 1. cisplatin and transplatin 2. $\Delta$-Fe(bpy)3 and $\Lambda$-Fe(bpy)3 3. fac-Ir(ppy)3 and mer-Ir(ppy)3
\end{markdown}
\end{tcolorbox}
\setlength{\parindent}{5pt} \robot \hspace{2pt} \textbf{Estructural}

\begin{tcolorbox}[
    colback=matterbg2,
    colframe=mattergreen1,
    width=\textwidth,
    arc=2mm,
    boxrule=0.2mm,
    leftrule=0.2mm, rightrule=0.2mm,
    toprule=0.2mm, bottomrule=0.2mm,
    enhanced,
    breakable
]
\textbf{Tool used:}

\setlength{\parindent}{5pt}\underline{\texttt{Tool Name:}} \texttt{find\_available\_fragments}\par
\setlength{\parindent}{5pt}\underline{\texttt{Arguments:}}\par
\setlength{\parindent}{10pt}\texttt{type = ligand}\par
\smallskip
\setlength{\parindent}{5pt}\underline{\texttt{Tool Name:}} \texttt{find\_available\_fragments}\par
\setlength{\parindent}{5pt}\underline{\texttt{Arguments:}}\par
\setlength{\parindent}{10pt}\texttt{type = bidentate\_ligand}\par
\smallskip
\end{tcolorbox}

\setlength{\parindent}{5pt} \robot \hspace{2pt} \textbf{Estructural}

\begin{tcolorbox}[
    colback=matterbg2,
    colframe=mattergreen1,
    width=\textwidth,
    arc=2mm,
    boxrule=0.2mm,
    leftrule=0.2mm, rightrule=0.2mm,
    toprule=0.2mm, bottomrule=0.2mm,
    enhanced,
    breakable
]
\textbf{Tool used:}

\setlength{\parindent}{5pt}\underline{\texttt{Tool Name:}} \texttt{repl\_tool}\par
\setlength{\parindent}{5pt}\underline{\texttt{Arguments:}}\par
\setlength{\parindent}{10pt}\texttt{code =}\par
\begin{verbatim}
import os
os.makedirs('isomers_project', exist_ok=True)
print("Directory created")
\end{verbatim}\par
\smallskip
\end{tcolorbox}

\setlength{\parindent}{5pt} \robot \hspace{2pt} \textbf{Estructural}

\begin{tcolorbox}[
    colback=matterbg2,
    colframe=mattergreen1,
    width=\textwidth,
    arc=2mm,
    boxrule=0.2mm,
    leftrule=0.2mm, rightrule=0.2mm,
    toprule=0.2mm, bottomrule=0.2mm,
    enhanced,
    breakable
]
\textbf{Tool used:}

\setlength{\parindent}{5pt}\underline{\texttt{Tool Name:}} \texttt{build\_tm\_complex\_from\_template}\par
\setlength{\parindent}{5pt}\underline{\texttt{Arguments:}}\par
\setlength{\parindent}{10pt}\texttt{ligand\_bindings = [\{"NH3": [1, 2]\}]}\par
\setlength{\parindent}{10pt}\texttt{metal = Pt}\par
\setlength{\parindent}{10pt}\texttt{coordination\_geometry = square\_planar}\par
\setlength{\parindent}{10pt}\texttt{output\_path = isomers\_project/cisplatin.xyz}\par
\smallskip
\setlength{\parindent}{5pt}\underline{\texttt{Tool Name:}} \texttt{build\_tm\_complex\_from\_template}\par
\setlength{\parindent}{5pt}\underline{\texttt{Arguments:}}\par
\setlength{\parindent}{10pt}\texttt{ligand\_bindings = [\{"NH3": [1, 3]\}]}\par
\setlength{\parindent}{10pt}\texttt{output\_path = isomers\_project/transplatin.xyz}\par
\setlength{\parindent}{10pt}\texttt{coordination\_geometry = square\_planar}\par
\setlength{\parindent}{10pt}\texttt{metal = Pt}\par
\smallskip
\setlength{\parindent}{5pt}\underline{\texttt{Tool Name:}} \texttt{build\_tm\_complex\_from\_template}\par
\setlength{\parindent}{5pt}\underline{\texttt{Arguments:}}\par
\setlength{\parindent}{10pt}\texttt{ligand\_bindings = [\{"bpy": [[1, 4], [2, 3], [5, 6]]\}]}\par
\setlength{\parindent}{10pt}\texttt{metal = Fe}\par
\setlength{\parindent}{10pt}\texttt{coordination\_geometry = octahedral}\par
\setlength{\parindent}{10pt}\texttt{output\_path = isomers\_project/delta\_Fe\_bpy3.xyz}\par
\smallskip
\setlength{\parindent}{5pt}\underline{\texttt{Tool Name:}} \texttt{build\_tm\_complex\_from\_template}\par
\setlength{\parindent}{5pt}\underline{\texttt{Arguments:}}\par
\setlength{\parindent}{10pt}\texttt{ligand\_bindings = [\{"bpy": [[1, 5], [2, 6], [3, 4]]\}]}\par
\setlength{\parindent}{10pt}\texttt{metal = Fe}\par
\setlength{\parindent}{10pt}\texttt{coordination\_geometry = octahedral}\par
\setlength{\parindent}{10pt}\texttt{output\_path = isomers\_project/lambda\_Fe\_bpy3.xyz}\par
\smallskip
\setlength{\parindent}{5pt}\underline{\texttt{Tool Name:}} \texttt{build\_tm\_complex\_from\_template}\par
\setlength{\parindent}{5pt}\underline{\texttt{Arguments:}}\par
\setlength{\parindent}{10pt}\texttt{ligand\_bindings = [\{"ppy": [[1, 5], [3, 4], [6, 2]]\}]}\par
\setlength{\parindent}{10pt}\texttt{metal = Ir}\par
\setlength{\parindent}{10pt}\texttt{coordination\_geometry = octahedral}\par
\setlength{\parindent}{10pt}\texttt{output\_path = isomers\_project/fac\_Ir\_ppy3.xyz}\par
\smallskip
\setlength{\parindent}{5pt}\underline{\texttt{Tool Name:}} \texttt{build\_tm\_complex\_from\_template}\par
\setlength{\parindent}{5pt}\underline{\texttt{Arguments:}}\par
\setlength{\parindent}{10pt}\texttt{ligand\_bindings = [\{"ppy": [[1, 5], [3, 4], [2, 6]]\}]}\par
\setlength{\parindent}{10pt}\texttt{metal = Ir}\par
\setlength{\parindent}{10pt}\texttt{coordination\_geometry = octahedral}\par
\setlength{\parindent}{10pt}\texttt{output\_path = isomers\_project/mer\_Ir\_ppy3.xyz}\par
\smallskip
\end{tcolorbox}

\setlength{\parindent}{5pt} \robot \hspace{2pt} \textbf{Estructural}

\begin{tcolorbox}[
    colback=matterbg2,
    colframe=mattergreen1,
    width=\textwidth,
    arc=2mm,
    boxrule=0.2mm,
    leftrule=0.2mm, rightrule=0.2mm,
    toprule=0.2mm, bottomrule=0.2mm,
    enhanced,
    breakable
]
\textbf{Action:}

\begin{markdown}
I have generated the requested structures and their isomers in the `isomers_project` folder.

**1. Cisplatin and Transplatin (Pt(NH3)2Cl2)**
*   **Cisplatin:** `isomers_project/cisplatin.xyz`
    *   Generated using a square planar template with NH3 ligands at cis positions (indices [1, 2]).
*   **Transplatin:** `isomers_project/transplatin.xyz`
    *   Generated using a square planar template with NH3 ligands at trans positions (indices [1, 3]).

**2. $\Delta$-Fe(bpy)3 and $\Lambda$-Fe(bpy)3**
*   **$\Delta$-Fe(bpy)3:** `isomers_project/delta_Fe_bpy3.xyz`
    *   Generated using an octahedral template with 2,2'-bipyridine (bpy) ligands arranged in the Delta ($\Delta$) configuration (indices [[1, 4], [2, 3], [5, 6]]).
*   **$\Lambda$-Fe(bpy)3:** `isomers_project/lambda_Fe_bpy3.xyz`
    *   Generated using an octahedral template with bpy ligands arranged in the Lambda ($\Lambda$) configuration (indices [[1, 5], [2, 6], [3, 4]]).

**3. fac-Ir(ppy)3 and mer-Ir(ppy)3**
*   **fac-Ir(ppy)3:** `isomers_project/fac_Ir_ppy3.xyz`
    *   Generated using an octahedral template with 2-phenylpyridine (ppy) ligands in the facial (fac) arrangement (indices [[1, 5], [3, 4], [6, 2]]).
*   **mer-Ir(ppy)3:** `isomers_project/mer_Ir_ppy3.xyz`
    *   Generated using an octahedral template with ppy ligands in the meridional (mer) arrangement (indices [[1, 5], [3, 4], [2, 6]]).
\end{markdown}

\end{tcolorbox}
