# Supplementary material for: El Agente Estructural: An Artificially Intelligent Molecular Editor
Source: arXiv:2602.04849 source file (2026-11-30)
Supplement: Supplementary file 7 [file ligand_exchange.tex]

\setlength{\parindent}{5pt} \textbf{\textcolor{blue}{User:}}
\begin{tcolorbox}[
    colback=blue!10,
    colframe=blue,
    width=\textwidth,
    arc=2mm,
    boxrule=0.2mm,
    leftrule=0.2mm, rightrule=0.2mm,
    toprule=0.2mm, bottomrule=0.2mm,
    enhanced,
    breakable
]
\begin{markdown}
Given Fe\\textunderscore{}CO\\textunderscore{}6.xyz and Ru\\textunderscore{}bpy\\textunderscore{}2\\textunderscore{}H2O\\textunderscore{}2.xyz:
1. For Fe\\textunderscore{}CO\\textunderscore{}6, replace the two axial CO ligands with water molecules.
2. For Ru\\textunderscore{}bpy\\textunderscore{}2\\textunderscore{}H2O\\textunderscore{}2, replace one water ligand with acetonitrile.
\end{markdown}
\end{tcolorbox}
\setlength{\parindent}{5pt} \robot \hspace{2pt} \textbf{Estructural}

\begin{tcolorbox}[
    colback=matterbg2,
    colframe=mattergreen1,
    width=\textwidth,
    arc=2mm,
    boxrule=0.2mm,
    leftrule=0.2mm, rightrule=0.2mm,
    toprule=0.2mm, bottomrule=0.2mm,
    enhanced,
    breakable
]
\textbf{Tool used:}

\setlength{\parindent}{5pt}\underline{\texttt{Tool Name:}} \texttt{repl\_tool}\par
\setlength{\parindent}{5pt}\underline{\texttt{Arguments:}}\par
\setlength{\parindent}{10pt}\texttt{code =}\par
\begin{verbatim}
import os
import shutil

project_dir = "ligand_exchange_project"
os.makedirs(project_dir, exist_ok=True)

files_to_move = ["Fe_CO_6.xyz", "Ru_bpy_2_H2O_2.xyz"]
for f in files_to_move:
    if os.path.exists(f):
        shutil.move(f, os.path.join(project_dir, f))
        print(f"Moved {f} to {project_dir}")
    else:
        print(f"Warning: {f} not found")

\end{verbatim}\par
\smallskip
\end{tcolorbox}

\setlength{\parindent}{5pt} \robot \hspace{2pt} \textbf{Estructural}

\begin{tcolorbox}[
    colback=matterbg2,
    colframe=mattergreen1,
    width=\textwidth,
    arc=2mm,
    boxrule=0.2mm,
    leftrule=0.2mm, rightrule=0.2mm,
    toprule=0.2mm, bottomrule=0.2mm,
    enhanced,
    breakable
]
\textbf{Tool used:}

\setlength{\parindent}{5pt}\underline{\texttt{Tool Name:}} \texttt{find\_available\_fragments}\par
\setlength{\parindent}{5pt}\underline{\texttt{Arguments:}}\par
\setlength{\parindent}{10pt}\texttt{name = water}\par
\smallskip
\setlength{\parindent}{5pt}\underline{\texttt{Tool Name:}} \texttt{find\_available\_fragments}\par
\setlength{\parindent}{5pt}\underline{\texttt{Arguments:}}\par
\setlength{\parindent}{10pt}\texttt{name = acetonitrile}\par
\smallskip
\setlength{\parindent}{5pt}\underline{\texttt{Tool Name:}} \texttt{get\_atomic\_neighbors}\par
\setlength{\parindent}{5pt}\underline{\texttt{Arguments:}}\par
\setlength{\parindent}{10pt}\texttt{target = Fe}\par
\setlength{\parindent}{10pt}\texttt{file\_path = ligand\_exchange\_project/Fe\_CO\_6.xyz}\par
\smallskip
\end{tcolorbox}

\setlength{\parindent}{5pt} \robot \hspace{2pt} \textbf{Estructural}

\begin{tcolorbox}[
    colback=matterbg2,
    colframe=mattergreen1,
    width=\textwidth,
    arc=2mm,
    boxrule=0.2mm,
    leftrule=0.2mm, rightrule=0.2mm,
    toprule=0.2mm, bottomrule=0.2mm,
    enhanced,
    breakable
]
\textbf{Tool used:}

\setlength{\parindent}{5pt}\underline{\texttt{Tool Name:}} \texttt{repl\_tool}\par
\setlength{\parindent}{5pt}\underline{\texttt{Arguments:}}\par
\setlength{\parindent}{10pt}\texttt{code =}\par
\begin{verbatim}
import math

def calculate_angle(c1, c2, c3):
    # simple angle calculation
    # c2 is the center (Fe)
    v1 = [c1[0]-c2[0], c1[1]-c2[1], c1[2]-c2[2]]
    v2 = [c3[0]-c2[0], c3[1]-c2[1], c3[2]-c2[2]]
    
    dot = v1[0]*v2[0] + v1[1]*v2[1] + v1[2]*v2[2]
    mag1 = math.sqrt(v1[0]**2 + v1[1]**2 + v1[2]**2)
    mag2 = math.sqrt(v2[0]**2 + v2[1]**2 + v2[2]**2)
    
    if mag1 == 0 or mag2 == 0: return 0
    cos_theta = dot / (mag1 * mag2)
    cos_theta = max(min(cos_theta, 1), -1)
    return math.degrees(math.acos(cos_theta))

def read_xyz(path):
    with open(path, 'r') as f:
        lines = f.readlines()
    atoms = []
    for line in lines[2:]:
        parts = line.split()
        if not parts: continue
        atoms.append((parts[0], [float(parts[1]), float(parts[2]), float(parts[3])]))
    return atoms

# Fe_CO_6 analysis
fe_atoms = read_xyz("ligand_exchange_project/Fe_CO_6.xyz")
fe_idx = 0
ligand_indices = [7, 8, 9, 10, 11, 12] # From previous tool output
trans_pair = []

print("Searching for trans pair in Fe_CO_6...")
found = False
for i in range(len(ligand_indices)):
    for j in range(i+1, len(ligand_indices)):
        idx1 = ligand_indices[i]
        idx2 = ligand_indices[j]
        angle = calculate_angle(fe_atoms[idx1][1], fe_atoms[fe_idx][1], fe_atoms[idx2][1])
        if angle > 170: # Tolerance for trans
            print(f"Found trans pair: {idx1} and {idx2} (Angle: {angle:.2f})")
            trans_pair = [idx1, idx2]
            found = True
            break
    if found: break

# Ru analysis
# I need to find Ru index and O neighbors
print("
Analyzing Ru_bpy_2_H2O_2...")
ru_atoms = read_xyz("ligand_exchange_project/Ru_bpy_2_H2O_2.xyz")
ru_idx = -1
o_indices = []

for i, (elem, coords) in enumerate(ru_atoms):
    if elem == "Ru":
        ru_idx = i
        break

if ru_idx != -1:
    print(f"Ru index: {ru_idx}")
    # Find neighbors
    for i, (elem, coords) in enumerate(ru_atoms):
        if i == ru_idx: continue
        dist = math.sqrt(sum([(coords[k]-ru_atoms[ru_idx][1][k])**2 for k in range(3)]))
        if dist < 2.5: # typical bonding distance
             print(f"Neighbor: {i} ({elem}) Dist: {dist:.2f}")
             if elem == "O":
                 o_indices.append(i)
print(f"Water Oxygen indices: {o_indices}")

\end{verbatim}\par
\smallskip
\end{tcolorbox}

\setlength{\parindent}{5pt} \robot \hspace{2pt} \textbf{Estructural}

\begin{tcolorbox}[
    colback=matterbg2,
    colframe=mattergreen1,
    width=\textwidth,
    arc=2mm,
    boxrule=0.2mm,
    leftrule=0.2mm, rightrule=0.2mm,
    toprule=0.2mm, bottomrule=0.2mm,
    enhanced,
    breakable
]
\textbf{Tool used:}

\setlength{\parindent}{5pt}\underline{\texttt{Tool Name:}} \texttt{organic\_molecules\_xyz\_generation}\par
\setlength{\parindent}{5pt}\underline{\texttt{Arguments:}}\par
\setlength{\parindent}{10pt}\texttt{filenames = ["ligand\_exchange\_project/MeCN.xyz"]}\par
\setlength{\parindent}{10pt}\texttt{smiles\_list = ["CC\#N"]}\par
\smallskip
\end{tcolorbox}

\setlength{\parindent}{5pt} \robot \hspace{2pt} \textbf{Estructural}

\begin{tcolorbox}[
    colback=matterbg2,
    colframe=mattergreen1,
    width=\textwidth,
    arc=2mm,
    boxrule=0.2mm,
    leftrule=0.2mm, rightrule=0.2mm,
    toprule=0.2mm, bottomrule=0.2mm,
    enhanced,
    breakable
]
\textbf{Tool used:}

\setlength{\parindent}{5pt}\underline{\texttt{Tool Name:}} \texttt{repl\_tool}\par
\setlength{\parindent}{5pt}\underline{\texttt{Arguments:}}\par
\setlength{\parindent}{10pt}\texttt{code =}\par
\begin{verbatim}
def find_N_index(path):
    with open(path, 'r') as f:
        lines = f.readlines()
    for i, line in enumerate(lines[2:]):
        parts = line.split()
        if not parts: continue
        if parts[0] == 'N':
            print(f"Nitrogen found at index: {i}")
            return i
    return -1

n_idx = find_N_index("ligand_exchange_project/MeCN.xyz")

\end{verbatim}\par
\smallskip
\end{tcolorbox}

\setlength{\parindent}{5pt} \robot \hspace{2pt} \textbf{Estructural}

\begin{tcolorbox}[
    colback=matterbg2,
    colframe=mattergreen1,
    width=\textwidth,
    arc=2mm,
    boxrule=0.2mm,
    leftrule=0.2mm, rightrule=0.2mm,
    toprule=0.2mm, bottomrule=0.2mm,
    enhanced,
    breakable
]
\textbf{Tool used:}

\setlength{\parindent}{5pt}\underline{\texttt{Tool Name:}} \texttt{replace\_branch\_with\_predefined\_FG}\par
\setlength{\parindent}{5pt}\underline{\texttt{Arguments:}}\par
\setlength{\parindent}{10pt}\texttt{output\_path = ligand\_exchange\_project/Fe\_axial\_H2O.xyz}\par
\setlength{\parindent}{10pt}\texttt{FG\_name = H2O}\par
\setlength{\parindent}{10pt}\texttt{bond\_pair = [[0, 7], [0, 12]]}\par
\setlength{\parindent}{10pt}\texttt{core\_file\_path = ligand\_exchange\_project/Fe\_CO\_6.xyz}\par
\smallskip
\setlength{\parindent}{5pt}\underline{\texttt{Tool Name:}} \texttt{replace\_branch}\par
\setlength{\parindent}{5pt}\underline{\texttt{Arguments:}}\par
\setlength{\parindent}{10pt}\texttt{FG\_file\_path = ligand\_exchange\_project/MeCN.xyz}\par
\setlength{\parindent}{10pt}\texttt{output\_path = ligand\_exchange\_project/Ru\_bpy\_2\_H2O\_MeCN.xyz}\par
\setlength{\parindent}{10pt}\texttt{bond\_pair = [[24, 45]]}\par
\setlength{\parindent}{10pt}\texttt{binding\_mode = connect}\par
\setlength{\parindent}{10pt}\texttt{FG\_connection\_idx = 2}\par
\setlength{\parindent}{10pt}\texttt{core\_file\_path = ligand\_exchange\_project/Ru\_bpy\_2\_H2O\_2.xyz}\par
\smallskip
\end{tcolorbox}

\setlength{\parindent}{5pt} \robot \hspace{2pt} \textbf{Estructural}

\begin{tcolorbox}[
    colback=matterbg2,
    colframe=mattergreen1,
    width=\textwidth,
    arc=2mm,
    boxrule=0.2mm,
    leftrule=0.2mm, rightrule=0.2mm,
    toprule=0.2mm, bottomrule=0.2mm,
    enhanced,
    breakable
]
\textbf{Action:}

\begin{markdown}
The requested ligand exchange operations have been successfully completed.

****1. Fe(CO)$_6$ Modification****
- **Objective:** Replace two axial CO ligands with water molecules.
- **Input:** `Fe_CO_6.xyz`
- **Procedure:** 
  - Identified the central Iron (Fe) atom at index 0.
  - Calculated angles between Fe-C bonds to identify the trans (axial) pair of Carbon atoms (indices 7 and 12, angle ~180$^{\circ}$).
  - Used `replace_branch_with_predefined_FG` to substitute the branches at these indices with `H2O` ligands.
- **Output:** `ligand_exchange_project/Fe_axial_H2O.xyz`

****2. Ru(bpy)$_2$(H$_2$O)$_2$ Modification****
- **Objective:** Replace one water ligand with acetonitrile (MeCN).
- **Input:** `Ru_bpy_2_H2O_2.xyz`
- **Procedure:**
  - Identified the central Ruthenium (Ru) atom at index 24.
  - Identified the coordinated Oxygen atoms of the water ligands (indices 45 and 46).
  - Generated an XYZ structure for Acetonitrile (`MeCN.xyz`) from the SMILES string `CC#N` and identified the Nitrogen atom (index 2) as the coordination site.
  - Used `replace_branch` to replace the water ligand at index 45 with the generated MeCN fragment, binding via the Nitrogen atom.
- **Output:** `ligand_exchange_project/Ru_bpy_2_H2O_MeCN.xyz`

All generated files are located in the `ligand_exchange_project` directory.
\end{markdown}

\end{tcolorbox}
