# Supplementary material for: El Agente Estructural: An Artificially Intelligent Molecular Editor
Source: arXiv:2602.04849 source file (2026-11-30)
Supplement: Supplementary file 9 [file stilbene.tex]

\setlength{\parindent}{5pt} \textbf{\textcolor{blue}{User:}}
\begin{tcolorbox}[
    colback=blue!10,
    colframe=blue,
    width=\textwidth,
    arc=2mm,
    boxrule=0.2mm,
    leftrule=0.2mm, rightrule=0.2mm,
    toprule=0.2mm, bottomrule=0.2mm,
    enhanced,
    breakable
]
\begin{markdown}
You are given trans-stilbene.xyz and L-alanine.xyz. 1. Make edits to trans-stilbene.xyz to create its photoisomerization TS and also cis-stilbene. 2. Make edits to L-alanine.xyz to generate its enantiomer.
\end{markdown}
\end{tcolorbox}
\setlength{\parindent}{5pt} \robot \hspace{2pt} \textbf{Estructural}

\begin{tcolorbox}[
    colback=matterbg2,
    colframe=mattergreen1,
    width=\textwidth,
    arc=2mm,
    boxrule=0.2mm,
    leftrule=0.2mm, rightrule=0.2mm,
    toprule=0.2mm, bottomrule=0.2mm,
    enhanced,
    breakable
]
\textbf{Tool used:}

\setlength{\parindent}{5pt}\underline{\texttt{Tool Name:}} \texttt{repl\_tool}\par
\setlength{\parindent}{5pt}\underline{\texttt{Arguments:}}\par
\setlength{\parindent}{10pt}\texttt{code =}\par
\begin{verbatim}
import os
import shutil

project_dir = "isomers_and_enantiomers_project"
os.makedirs(project_dir, exist_ok=True)

shutil.copy("trans-stilbene.xyz", os.path.join(project_dir, "trans-stilbene.xyz"))
shutil.copy("L-alanine.xyz", os.path.join(project_dir, "L-alanine.xyz"))

print(f"Created {project_dir} and copied files.")
\end{verbatim}\par
\smallskip
\end{tcolorbox}

\setlength{\parindent}{5pt} \robot \hspace{2pt} \textbf{Estructural}

\begin{tcolorbox}[
    colback=matterbg2,
    colframe=mattergreen1,
    width=\textwidth,
    arc=2mm,
    boxrule=0.2mm,
    leftrule=0.2mm, rightrule=0.2mm,
    toprule=0.2mm, bottomrule=0.2mm,
    enhanced,
    breakable
]
\textbf{Tool used:}

\setlength{\parindent}{5pt}\underline{\texttt{Tool Name:}} \texttt{match\_smarts\_in\_xyz}\par
\setlength{\parindent}{5pt}\underline{\texttt{Arguments:}}\par
\setlength{\parindent}{10pt}\texttt{file\_path = isomers\_and\_enantiomers\_project/trans-stilbene.xyz}\par
\setlength{\parindent}{10pt}\texttt{smarts = C=C}\par
\smallskip
\setlength{\parindent}{5pt}\underline{\texttt{Tool Name:}} \texttt{match\_smarts\_in\_xyz}\par
\setlength{\parindent}{5pt}\underline{\texttt{Arguments:}}\par
\setlength{\parindent}{10pt}\texttt{file\_path = isomers\_and\_enantiomers\_project/L-alanine.xyz}\par
\setlength{\parindent}{10pt}\texttt{smarts = C(N)(C)C(=O)O}\par
\smallskip
\end{tcolorbox}

\setlength{\parindent}{5pt} \robot \hspace{2pt} \textbf{Estructural}

\begin{tcolorbox}[
    colback=matterbg2,
    colframe=mattergreen1,
    width=\textwidth,
    arc=2mm,
    boxrule=0.2mm,
    leftrule=0.2mm, rightrule=0.2mm,
    toprule=0.2mm, bottomrule=0.2mm,
    enhanced,
    breakable
]
\textbf{Tool used:}

\setlength{\parindent}{5pt}\underline{\texttt{Tool Name:}} \texttt{get\_atomic\_neighbors}\par
\setlength{\parindent}{5pt}\underline{\texttt{Arguments:}}\par
\setlength{\parindent}{10pt}\texttt{target = 2}\par
\setlength{\parindent}{10pt}\texttt{file\_path = isomers\_and\_enantiomers\_project/trans-stilbene.xyz}\par
\smallskip
\setlength{\parindent}{5pt}\underline{\texttt{Tool Name:}} \texttt{get\_atomic\_neighbors}\par
\setlength{\parindent}{5pt}\underline{\texttt{Arguments:}}\par
\setlength{\parindent}{10pt}\texttt{target = 3}\par
\setlength{\parindent}{10pt}\texttt{file\_path = isomers\_and\_enantiomers\_project/trans-stilbene.xyz}\par
\smallskip
\setlength{\parindent}{5pt}\underline{\texttt{Tool Name:}} \texttt{get\_atomic\_neighbors}\par
\setlength{\parindent}{5pt}\underline{\texttt{Arguments:}}\par
\setlength{\parindent}{10pt}\texttt{target = 0}\par
\setlength{\parindent}{10pt}\texttt{file\_path = isomers\_and\_enantiomers\_project/L-alanine.xyz}\par
\smallskip
\end{tcolorbox}

\setlength{\parindent}{5pt} \robot \hspace{2pt} \textbf{Estructural}

\begin{tcolorbox}[
    colback=matterbg2,
    colframe=mattergreen1,
    width=\textwidth,
    arc=2mm,
    boxrule=0.2mm,
    leftrule=0.2mm, rightrule=0.2mm,
    toprule=0.2mm, bottomrule=0.2mm,
    enhanced,
    breakable
]
\textbf{Tool used:}

\setlength{\parindent}{5pt}\underline{\texttt{Tool Name:}} \texttt{repl\_tool}\par
\setlength{\parindent}{5pt}\underline{\texttt{Arguments:}}\par
\setlength{\parindent}{10pt}\texttt{code =}\par
\begin{verbatim}
import json

def parse_neighbors(output_str):
    # This is a dummy parser, I will just print the output in the next step
    pass

print("Checking neighbors for L-alanine atoms 1, 2, 3, 4, 5...")

\end{verbatim}\par
\smallskip
\end{tcolorbox}

\setlength{\parindent}{5pt} \robot \hspace{2pt} \textbf{Estructural}

\begin{tcolorbox}[
    colback=matterbg2,
    colframe=mattergreen1,
    width=\textwidth,
    arc=2mm,
    boxrule=0.2mm,
    leftrule=0.2mm, rightrule=0.2mm,
    toprule=0.2mm, bottomrule=0.2mm,
    enhanced,
    breakable
]
\textbf{Tool used:}

\setlength{\parindent}{5pt}\underline{\texttt{Tool Name:}} \texttt{get\_atomic\_neighbors}\par
\setlength{\parindent}{5pt}\underline{\texttt{Arguments:}}\par
\setlength{\parindent}{10pt}\texttt{target = 5}\par
\setlength{\parindent}{10pt}\texttt{file\_path = isomers\_and\_enantiomers\_project/L-alanine.xyz}\par
\smallskip
\end{tcolorbox}

\setlength{\parindent}{5pt} \robot \hspace{2pt} \textbf{Estructural}

\begin{tcolorbox}[
    colback=matterbg2,
    colframe=mattergreen1,
    width=\textwidth,
    arc=2mm,
    boxrule=0.2mm,
    leftrule=0.2mm, rightrule=0.2mm,
    toprule=0.2mm, bottomrule=0.2mm,
    enhanced,
    breakable
]
\textbf{Tool used:}

\setlength{\parindent}{5pt}\underline{\texttt{Tool Name:}} \texttt{get\_atomic\_neighbors}\par
\setlength{\parindent}{5pt}\underline{\texttt{Arguments:}}\par
\setlength{\parindent}{10pt}\texttt{target = 3}\par
\setlength{\parindent}{10pt}\texttt{file\_path = isomers\_and\_enantiomers\_project/L-alanine.xyz}\par
\smallskip
\end{tcolorbox}

\setlength{\parindent}{5pt} \robot \hspace{2pt} \textbf{Estructural}

\begin{tcolorbox}[
    colback=matterbg2,
    colframe=mattergreen1,
    width=\textwidth,
    arc=2mm,
    boxrule=0.2mm,
    leftrule=0.2mm, rightrule=0.2mm,
    toprule=0.2mm, bottomrule=0.2mm,
    enhanced,
    breakable
]
\textbf{Tool used:}

\setlength{\parindent}{5pt}\underline{\texttt{Tool Name:}} \texttt{set\_dihedral\_between\_fragments}\par
\setlength{\parindent}{5pt}\underline{\texttt{Arguments:}}\par
\setlength{\parindent}{10pt}\texttt{input\_path = isomers\_and\_enantiomers\_project/trans-stilbene.xyz}\par
\setlength{\parindent}{10pt}\texttt{output\_path = isomers\_and\_enantiomers\_project/stilbene\_photoisomerization\_TS.xyz}\par
\setlength{\parindent}{10pt}\texttt{angle = 90}\par
\setlength{\parindent}{10pt}\texttt{consider\_fragments = True}\par
\setlength{\parindent}{10pt}\texttt{atoms\_list = [0, 2, 3, 1]}\par
\smallskip
\setlength{\parindent}{5pt}\underline{\texttt{Tool Name:}} \texttt{set\_dihedral\_between\_fragments}\par
\setlength{\parindent}{5pt}\underline{\texttt{Arguments:}}\par
\setlength{\parindent}{10pt}\texttt{input\_path = isomers\_and\_enantiomers\_project/trans-stilbene.xyz}\par
\setlength{\parindent}{10pt}\texttt{output\_path = isomers\_and\_enantiomers\_project/cis-stilbene.xyz}\par
\setlength{\parindent}{10pt}\texttt{angle = 0}\par
\setlength{\parindent}{10pt}\texttt{consider\_fragments = True}\par
\setlength{\parindent}{10pt}\texttt{atoms\_list = [0, 2, 3, 1]}\par
\smallskip
\setlength{\parindent}{5pt}\underline{\texttt{Tool Name:}} \texttt{rotate\_substituents\_around\_bisector}\par
\setlength{\parindent}{5pt}\underline{\texttt{Arguments:}}\par
\setlength{\parindent}{10pt}\texttt{center\_idx = 3}\par
\setlength{\parindent}{10pt}\texttt{output\_path = isomers\_and\_enantiomers\_project/D-alanine.xyz}\par
\setlength{\parindent}{10pt}\texttt{fragment\_mode = auto}\par
\setlength{\parindent}{10pt}\texttt{base\_vector\_indices = [4, 6]}\par
\setlength{\parindent}{10pt}\texttt{input\_path = isomers\_and\_enantiomers\_project/L-alanine.xyz}\par
\setlength{\parindent}{10pt}\texttt{angle\_deg = 180}\par
\smallskip
\end{tcolorbox}

\setlength{\parindent}{5pt} \robot \hspace{2pt} \textbf{Estructural}

\begin{tcolorbox}[
    colback=matterbg2,
    colframe=mattergreen1,
    width=\textwidth,
    arc=2mm,
    boxrule=0.2mm,
    leftrule=0.2mm, rightrule=0.2mm,
    toprule=0.2mm, bottomrule=0.2mm,
    enhanced,
    breakable
]
\textbf{Action:}

\begin{markdown}
The requested edits have been performed on `trans-stilbene.xyz` and `L-alanine.xyz` to generate the specified isomers and enantiomers. The output files are saved in the `isomers_and_enantiomers_project` directory.

****1. Stilbene Isomerization****
Using `trans-stilbene.xyz` as the starting structure, two new geometries were generated by modifying the C-C=C-C dihedral angle defined by the central double bond (atoms 2 and 3) and their phenyl attachments (atoms 0 and 1).

*   **Photoisomerization Transition State (TS):**
    *   **File:** `isomers_and_enantiomers_project/stilbene_photoisomerization_TS.xyz`
    *   **Method:** The central dihedral angle was set to **90$^{\circ}$** to approximate the perpendicular transition state characteristic of stilbene photoisomerization.

*   **Cis-Stilbene:**
    *   **File:** `isomers_and_enantiomers_project/cis-stilbene.xyz`
    *   **Method:** The central dihedral angle was set to **0$^{\circ}$**, converting the trans isomer (dihedral ~180$^{\circ}$) to the cis configuration.

****2. L-Alanine Enantiomer Generation****
Using `L-alanine.xyz`, the D-alanine enantiomer was created by inverting the configuration at the chiral center.

*   **D-Alanine:**
    *   **File:** `isomers_and_enantiomers_project/D-alanine.xyz`
    *   **Method:** The chiral center was identified at atom **C:3**. Its substituents, the methyl group (C:4) and the alpha-hydrogen (H:6), were swapped by rotating them 180$^{\circ}$ around their bisector axis. This operation inverted the stereocenter from L- to D-alanine.
\end{markdown}

\end{tcolorbox}
