# Supplementary material for: El Agente Estructural: An Artificially Intelligent Molecular Editor
Source: arXiv:2602.04849 source file (2026-11-30)
Supplement: Supplementary file 10 [file sumanene.tex]

\setlength{\parindent}{5pt} \textbf{\textcolor{blue}{User:}}
\begin{tcolorbox}[
    colback=blue!10,
    colframe=blue,
    width=\textwidth,
    arc=2mm,
    boxrule=0.2mm,
    leftrule=0.2mm, rightrule=0.2mm,
    toprule=0.2mm, bottomrule=0.2mm,
    enhanced,
    breakable
]
\begin{markdown}
Build the concave and convex CpRu($\eta$$^6$-sumanene)$^+$ complexes by inspecting the three-dimensional shape of the molecule.
\end{markdown}
\end{tcolorbox}
\setlength{\parindent}{5pt} \robot \hspace{2pt} \textbf{Estructural}

\begin{tcolorbox}[
    colback=matterbg2,
    colframe=mattergreen1,
    width=\textwidth,
    arc=2mm,
    boxrule=0.2mm,
    leftrule=0.2mm, rightrule=0.2mm,
    toprule=0.2mm, bottomrule=0.2mm,
    enhanced,
    breakable
]
\textbf{Action:}

\begin{markdown}
I'll help you build the concave and convex CpRu($\eta$$^6$-sumanene)$^+$ complexes. Sumanene is a bowl-shaped polycyclic aromatic hydrocarbon, so the Ru metal center can coordinate to the central benzene ring from either the inside (concave) or outside (convex) of the bowl.

Let me start by checking available predefined organometallic templates that might be useful for this construction:
\end{markdown}

\textbf{Tool used:}

\setlength{\parindent}{5pt}\underline{\texttt{Tool Name:}} \texttt{find\_available\_fragments}\par
\setlength{\parindent}{5pt}\underline{\texttt{Arguments:}}\par
\setlength{\parindent}{10pt}\texttt{type = predefined\_organometallics}\par
\smallskip
\end{tcolorbox}

\setlength{\parindent}{5pt} \robot \hspace{2pt} \textbf{Estructural}

\begin{tcolorbox}[
    colback=matterbg2,
    colframe=mattergreen1,
    width=\textwidth,
    arc=2mm,
    boxrule=0.2mm,
    leftrule=0.2mm, rightrule=0.2mm,
    toprule=0.2mm, bottomrule=0.2mm,
    enhanced,
    breakable
]
\textbf{Action:}

\begin{markdown}
I can see from the directory that sumanene-related files exist. Let me first view the sumanene structure to understand its 3D bowl shape and identify the central benzene ring for coordination:
\end{markdown}

\textbf{Tool used:}

\setlength{\parindent}{5pt}\underline{\texttt{Tool Name:}} \texttt{view\_molecule}\par
\setlength{\parindent}{5pt}\underline{\texttt{Arguments:}}\par
\setlength{\parindent}{10pt}\texttt{xyz\_file\_relative\_path = sumanene.xyz}\par
\setlength{\parindent}{10pt}\texttt{left\_right\_deg = 0}\par
\setlength{\parindent}{10pt}\texttt{up\_down\_deg = 0}\par
\smallskip
\end{tcolorbox}

\setlength{\parindent}{5pt} \robot \hspace{2pt} \textbf{Estructural}

\begin{tcolorbox}[
    colback=matterbg2,
    colframe=mattergreen1,
    width=\textwidth,
    arc=2mm,
    boxrule=0.2mm,
    leftrule=0.2mm, rightrule=0.2mm,
    toprule=0.2mm, bottomrule=0.2mm,
    enhanced,
    breakable
]
\textbf{Action:}

\begin{markdown}
The sumanene.xyz file doesn't exist yet - I need to create it. Let me look up the SMILES for sumanene:
\end{markdown}

\textbf{Tool used:}

\setlength{\parindent}{5pt}\underline{\texttt{Tool Name:}} \texttt{lookup\_smiles\_from\_name}\par
\setlength{\parindent}{5pt}\underline{\texttt{Arguments:}}\par
\setlength{\parindent}{10pt}\texttt{compound\_name = sumanene}\par
\smallskip
\end{tcolorbox}

\setlength{\parindent}{5pt} \robot \hspace{2pt} \textbf{Estructural}

\begin{tcolorbox}[
    colback=matterbg2,
    colframe=mattergreen1,
    width=\textwidth,
    arc=2mm,
    boxrule=0.2mm,
    leftrule=0.2mm, rightrule=0.2mm,
    toprule=0.2mm, bottomrule=0.2mm,
    enhanced,
    breakable
]
\textbf{Action:}

\begin{markdown}
Excellent! I found the SMILES for sumanene. Now let me generate the 3D structure:
\end{markdown}

\textbf{Tool used:}

\setlength{\parindent}{5pt}\underline{\texttt{Tool Name:}} \texttt{organic\_molecules\_xyz\_generation}\par
\setlength{\parindent}{5pt}\underline{\texttt{Arguments:}}\par
\setlength{\parindent}{10pt}\texttt{smiles\_list = ["C1C2=C3C4=C(CC5=C4C6=C(CC7=C6C3=C1C=C7)C=C5)C=C2"]}\par
\setlength{\parindent}{10pt}\texttt{filenames = ["sumanene.xyz"]}\par
\smallskip
\end{tcolorbox}

\setlength{\parindent}{5pt} \robot \hspace{2pt} \textbf{Estructural}

\begin{tcolorbox}[
    colback=matterbg2,
    colframe=mattergreen1,
    width=\textwidth,
    arc=2mm,
    boxrule=0.2mm,
    leftrule=0.2mm, rightrule=0.2mm,
    toprule=0.2mm, bottomrule=0.2mm,
    enhanced,
    breakable
]
\textbf{Action:}

\begin{markdown}
Now let me view the sumanene structure to understand its 3D bowl shape:
\end{markdown}

\textbf{Tool used:}

\setlength{\parindent}{5pt}\underline{\texttt{Tool Name:}} \texttt{view\_molecule}\par
\setlength{\parindent}{5pt}\underline{\texttt{Arguments:}}\par
\setlength{\parindent}{10pt}\texttt{xyz\_file\_relative\_path = sumanene.xyz}\par
\setlength{\parindent}{10pt}\texttt{left\_right\_deg = 0}\par
\setlength{\parindent}{10pt}\texttt{up\_down\_deg = 0}\par
\smallskip
\end{tcolorbox}

\setlength{\parindent}{5pt} \robot \hspace{2pt} \textbf{Estructural}

\begin{tcolorbox}[
    colback=matterbg2,
    colframe=mattergreen1,
    width=\textwidth,
    arc=2mm,
    boxrule=0.2mm,
    leftrule=0.2mm, rightrule=0.2mm,
    toprule=0.2mm, bottomrule=0.2mm,
    enhanced,
    breakable
]
\textbf{Action:}

\begin{markdown}
I can see the structure from above. Let me rotate it to see the bowl shape from the side:
\end{markdown}

\textbf{Tool used:}

\setlength{\parindent}{5pt}\underline{\texttt{Tool Name:}} \texttt{view\_molecule}\par
\setlength{\parindent}{5pt}\underline{\texttt{Arguments:}}\par
\setlength{\parindent}{10pt}\texttt{xyz\_file\_relative\_path = sumanene.xyz}\par
\setlength{\parindent}{10pt}\texttt{left\_right\_deg = 0}\par
\setlength{\parindent}{10pt}\texttt{up\_down\_deg = 90}\par
\smallskip
\end{tcolorbox}

\setlength{\parindent}{5pt} \robot \hspace{2pt} \textbf{Estructural}

\begin{tcolorbox}[
    colback=matterbg2,
    colframe=mattergreen1,
    width=\textwidth,
    arc=2mm,
    boxrule=0.2mm,
    leftrule=0.2mm, rightrule=0.2mm,
    toprule=0.2mm, bottomrule=0.2mm,
    enhanced,
    breakable
]
\textbf{Action:}

\begin{markdown}
Excellent! Now I can clearly see the **bowl shape** of sumanene:
- The **concave side** (inside the bowl) is at the bottom of the image
- The **convex side** (outside the bowl) is at the top

Now I need to identify the central benzene ring atoms where the Ru will coordinate. Let me match the aromatic ring pattern:
\end{markdown}

\textbf{Tool used:}

\setlength{\parindent}{5pt}\underline{\texttt{Tool Name:}} \texttt{match\_smarts\_in\_xyz}\par
\setlength{\parindent}{5pt}\underline{\texttt{Arguments:}}\par
\setlength{\parindent}{10pt}\texttt{file\_path = sumanene.xyz}\par
\setlength{\parindent}{10pt}\texttt{smarts = c1ccccc1}\par
\smallskip
\end{tcolorbox}

\setlength{\parindent}{5pt} \robot \hspace{2pt} \textbf{Estructural}

\begin{tcolorbox}[
    colback=matterbg2,
    colframe=mattergreen1,
    width=\textwidth,
    arc=2mm,
    boxrule=0.2mm,
    leftrule=0.2mm, rightrule=0.2mm,
    toprule=0.2mm, bottomrule=0.2mm,
    enhanced,
    breakable
]
\textbf{Action:}

\begin{markdown}
I see multiple aromatic rings detected. In sumanene, the central benzene ring is the one at the bottom of the bowl. Let me examine the atom neighbors to identify the central ring accurately:
\end{markdown}

\textbf{Tool used:}

\setlength{\parindent}{5pt}\underline{\texttt{Tool Name:}} \texttt{get\_atomic\_neighbors}\par
\setlength{\parindent}{5pt}\underline{\texttt{Arguments:}}\par
\setlength{\parindent}{10pt}\texttt{file\_path = sumanene.xyz}\par
\setlength{\parindent}{10pt}\texttt{target = 7}\par
\smallskip
\end{tcolorbox}

\setlength{\parindent}{5pt} \robot \hspace{2pt} \textbf{Estructural}

\begin{tcolorbox}[
    colback=matterbg2,
    colframe=mattergreen1,
    width=\textwidth,
    arc=2mm,
    boxrule=0.2mm,
    leftrule=0.2mm, rightrule=0.2mm,
    toprule=0.2mm, bottomrule=0.2mm,
    enhanced,
    breakable
]
\textbf{Tool used:}

\setlength{\parindent}{5pt}\underline{\texttt{Tool Name:}} \texttt{get\_atomic\_neighbors}\par
\setlength{\parindent}{5pt}\underline{\texttt{Arguments:}}\par
\setlength{\parindent}{10pt}\texttt{file\_path = sumanene.xyz}\par
\setlength{\parindent}{10pt}\texttt{target = 8}\par
\smallskip
\end{tcolorbox}

\setlength{\parindent}{5pt} \robot \hspace{2pt} \textbf{Estructural}

\begin{tcolorbox}[
    colback=matterbg2,
    colframe=mattergreen1,
    width=\textwidth,
    arc=2mm,
    boxrule=0.2mm,
    leftrule=0.2mm, rightrule=0.2mm,
    toprule=0.2mm, bottomrule=0.2mm,
    enhanced,
    breakable
]
\textbf{Action:}

\begin{markdown}
Let me check a few more atoms to confirm the central benzene ring:
\end{markdown}

\textbf{Tool used:}

\setlength{\parindent}{5pt}\underline{\texttt{Tool Name:}} \texttt{get\_atomic\_neighbors}\par
\setlength{\parindent}{5pt}\underline{\texttt{Arguments:}}\par
\setlength{\parindent}{10pt}\texttt{file\_path = sumanene.xyz}\par
\setlength{\parindent}{10pt}\texttt{target = 3}\par
\smallskip
\end{tcolorbox}

\setlength{\parindent}{5pt} \robot \hspace{2pt} \textbf{Estructural}

\begin{tcolorbox}[
    colback=matterbg2,
    colframe=mattergreen1,
    width=\textwidth,
    arc=2mm,
    boxrule=0.2mm,
    leftrule=0.2mm, rightrule=0.2mm,
    toprule=0.2mm, bottomrule=0.2mm,
    enhanced,
    breakable
]
\textbf{Tool used:}

\setlength{\parindent}{5pt}\underline{\texttt{Tool Name:}} \texttt{get\_atomic\_neighbors}\par
\setlength{\parindent}{5pt}\underline{\texttt{Arguments:}}\par
\setlength{\parindent}{10pt}\texttt{file\_path = sumanene.xyz}\par
\setlength{\parindent}{10pt}\texttt{target = 12}\par
\smallskip
\end{tcolorbox}

\setlength{\parindent}{5pt} \robot \hspace{2pt} \textbf{Estructural}

\begin{tcolorbox}[
    colback=matterbg2,
    colframe=mattergreen1,
    width=\textwidth,
    arc=2mm,
    boxrule=0.2mm,
    leftrule=0.2mm, rightrule=0.2mm,
    toprule=0.2mm, bottomrule=0.2mm,
    enhanced,
    breakable
]
\textbf{Action:}

\begin{markdown}
Let me check which atoms are the CH$_2$ groups (sp$^3$ carbons) to identify the central benzene ring more clearly:
\end{markdown}

\textbf{Tool used:}

\setlength{\parindent}{5pt}\underline{\texttt{Tool Name:}} \texttt{repl\_tool}\par
\setlength{\parindent}{5pt}\underline{\texttt{Arguments:}}\par
\setlength{\parindent}{10pt}\texttt{code =}\par
\begin{verbatim}

# Read sumanene.xyz and analyze the structure
with open('sumanene.xyz', 'r') as f:
    lines = f.readlines()

n_atoms = int(lines[0].strip())
print(f"Total atoms: {n_atoms}")

atoms = []
for i, line in enumerate(lines[2:2+n_atoms]):
    parts = line.split()
    element = parts[0]
    x, y, z = float(parts[1]), float(parts[2]), float(parts[3])
    atoms.append((i, element, x, y, z))
    print(f"Index {i}: {element} at ({x:.3f}, {y:.3f}, {z:.3f})")

\end{verbatim}\par
\smallskip
\end{tcolorbox}

\setlength{\parindent}{5pt} \robot \hspace{2pt} \textbf{Estructural}

\begin{tcolorbox}[
    colback=matterbg2,
    colframe=mattergreen1,
    width=\textwidth,
    arc=2mm,
    boxrule=0.2mm,
    leftrule=0.2mm, rightrule=0.2mm,
    toprule=0.2mm, bottomrule=0.2mm,
    enhanced,
    breakable
]
\textbf{Action:}

\begin{markdown}
Now I can see the structure clearly. The atoms with the highest z-coordinates (around z $\approx$ 1.0-1.2) form the **central benzene ring**: atoms **2, 3, 7, 8, 12, 13**. The CH$_2$ groups (atoms 0, 5, 10) have lower z values, indicating the bowl opens downward.

Therefore:
- **Convex binding**: Ru approaches from above (z > 1.06) - outside the bowl
- **Concave binding**: Ru approaches from below (z < 1.06) - inside the bowl

Let me check available Cp ligand in the fragment library:
\end{markdown}

\textbf{Tool used:}

\setlength{\parindent}{5pt}\underline{\texttt{Tool Name:}} \texttt{find\_available\_fragments}\par
\setlength{\parindent}{5pt}\underline{\texttt{Arguments:}}\par
\setlength{\parindent}{10pt}\texttt{name = Cp}\par
\smallskip
\end{tcolorbox}

\setlength{\parindent}{5pt} \robot \hspace{2pt} \textbf{Estructural}

\begin{tcolorbox}[
    colback=matterbg2,
    colframe=mattergreen1,
    width=\textwidth,
    arc=2mm,
    boxrule=0.2mm,
    leftrule=0.2mm, rightrule=0.2mm,
    toprule=0.2mm, bottomrule=0.2mm,
    enhanced,
    breakable
]
\textbf{Action:}

\begin{markdown}
The Cp ligand is available. Now let me build the complexes step by step.

**Step 1**: First, I'll place a Ru atom at the centroid of the central benzene ring (atoms 2, 3, 7, 8, 12, 13):
\end{markdown}

\textbf{Tool used:}

\setlength{\parindent}{5pt}\underline{\texttt{Tool Name:}} \texttt{insert\_atom\_at\_centroid}\par
\setlength{\parindent}{5pt}\underline{\texttt{Arguments:}}\par
\setlength{\parindent}{10pt}\texttt{core\_file\_path = sumanene.xyz}\par
\setlength{\parindent}{10pt}\texttt{element = Ru}\par
\setlength{\parindent}{10pt}\texttt{centroid\_atom\_indices = [2, 3, 7, 8, 12, 13]}\par
\setlength{\parindent}{10pt}\texttt{output\_path = sumanene\_Ru\_center.xyz}\par
\smallskip
\end{tcolorbox}

\setlength{\parindent}{5pt} \robot \hspace{2pt} \textbf{Estructural}

\begin{tcolorbox}[
    colback=matterbg2,
    colframe=mattergreen1,
    width=\textwidth,
    arc=2mm,
    boxrule=0.2mm,
    leftrule=0.2mm, rightrule=0.2mm,
    toprule=0.2mm, bottomrule=0.2mm,
    enhanced,
    breakable
]
\textbf{Action:}

\begin{markdown}
Ru is now at the centroid of the central benzene ring. Let me view this intermediate structure:
\end{markdown}

\textbf{Tool used:}

\setlength{\parindent}{5pt}\underline{\texttt{Tool Name:}} \texttt{view\_molecule}\par
\setlength{\parindent}{5pt}\underline{\texttt{Arguments:}}\par
\setlength{\parindent}{10pt}\texttt{xyz\_file\_relative\_path = sumanene\_Ru\_center.xyz}\par
\setlength{\parindent}{10pt}\texttt{left\_right\_deg = 0}\par
\setlength{\parindent}{10pt}\texttt{up\_down\_deg = 90}\par
\smallskip
\end{tcolorbox}

\setlength{\parindent}{5pt} \robot \hspace{2pt} \textbf{Estructural}

\begin{tcolorbox}[
    colback=matterbg2,
    colframe=mattergreen1,
    width=\textwidth,
    arc=2mm,
    boxrule=0.2mm,
    leftrule=0.2mm, rightrule=0.2mm,
    toprule=0.2mm, bottomrule=0.2mm,
    enhanced,
    breakable
]
\textbf{Action:}

\begin{markdown}
I can see the bowl shape clearly. The Ru is currently at the centroid (in the plane of the central ring). For proper $\eta$$^6$ coordination, I need to position Ru about 1.65-1.70 Å away from the ring plane.

Looking at the geometry:
- The bowl opens **upward** in the image
- **Convex** binding: Ru below the central ring (outside the bowl)
- **Concave** binding: Ru above the central ring (inside the bowl)

Let me calculate the positions and build both complexes. First, let me check the Ru position and move it appropriately:
\end{markdown}

\textbf{Tool used:}

\setlength{\parindent}{5pt}\underline{\texttt{Tool Name:}} \texttt{repl\_tool}\par
\setlength{\parindent}{5pt}\underline{\texttt{Arguments:}}\par
\setlength{\parindent}{10pt}\texttt{code =}\par
\begin{verbatim}

import numpy as np

# Read the structure with Ru at centroid
with open('sumanene_Ru_center.xyz', 'r') as f:
    lines = f.readlines()

n_atoms = int(lines[0].strip())
atoms = []
for i, line in enumerate(lines[2:2+n_atoms]):
    parts = line.split()
    element = parts[0]
    x, y, z = float(parts[1]), float(parts[2]), float(parts[3])
    atoms.append((element, np.array([x, y, z])))

# Central benzene ring indices in original sumanene: 2, 3, 7, 8, 12, 13
# After adding Ru (index 33), these indices remain the same
central_ring_indices = [2, 3, 7, 8, 12, 13]

# Calculate centroid and normal vector of the central benzene ring
ring_coords = np.array([atoms[i][1] for i in central_ring_indices])
centroid = np.mean(ring_coords, axis=0)
print(f"Central ring centroid: {centroid}")

# Calculate normal vector using two vectors in the plane
v1 = ring_coords[1] - ring_coords[0]
v2 = ring_coords[2] - ring_coords[0]
normal = np.cross(v1, v2)
normal = normal / np.linalg.norm(normal)
print(f"Normal vector: {normal}")

# Ru position (index 33)
ru_pos = atoms[33][1]
print(f"Current Ru position: {ru_pos}")

# For $\eta$$^6$ coordination, Ru should be ~1.7 Å from the ring plane
ru_distance = 1.70  # Å

# Convex position: Ru on the outside of the bowl (opposite to bowl opening)
# Concave position: Ru on the inside of the bowl

# Determine bowl direction by checking where CH2 groups are relative to central ring
# CH2 groups: atoms 0, 5, 10 in original (same indices in new file)
ch2_centroid = np.mean([atoms[0][1], atoms[5][1], atoms[10][1]], axis=0)
print(f"CH2 centroid: {ch2_centroid}")

# Vector from ring centroid to CH2 centroid points into the bowl (concave direction)
bowl_direction = ch2_centroid - centroid
bowl_direction_z = bowl_direction[2]
print(f"Bowl opens toward z: {bowl_direction_z} (negative = down, positive = up)")

# Normal vector should point in one of two directions
# Let's make sure it points AWAY from the bowl (convex direction)
if np.dot(normal, bowl_direction) > 0:
    normal = -normal  # Flip so it points away from bowl

print(f"Normal pointing to convex (outside) direction: {normal}")

# Convex position: centroid - normal * distance
convex_ru_pos = centroid - normal * ru_distance
print(f"Convex Ru position: {convex_ru_pos}")

# Concave position: centroid + normal * distance (into the bowl)
concave_ru_pos = centroid + normal * ru_distance
print(f"Concave Ru position: {concave_ru_pos}")

\end{verbatim}\par
\smallskip
\end{tcolorbox}

\setlength{\parindent}{5pt} \robot \hspace{2pt} \textbf{Estructural}

\begin{tcolorbox}[
    colback=matterbg2,
    colframe=mattergreen1,
    width=\textwidth,
    arc=2mm,
    boxrule=0.2mm,
    leftrule=0.2mm, rightrule=0.2mm,
    toprule=0.2mm, bottomrule=0.2mm,
    enhanced,
    breakable
]
\textbf{Action:}

\begin{markdown}
Now I have the correct positions:
- **Convex Ru**: [0.026, 0.045, -0.639] (outside the bowl)
- **Concave Ru**: [-0.111, -0.193, 2.75] (inside the bowl)

Let me build both isomers. First, I'll create the convex isomer by moving Ru to its proper position:
\end{markdown}

\textbf{Tool used:}

\setlength{\parindent}{5pt}\underline{\texttt{Tool Name:}} \texttt{repl\_tool}\par
\setlength{\parindent}{5pt}\underline{\texttt{Arguments:}}\par
\setlength{\parindent}{10pt}\texttt{code =}\par
\begin{verbatim}

import numpy as np

# Read the structure
with open('sumanene_Ru_center.xyz', 'r') as f:
    lines = f.readlines()

n_atoms = int(lines[0].strip())

# Convex Ru position (outside the bowl)
convex_ru_pos = np.array([0.02572911, 0.04484847, -0.6389134])

# Create new file with Ru at convex position
new_lines = lines[:2]  # Keep header
for i, line in enumerate(lines[2:2+n_atoms]):
    parts = line.split()
    element = parts[0]
    if i == 33:  # Ru atom
        new_lines.append(f"{element}    {convex_ru_pos[0]:.8f}    {convex_ru_pos[1]:.8f}    {convex_ru_pos[2]:.8f}
")
    else:
        new_lines.append(line)

with open('sumanene_Ru_convex.xyz', 'w') as f:
    f.writelines(new_lines)

print("Created sumanene_Ru_convex.xyz with Ru outside the bowl")

# Concave Ru position (inside the bowl)
concave_ru_pos = np.array([-0.11073344, -0.19302213, 2.75000907])

# Create new file with Ru at concave position
new_lines = lines[:2]  # Keep header
for i, line in enumerate(lines[2:2+n_atoms]):
    parts = line.split()
    element = parts[0]
    if i == 33:  # Ru atom
        new_lines.append(f"{element}    {concave_ru_pos[0]:.8f}    {concave_ru_pos[1]:.8f}    {concave_ru_pos[2]:.8f}
")
    else:
        new_lines.append(line)

with open('sumanene_Ru_concave.xyz', 'w') as f:
    f.writelines(new_lines)

print("Created sumanene_Ru_concave.xyz with Ru inside the bowl")

\end{verbatim}\par
\smallskip
\end{tcolorbox}

\setlength{\parindent}{5pt} \robot \hspace{2pt} \textbf{Estructural}

\begin{tcolorbox}[
    colback=matterbg2,
    colframe=mattergreen1,
    width=\textwidth,
    arc=2mm,
    boxrule=0.2mm,
    leftrule=0.2mm, rightrule=0.2mm,
    toprule=0.2mm, bottomrule=0.2mm,
    enhanced,
    breakable
]
\textbf{Action:}

\begin{markdown}
I've created intermediate structures with Ru positioned correctly. Let me verify the convex structure:
\end{markdown}

\textbf{Tool used:}

\setlength{\parindent}{5pt}\underline{\texttt{Tool Name:}} \texttt{view\_molecule}\par
\setlength{\parindent}{5pt}\underline{\texttt{Arguments:}}\par
\setlength{\parindent}{10pt}\texttt{xyz\_file\_relative\_path = sumanene\_Ru\_convex.xyz}\par
\setlength{\parindent}{10pt}\texttt{left\_right\_deg = 0}\par
\setlength{\parindent}{10pt}\texttt{up\_down\_deg = 90}\par
\smallskip
\end{tcolorbox}

\setlength{\parindent}{5pt} \robot \hspace{2pt} \textbf{Estructural}

\begin{tcolorbox}[
    colback=matterbg2,
    colframe=mattergreen1,
    width=\textwidth,
    arc=2mm,
    boxrule=0.2mm,
    leftrule=0.2mm, rightrule=0.2mm,
    toprule=0.2mm, bottomrule=0.2mm,
    enhanced,
    breakable
]
\textbf{Action:}

\begin{markdown}
I notice there might be some confusion in the orientation. Let me view from the default angle to better understand the 3D positions:
\end{markdown}

\textbf{Tool used:}

\setlength{\parindent}{5pt}\underline{\texttt{Tool Name:}} \texttt{view\_molecule}\par
\setlength{\parindent}{5pt}\underline{\texttt{Arguments:}}\par
\setlength{\parindent}{10pt}\texttt{xyz\_file\_relative\_path = sumanene\_Ru\_convex.xyz}\par
\setlength{\parindent}{10pt}\texttt{left\_right\_deg = 0}\par
\setlength{\parindent}{10pt}\texttt{up\_down\_deg = 0}\par
\smallskip
\end{tcolorbox}

\setlength{\parindent}{5pt} \robot \hspace{2pt} \textbf{Estructural}

\begin{tcolorbox}[
    colback=matterbg2,
    colframe=mattergreen1,
    width=\textwidth,
    arc=2mm,
    boxrule=0.2mm,
    leftrule=0.2mm, rightrule=0.2mm,
    toprule=0.2mm, bottomrule=0.2mm,
    enhanced,
    breakable
]
\textbf{Action:}

\begin{markdown}
I can see the structure now. Looking at the image:
- The Ru:33 (teal atom) is positioned at the top of the bowl
- The central benzene ring (C:8, C:12, C:7, C:3) is at the bottom
- The bowl opens upward with the peripheral rings curving up

Based on the bowl orientation analysis:
- **Concave (inside the bowl)**: toward negative z (below the central ring)
- **Convex (outside the bowl)**: toward positive z (above the central ring)

I realize my labels were swapped! Let me correct them and also check the concave structure:
\end{markdown}

\textbf{Tool used:}

\setlength{\parindent}{5pt}\underline{\texttt{Tool Name:}} \texttt{view\_molecule}\par
\setlength{\parindent}{5pt}\underline{\texttt{Arguments:}}\par
\setlength{\parindent}{10pt}\texttt{xyz\_file\_relative\_path = sumanene\_Ru\_concave.xyz}\par
\setlength{\parindent}{10pt}\texttt{left\_right\_deg = 0}\par
\setlength{\parindent}{10pt}\texttt{up\_down\_deg = 0}\par
\smallskip
\end{tcolorbox}

\setlength{\parindent}{5pt} \robot \hspace{2pt} \textbf{Estructural}

\begin{tcolorbox}[
    colback=matterbg2,
    colframe=mattergreen1,
    width=\textwidth,
    arc=2mm,
    boxrule=0.2mm,
    leftrule=0.2mm, rightrule=0.2mm,
    toprule=0.2mm, bottomrule=0.2mm,
    enhanced,
    breakable
]
\textbf{Action:}

\begin{markdown}
Looking at the structure from this angle:
- In `sumanene_Ru_concave.xyz`: Ru is clearly positioned inside the bowl cavity - this is the **concave** isomer $\checkmark$
- In `sumanene_Ru_convex.xyz`: Ru should be on the outer surface of the bowl - this is the **convex** isomer $\checkmark$

It seems my labels got corrected during the calculation. Let me verify by checking the side view of sumanene\\textunderscore{}Ru\\textunderscore{}concave.xyz:
\end{markdown}

\textbf{Tool used:}

\setlength{\parindent}{5pt}\underline{\texttt{Tool Name:}} \texttt{view\_molecule}\par
\setlength{\parindent}{5pt}\underline{\texttt{Arguments:}}\par
\setlength{\parindent}{10pt}\texttt{xyz\_file\_relative\_path = sumanene\_Ru\_concave.xyz}\par
\setlength{\parindent}{10pt}\texttt{left\_right\_deg = 0}\par
\setlength{\parindent}{10pt}\texttt{up\_down\_deg = 90}\par
\smallskip
\end{tcolorbox}

\setlength{\parindent}{5pt} \robot \hspace{2pt} \textbf{Estructural}

\begin{tcolorbox}[
    colback=matterbg2,
    colframe=mattergreen1,
    width=\textwidth,
    arc=2mm,
    boxrule=0.2mm,
    leftrule=0.2mm, rightrule=0.2mm,
    toprule=0.2mm, bottomrule=0.2mm,
    enhanced,
    breakable
]
\textbf{Action:}

\begin{markdown}
Excellent! Now I can see clearly from the side view:
- The bowl opens **upward** 
- In `sumanene_Ru_concave.xyz`, the Ru:33 is positioned **below** the central ring (C:8, C:12, C:7, C:3)
- The CH$_2$ groups and peripheral rings are at the **top** (inside the bowl)

I now realize there's a label swap issue. Let me correct this based on the bowl geometry:
- Ru BELOW the central ring (closer to the outer surface) = **CONVEX**
- Ru ABOVE the central ring (inside the bowl cavity) = **CONCAVE**

Let me properly analyze and fix the structures:
\end{markdown}

\textbf{Tool used:}

\setlength{\parindent}{5pt}\underline{\texttt{Tool Name:}} \texttt{repl\_tool}\par
\setlength{\parindent}{5pt}\underline{\texttt{Arguments:}}\par
\setlength{\parindent}{10pt}\texttt{code =}\par
\begin{verbatim}

import numpy as np

# Read the sumanene_Ru_concave.xyz file to check Ru position
with open('sumanene_Ru_concave.xyz', 'r') as f:
    lines = f.readlines()
    
# Find Ru position
for i, line in enumerate(lines[2:]):
    parts = line.split()
    if parts[0] == 'Ru':
        print(f"In sumanene_Ru_concave.xyz: Ru at z = {parts[3]}")
        break

# Read the sumanene_Ru_convex.xyz file
with open('sumanene_Ru_convex.xyz', 'r') as f:
    lines = f.readlines()
    
# Find Ru position
for i, line in enumerate(lines[2:]):
    parts = line.split()
    if parts[0] == 'Ru':
        print(f"In sumanene_Ru_convex.xyz: Ru at z = {parts[3]}")
        break

# Central ring and CH2 positions for reference
print(f"
Central ring centroid z $\approx$ 1.06")
print(f"CH2 groups centroid z $\approx$ -0.008")
print("
Conclusion:")
print("- Ru at z = 2.75 is ABOVE the central ring (z=1.06), AWAY from CH2 (z=-0.008)")
print("  $\rightarrow$ This is the CONVEX isomer (Ru on outer surface)")
print("- Ru at z = -0.64 is BELOW the central ring, NEAR the CH2 groups")
print("  $\rightarrow$ This is the CONCAVE isomer (Ru inside the bowl)")

\end{verbatim}\par
\smallskip
\end{tcolorbox}

\setlength{\parindent}{5pt} \robot \hspace{2pt} \textbf{Estructural}

\begin{tcolorbox}[
    colback=matterbg2,
    colframe=mattergreen1,
    width=\textwidth,
    arc=2mm,
    boxrule=0.2mm,
    leftrule=0.2mm, rightrule=0.2mm,
    toprule=0.2mm, bottomrule=0.2mm,
    enhanced,
    breakable
]
\textbf{Action:}

\begin{markdown}
The labels are indeed swapped! Let me correct this:
- `sumanene_Ru_concave.xyz` (Ru at z=2.75, outside the bowl) $\rightarrow$ should be **CONVEX**
- `sumanene_Ru_convex.xyz` (Ru at z=-0.64, inside the bowl cavity) $\rightarrow$ should be **CONCAVE**

Let me fix the files and bind the Cp ligand to create the final structures:
\end{markdown}

\textbf{Tool used:}

\setlength{\parindent}{5pt}\underline{\texttt{Tool Name:}} \texttt{repl\_tool}\par
\setlength{\parindent}{5pt}\underline{\texttt{Arguments:}}\par
\setlength{\parindent}{10pt}\texttt{code =}\par
\begin{verbatim}

import os
import shutil

# Swap the file names to correct the labels
# sumanene_Ru_concave.xyz (Ru at z=2.75) -> should be sumanene_Ru_convex_temp.xyz
# sumanene_Ru_convex.xyz (Ru at z=-0.64) -> should be sumanene_Ru_concave_temp.xyz

# Read both files
with open('sumanene_Ru_concave.xyz', 'r') as f:
    concave_content = f.read()  # This is actually convex

with open('sumanene_Ru_convex.xyz', 'r') as f:
    convex_content = f.read()  # This is actually concave

# Write with correct names
with open('sumanene_Ru_convex_corrected.xyz', 'w') as f:
    f.write(concave_content)  # z=2.75, outside bowl = convex

with open('sumanene_Ru_concave_corrected.xyz', 'w') as f:
    f.write(convex_content)  # z=-0.64, inside bowl = concave

print("Created corrected files:")
print("- sumanene_Ru_convex_corrected.xyz: Ru at z=2.75 (outside bowl)")
print("- sumanene_Ru_concave_corrected.xyz: Ru at z=-0.64 (inside bowl)")

\end{verbatim}\par
\smallskip
\end{tcolorbox}

\setlength{\parindent}{5pt} \robot \hspace{2pt} \textbf{Estructural}

\begin{tcolorbox}[
    colback=matterbg2,
    colframe=mattergreen1,
    width=\textwidth,
    arc=2mm,
    boxrule=0.2mm,
    leftrule=0.2mm, rightrule=0.2mm,
    toprule=0.2mm, bottomrule=0.2mm,
    enhanced,
    breakable
]
\textbf{Action:}

\begin{markdown}
Now I need to bind the Cp ligand to Ru (index 33) in both corrected structures. Let me start with the convex isomer:
\end{markdown}

\textbf{Tool used:}

\setlength{\parindent}{5pt}\underline{\texttt{Tool Name:}} \texttt{bind\_predefined\_fragment}\par
\setlength{\parindent}{5pt}\underline{\texttt{Arguments:}}\par
\setlength{\parindent}{10pt}\texttt{core\_file\_path = sumanene\_Ru\_convex\_corrected.xyz}\par
\setlength{\parindent}{10pt}\texttt{core\_indices = [33]}\par
\setlength{\parindent}{10pt}\texttt{ligand\_name = Cp}\par
\setlength{\parindent}{10pt}\texttt{output\_path = CpRu\_sumanene\_convex.xyz}\par
\smallskip
\end{tcolorbox}

\setlength{\parindent}{5pt} \robot \hspace{2pt} \textbf{Estructural}

\begin{tcolorbox}[
    colback=matterbg2,
    colframe=mattergreen1,
    width=\textwidth,
    arc=2mm,
    boxrule=0.2mm,
    leftrule=0.2mm, rightrule=0.2mm,
    toprule=0.2mm, bottomrule=0.2mm,
    enhanced,
    breakable
]
\textbf{Action:}

\begin{markdown}
Excellent! The Cp has been bound to Ru for the convex isomer. Now let me bind Cp to the concave isomer:
\end{markdown}

\textbf{Tool used:}

\setlength{\parindent}{5pt}\underline{\texttt{Tool Name:}} \texttt{bind\_predefined\_fragment}\par
\setlength{\parindent}{5pt}\underline{\texttt{Arguments:}}\par
\setlength{\parindent}{10pt}\texttt{core\_file\_path = sumanene\_Ru\_concave\_corrected.xyz}\par
\setlength{\parindent}{10pt}\texttt{core\_indices = [33]}\par
\setlength{\parindent}{10pt}\texttt{ligand\_name = Cp}\par
\setlength{\parindent}{10pt}\texttt{output\_path = CpRu\_sumanene\_concave.xyz}\par
\smallskip
\end{tcolorbox}

\setlength{\parindent}{5pt} \robot \hspace{2pt} \textbf{Estructural}

\begin{tcolorbox}[
    colback=matterbg2,
    colframe=mattergreen1,
    width=\textwidth,
    arc=2mm,
    boxrule=0.2mm,
    leftrule=0.2mm, rightrule=0.2mm,
    toprule=0.2mm, bottomrule=0.2mm,
    enhanced,
    breakable
]
\textbf{Action:}

\begin{markdown}
Both complexes have been created. Let me visualize them to verify the structures. First, let me view the **convex** isomer:
\end{markdown}

\textbf{Tool used:}

\setlength{\parindent}{5pt}\underline{\texttt{Tool Name:}} \texttt{view\_molecule}\par
\setlength{\parindent}{5pt}\underline{\texttt{Arguments:}}\par
\setlength{\parindent}{10pt}\texttt{xyz\_file\_relative\_path = CpRu\_sumanene\_convex.xyz}\par
\setlength{\parindent}{10pt}\texttt{left\_right\_deg = 0}\par
\setlength{\parindent}{10pt}\texttt{up\_down\_deg = 90}\par
\smallskip
\end{tcolorbox}

\setlength{\parindent}{5pt} \robot \hspace{2pt} \textbf{Estructural}

\begin{tcolorbox}[
    colback=matterbg2,
    colframe=mattergreen1,
    width=\textwidth,
    arc=2mm,
    boxrule=0.2mm,
    leftrule=0.2mm, rightrule=0.2mm,
    toprule=0.2mm, bottomrule=0.2mm,
    enhanced,
    breakable
]
\textbf{Action:}

\begin{markdown}
I can see the **convex** CpRu($\eta$$^6$-sumanene)$^+$ complex:
- Ru:33 (teal) is coordinated to the **outer surface** of the sumanene bowl
- The Cp ring (C:34-38 with H atoms) is on the opposite side from sumanene
- The bowl opens away from the Ru center

Now let me view the **concave** isomer:
\end{markdown}

\textbf{Tool used:}

\setlength{\parindent}{5pt}\underline{\texttt{Tool Name:}} \texttt{view\_molecule}\par
\setlength{\parindent}{5pt}\underline{\texttt{Arguments:}}\par
\setlength{\parindent}{10pt}\texttt{xyz\_file\_relative\_path = CpRu\_sumanene\_concave.xyz}\par
\setlength{\parindent}{10pt}\texttt{left\_right\_deg = 0}\par
\setlength{\parindent}{10pt}\texttt{up\_down\_deg = 90}\par
\smallskip
\end{tcolorbox}

\setlength{\parindent}{5pt} \robot \hspace{2pt} \textbf{Estructural}

\begin{tcolorbox}[
    colback=matterbg2,
    colframe=mattergreen1,
    width=\textwidth,
    arc=2mm,
    boxrule=0.2mm,
    leftrule=0.2mm, rightrule=0.2mm,
    toprule=0.2mm, bottomrule=0.2mm,
    enhanced,
    breakable
]
\textbf{Action:}

\begin{markdown}
Now I can clearly see the **concave** CpRu($\eta$$^6$-sumanene)$^+$ complex:
- Ru:33 (teal) is coordinated to the **inner surface** of the sumanene bowl
- The Cp ring (C:34-38) is positioned inside the bowl cavity
- The sumanene bowl curves around the Ru-Cp unit
- The CH$_2$ groups (H:23, H:24, H:26, etc.) form the rim around the complex

Let me view both complexes from another angle to better highlight the structural difference:
\end{markdown}

\textbf{Tool used:}

\setlength{\parindent}{5pt}\underline{\texttt{Tool Name:}} \texttt{view\_molecule}\par
\setlength{\parindent}{5pt}\underline{\texttt{Arguments:}}\par
\setlength{\parindent}{10pt}\texttt{xyz\_file\_relative\_path = CpRu\_sumanene\_convex.xyz}\par
\setlength{\parindent}{10pt}\texttt{left\_right\_deg = 30}\par
\setlength{\parindent}{10pt}\texttt{up\_down\_deg = 45}\par
\smallskip
\end{tcolorbox}

\setlength{\parindent}{5pt} \robot \hspace{2pt} \textbf{Estructural}

\begin{tcolorbox}[
    colback=matterbg2,
    colframe=mattergreen1,
    width=\textwidth,
    arc=2mm,
    boxrule=0.2mm,
    leftrule=0.2mm, rightrule=0.2mm,
    toprule=0.2mm, bottomrule=0.2mm,
    enhanced,
    breakable
]
\textbf{Action:}

\begin{markdown}
This is an excellent view of the **convex** CpRu($\eta$$^6$-sumanene)$^+$ complex:
- Ru:33 (teal) is on the **outer surface** of the sumanene bowl
- The Cp ring (C:35-38 with H atoms) is positioned away from the bowl
- The sumanene bowl curves away from the Ru-Cp unit

Now let me view the **concave** isomer from the same angle:
\end{markdown}

\textbf{Tool used:}

\setlength{\parindent}{5pt}\underline{\texttt{Tool Name:}} \texttt{view\_molecule}\par
\setlength{\parindent}{5pt}\underline{\texttt{Arguments:}}\par
\setlength{\parindent}{10pt}\texttt{xyz\_file\_relative\_path = CpRu\_sumanene\_concave.xyz}\par
\setlength{\parindent}{10pt}\texttt{left\_right\_deg = 30}\par
\setlength{\parindent}{10pt}\texttt{up\_down\_deg = 45}\par
\smallskip
\end{tcolorbox}

\setlength{\parindent}{5pt} \robot \hspace{2pt} \textbf{Estructural}

\begin{tcolorbox}[
    colback=matterbg2,
    colframe=mattergreen1,
    width=\textwidth,
    arc=2mm,
    boxrule=0.2mm,
    leftrule=0.2mm, rightrule=0.2mm,
    toprule=0.2mm, bottomrule=0.2mm,
    enhanced,
    breakable
]
\textbf{Action:}

\begin{markdown}
This is an excellent view of the **concave** CpRu($\eta$$^6$-sumanene)$^+$ complex:
- **Ru:33** (teal) is coordinated to the **inner surface** of the sumanene bowl
- The **Cp ring** (C:34-38 with H atoms) is positioned **inside the bowl cavity**
- The sumanene bowl curves **around** the Ru-Cp unit
- The CH$_2$ groups form the rim surrounding the complex

**Summary**

I have successfully built both isomeric **CpRu($\eta$$^6$-sumanene)$^+$** complexes:

| Isomer | File | Description |
|--------|------|-------------|
| **Convex** | `CpRu_sumanene_convex.xyz` | Ru coordinates to the **outer surface** of the bowl-shaped sumanene. The Cp ligand points away from the bowl. |
| **Concave** | `CpRu_sumanene_concave.xyz` | Ru coordinates to the **inner surface** of the bowl. The Cp ligand is nestled inside the bowl cavity. |

**Key structural features:**
- **Sumanene** is a C$_2$$_1$H$_1$$_2$ bowl-shaped polycyclic aromatic hydrocarbon
- **Central benzene ring** (atoms 2, 3, 7, 8, 12, 13) serves as the $\eta$$^6$-coordination site for Ru
- **Ru-ring distance**: ~1.70 Å (typical for $\eta$$^6$-arene coordination)
- The **3 CH$_2$ groups** define the rim of the bowl and allow clear distinction between the concave and convex faces

Would you like me to perform a geometry optimization on these structures using xTB to refine the bond distances and angles?
\end{markdown}

\end{tcolorbox}

\setlength{\parindent}{5pt} \textbf{\textcolor{blue}{User:}}
\begin{tcolorbox}[
    colback=blue!10,
    colframe=blue,
    width=\textwidth,
    arc=2mm,
    boxrule=0.2mm,
    leftrule=0.2mm, rightrule=0.2mm,
    toprule=0.2mm, bottomrule=0.2mm,
    enhanced,
    breakable
]
\begin{markdown}
In the previous structures, Ru was $\eta$$^6$-coordinated to the central hexagon of sumanene.
Please also generate structures in which Ru is $\eta$$^6$-coordinated to a peripheral hexagonal ring of sumanene, while keeping the Cp ligand bound to Ru.
Provide both concave and convex coordination geometries.
\end{markdown}
\end{tcolorbox}
\setlength{\parindent}{5pt} \robot \hspace{2pt} \textbf{Estructural}

\begin{tcolorbox}[
    colback=matterbg2,
    colframe=mattergreen1,
    width=\textwidth,
    arc=2mm,
    boxrule=0.2mm,
    leftrule=0.2mm, rightrule=0.2mm,
    toprule=0.2mm, bottomrule=0.2mm,
    enhanced,
    breakable
]
\textbf{Action:}

\begin{markdown}
I'll generate CpRu($\eta$$^6$-sumanene)$^+$ complexes where Ru coordinates to a **peripheral benzene ring** of sumanene. From my earlier SMARTS analysis, I identified the peripheral benzene rings. Let me first identify them clearly and determine which faces are concave vs convex:
\end{markdown}

\textbf{Tool used:}

\setlength{\parindent}{5pt}\underline{\texttt{Tool Name:}} \texttt{repl\_tool}\par
\setlength{\parindent}{5pt}\underline{\texttt{Arguments:}}\par
\setlength{\parindent}{10pt}\texttt{code =}\par
\begin{verbatim}

import numpy as np

# Read sumanene structure
with open('sumanene.xyz', 'r') as f:
    lines = f.readlines()

n_atoms = int(lines[0].strip())
atoms = []
for i, line in enumerate(lines[2:2+n_atoms]):
    parts = line.split()
    element = parts[0]
    x, y, z = float(parts[1]), float(parts[2]), float(parts[3])
    atoms.append((element, np.array([x, y, z])))

# Peripheral benzene rings from SMARTS matching
peripheral_ring_1 = [1, 2, 3, 4, 19, 20]  # One peripheral ring
peripheral_ring_2 = [11, 12, 13, 14, 15, 16]  # Another peripheral ring

# Central benzene ring for reference
central_ring = [2, 3, 7, 8, 12, 13]

# Calculate centroids
def get_centroid(indices):
    coords = np.array([atoms[i][1] for i in indices])
    return np.mean(coords, axis=0)

central_centroid = get_centroid(central_ring)
periph1_centroid = get_centroid(peripheral_ring_1)
periph2_centroid = get_centroid(peripheral_ring_2)

print("Central benzene ring centroid:", central_centroid)
print("Peripheral ring 1 (atoms 1,2,3,4,19,20) centroid:", periph1_centroid)
print("Peripheral ring 2 (atoms 11,12,13,14,15,16) centroid:", periph2_centroid)

# Calculate normal vector for peripheral ring 1
ring_coords = np.array([atoms[i][1] for i in peripheral_ring_1])
v1 = ring_coords[1] - ring_coords[0]
v2 = ring_coords[2] - ring_coords[0]
normal_periph1 = np.cross(v1, v2)
normal_periph1 = normal_periph1 / np.linalg.norm(normal_periph1)

print("
Peripheral ring 1 normal vector:", normal_periph1)

# Determine concave/convex direction
# Vector from peripheral ring centroid to central ring centroid points toward the "inside" of the bowl
to_center = central_centroid - periph1_centroid
print("Vector from peripheral to central:", to_center)

# The concave side is toward the interior of the bowl
# Check if normal points toward or away from center
dot_product = np.dot(normal_periph1, to_center)
print(f"Dot product of normal with to_center: {dot_product}")

if dot_product > 0:
    concave_direction = normal_periph1
    convex_direction = -normal_periph1
else:
    concave_direction = -normal_periph1
    convex_direction = normal_periph1

print("
Concave direction (toward bowl interior):", concave_direction)
print("Convex direction (away from bowl):", convex_direction)

# Ru-ring distance for $\eta$$^6$ coordination
ru_distance = 1.70  # Å

# Calculate Ru positions for peripheral ring 1
ru_concave_pos = periph1_centroid + concave_direction * ru_distance
ru_convex_pos = periph1_centroid + convex_direction * ru_distance

print(f"
For Peripheral Ring 1 coordination:")
print(f"Ru CONCAVE position: {ru_concave_pos}")
print(f"Ru CONVEX position: {ru_convex_pos}")

\end{verbatim}\par
\smallskip
\end{tcolorbox}

\setlength{\parindent}{5pt} \robot \hspace{2pt} \textbf{Estructural}

\begin{tcolorbox}[
    colback=matterbg2,
    colframe=mattergreen1,
    width=\textwidth,
    arc=2mm,
    boxrule=0.2mm,
    leftrule=0.2mm, rightrule=0.2mm,
    toprule=0.2mm, bottomrule=0.2mm,
    enhanced,
    breakable
]
\textbf{Action:}

\begin{markdown}
I've identified the peripheral benzene ring and calculated the Ru positions. The peripheral ring 1 (atoms 1, 2, 3, 4, 19, 20) is tilted relative to the central ring. Now let me create the structures:
\end{markdown}

\textbf{Tool used:}

\setlength{\parindent}{5pt}\underline{\texttt{Tool Name:}} \texttt{repl\_tool}\par
\setlength{\parindent}{5pt}\underline{\texttt{Arguments:}}\par
\setlength{\parindent}{10pt}\texttt{code =}\par
\begin{verbatim}

import numpy as np

# Read sumanene structure
with open('sumanene.xyz', 'r') as f:
    lines = f.readlines()

n_atoms = int(lines[0].strip())

# Ru positions for peripheral ring 1 coordination
ru_concave_pos = np.array([1.22859192, 0.26047285, -0.93649893])  # Inside bowl
ru_convex_pos = np.array([3.05310908, 0.37648782, 1.93015027])    # Outside bowl

# Create file with Ru at CONCAVE position (inside bowl)
with open('sumanene_Ru_periph_concave.xyz', 'w') as f:
    f.write(f"{n_atoms + 1}
")
    f.write("Sumanene with Ru at peripheral ring concave position
")
    # Write original atoms
    for line in lines[2:2+n_atoms]:
        f.write(line)
    # Add Ru atom
    f.write(f"Ru    {ru_concave_pos[0]:.8f}    {ru_concave_pos[1]:.8f}    {ru_concave_pos[2]:.8f}
")

print("Created sumanene_Ru_periph_concave.xyz with Ru inside the bowl (concave)")

# Create file with Ru at CONVEX position (outside bowl)
with open('sumanene_Ru_periph_convex.xyz', 'w') as f:
    f.write(f"{n_atoms + 1}
")
    f.write("Sumanene with Ru at peripheral ring convex position
")
    # Write original atoms
    for line in lines[2:2+n_atoms]:
        f.write(line)
    # Add Ru atom
    f.write(f"Ru    {ru_convex_pos[0]:.8f}    {ru_convex_pos[1]:.8f}    {ru_convex_pos[2]:.8f}
")

print("Created sumanene_Ru_periph_convex.xyz with Ru outside the bowl (convex)")

print(f"
Ru is at index 33 in both files")
print(f"Peripheral ring atoms: 1, 2, 3, 4, 19, 20")

\end{verbatim}\par
\smallskip
\end{tcolorbox}

\setlength{\parindent}{5pt} \robot \hspace{2pt} \textbf{Estructural}

\begin{tcolorbox}[
    colback=matterbg2,
    colframe=mattergreen1,
    width=\textwidth,
    arc=2mm,
    boxrule=0.2mm,
    leftrule=0.2mm, rightrule=0.2mm,
    toprule=0.2mm, bottomrule=0.2mm,
    enhanced,
    breakable
]
\textbf{Action:}

\begin{markdown}
I've created the intermediate structures. Let me verify the Ru positions by viewing them:
\end{markdown}

\textbf{Tool used:}

\setlength{\parindent}{5pt}\underline{\texttt{Tool Name:}} \texttt{view\_molecule}\par
\setlength{\parindent}{5pt}\underline{\texttt{Arguments:}}\par
\setlength{\parindent}{10pt}\texttt{xyz\_file\_relative\_path = sumanene\_Ru\_periph\_concave.xyz}\par
\setlength{\parindent}{10pt}\texttt{left\_right\_deg = 30}\par
\setlength{\parindent}{10pt}\texttt{up\_down\_deg = 45}\par
\smallskip
\end{tcolorbox}

\setlength{\parindent}{5pt} \robot \hspace{2pt} \textbf{Estructural}

\begin{tcolorbox}[
    colback=matterbg2,
    colframe=mattergreen1,
    width=\textwidth,
    arc=2mm,
    boxrule=0.2mm,
    leftrule=0.2mm, rightrule=0.2mm,
    toprule=0.2mm, bottomrule=0.2mm,
    enhanced,
    breakable
]
\textbf{Action:}

\begin{markdown}
Excellent! I can see the **concave** peripheral ring coordination - Ru:33 (teal) is positioned on the inner side of the bowl, near the peripheral benzene ring (C:1, C:2, C:3, C:4, C:19, C:20). Now let me view the convex structure:
\end{markdown}

\textbf{Tool used:}

\setlength{\parindent}{5pt}\underline{\texttt{Tool Name:}} \texttt{view\_molecule}\par
\setlength{\parindent}{5pt}\underline{\texttt{Arguments:}}\par
\setlength{\parindent}{10pt}\texttt{xyz\_file\_relative\_path = sumanene\_Ru\_periph\_convex.xyz}\par
\setlength{\parindent}{10pt}\texttt{left\_right\_deg = 30}\par
\setlength{\parindent}{10pt}\texttt{up\_down\_deg = 45}\par
\smallskip
\end{tcolorbox}

\setlength{\parindent}{5pt} \robot \hspace{2pt} \textbf{Estructural}

\begin{tcolorbox}[
    colback=matterbg2,
    colframe=mattergreen1,
    width=\textwidth,
    arc=2mm,
    boxrule=0.2mm,
    leftrule=0.2mm, rightrule=0.2mm,
    toprule=0.2mm, bottomrule=0.2mm,
    enhanced,
    breakable
]
\textbf{Action:}

\begin{markdown}
I can see the **convex** peripheral ring coordination - Ru:33 (teal) is positioned on the **outer surface** of the bowl, near the peripheral benzene ring. The bowl cavity is on the opposite side.

Now let me bind the Cp ligand to Ru in both structures:
\end{markdown}

\textbf{Tool used:}

\setlength{\parindent}{5pt}\underline{\texttt{Tool Name:}} \texttt{bind\_predefined\_fragment}\par
\setlength{\parindent}{5pt}\underline{\texttt{Arguments:}}\par
\setlength{\parindent}{10pt}\texttt{core\_file\_path = sumanene\_Ru\_periph\_concave.xyz}\par
\setlength{\parindent}{10pt}\texttt{core\_indices = [33]}\par
\setlength{\parindent}{10pt}\texttt{ligand\_name = Cp}\par
\setlength{\parindent}{10pt}\texttt{output\_path = CpRu\_sumanene\_periph\_concave.xyz}\par
\smallskip
\end{tcolorbox}

\setlength{\parindent}{5pt} \robot \hspace{2pt} \textbf{Estructural}

\begin{tcolorbox}[
    colback=matterbg2,
    colframe=mattergreen1,
    width=\textwidth,
    arc=2mm,
    boxrule=0.2mm,
    leftrule=0.2mm, rightrule=0.2mm,
    toprule=0.2mm, bottomrule=0.2mm,
    enhanced,
    breakable
]
\textbf{Action:}

\begin{markdown}
The concave peripheral structure is created. Now let me bind Cp to the convex structure:
\end{markdown}

\textbf{Tool used:}

\setlength{\parindent}{5pt}\underline{\texttt{Tool Name:}} \texttt{bind\_predefined\_fragment}\par
\setlength{\parindent}{5pt}\underline{\texttt{Arguments:}}\par
\setlength{\parindent}{10pt}\texttt{core\_file\_path = sumanene\_Ru\_periph\_convex.xyz}\par
\setlength{\parindent}{10pt}\texttt{core\_indices = [33]}\par
\setlength{\parindent}{10pt}\texttt{ligand\_name = Cp}\par
\setlength{\parindent}{10pt}\texttt{output\_path = CpRu\_sumanene\_periph\_convex.xyz}\par
\smallskip
\end{tcolorbox}

\setlength{\parindent}{5pt} \robot \hspace{2pt} \textbf{Estructural}

\begin{tcolorbox}[
    colback=matterbg2,
    colframe=mattergreen1,
    width=\textwidth,
    arc=2mm,
    boxrule=0.2mm,
    leftrule=0.2mm, rightrule=0.2mm,
    toprule=0.2mm, bottomrule=0.2mm,
    enhanced,
    breakable
]
\textbf{Action:}

\begin{markdown}
Both peripheral ring complexes are created. Let me visualize them to verify the structures. First, the **concave** peripheral coordination:
\end{markdown}

\textbf{Tool used:}

\setlength{\parindent}{5pt}\underline{\texttt{Tool Name:}} \texttt{view\_molecule}\par
\setlength{\parindent}{5pt}\underline{\texttt{Arguments:}}\par
\setlength{\parindent}{10pt}\texttt{xyz\_file\_relative\_path = CpRu\_sumanene\_periph\_concave.xyz}\par
\setlength{\parindent}{10pt}\texttt{left\_right\_deg = 30}\par
\setlength{\parindent}{10pt}\texttt{up\_down\_deg = 45}\par
\smallskip
\end{tcolorbox}

\setlength{\parindent}{5pt} \robot \hspace{2pt} \textbf{Estructural}

\begin{tcolorbox}[
    colback=matterbg2,
    colframe=mattergreen1,
    width=\textwidth,
    arc=2mm,
    boxrule=0.2mm,
    leftrule=0.2mm, rightrule=0.2mm,
    toprule=0.2mm, bottomrule=0.2mm,
    enhanced,
    breakable
]
\textbf{Action:}

\begin{markdown}
Excellent! I can see the **concave peripheral ring** CpRu($\eta$$^6$-sumanene)$^+$ complex:
- **Ru:33** (teal) is coordinated to the **peripheral benzene ring** (C:1, C:2, C:3, C:4, C:19, C:20)
- The **Cp ring** (C:36, C:37 with H atoms) is positioned **inside the bowl cavity**
- The central benzene ring and other peripheral rings are visible as part of the sumanene framework

Now let me view the **convex peripheral** coordination:
\end{markdown}

\textbf{Tool used:}

\setlength{\parindent}{5pt}\underline{\texttt{Tool Name:}} \texttt{view\_molecule}\par
\setlength{\parindent}{5pt}\underline{\texttt{Arguments:}}\par
\setlength{\parindent}{10pt}\texttt{xyz\_file\_relative\_path = CpRu\_sumanene\_periph\_convex.xyz}\par
\setlength{\parindent}{10pt}\texttt{left\_right\_deg = 30}\par
\setlength{\parindent}{10pt}\texttt{up\_down\_deg = 45}\par
\smallskip
\end{tcolorbox}

\setlength{\parindent}{5pt} \robot \hspace{2pt} \textbf{Estructural}

\begin{tcolorbox}[
    colback=matterbg2,
    colframe=mattergreen1,
    width=\textwidth,
    arc=2mm,
    boxrule=0.2mm,
    leftrule=0.2mm, rightrule=0.2mm,
    toprule=0.2mm, bottomrule=0.2mm,
    enhanced,
    breakable
]
\textbf{Action:}

\begin{markdown}
I can now see the **convex peripheral ring** CpRu($\eta$$^6$-sumanene)$^+$ complex clearly:
- **Ru:33** (teal) is coordinated to the **outer surface** of the peripheral benzene ring
- The **Cp ring** (C:34-38 with H atoms) extends **outward**, away from the bowl
- The sumanene bowl structure is clearly visible with the peripheral ring (C:2, C:3, C:4, etc.) serving as the $\eta$$^6$ coordination site

Let me also view these from a side angle to better show the bowl geometry:
\end{markdown}

\textbf{Tool used:}

\setlength{\parindent}{5pt}\underline{\texttt{Tool Name:}} \texttt{view\_molecule}\par
\setlength{\parindent}{5pt}\underline{\texttt{Arguments:}}\par
\setlength{\parindent}{10pt}\texttt{xyz\_file\_relative\_path = CpRu\_sumanene\_periph\_concave.xyz}\par
\setlength{\parindent}{10pt}\texttt{left\_right\_deg = 0}\par
\setlength{\parindent}{10pt}\texttt{up\_down\_deg = 90}\par
\smallskip
\end{tcolorbox}

\setlength{\parindent}{5pt} \robot \hspace{2pt} \textbf{Estructural}

\begin{tcolorbox}[
    colback=matterbg2,
    colframe=mattergreen1,
    width=\textwidth,
    arc=2mm,
    boxrule=0.2mm,
    leftrule=0.2mm, rightrule=0.2mm,
    toprule=0.2mm, bottomrule=0.2mm,
    enhanced,
    breakable
]
\textbf{Action:}

\begin{markdown}
This is an excellent side view showing the **concave peripheral ring** coordination:
- **Ru:33** (teal) is positioned **inside the bowl cavity**
- The **Cp ring** (C:34-38) is oriented inside the bowl
- The **peripheral benzene ring** (C:1, C:2, C:3, C:4, C:19, C:20) serves as the $\eta$$^6$ coordination site
- The bowl structure curves around the Ru-Cp unit

Now let me view the **convex peripheral** complex from the same angle:
\end{markdown}

\textbf{Tool used:}

\setlength{\parindent}{5pt}\underline{\texttt{Tool Name:}} \texttt{view\_molecule}\par
\setlength{\parindent}{5pt}\underline{\texttt{Arguments:}}\par
\setlength{\parindent}{10pt}\texttt{xyz\_file\_relative\_path = CpRu\_sumanene\_periph\_convex.xyz}\par
\setlength{\parindent}{10pt}\texttt{left\_right\_deg = 0}\par
\setlength{\parindent}{10pt}\texttt{up\_down\_deg = 90}\par
\smallskip
\end{tcolorbox}

\setlength{\parindent}{5pt} \robot \hspace{2pt} \textbf{Estructural}

\begin{tcolorbox}[
    colback=matterbg2,
    colframe=mattergreen1,
    width=\textwidth,
    arc=2mm,
    boxrule=0.2mm,
    leftrule=0.2mm, rightrule=0.2mm,
    toprule=0.2mm, bottomrule=0.2mm,
    enhanced,
    breakable
]
\textbf{Action:}

\begin{markdown}
This side view clearly shows the **convex peripheral ring** coordination:
- **Ru:33** (teal) is positioned on the **outer surface** of the bowl
- The **Cp ring** (C:34-38) extends **outward** from the bowl
- The **peripheral benzene ring** (C:1, C:2, C:3, C:4, C:19, C:20) serves as the $\eta$$^6$ coordination site
- The bowl cavity is on the opposite side from the Ru-Cp unit

**Summary**

I have successfully built all four **CpRu($\eta$$^6$-sumanene)$^+$** isomeric complexes:

**Central Ring Coordination (from previous task):**
| Isomer | File | Description |
|--------|------|-------------|
| **Convex** | `CpRu_sumanene_convex.xyz` | Ru $\eta$$^6$-coordinated to **central benzene ring** (atoms 2,3,7,8,12,13) from the **outer surface** |
| **Concave** | `CpRu_sumanene_concave.xyz` | Ru $\eta$$^6$-coordinated to **central benzene ring** from the **inner surface** (inside the bowl) |

**Peripheral Ring Coordination (new):**
| Isomer | File | Description |
|--------|------|-------------|
| **Convex** | `CpRu_sumanene_periph_convex.xyz` | Ru $\eta$$^6$-coordinated to **peripheral benzene ring** (atoms 1,2,3,4,19,20) from the **outer surface** |
| **Concave** | `CpRu_sumanene_periph_concave.xyz` | Ru $\eta$$^6$-coordinated to **peripheral benzene ring** from the **inner surface** (inside the bowl) |

**Key structural features:**
- **Peripheral benzene ring** (atoms 1, 2, 3, 4, 19, 20) is tilted relative to the central ring
- **Ru-ring distance**: ~1.70 Å (typical for $\eta$$^6$-arene coordination)
- **Convex** isomers have Cp pointing away from the bowl cavity
- **Concave** isomers have Cp nestled inside the bowl cavity

Would you like me to perform geometry optimization on any of these structures using xTB to refine the geometries?
\end{markdown}

\end{tcolorbox}
