# Supplementary material for: El Agente Estructural: An Artificially Intelligent Molecular Editor
Source: arXiv:2602.04849 source file (2026-11-30)
Supplement: Supplementary file 13 [file CoPor_symmetric.tex]

\setlength{\parindent}{5pt} \textbf{\textcolor{blue}{User:}}
\begin{tcolorbox}[
    colback=blue!10,
    colframe=blue,
    width=\textwidth,
    arc=2mm,
    boxrule=0.2mm,
    leftrule=0.2mm, rightrule=0.2mm,
    toprule=0.2mm, bottomrule=0.2mm,
    enhanced,
    breakable
]
\begin{markdown}
Given Co-porphyrin.xyz, find four hydrogens that are symmetry-equivalent.
Replace these hydrogens with phenyl groups while keeping the rest of the hydrogens unchanged.
\end{markdown}
\end{tcolorbox}
\setlength{\parindent}{5pt} \robot \hspace{2pt} \textbf{Estructural}

\begin{tcolorbox}[
    colback=matterbg2,
    colframe=mattergreen1,
    width=\textwidth,
    arc=2mm,
    boxrule=0.2mm,
    leftrule=0.2mm, rightrule=0.2mm,
    toprule=0.2mm, bottomrule=0.2mm,
    enhanced,
    breakable
]
\textbf{Tool used:}

\setlength{\parindent}{5pt}\underline{\texttt{Tool Name:}} \texttt{repl\_tool}\par
\setlength{\parindent}{5pt}\underline{\texttt{Arguments:}}\par
\setlength{\parindent}{10pt}\texttt{code =}\par
\begin{verbatim}
import os
import shutil

project_dir = "porphyrin_phenyl_project"
if not os.path.exists(project_dir):
    os.makedirs(project_dir)

source_file = "Co-porphyrin.xyz"
dest_file = os.path.join(project_dir, "Co-porphyrin.xyz")

if os.path.exists(source_file):
    shutil.copy(source_file, dest_file)
    print(f"Copied {source_file} to {dest_file}")
else:
    print(f"{source_file} not found in root.")

\end{verbatim}\par
\smallskip
\end{tcolorbox}

\setlength{\parindent}{5pt} \robot \hspace{2pt} \textbf{Estructural}

\begin{tcolorbox}[
    colback=matterbg2,
    colframe=mattergreen1,
    width=\textwidth,
    arc=2mm,
    boxrule=0.2mm,
    leftrule=0.2mm, rightrule=0.2mm,
    toprule=0.2mm, bottomrule=0.2mm,
    enhanced,
    breakable
]
\textbf{Tool used:}

\setlength{\parindent}{5pt}\underline{\texttt{Tool Name:}} \texttt{find\_pointgroup\_equivalent\_atoms}\par
\setlength{\parindent}{5pt}\underline{\texttt{Arguments:}}\par
\setlength{\parindent}{10pt}\texttt{file\_path = porphyrin\_phenyl\_project/Co-porphyrin.xyz}\par
\smallskip
\end{tcolorbox}

\setlength{\parindent}{5pt} \robot \hspace{2pt} \textbf{Estructural}

\begin{tcolorbox}[
    colback=matterbg2,
    colframe=mattergreen1,
    width=\textwidth,
    arc=2mm,
    boxrule=0.2mm,
    leftrule=0.2mm, rightrule=0.2mm,
    toprule=0.2mm, bottomrule=0.2mm,
    enhanced,
    breakable
]
\textbf{Tool used:}

\setlength{\parindent}{5pt}\underline{\texttt{Tool Name:}} \texttt{replace\_terminal\_atom\_with\_predefined\_FG}\par
\setlength{\parindent}{5pt}\underline{\texttt{Arguments:}}\par
\setlength{\parindent}{10pt}\texttt{core\_indices = [33, 34, 35, 36]}\par
\setlength{\parindent}{10pt}\texttt{FG\_name = Ph}\par
\setlength{\parindent}{10pt}\texttt{output\_path = porphyrin\_phenyl\_project/Co-tetraphenylporphyrin.xyz}\par
\setlength{\parindent}{10pt}\texttt{core\_file\_path = porphyrin\_phenyl\_project/Co-porphyrin.xyz}\par
\smallskip
\end{tcolorbox}

\setlength{\parindent}{5pt} \robot \hspace{2pt} \textbf{Estructural}

\begin{tcolorbox}[
    colback=matterbg2,
    colframe=mattergreen1,
    width=\textwidth,
    arc=2mm,
    boxrule=0.2mm,
    leftrule=0.2mm, rightrule=0.2mm,
    toprule=0.2mm, bottomrule=0.2mm,
    enhanced,
    breakable
]
\textbf{Action:}

\begin{markdown}
The four symmetry-equivalent hydrogen atoms in `Co-porphyrin.xyz` were identified at indices **[33, 34, 35, 36]**. These correspond to the meso-positions of the porphyrin ring.

I have successfully replaced these hydrogens with phenyl groups (Ph) to generate the Co-tetraphenylporphyrin structure.

**Output File:**
`porphyrin_phenyl_project/Co-tetraphenylporphyrin.xyz`
\end{markdown}

\end{tcolorbox}
