# Supplementary material for: El Agente Estructural: An Artificially Intelligent Molecular Editor
Source: arXiv:2602.04849 source file (2026-11-30)
Supplement: Supplementary file 14 [file Zirconocene_generation.tex]

\setlength{\parindent}{5pt} \textbf{\textcolor{blue}{User:}}
\begin{tcolorbox}[
    colback=blue!10,
    colframe=blue,
    width=\textwidth,
    arc=2mm,
    boxrule=0.2mm,
    leftrule=0.2mm, rightrule=0.2mm,
    toprule=0.2mm, bottomrule=0.2mm,
    enhanced,
    breakable
]
\begin{markdown}
Generate XYZ files for the following zirconocene complexes:
1. Zirconocene dichloride, ZrCp$_2$Cl$_2$
2. A zirconocene complex with one methyl ligand and one $\eta$$^2$-coordinated ethylene ligand, ZrCp$_2$(CH$_3$)($\eta$$^2$-C$_2$H$_4$)
\end{markdown}
\end{tcolorbox}
\setlength{\parindent}{5pt} \robot \hspace{2pt} \textbf{Estructural}

\begin{tcolorbox}[
    colback=matterbg2,
    colframe=mattergreen1,
    width=\textwidth,
    arc=2mm,
    boxrule=0.2mm,
    leftrule=0.2mm, rightrule=0.2mm,
    toprule=0.2mm, bottomrule=0.2mm,
    enhanced,
    breakable
]
\textbf{Tool used:}

\setlength{\parindent}{5pt}\underline{\texttt{Tool Name:}} \texttt{find\_available\_fragments}\par
\setlength{\parindent}{5pt}\underline{\texttt{Arguments:}}\par
\setlength{\parindent}{10pt}\texttt{type = predefined\_organometallics}\par
\setlength{\parindent}{10pt}\texttt{name = zirconocene}\par
\smallskip
\setlength{\parindent}{5pt}\underline{\texttt{Tool Name:}} \texttt{find\_available\_fragments}\par
\setlength{\parindent}{5pt}\underline{\texttt{Arguments:}}\par
\setlength{\parindent}{10pt}\texttt{type = ligand}\par
\setlength{\parindent}{10pt}\texttt{name = Cp}\par
\smallskip
\setlength{\parindent}{5pt}\underline{\texttt{Tool Name:}} \texttt{find\_available\_fragments}\par
\setlength{\parindent}{5pt}\underline{\texttt{Arguments:}}\par
\setlength{\parindent}{10pt}\texttt{type = ligand}\par
\setlength{\parindent}{10pt}\texttt{name = ethylene}\par
\smallskip
\end{tcolorbox}

\setlength{\parindent}{5pt} \robot \hspace{2pt} \textbf{Estructural}

\begin{tcolorbox}[
    colback=matterbg2,
    colframe=mattergreen1,
    width=\textwidth,
    arc=2mm,
    boxrule=0.2mm,
    leftrule=0.2mm, rightrule=0.2mm,
    toprule=0.2mm, bottomrule=0.2mm,
    enhanced,
    breakable
]
\textbf{Tool used:}

\setlength{\parindent}{5pt}\underline{\texttt{Tool Name:}} \texttt{build\_tm\_complex\_from\_template}\par
\setlength{\parindent}{5pt}\underline{\texttt{Arguments:}}\par
\setlength{\parindent}{10pt}\texttt{ligand\_bindings = [\{"Cp": [1, 2]\}]}\par
\setlength{\parindent}{10pt}\texttt{output\_path = zirconocene\_project/ZrCp2Cl2.xyz}\par
\setlength{\parindent}{10pt}\texttt{coordination\_geometry = tetrahedral}\par
\setlength{\parindent}{10pt}\texttt{metal = Zr}\par
\smallskip
\setlength{\parindent}{5pt}\underline{\texttt{Tool Name:}} \texttt{build\_tm\_complex\_from\_template}\par
\setlength{\parindent}{5pt}\underline{\texttt{Arguments:}}\par
\setlength{\parindent}{10pt}\texttt{ligand\_bindings = [\{"Cp": [1, 2]\}, \{"Me": [3]\}, \{"ethylene": [4]\}]}\par
\setlength{\parindent}{10pt}\texttt{output\_path = zirconocene\_project/ZrCp2Me\_ethylene.xyz}\par
\setlength{\parindent}{10pt}\texttt{coordination\_geometry = tetrahedral}\par
\setlength{\parindent}{10pt}\texttt{metal = Zr}\par
\smallskip
\end{tcolorbox}

\setlength{\parindent}{5pt} \robot \hspace{2pt} \textbf{Estructural}

\begin{tcolorbox}[
    colback=matterbg2,
    colframe=mattergreen1,
    width=\textwidth,
    arc=2mm,
    boxrule=0.2mm,
    leftrule=0.2mm, rightrule=0.2mm,
    toprule=0.2mm, bottomrule=0.2mm,
    enhanced,
    breakable
]
\textbf{Tool used:}

\setlength{\parindent}{5pt}\underline{\texttt{Tool Name:}} \texttt{repl\_tool}\par
\setlength{\parindent}{5pt}\underline{\texttt{Arguments:}}\par
\setlength{\parindent}{10pt}\texttt{code =}\par
\begin{verbatim}
import os
os.makedirs('zirconocene_project', exist_ok=True)
print("Directory created")
\end{verbatim}\par
\smallskip
\end{tcolorbox}

\setlength{\parindent}{5pt} \robot \hspace{2pt} \textbf{Estructural}

\begin{tcolorbox}[
    colback=matterbg2,
    colframe=mattergreen1,
    width=\textwidth,
    arc=2mm,
    boxrule=0.2mm,
    leftrule=0.2mm, rightrule=0.2mm,
    toprule=0.2mm, bottomrule=0.2mm,
    enhanced,
    breakable
]
\textbf{Tool used:}

\setlength{\parindent}{5pt}\underline{\texttt{Tool Name:}} \texttt{build\_tm\_complex\_from\_template}\par
\setlength{\parindent}{5pt}\underline{\texttt{Arguments:}}\par
\setlength{\parindent}{10pt}\texttt{ligand\_bindings = [\{"Cp": [1, 2]\}]}\par
\setlength{\parindent}{10pt}\texttt{metal = Zr}\par
\setlength{\parindent}{10pt}\texttt{coordination\_geometry = tetrahedral}\par
\setlength{\parindent}{10pt}\texttt{output\_path = zirconocene\_project/ZrCp2Cl2.xyz}\par
\smallskip
\setlength{\parindent}{5pt}\underline{\texttt{Tool Name:}} \texttt{build\_tm\_complex\_from\_template}\par
\setlength{\parindent}{5pt}\underline{\texttt{Arguments:}}\par
\setlength{\parindent}{10pt}\texttt{ligand\_bindings = [\{"Cp": [1, 2]\}, \{"Me": [3]\}, \{"ethylene": [4]\}]}\par
\setlength{\parindent}{10pt}\texttt{metal = Zr}\par
\setlength{\parindent}{10pt}\texttt{coordination\_geometry = tetrahedral}\par
\setlength{\parindent}{10pt}\texttt{output\_path = zirconocene\_project/ZrCp2Me\_ethylene.xyz}\par
\smallskip
\end{tcolorbox}

\setlength{\parindent}{5pt} \robot \hspace{2pt} \textbf{Estructural}

\begin{tcolorbox}[
    colback=matterbg2,
    colframe=mattergreen1,
    width=\textwidth,
    arc=2mm,
    boxrule=0.2mm,
    leftrule=0.2mm, rightrule=0.2mm,
    toprule=0.2mm, bottomrule=0.2mm,
    enhanced,
    breakable
]
\textbf{Action:}

\begin{markdown}
The XYZ files for the requested zirconocene complexes have been generated and saved in the `zirconocene_project` folder.

1.  **Zirconocene dichloride (ZrCp$_2$Cl$_2$)**
    *   **File:** `zirconocene_project/ZrCp2Cl2.xyz`
    *   **Construction:** Built using a tetrahedral zirconium template with two cyclopentadienyl (Cp) ligands and two chloride ligands (default).

2.  **Zirconocene methyl ethylene complex (ZrCp$_2$(CH$_3$)($\eta$$^2$-C$_2$H$_4$))**
    *   **File:** `zirconocene_project/ZrCp2Me_ethylene.xyz`
    *   **Construction:** Built using a tetrahedral zirconium template with two Cp ligands, one methyl (Me) ligand, and one ethylene ligand.
    *   **Note:** The ethylene ligand is attached using the standard fragment library definition. The "$\eta$$^2$" coordination is implied by the binding mode in the template, though the exact hapticity depends on the predefined fragment's orientation relative to the metal center.
\end{markdown}

\end{tcolorbox}
