# Supplementary material for: El Agente Estructural: An Artificially Intelligent Molecular Editor
Source: arXiv:2602.04849 source file (2026-11-30)
Supplement: Supplementary file 15 [file ferrocene_single.tex]

\setlength{\parindent}{5pt} \textbf{\textcolor{blue}{User:}}
\begin{tcolorbox}[
    colback=blue!10,
    colframe=blue,
    width=\textwidth,
    arc=2mm,
    boxrule=0.2mm,
    leftrule=0.2mm, rightrule=0.2mm,
    toprule=0.2mm, bottomrule=0.2mm,
    enhanced,
    breakable
]
\begin{markdown}
Generate an XYZ file for ferrocene. Then create and save separate XYZ files for the following structural modifications:
1. Stretch the distance between the Fe atom and one Cp ring to 4.5 Å
2. Change the Cp--Fe--Cp angle to 120$^{\circ}$.
\end{markdown}
\end{tcolorbox}
\setlength{\parindent}{5pt} \robot \hspace{2pt} \textbf{Estructural}

\begin{tcolorbox}[
    colback=matterbg2,
    colframe=mattergreen1,
    width=\textwidth,
    arc=2mm,
    boxrule=0.2mm,
    leftrule=0.2mm, rightrule=0.2mm,
    toprule=0.2mm, bottomrule=0.2mm,
    enhanced,
    breakable
]
\textbf{Tool used:}

\setlength{\parindent}{5pt}\underline{\texttt{Tool Name:}} \texttt{find\_available\_fragments}\par
\setlength{\parindent}{5pt}\underline{\texttt{Arguments:}}\par
\setlength{\parindent}{10pt}\texttt{type = predefined\_organometallics}\par
\smallskip
\end{tcolorbox}

\setlength{\parindent}{5pt} \robot \hspace{2pt} \textbf{Estructural}

\begin{tcolorbox}[
    colback=matterbg2,
    colframe=mattergreen1,
    width=\textwidth,
    arc=2mm,
    boxrule=0.2mm,
    leftrule=0.2mm, rightrule=0.2mm,
    toprule=0.2mm, bottomrule=0.2mm,
    enhanced,
    breakable
]
\textbf{Tool used:}

\setlength{\parindent}{5pt}\underline{\texttt{Tool Name:}} \texttt{find\_available\_fragments}\par
\setlength{\parindent}{5pt}\underline{\texttt{Arguments:}}\par
\setlength{\parindent}{10pt}\texttt{type = ligand}\par
\setlength{\parindent}{10pt}\texttt{name = Cp}\par
\smallskip
\end{tcolorbox}

\setlength{\parindent}{5pt} \robot \hspace{2pt} \textbf{Estructural}

\begin{tcolorbox}[
    colback=matterbg2,
    colframe=mattergreen1,
    width=\textwidth,
    arc=2mm,
    boxrule=0.2mm,
    leftrule=0.2mm, rightrule=0.2mm,
    toprule=0.2mm, bottomrule=0.2mm,
    enhanced,
    breakable
]
\textbf{Tool used:}

\setlength{\parindent}{5pt}\underline{\texttt{Tool Name:}} \texttt{build\_tm\_complex\_from\_template}\par
\setlength{\parindent}{5pt}\underline{\texttt{Arguments:}}\par
\setlength{\parindent}{10pt}\texttt{ligand\_bindings = [\{"Cp": [1, 2]\}]}\par
\setlength{\parindent}{10pt}\texttt{output\_path = ferrocene\_mods\_project/ferrocene.xyz}\par
\setlength{\parindent}{10pt}\texttt{coordination\_geometry = linear}\par
\setlength{\parindent}{10pt}\texttt{metal = Fe}\par
\smallskip
\end{tcolorbox}

\setlength{\parindent}{5pt} \robot \hspace{2pt} \textbf{Estructural}

\begin{tcolorbox}[
    colback=matterbg2,
    colframe=mattergreen1,
    width=\textwidth,
    arc=2mm,
    boxrule=0.2mm,
    leftrule=0.2mm, rightrule=0.2mm,
    toprule=0.2mm, bottomrule=0.2mm,
    enhanced,
    breakable
]
\textbf{Tool used:}

\setlength{\parindent}{5pt}\underline{\texttt{Tool Name:}} \texttt{build\_tm\_complex\_from\_template}\par
\setlength{\parindent}{5pt}\underline{\texttt{Arguments:}}\par
\setlength{\parindent}{10pt}\texttt{ligand\_bindings = [\{"Cp": [1, 2]\}]}\par
\setlength{\parindent}{10pt}\texttt{output\_path = ferrocene\_project/ferrocene.xyz}\par
\setlength{\parindent}{10pt}\texttt{coordination\_geometry = linear}\par
\setlength{\parindent}{10pt}\texttt{metal = Fe}\par
\smallskip
\end{tcolorbox}

\setlength{\parindent}{5pt} \robot \hspace{2pt} \textbf{Estructural}

\begin{tcolorbox}[
    colback=matterbg2,
    colframe=mattergreen1,
    width=\textwidth,
    arc=2mm,
    boxrule=0.2mm,
    leftrule=0.2mm, rightrule=0.2mm,
    toprule=0.2mm, bottomrule=0.2mm,
    enhanced,
    breakable
]
\textbf{Tool used:}

\setlength{\parindent}{5pt}\underline{\texttt{Tool Name:}} \texttt{match\_smarts\_in\_xyz}\par
\setlength{\parindent}{5pt}\underline{\texttt{Arguments:}}\par
\setlength{\parindent}{10pt}\texttt{file\_path = ferrocene\_project/ferrocene.xyz}\par
\setlength{\parindent}{10pt}\texttt{smarts = c1cccc1}\par
\smallskip
\end{tcolorbox}

\setlength{\parindent}{5pt} \robot \hspace{2pt} \textbf{Estructural}

\begin{tcolorbox}[
    colback=matterbg2,
    colframe=mattergreen1,
    width=\textwidth,
    arc=2mm,
    boxrule=0.2mm,
    leftrule=0.2mm, rightrule=0.2mm,
    toprule=0.2mm, bottomrule=0.2mm,
    enhanced,
    breakable
]
\textbf{Tool used:}

\setlength{\parindent}{5pt}\underline{\texttt{Tool Name:}} \texttt{match\_smarts\_in\_xyz}\par
\setlength{\parindent}{5pt}\underline{\texttt{Arguments:}}\par
\setlength{\parindent}{10pt}\texttt{smarts = [\#6]}\par
\setlength{\parindent}{10pt}\texttt{file\_path = ferrocene\_project/ferrocene.xyz}\par
\smallskip
\end{tcolorbox}

\setlength{\parindent}{5pt} \robot \hspace{2pt} \textbf{Estructural}

\begin{tcolorbox}[
    colback=matterbg2,
    colframe=mattergreen1,
    width=\textwidth,
    arc=2mm,
    boxrule=0.2mm,
    leftrule=0.2mm, rightrule=0.2mm,
    toprule=0.2mm, bottomrule=0.2mm,
    enhanced,
    breakable
]
\textbf{Tool used:}

\setlength{\parindent}{5pt}\underline{\texttt{Tool Name:}} \texttt{get\_connected\_subgraph\_indices}\par
\setlength{\parindent}{5pt}\underline{\texttt{Arguments:}}\par
\setlength{\parindent}{10pt}\texttt{exclude = 0}\par
\setlength{\parindent}{10pt}\texttt{file\_path = ferrocene\_project/ferrocene.xyz}\par
\setlength{\parindent}{10pt}\texttt{start\_index = 1}\par
\smallskip
\end{tcolorbox}

\setlength{\parindent}{5pt} \robot \hspace{2pt} \textbf{Estructural}

\begin{tcolorbox}[
    colback=matterbg2,
    colframe=mattergreen1,
    width=\textwidth,
    arc=2mm,
    boxrule=0.2mm,
    leftrule=0.2mm, rightrule=0.2mm,
    toprule=0.2mm, bottomrule=0.2mm,
    enhanced,
    breakable
]
\textbf{Tool used:}

\setlength{\parindent}{5pt}\underline{\texttt{Tool Name:}} \texttt{get\_connected\_subgraph\_indices}\par
\setlength{\parindent}{5pt}\underline{\texttt{Arguments:}}\par
\setlength{\parindent}{10pt}\texttt{exclude = 0}\par
\setlength{\parindent}{10pt}\texttt{file\_path = ferrocene\_project/ferrocene.xyz}\par
\setlength{\parindent}{10pt}\texttt{start\_index = 11}\par
\smallskip
\end{tcolorbox}

\setlength{\parindent}{5pt} \robot \hspace{2pt} \textbf{Estructural}

\begin{tcolorbox}[
    colback=matterbg2,
    colframe=mattergreen1,
    width=\textwidth,
    arc=2mm,
    boxrule=0.2mm,
    leftrule=0.2mm, rightrule=0.2mm,
    toprule=0.2mm, bottomrule=0.2mm,
    enhanced,
    breakable
]
\textbf{Tool used:}

\setlength{\parindent}{5pt}\underline{\texttt{Tool Name:}} \texttt{set\_distance\_between\_fragments}\par
\setlength{\parindent}{5pt}\underline{\texttt{Arguments:}}\par
\setlength{\parindent}{10pt}\texttt{input\_path = ferrocene\_project/ferrocene.xyz}\par
\setlength{\parindent}{10pt}\texttt{output\_path = ferrocene\_project/ferrocene\_dist\_4.5.xyz}\par
\setlength{\parindent}{10pt}\texttt{fragment\_indices = [1, 2, 3, 4, 5, 6, 7, 8, 9, 10]}\par
\setlength{\parindent}{10pt}\texttt{targets = [\{"atom": [0]\}, \{"group": [1, 2, 3, 4, 5]\}]}\par
\setlength{\parindent}{10pt}\texttt{distance = 4.5}\par
\setlength{\parindent}{10pt}\texttt{fragment\_mode = manual}\par
\smallskip
\end{tcolorbox}

\setlength{\parindent}{5pt} \robot \hspace{2pt} \textbf{Estructural}

\begin{tcolorbox}[
    colback=matterbg2,
    colframe=mattergreen1,
    width=\textwidth,
    arc=2mm,
    boxrule=0.2mm,
    leftrule=0.2mm, rightrule=0.2mm,
    toprule=0.2mm, bottomrule=0.2mm,
    enhanced,
    breakable
]
\textbf{Tool used:}

\setlength{\parindent}{5pt}\underline{\texttt{Tool Name:}} \texttt{set\_angle\_between\_fragments}\par
\setlength{\parindent}{5pt}\underline{\texttt{Arguments:}}\par
\setlength{\parindent}{10pt}\texttt{fragment\_indices = [11, 12, 13, 14, 15, 16, 17, 18, 19, 20]}\par
\setlength{\parindent}{10pt}\texttt{output\_path = ferrocene\_project/ferrocene\_angle\_120.xyz}\par
\setlength{\parindent}{10pt}\texttt{targets = [\{"group": [1, 2, 3, 4, 5]\}, \{"atom": [0]\}, \{"group": [11, 12, 13, 14, 15]\}]}\par
\setlength{\parindent}{10pt}\texttt{input\_path = ferrocene\_project/ferrocene.xyz}\par
\setlength{\parindent}{10pt}\texttt{angle = 120}\par
\setlength{\parindent}{10pt}\texttt{fragment\_mode = manual}\par
\smallskip
\end{tcolorbox}

\setlength{\parindent}{5pt} \robot \hspace{2pt} \textbf{Estructural}

\begin{tcolorbox}[
    colback=matterbg2,
    colframe=mattergreen1,
    width=\textwidth,
    arc=2mm,
    boxrule=0.2mm,
    leftrule=0.2mm, rightrule=0.2mm,
    toprule=0.2mm, bottomrule=0.2mm,
    enhanced,
    breakable
]
\textbf{Action:}

\begin{markdown}
The requested XYZ files have been generated and saved in the `ferrocene_project` directory.

1.  **Base Structure**: `ferrocene_project/ferrocene.xyz`
    - Generated using a linear iron template with two cyclopentadienyl (Cp) ligands.
2.  **Distance Modification**: `ferrocene_project/ferrocene_dist_4.5.xyz`
    - The distance between the Iron atom and one Cp ring centroid was set to **4.5 Å**.
3.  **Angle Modification**: `ferrocene_project/ferrocene_angle_120.xyz`
    - The Cp(centroid)--Fe--Cp(centroid) angle was adjusted to **120$^{\circ}$**.
\end{markdown}

\end{tcolorbox}
