# Supplementary material for: El Agente Estructural: An Artificially Intelligent Molecular Editor
Source: arXiv:2602.04849 source file (2026-11-30)
Supplement: Supplementary file 16 [file reactant_axial_ligands.tex]

\setlength{\parindent}{5pt} \textbf{\textcolor{blue}{User:}}
\begin{tcolorbox}[
    colback=blue!10,
    colframe=blue,
    width=\textwidth,
    arc=2mm,
    boxrule=0.2mm,
    leftrule=0.2mm, rightrule=0.2mm,
    toprule=0.2mm, bottomrule=0.2mm,
    enhanced,
    breakable
]
\begin{markdown}
Given the cobalt-phthalocyanine complex (Co-Pc.xyz), bind the following ligands to the Co atom: CO2, COOH, CO, H, OH, and H2O.
\end{markdown}
\end{tcolorbox}
\setlength{\parindent}{5pt} \robot \hspace{2pt} \textbf{Estructural}

\begin{tcolorbox}[
    colback=matterbg2,
    colframe=mattergreen1,
    width=\textwidth,
    arc=2mm,
    boxrule=0.2mm,
    leftrule=0.2mm, rightrule=0.2mm,
    toprule=0.2mm, bottomrule=0.2mm,
    enhanced,
    breakable
]
\textbf{Tool used:}

\setlength{\parindent}{5pt}\underline{\texttt{Tool Name:}} \texttt{repl\_tool}\par
\setlength{\parindent}{5pt}\underline{\texttt{Arguments:}}\par
\setlength{\parindent}{10pt}\texttt{code =}\par
\begin{verbatim}
import os
import shutil

project_dir = 'CoPc_ligand_binding_project'
os.makedirs(project_dir, exist_ok=True)
source_file = 'Co-Pc.xyz'
target_file = os.path.join(project_dir, 'Co-Pc.xyz')

if os.path.exists(source_file):
    shutil.move(source_file, target_file)
    print(f"Moved {source_file} to {target_file}")
else:
    print(f"{source_file} not found in root (it might have been moved already). Checking target...")
    if os.path.exists(target_file):
        print(f"Found {target_file}")
    else:
        print(f"Error: {source_file} missing.")
\end{verbatim}\par
\smallskip
\setlength{\parindent}{5pt}\underline{\texttt{Tool Name:}} \texttt{find\_available\_fragments}\par
\setlength{\parindent}{5pt}\underline{\texttt{Arguments:}}\par
\setlength{\parindent}{10pt}\texttt{name = CO2}\par
\smallskip
\setlength{\parindent}{5pt}\underline{\texttt{Tool Name:}} \texttt{find\_available\_fragments}\par
\setlength{\parindent}{5pt}\underline{\texttt{Arguments:}}\par
\setlength{\parindent}{10pt}\texttt{name = COOH}\par
\smallskip
\setlength{\parindent}{5pt}\underline{\texttt{Tool Name:}} \texttt{find\_available\_fragments}\par
\setlength{\parindent}{5pt}\underline{\texttt{Arguments:}}\par
\setlength{\parindent}{10pt}\texttt{name = CO}\par
\smallskip
\setlength{\parindent}{5pt}\underline{\texttt{Tool Name:}} \texttt{find\_available\_fragments}\par
\setlength{\parindent}{5pt}\underline{\texttt{Arguments:}}\par
\setlength{\parindent}{10pt}\texttt{name = OH}\par
\smallskip
\setlength{\parindent}{5pt}\underline{\texttt{Tool Name:}} \texttt{find\_available\_fragments}\par
\setlength{\parindent}{5pt}\underline{\texttt{Arguments:}}\par
\setlength{\parindent}{10pt}\texttt{name = H2O}\par
\smallskip
\end{tcolorbox}

\setlength{\parindent}{5pt} \robot \hspace{2pt} \textbf{Estructural}

\begin{tcolorbox}[
    colback=matterbg2,
    colframe=mattergreen1,
    width=\textwidth,
    arc=2mm,
    boxrule=0.2mm,
    leftrule=0.2mm, rightrule=0.2mm,
    toprule=0.2mm, bottomrule=0.2mm,
    enhanced,
    breakable
]
\textbf{Tool used:}

\setlength{\parindent}{5pt}\underline{\texttt{Tool Name:}} \texttt{bind\_atom\_ligands\_library}\par
\setlength{\parindent}{5pt}\underline{\texttt{Arguments:}}\par
\setlength{\parindent}{10pt}\texttt{output\_path = CoPc\_ligand\_binding\_project/CoPc\_CO2.xyz}\par
\setlength{\parindent}{10pt}\texttt{ligand\_name = CO2}\par
\setlength{\parindent}{10pt}\texttt{core\_element = Co}\par
\setlength{\parindent}{10pt}\texttt{core\_file\_path = CoPc\_ligand\_binding\_project/Co-Pc.xyz}\par
\smallskip
\setlength{\parindent}{5pt}\underline{\texttt{Tool Name:}} \texttt{bind\_atom\_ligands\_library}\par
\setlength{\parindent}{5pt}\underline{\texttt{Arguments:}}\par
\setlength{\parindent}{10pt}\texttt{output\_path = CoPc\_ligand\_binding\_project/CoPc\_COOH.xyz}\par
\setlength{\parindent}{10pt}\texttt{ligand\_name = COOH}\par
\setlength{\parindent}{10pt}\texttt{core\_element = Co}\par
\setlength{\parindent}{10pt}\texttt{core\_file\_path = CoPc\_ligand\_binding\_project/Co-Pc.xyz}\par
\smallskip
\setlength{\parindent}{5pt}\underline{\texttt{Tool Name:}} \texttt{bind\_atom\_ligands\_library}\par
\setlength{\parindent}{5pt}\underline{\texttt{Arguments:}}\par
\setlength{\parindent}{10pt}\texttt{output\_path = CoPc\_ligand\_binding\_project/CoPc\_CO.xyz}\par
\setlength{\parindent}{10pt}\texttt{ligand\_name = CO}\par
\setlength{\parindent}{10pt}\texttt{core\_element = Co}\par
\setlength{\parindent}{10pt}\texttt{core\_file\_path = CoPc\_ligand\_binding\_project/Co-Pc.xyz}\par
\smallskip
\setlength{\parindent}{5pt}\underline{\texttt{Tool Name:}} \texttt{bind\_atom\_ligands\_library}\par
\setlength{\parindent}{5pt}\underline{\texttt{Arguments:}}\par
\setlength{\parindent}{10pt}\texttt{ligand\_name = H}\par
\setlength{\parindent}{10pt}\texttt{output\_path = CoPc\_ligand\_binding\_project/CoPc\_H.xyz}\par
\setlength{\parindent}{10pt}\texttt{core\_element = Co}\par
\setlength{\parindent}{10pt}\texttt{core\_file\_path = CoPc\_ligand\_binding\_project/Co-Pc.xyz}\par
\smallskip
\setlength{\parindent}{5pt}\underline{\texttt{Tool Name:}} \texttt{bind\_atom\_ligands\_library}\par
\setlength{\parindent}{5pt}\underline{\texttt{Arguments:}}\par
\setlength{\parindent}{10pt}\texttt{ligand\_name = OH}\par
\setlength{\parindent}{10pt}\texttt{output\_path = CoPc\_ligand\_binding\_project/CoPc\_OH.xyz}\par
\setlength{\parindent}{10pt}\texttt{core\_element = Co}\par
\setlength{\parindent}{10pt}\texttt{core\_file\_path = CoPc\_ligand\_binding\_project/Co-Pc.xyz}\par
\smallskip
\setlength{\parindent}{5pt}\underline{\texttt{Tool Name:}} \texttt{bind\_atom\_ligands\_library}\par
\setlength{\parindent}{5pt}\underline{\texttt{Arguments:}}\par
\setlength{\parindent}{10pt}\texttt{ligand\_name = H2O}\par
\setlength{\parindent}{10pt}\texttt{output\_path = CoPc\_ligand\_binding\_project/CoPc\_H2O.xyz}\par
\setlength{\parindent}{10pt}\texttt{core\_element = Co}\par
\setlength{\parindent}{10pt}\texttt{core\_file\_path = CoPc\_ligand\_binding\_project/Co-Pc.xyz}\par
\smallskip
\end{tcolorbox}

\setlength{\parindent}{5pt} \robot \hspace{2pt} \textbf{Estructural}

\begin{tcolorbox}[
    colback=matterbg2,
    colframe=mattergreen1,
    width=\textwidth,
    arc=2mm,
    boxrule=0.2mm,
    leftrule=0.2mm, rightrule=0.2mm,
    toprule=0.2mm, bottomrule=0.2mm,
    enhanced,
    breakable
]
\textbf{Action:}

\begin{markdown}
I have successfully bound the requested ligands (CO2, COOH, CO, H, OH, H2O) to the Cobalt atom in the Co-Pc complex.

**Action Summary:**
1.  **Project Organization:** Created a new directory `CoPc_ligand_binding_project` and moved the original `Co-Pc.xyz` file into it to keep the workspace organized.
2.  **Ligand Binding:** Used the `bind_atom_ligands_library` tool to attach each specified ligand to the central Co atom (element 'Co'). The tool automatically handled the orientation and bonding.

**Generated Files:**
All output files are located in the `CoPc_ligand_binding_project` directory:
-   `CoPc_CO2.xyz`: Cobalt-phthalocyanine with a CO2 ligand.
-   `CoPc_COOH.xyz`: Cobalt-phthalocyanine with a Carboxyl (COOH) group.
-   `CoPc_CO.xyz`: Cobalt-phthalocyanine with a Carbon Monoxide (CO) ligand.
-   `CoPc_H.xyz`: Cobalt-phthalocyanine with a Hydride (H) ligand.
-   `CoPc_OH.xyz`: Cobalt-phthalocyanine with a Hydroxyl (OH) group.
-   `CoPc_H2O.xyz`: Cobalt-phthalocyanine with a Water (H2O) ligand.
\end{markdown}

\end{tcolorbox}

\setlength{\parindent}{5pt} \textbf{\textcolor{blue}{User:}}
\begin{tcolorbox}[
    colback=blue!10,
    colframe=blue,
    width=\textwidth,
    arc=2mm,
    boxrule=0.2mm,
    leftrule=0.2mm, rightrule=0.2mm,
    toprule=0.2mm, bottomrule=0.2mm,
    enhanced,
    breakable
]
\begin{markdown}
To explore the axial ligand effect, take both the original Co-Pc.xyz (bare complex) and all the previously modified Co-Pc structures.
For each structure, attach one of the following axial ligands to the Co atom: thiophene, pyridine, and Cl.
\end{markdown}
\end{tcolorbox}
\setlength{\parindent}{5pt} \robot \hspace{2pt} \textbf{Estructural}

\begin{tcolorbox}[
    colback=matterbg2,
    colframe=mattergreen1,
    width=\textwidth,
    arc=2mm,
    boxrule=0.2mm,
    leftrule=0.2mm, rightrule=0.2mm,
    toprule=0.2mm, bottomrule=0.2mm,
    enhanced,
    breakable
]
\textbf{Tool used:}

\setlength{\parindent}{5pt}\underline{\texttt{Tool Name:}} \texttt{find\_available\_fragments}\par
\setlength{\parindent}{5pt}\underline{\texttt{Arguments:}}\par
\setlength{\parindent}{10pt}\texttt{name = thiophene}\par
\smallskip
\setlength{\parindent}{5pt}\underline{\texttt{Tool Name:}} \texttt{find\_available\_fragments}\par
\setlength{\parindent}{5pt}\underline{\texttt{Arguments:}}\par
\setlength{\parindent}{10pt}\texttt{name = pyridine}\par
\smallskip
\setlength{\parindent}{5pt}\underline{\texttt{Tool Name:}} \texttt{find\_available\_fragments}\par
\setlength{\parindent}{5pt}\underline{\texttt{Arguments:}}\par
\setlength{\parindent}{10pt}\texttt{name = Cl}\par
\smallskip
\end{tcolorbox}

\setlength{\parindent}{5pt} \robot \hspace{2pt} \textbf{Estructural}

\begin{tcolorbox}[
    colback=matterbg2,
    colframe=mattergreen1,
    width=\textwidth,
    arc=2mm,
    boxrule=0.2mm,
    leftrule=0.2mm, rightrule=0.2mm,
    toprule=0.2mm, bottomrule=0.2mm,
    enhanced,
    breakable
]
\textbf{Tool used:}

\setlength{\parindent}{5pt}\underline{\texttt{Tool Name:}} \texttt{bind\_atom\_ligands\_library}\par
\setlength{\parindent}{5pt}\underline{\texttt{Arguments:}}\par
\setlength{\parindent}{10pt}\texttt{output\_path = CoPc\_ligand\_binding\_project/CoPc\_thiophene.xyz}\par
\setlength{\parindent}{10pt}\texttt{ligand\_name = Thiophene}\par
\setlength{\parindent}{10pt}\texttt{core\_element = Co}\par
\setlength{\parindent}{10pt}\texttt{core\_file\_path = CoPc\_ligand\_binding\_project/Co-Pc.xyz}\par
\smallskip
\setlength{\parindent}{5pt}\underline{\texttt{Tool Name:}} \texttt{bind\_atom\_ligands\_library}\par
\setlength{\parindent}{5pt}\underline{\texttt{Arguments:}}\par
\setlength{\parindent}{10pt}\texttt{output\_path = CoPc\_ligand\_binding\_project/CoPc\_CO2\_thiophene.xyz}\par
\setlength{\parindent}{10pt}\texttt{ligand\_name = Thiophene}\par
\setlength{\parindent}{10pt}\texttt{core\_element = Co}\par
\setlength{\parindent}{10pt}\texttt{core\_file\_path = CoPc\_ligand\_binding\_project/CoPc\_CO2.xyz}\par
\smallskip
\setlength{\parindent}{5pt}\underline{\texttt{Tool Name:}} \texttt{bind\_atom\_ligands\_library}\par
\setlength{\parindent}{5pt}\underline{\texttt{Arguments:}}\par
\setlength{\parindent}{10pt}\texttt{output\_path = CoPc\_ligand\_binding\_project/CoPc\_COOH\_thiophene.xyz}\par
\setlength{\parindent}{10pt}\texttt{ligand\_name = Thiophene}\par
\setlength{\parindent}{10pt}\texttt{core\_element = Co}\par
\setlength{\parindent}{10pt}\texttt{core\_file\_path = CoPc\_ligand\_binding\_project/CoPc\_COOH.xyz}\par
\smallskip
\setlength{\parindent}{5pt}\underline{\texttt{Tool Name:}} \texttt{bind\_atom\_ligands\_library}\par
\setlength{\parindent}{5pt}\underline{\texttt{Arguments:}}\par
\setlength{\parindent}{10pt}\texttt{output\_path = CoPc\_ligand\_binding\_project/CoPc\_CO\_thiophene.xyz}\par
\setlength{\parindent}{10pt}\texttt{ligand\_name = Thiophene}\par
\setlength{\parindent}{10pt}\texttt{core\_element = Co}\par
\setlength{\parindent}{10pt}\texttt{core\_file\_path = CoPc\_ligand\_binding\_project/CoPc\_CO.xyz}\par
\smallskip
\setlength{\parindent}{5pt}\underline{\texttt{Tool Name:}} \texttt{bind\_atom\_ligands\_library}\par
\setlength{\parindent}{5pt}\underline{\texttt{Arguments:}}\par
\setlength{\parindent}{10pt}\texttt{output\_path = CoPc\_ligand\_binding\_project/CoPc\_H\_thiophene.xyz}\par
\setlength{\parindent}{10pt}\texttt{ligand\_name = Thiophene}\par
\setlength{\parindent}{10pt}\texttt{core\_element = Co}\par
\setlength{\parindent}{10pt}\texttt{core\_file\_path = CoPc\_ligand\_binding\_project/CoPc\_H.xyz}\par
\smallskip
\setlength{\parindent}{5pt}\underline{\texttt{Tool Name:}} \texttt{bind\_atom\_ligands\_library}\par
\setlength{\parindent}{5pt}\underline{\texttt{Arguments:}}\par
\setlength{\parindent}{10pt}\texttt{ligand\_name = Thiophene}\par
\setlength{\parindent}{10pt}\texttt{output\_path = CoPc\_ligand\_binding\_project/CoPc\_OH\_thiophene.xyz}\par
\setlength{\parindent}{10pt}\texttt{core\_element = Co}\par
\setlength{\parindent}{10pt}\texttt{core\_file\_path = CoPc\_ligand\_binding\_project/CoPc\_OH.xyz}\par
\smallskip
\setlength{\parindent}{5pt}\underline{\texttt{Tool Name:}} \texttt{bind\_atom\_ligands\_library}\par
\setlength{\parindent}{5pt}\underline{\texttt{Arguments:}}\par
\setlength{\parindent}{10pt}\texttt{output\_path = CoPc\_ligand\_binding\_project/CoPc\_H2O\_thiophene.xyz}\par
\setlength{\parindent}{10pt}\texttt{ligand\_name = Thiophene}\par
\setlength{\parindent}{10pt}\texttt{core\_element = Co}\par
\setlength{\parindent}{10pt}\texttt{core\_file\_path = CoPc\_ligand\_binding\_project/CoPc\_H2O.xyz}\par
\smallskip
\end{tcolorbox}

\setlength{\parindent}{5pt} \robot \hspace{2pt} \textbf{Estructural}

\begin{tcolorbox}[
    colback=matterbg2,
    colframe=mattergreen1,
    width=\textwidth,
    arc=2mm,
    boxrule=0.2mm,
    leftrule=0.2mm, rightrule=0.2mm,
    toprule=0.2mm, bottomrule=0.2mm,
    enhanced,
    breakable
]
\textbf{Tool used:}

\setlength{\parindent}{5pt}\underline{\texttt{Tool Name:}} \texttt{organic\_molecules\_xyz\_generation}\par
\setlength{\parindent}{5pt}\underline{\texttt{Arguments:}}\par
\setlength{\parindent}{10pt}\texttt{filenames = ["CoPc\_ligand\_binding\_project/thiophene.xyz"]}\par
\setlength{\parindent}{10pt}\texttt{smiles\_list = ["c1ccsc1"]}\par
\smallskip
\end{tcolorbox}

\setlength{\parindent}{5pt} \robot \hspace{2pt} \textbf{Estructural}

\begin{tcolorbox}[
    colback=matterbg2,
    colframe=mattergreen1,
    width=\textwidth,
    arc=2mm,
    boxrule=0.2mm,
    leftrule=0.2mm, rightrule=0.2mm,
    toprule=0.2mm, bottomrule=0.2mm,
    enhanced,
    breakable
]
\textbf{Tool used:}

\setlength{\parindent}{5pt}\underline{\texttt{Tool Name:}} \texttt{get\_atomic\_neighbors}\par
\setlength{\parindent}{5pt}\underline{\texttt{Arguments:}}\par
\setlength{\parindent}{10pt}\texttt{target = S}\par
\setlength{\parindent}{10pt}\texttt{file\_path = CoPc\_ligand\_binding\_project/thiophene.xyz}\par
\smallskip
\end{tcolorbox}

\setlength{\parindent}{5pt} \robot \hspace{2pt} \textbf{Estructural}

\begin{tcolorbox}[
    colback=matterbg2,
    colframe=mattergreen1,
    width=\textwidth,
    arc=2mm,
    boxrule=0.2mm,
    leftrule=0.2mm, rightrule=0.2mm,
    toprule=0.2mm, bottomrule=0.2mm,
    enhanced,
    breakable
]
\textbf{Tool used:}

\setlength{\parindent}{5pt}\underline{\texttt{Tool Name:}} \texttt{bind\_two\_molecules}\par
\setlength{\parindent}{5pt}\underline{\texttt{Arguments:}}\par
\setlength{\parindent}{10pt}\texttt{output\_path = CoPc\_ligand\_binding\_project/CoPc\_thiophene.xyz}\par
\setlength{\parindent}{10pt}\texttt{core\_indices = [0]}\par
\setlength{\parindent}{10pt}\texttt{ligand\_file\_path = CoPc\_ligand\_binding\_project/thiophene.xyz}\par
\setlength{\parindent}{10pt}\texttt{ligand\_idx = 3}\par
\setlength{\parindent}{10pt}\texttt{ligand\_type = ligand}\par
\setlength{\parindent}{10pt}\texttt{core\_file\_path = CoPc\_ligand\_binding\_project/Co-Pc.xyz}\par
\smallskip
\setlength{\parindent}{5pt}\underline{\texttt{Tool Name:}} \texttt{bind\_two\_molecules}\par
\setlength{\parindent}{5pt}\underline{\texttt{Arguments:}}\par
\setlength{\parindent}{10pt}\texttt{output\_path = CoPc\_ligand\_binding\_project/CoPc\_CO2\_thiophene.xyz}\par
\setlength{\parindent}{10pt}\texttt{core\_indices = [0]}\par
\setlength{\parindent}{10pt}\texttt{ligand\_file\_path = CoPc\_ligand\_binding\_project/thiophene.xyz}\par
\setlength{\parindent}{10pt}\texttt{ligand\_idx = 3}\par
\setlength{\parindent}{10pt}\texttt{ligand\_type = ligand}\par
\setlength{\parindent}{10pt}\texttt{core\_file\_path = CoPc\_ligand\_binding\_project/CoPc\_CO2.xyz}\par
\smallskip
\setlength{\parindent}{5pt}\underline{\texttt{Tool Name:}} \texttt{bind\_two\_molecules}\par
\setlength{\parindent}{5pt}\underline{\texttt{Arguments:}}\par
\setlength{\parindent}{10pt}\texttt{output\_path = CoPc\_ligand\_binding\_project/CoPc\_COOH\_thiophene.xyz}\par
\setlength{\parindent}{10pt}\texttt{core\_indices = [0]}\par
\setlength{\parindent}{10pt}\texttt{ligand\_file\_path = CoPc\_ligand\_binding\_project/thiophene.xyz}\par
\setlength{\parindent}{10pt}\texttt{core\_file\_path = CoPc\_ligand\_binding\_project/CoPc\_COOH.xyz}\par
\setlength{\parindent}{10pt}\texttt{ligand\_type = ligand}\par
\setlength{\parindent}{10pt}\texttt{ligand\_idx = 3}\par
\smallskip
\setlength{\parindent}{5pt}\underline{\texttt{Tool Name:}} \texttt{bind\_two\_molecules}\par
\setlength{\parindent}{5pt}\underline{\texttt{Arguments:}}\par
\setlength{\parindent}{10pt}\texttt{output\_path = CoPc\_ligand\_binding\_project/CoPc\_CO\_thiophene.xyz}\par
\setlength{\parindent}{10pt}\texttt{core\_indices = [0]}\par
\setlength{\parindent}{10pt}\texttt{ligand\_file\_path = CoPc\_ligand\_binding\_project/thiophene.xyz}\par
\setlength{\parindent}{10pt}\texttt{core\_file\_path = CoPc\_ligand\_binding\_project/CoPc\_CO.xyz}\par
\setlength{\parindent}{10pt}\texttt{ligand\_type = ligand}\par
\setlength{\parindent}{10pt}\texttt{ligand\_idx = 3}\par
\smallskip
\setlength{\parindent}{5pt}\underline{\texttt{Tool Name:}} \texttt{bind\_two\_molecules}\par
\setlength{\parindent}{5pt}\underline{\texttt{Arguments:}}\par
\setlength{\parindent}{10pt}\texttt{output\_path = CoPc\_ligand\_binding\_project/CoPc\_H\_thiophene.xyz}\par
\setlength{\parindent}{10pt}\texttt{core\_indices = [0]}\par
\setlength{\parindent}{10pt}\texttt{ligand\_file\_path = CoPc\_ligand\_binding\_project/thiophene.xyz}\par
\setlength{\parindent}{10pt}\texttt{core\_file\_path = CoPc\_ligand\_binding\_project/CoPc\_H.xyz}\par
\setlength{\parindent}{10pt}\texttt{ligand\_type = ligand}\par
\setlength{\parindent}{10pt}\texttt{ligand\_idx = 3}\par
\smallskip
\setlength{\parindent}{5pt}\underline{\texttt{Tool Name:}} \texttt{bind\_two\_molecules}\par
\setlength{\parindent}{5pt}\underline{\texttt{Arguments:}}\par
\setlength{\parindent}{10pt}\texttt{output\_path = CoPc\_ligand\_binding\_project/CoPc\_OH\_thiophene.xyz}\par
\setlength{\parindent}{10pt}\texttt{core\_indices = [0]}\par
\setlength{\parindent}{10pt}\texttt{ligand\_file\_path = CoPc\_ligand\_binding\_project/thiophene.xyz}\par
\setlength{\parindent}{10pt}\texttt{core\_file\_path = CoPc\_ligand\_binding\_project/CoPc\_OH.xyz}\par
\setlength{\parindent}{10pt}\texttt{ligand\_type = ligand}\par
\setlength{\parindent}{10pt}\texttt{ligand\_idx = 3}\par
\smallskip
\setlength{\parindent}{5pt}\underline{\texttt{Tool Name:}} \texttt{bind\_two\_molecules}\par
\setlength{\parindent}{5pt}\underline{\texttt{Arguments:}}\par
\setlength{\parindent}{10pt}\texttt{core\_indices = [0]}\par
\setlength{\parindent}{10pt}\texttt{output\_path = CoPc\_ligand\_binding\_project/CoPc\_H2O\_thiophene.xyz}\par
\setlength{\parindent}{10pt}\texttt{ligand\_file\_path = CoPc\_ligand\_binding\_project/thiophene.xyz}\par
\setlength{\parindent}{10pt}\texttt{core\_file\_path = CoPc\_ligand\_binding\_project/CoPc\_H2O.xyz}\par
\setlength{\parindent}{10pt}\texttt{ligand\_type = ligand}\par
\setlength{\parindent}{10pt}\texttt{ligand\_idx = 3}\par
\smallskip
\setlength{\parindent}{5pt}\underline{\texttt{Tool Name:}} \texttt{bind\_atom\_ligands\_library}\par
\setlength{\parindent}{5pt}\underline{\texttt{Arguments:}}\par
\setlength{\parindent}{10pt}\texttt{output\_path = CoPc\_ligand\_binding\_project/CoPc\_pyridine.xyz}\par
\setlength{\parindent}{10pt}\texttt{ligand\_name = Pyridine}\par
\setlength{\parindent}{10pt}\texttt{core\_element = Co}\par
\setlength{\parindent}{10pt}\texttt{core\_file\_path = CoPc\_ligand\_binding\_project/Co-Pc.xyz}\par
\smallskip
\setlength{\parindent}{5pt}\underline{\texttt{Tool Name:}} \texttt{bind\_atom\_ligands\_library}\par
\setlength{\parindent}{5pt}\underline{\texttt{Arguments:}}\par
\setlength{\parindent}{10pt}\texttt{ligand\_name = Pyridine}\par
\setlength{\parindent}{10pt}\texttt{output\_path = CoPc\_ligand\_binding\_project/CoPc\_CO2\_pyridine.xyz}\par
\setlength{\parindent}{10pt}\texttt{core\_element = Co}\par
\setlength{\parindent}{10pt}\texttt{core\_file\_path = CoPc\_ligand\_binding\_project/CoPc\_CO2.xyz}\par
\smallskip
\setlength{\parindent}{5pt}\underline{\texttt{Tool Name:}} \texttt{bind\_atom\_ligands\_library}\par
\setlength{\parindent}{5pt}\underline{\texttt{Arguments:}}\par
\setlength{\parindent}{10pt}\texttt{output\_path = CoPc\_ligand\_binding\_project/CoPc\_COOH\_pyridine.xyz}\par
\setlength{\parindent}{10pt}\texttt{ligand\_name = Pyridine}\par
\setlength{\parindent}{10pt}\texttt{core\_element = Co}\par
\setlength{\parindent}{10pt}\texttt{core\_file\_path = CoPc\_ligand\_binding\_project/CoPc\_COOH.xyz}\par
\smallskip
\setlength{\parindent}{5pt}\underline{\texttt{Tool Name:}} \texttt{bind\_atom\_ligands\_library}\par
\setlength{\parindent}{5pt}\underline{\texttt{Arguments:}}\par
\setlength{\parindent}{10pt}\texttt{output\_path = CoPc\_ligand\_binding\_project/CoPc\_CO\_pyridine.xyz}\par
\setlength{\parindent}{10pt}\texttt{ligand\_name = Pyridine}\par
\setlength{\parindent}{10pt}\texttt{core\_element = Co}\par
\setlength{\parindent}{10pt}\texttt{core\_file\_path = CoPc\_ligand\_binding\_project/CoPc\_CO.xyz}\par
\smallskip
\setlength{\parindent}{5pt}\underline{\texttt{Tool Name:}} \texttt{bind\_atom\_ligands\_library}\par
\setlength{\parindent}{5pt}\underline{\texttt{Arguments:}}\par
\setlength{\parindent}{10pt}\texttt{ligand\_name = Pyridine}\par
\setlength{\parindent}{10pt}\texttt{output\_path = CoPc\_ligand\_binding\_project/CoPc\_H\_pyridine.xyz}\par
\setlength{\parindent}{10pt}\texttt{core\_element = Co}\par
\setlength{\parindent}{10pt}\texttt{core\_file\_path = CoPc\_ligand\_binding\_project/CoPc\_H.xyz}\par
\smallskip
\setlength{\parindent}{5pt}\underline{\texttt{Tool Name:}} \texttt{bind\_atom\_ligands\_library}\par
\setlength{\parindent}{5pt}\underline{\texttt{Arguments:}}\par
\setlength{\parindent}{10pt}\texttt{ligand\_name = Pyridine}\par
\setlength{\parindent}{10pt}\texttt{output\_path = CoPc\_ligand\_binding\_project/CoPc\_OH\_pyridine.xyz}\par
\setlength{\parindent}{10pt}\texttt{core\_element = Co}\par
\setlength{\parindent}{10pt}\texttt{core\_file\_path = CoPc\_ligand\_binding\_project/CoPc\_OH.xyz}\par
\smallskip
\setlength{\parindent}{5pt}\underline{\texttt{Tool Name:}} \texttt{bind\_atom\_ligands\_library}\par
\setlength{\parindent}{5pt}\underline{\texttt{Arguments:}}\par
\setlength{\parindent}{10pt}\texttt{ligand\_name = Pyridine}\par
\setlength{\parindent}{10pt}\texttt{output\_path = CoPc\_ligand\_binding\_project/CoPc\_H2O\_pyridine.xyz}\par
\setlength{\parindent}{10pt}\texttt{core\_element = Co}\par
\setlength{\parindent}{10pt}\texttt{core\_file\_path = CoPc\_ligand\_binding\_project/CoPc\_H2O.xyz}\par
\smallskip
\setlength{\parindent}{5pt}\underline{\texttt{Tool Name:}} \texttt{bind\_atom\_ligands\_library}\par
\setlength{\parindent}{5pt}\underline{\texttt{Arguments:}}\par
\setlength{\parindent}{10pt}\texttt{ligand\_name = Cl}\par
\setlength{\parindent}{10pt}\texttt{output\_path = CoPc\_ligand\_binding\_project/CoPc\_Cl.xyz}\par
\setlength{\parindent}{10pt}\texttt{core\_element = Co}\par
\setlength{\parindent}{10pt}\texttt{core\_file\_path = CoPc\_ligand\_binding\_project/Co-Pc.xyz}\par
\smallskip
\setlength{\parindent}{5pt}\underline{\texttt{Tool Name:}} \texttt{bind\_atom\_ligands\_library}\par
\setlength{\parindent}{5pt}\underline{\texttt{Arguments:}}\par
\setlength{\parindent}{10pt}\texttt{ligand\_name = Cl}\par
\setlength{\parindent}{10pt}\texttt{output\_path = CoPc\_ligand\_binding\_project/CoPc\_CO2\_Cl.xyz}\par
\setlength{\parindent}{10pt}\texttt{core\_element = Co}\par
\setlength{\parindent}{10pt}\texttt{core\_file\_path = CoPc\_ligand\_binding\_project/CoPc\_CO2.xyz}\par
\smallskip
\setlength{\parindent}{5pt}\underline{\texttt{Tool Name:}} \texttt{bind\_atom\_ligands\_library}\par
\setlength{\parindent}{5pt}\underline{\texttt{Arguments:}}\par
\setlength{\parindent}{10pt}\texttt{output\_path = CoPc\_ligand\_binding\_project/CoPc\_COOH\_Cl.xyz}\par
\setlength{\parindent}{10pt}\texttt{ligand\_name = Cl}\par
\setlength{\parindent}{10pt}\texttt{core\_element = Co}\par
\setlength{\parindent}{10pt}\texttt{core\_file\_path = CoPc\_ligand\_binding\_project/CoPc\_COOH.xyz}\par
\smallskip
\setlength{\parindent}{5pt}\underline{\texttt{Tool Name:}} \texttt{bind\_atom\_ligands\_library}\par
\setlength{\parindent}{5pt}\underline{\texttt{Arguments:}}\par
\setlength{\parindent}{10pt}\texttt{output\_path = CoPc\_ligand\_binding\_project/CoPc\_CO\_Cl.xyz}\par
\setlength{\parindent}{10pt}\texttt{ligand\_name = Cl}\par
\setlength{\parindent}{10pt}\texttt{core\_element = Co}\par
\setlength{\parindent}{10pt}\texttt{core\_file\_path = CoPc\_ligand\_binding\_project/CoPc\_CO.xyz}\par
\smallskip
\setlength{\parindent}{5pt}\underline{\texttt{Tool Name:}} \texttt{bind\_atom\_ligands\_library}\par
\setlength{\parindent}{5pt}\underline{\texttt{Arguments:}}\par
\setlength{\parindent}{10pt}\texttt{output\_path = CoPc\_ligand\_binding\_project/CoPc\_H\_Cl.xyz}\par
\setlength{\parindent}{10pt}\texttt{ligand\_name = Cl}\par
\setlength{\parindent}{10pt}\texttt{core\_element = Co}\par
\setlength{\parindent}{10pt}\texttt{core\_file\_path = CoPc\_ligand\_binding\_project/CoPc\_H.xyz}\par
\smallskip
\setlength{\parindent}{5pt}\underline{\texttt{Tool Name:}} \texttt{bind\_atom\_ligands\_library}\par
\setlength{\parindent}{5pt}\underline{\texttt{Arguments:}}\par
\setlength{\parindent}{10pt}\texttt{ligand\_name = Cl}\par
\setlength{\parindent}{10pt}\texttt{output\_path = CoPc\_ligand\_binding\_project/CoPc\_OH\_Cl.xyz}\par
\setlength{\parindent}{10pt}\texttt{core\_element = Co}\par
\setlength{\parindent}{10pt}\texttt{core\_file\_path = CoPc\_ligand\_binding\_project/CoPc\_OH.xyz}\par
\smallskip
\setlength{\parindent}{5pt}\underline{\texttt{Tool Name:}} \texttt{bind\_atom\_ligands\_library}\par
\setlength{\parindent}{5pt}\underline{\texttt{Arguments:}}\par
\setlength{\parindent}{10pt}\texttt{output\_path = CoPc\_ligand\_binding\_project/CoPc\_H2O\_Cl.xyz}\par
\setlength{\parindent}{10pt}\texttt{ligand\_name = Cl}\par
\setlength{\parindent}{10pt}\texttt{core\_element = Co}\par
\setlength{\parindent}{10pt}\texttt{core\_file\_path = CoPc\_ligand\_binding\_project/CoPc\_H2O.xyz}\par
\smallskip
\end{tcolorbox}

\setlength{\parindent}{5pt} \robot \hspace{2pt} \textbf{Estructural}

\begin{tcolorbox}[
    colback=matterbg2,
    colframe=mattergreen1,
    width=\textwidth,
    arc=2mm,
    boxrule=0.2mm,
    leftrule=0.2mm, rightrule=0.2mm,
    toprule=0.2mm, bottomrule=0.2mm,
    enhanced,
    breakable
]
\textbf{Tool used:}

\setlength{\parindent}{5pt}\underline{\texttt{Tool Name:}} \texttt{organic\_molecules\_xyz\_generation}\par
\setlength{\parindent}{5pt}\underline{\texttt{Arguments:}}\par
\setlength{\parindent}{10pt}\texttt{filenames = ["CoPc\_ligand\_binding\_project/pyridine.xyz"]}\par
\setlength{\parindent}{10pt}\texttt{smiles\_list = ["n1ccccc1"]}\par
\smallskip
\end{tcolorbox}

\setlength{\parindent}{5pt} \robot \hspace{2pt} \textbf{Estructural}

\begin{tcolorbox}[
    colback=matterbg2,
    colframe=mattergreen1,
    width=\textwidth,
    arc=2mm,
    boxrule=0.2mm,
    leftrule=0.2mm, rightrule=0.2mm,
    toprule=0.2mm, bottomrule=0.2mm,
    enhanced,
    breakable
]
\textbf{Tool used:}

\setlength{\parindent}{5pt}\underline{\texttt{Tool Name:}} \texttt{get\_atomic\_neighbors}\par
\setlength{\parindent}{5pt}\underline{\texttt{Arguments:}}\par
\setlength{\parindent}{10pt}\texttt{target = N}\par
\setlength{\parindent}{10pt}\texttt{file\_path = CoPc\_ligand\_binding\_project/pyridine.xyz}\par
\smallskip
\end{tcolorbox}

\setlength{\parindent}{5pt} \robot \hspace{2pt} \textbf{Estructural}

\begin{tcolorbox}[
    colback=matterbg2,
    colframe=mattergreen1,
    width=\textwidth,
    arc=2mm,
    boxrule=0.2mm,
    leftrule=0.2mm, rightrule=0.2mm,
    toprule=0.2mm, bottomrule=0.2mm,
    enhanced,
    breakable
]
\textbf{Tool used:}

\setlength{\parindent}{5pt}\underline{\texttt{Tool Name:}} \texttt{bind\_two\_molecules}\par
\setlength{\parindent}{5pt}\underline{\texttt{Arguments:}}\par
\setlength{\parindent}{10pt}\texttt{output\_path = CoPc\_ligand\_binding\_project/CoPc\_pyridine.xyz}\par
\setlength{\parindent}{10pt}\texttt{core\_indices = [0]}\par
\setlength{\parindent}{10pt}\texttt{ligand\_file\_path = CoPc\_ligand\_binding\_project/pyridine.xyz}\par
\setlength{\parindent}{10pt}\texttt{core\_file\_path = CoPc\_ligand\_binding\_project/Co-Pc.xyz}\par
\setlength{\parindent}{10pt}\texttt{ligand\_type = ligand}\par
\setlength{\parindent}{10pt}\texttt{ligand\_idx = 0}\par
\smallskip
\setlength{\parindent}{5pt}\underline{\texttt{Tool Name:}} \texttt{bind\_two\_molecules}\par
\setlength{\parindent}{5pt}\underline{\texttt{Arguments:}}\par
\setlength{\parindent}{10pt}\texttt{core\_indices = [0]}\par
\setlength{\parindent}{10pt}\texttt{output\_path = CoPc\_ligand\_binding\_project/CoPc\_CO2\_pyridine.xyz}\par
\setlength{\parindent}{10pt}\texttt{ligand\_file\_path = CoPc\_ligand\_binding\_project/pyridine.xyz}\par
\setlength{\parindent}{10pt}\texttt{core\_file\_path = CoPc\_ligand\_binding\_project/CoPc\_CO2.xyz}\par
\setlength{\parindent}{10pt}\texttt{ligand\_type = ligand}\par
\setlength{\parindent}{10pt}\texttt{ligand\_idx = 0}\par
\smallskip
\setlength{\parindent}{5pt}\underline{\texttt{Tool Name:}} \texttt{bind\_two\_molecules}\par
\setlength{\parindent}{5pt}\underline{\texttt{Arguments:}}\par
\setlength{\parindent}{10pt}\texttt{output\_path = CoPc\_ligand\_binding\_project/CoPc\_COOH\_pyridine.xyz}\par
\setlength{\parindent}{10pt}\texttt{core\_indices = [0]}\par
\setlength{\parindent}{10pt}\texttt{ligand\_file\_path = CoPc\_ligand\_binding\_project/pyridine.xyz}\par
\setlength{\parindent}{10pt}\texttt{ligand\_idx = 0}\par
\setlength{\parindent}{10pt}\texttt{ligand\_type = ligand}\par
\setlength{\parindent}{10pt}\texttt{core\_file\_path = CoPc\_ligand\_binding\_project/CoPc\_COOH.xyz}\par
\smallskip
\setlength{\parindent}{5pt}\underline{\texttt{Tool Name:}} \texttt{bind\_two\_molecules}\par
\setlength{\parindent}{5pt}\underline{\texttt{Arguments:}}\par
\setlength{\parindent}{10pt}\texttt{output\_path = CoPc\_ligand\_binding\_project/CoPc\_CO\_pyridine.xyz}\par
\setlength{\parindent}{10pt}\texttt{core\_indices = [0]}\par
\setlength{\parindent}{10pt}\texttt{ligand\_file\_path = CoPc\_ligand\_binding\_project/pyridine.xyz}\par
\setlength{\parindent}{10pt}\texttt{core\_file\_path = CoPc\_ligand\_binding\_project/CoPc\_CO.xyz}\par
\setlength{\parindent}{10pt}\texttt{ligand\_type = ligand}\par
\setlength{\parindent}{10pt}\texttt{ligand\_idx = 0}\par
\smallskip
\setlength{\parindent}{5pt}\underline{\texttt{Tool Name:}} \texttt{bind\_two\_molecules}\par
\setlength{\parindent}{5pt}\underline{\texttt{Arguments:}}\par
\setlength{\parindent}{10pt}\texttt{core\_indices = [0]}\par
\setlength{\parindent}{10pt}\texttt{output\_path = CoPc\_ligand\_binding\_project/CoPc\_H\_pyridine.xyz}\par
\setlength{\parindent}{10pt}\texttt{ligand\_file\_path = CoPc\_ligand\_binding\_project/pyridine.xyz}\par
\setlength{\parindent}{10pt}\texttt{core\_file\_path = CoPc\_ligand\_binding\_project/CoPc\_H.xyz}\par
\setlength{\parindent}{10pt}\texttt{ligand\_type = ligand}\par
\setlength{\parindent}{10pt}\texttt{ligand\_idx = 0}\par
\smallskip
\setlength{\parindent}{5pt}\underline{\texttt{Tool Name:}} \texttt{bind\_two\_molecules}\par
\setlength{\parindent}{5pt}\underline{\texttt{Arguments:}}\par
\setlength{\parindent}{10pt}\texttt{output\_path = CoPc\_ligand\_binding\_project/CoPc\_OH\_pyridine.xyz}\par
\setlength{\parindent}{10pt}\texttt{core\_indices = [0]}\par
\setlength{\parindent}{10pt}\texttt{ligand\_file\_path = CoPc\_ligand\_binding\_project/pyridine.xyz}\par
\setlength{\parindent}{10pt}\texttt{core\_file\_path = CoPc\_ligand\_binding\_project/CoPc\_OH.xyz}\par
\setlength{\parindent}{10pt}\texttt{ligand\_type = ligand}\par
\setlength{\parindent}{10pt}\texttt{ligand\_idx = 0}\par
\smallskip
\setlength{\parindent}{5pt}\underline{\texttt{Tool Name:}} \texttt{bind\_two\_molecules}\par
\setlength{\parindent}{5pt}\underline{\texttt{Arguments:}}\par
\setlength{\parindent}{10pt}\texttt{core\_indices = [0]}\par
\setlength{\parindent}{10pt}\texttt{output\_path = CoPc\_ligand\_binding\_project/CoPc\_H2O\_pyridine.xyz}\par
\setlength{\parindent}{10pt}\texttt{ligand\_file\_path = CoPc\_ligand\_binding\_project/pyridine.xyz}\par
\setlength{\parindent}{10pt}\texttt{ligand\_idx = 0}\par
\setlength{\parindent}{10pt}\texttt{ligand\_type = ligand}\par
\setlength{\parindent}{10pt}\texttt{core\_file\_path = CoPc\_ligand\_binding\_project/CoPc\_H2O.xyz}\par
\smallskip
\end{tcolorbox}

\setlength{\parindent}{5pt} \robot \hspace{2pt} \textbf{Estructural}

\begin{tcolorbox}[
    colback=matterbg2,
    colframe=mattergreen1,
    width=\textwidth,
    arc=2mm,
    boxrule=0.2mm,
    leftrule=0.2mm, rightrule=0.2mm,
    toprule=0.2mm, bottomrule=0.2mm,
    enhanced,
    breakable
]
\textbf{Action:}

\begin{markdown}
I have successfully generated all the requested structures to explore the axial ligand effect.

**Task Summary:**
For each of the 7 core structures (original Co-Pc + 6 derivatives), I attached three different axial ligands: Thiophene, Pyridine, and Chloride (Cl), resulting in 21 new structures.

**Execution Details:**
1.  **Thiophene:** Generated `thiophene.xyz` (SMILES: `c1ccsc1`), identified the Sulfur atom (index 3), and bound it to the Cobalt atom in each core structure.
2.  **Pyridine:** Generated `pyridine.xyz` (SMILES: `n1ccccc1`), identified the Nitrogen atom (index 0), and bound it to the Cobalt atom in each core structure.
3.  **Cl:** Used the `bind_atom_ligands_library` tool to bind a Chloride atom to the Cobalt atom in each core structure.

**Generated Files (in `CoPc_ligand_binding_project`):**

*   **Thiophene Series:**
    *   `CoPc_thiophene.xyz`
    *   `CoPc_CO2_thiophene.xyz`
    *   `CoPc_COOH_thiophene.xyz`
    *   `CoPc_CO_thiophene.xyz`
    *   `CoPc_H_thiophene.xyz`
    *   `CoPc_OH_thiophene.xyz`
    *   `CoPc_H2O_thiophene.xyz`

*   **Pyridine Series:**
    *   `CoPc_pyridine.xyz`
    *   `CoPc_CO2_pyridine.xyz`
    *   `CoPc_COOH_pyridine.xyz`
    *   `CoPc_CO_pyridine.xyz`
    *   `CoPc_H_pyridine.xyz`
    *   `CoPc_OH_pyridine.xyz`
    *   `CoPc_H2O_pyridine.xyz`

*   **Chloride (Cl) Series:**
    *   `CoPc_Cl.xyz`
    *   `CoPc_CO2_Cl.xyz`
    *   `CoPc_COOH_Cl.xyz`
    *   `CoPc_CO_Cl.xyz`
    *   `CoPc_H_Cl.xyz`
    *   `CoPc_OH_Cl.xyz`
    *   `CoPc_H2O_Cl.xyz`

All files are neatly organized in the `CoPc_ligand_binding_project` folder.
\end{markdown}

\end{tcolorbox}
